# Supplementary material for: Online deforestation detection
Source: arXiv:1704.00829 source file (2017-04-03)
Supplement: Supplementary file 1 [file 7A_AppendixSites.tex]

\chapter{Sites} \label{app:sites}

We include the figures for the remaining 7 sites not included in section \ref{s:studyArea}.  

\subsection{Forest to water sites}

		\subsubsection{Jalisco164}
		
      	 \begin{figure}[H]  %--- Picture 'H'ere, 'B'ottom or 'T'op; '!' Try to
      	                     %impose your will to LaTeX
      	  % \centering 
  
      	   \begin{subfigure}{.5\textwidth}
      	     \centering
      	 	\includegraphics[width=0.7\textwidth]{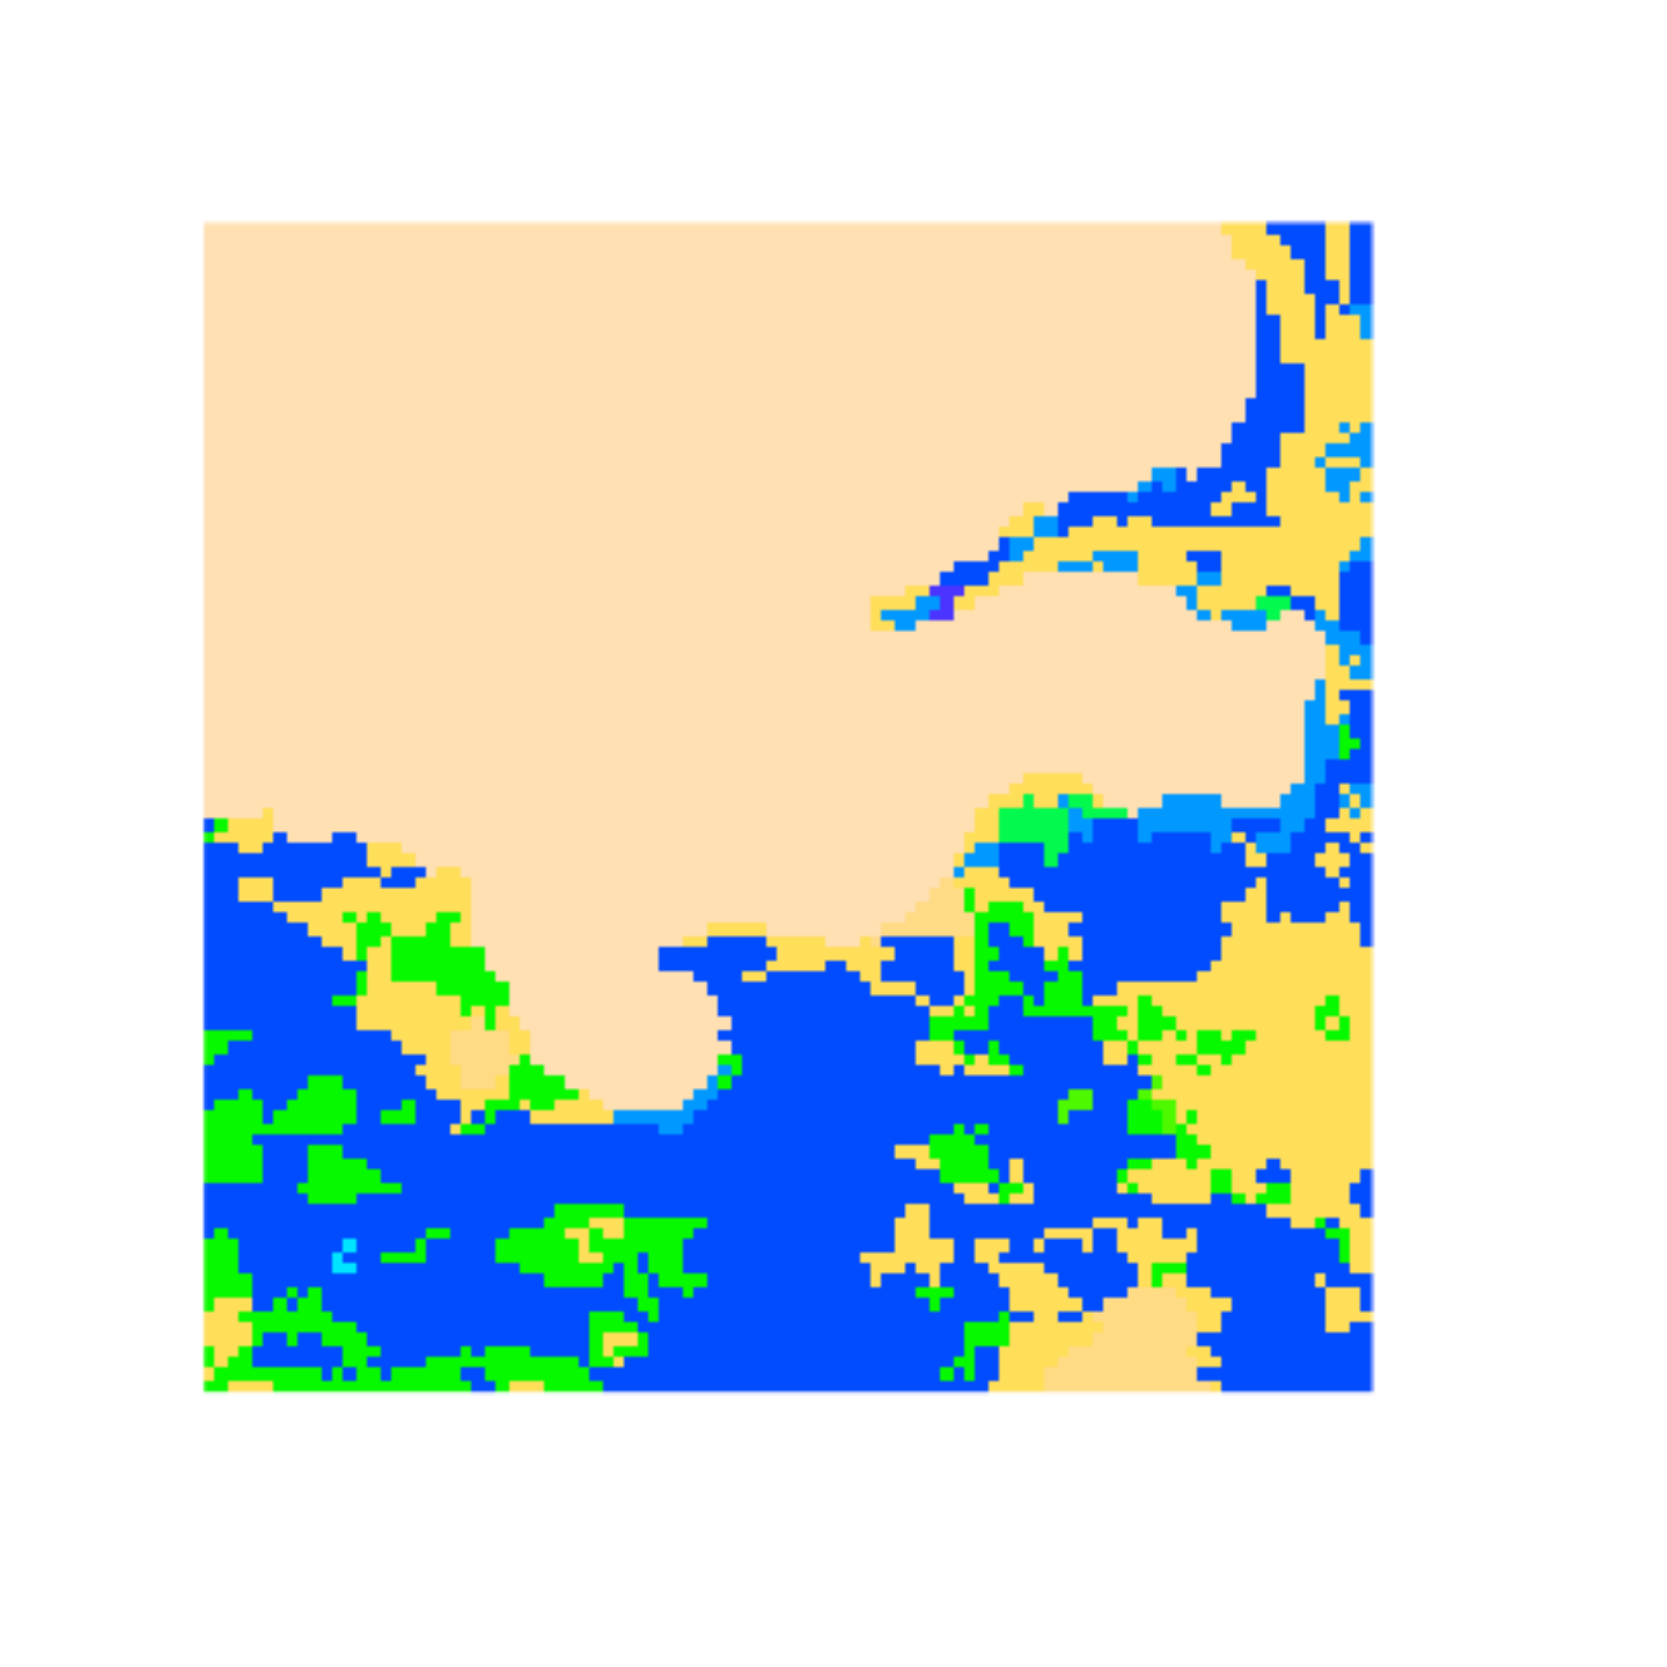} 
      	     \caption{Land-use 2005}
      	     \label{fig:sfig1a}
      	   \end{subfigure}%
      	   \begin{subfigure}{.5\textwidth}
      	     \centering
      	     \includegraphics[width=0.7\textwidth]{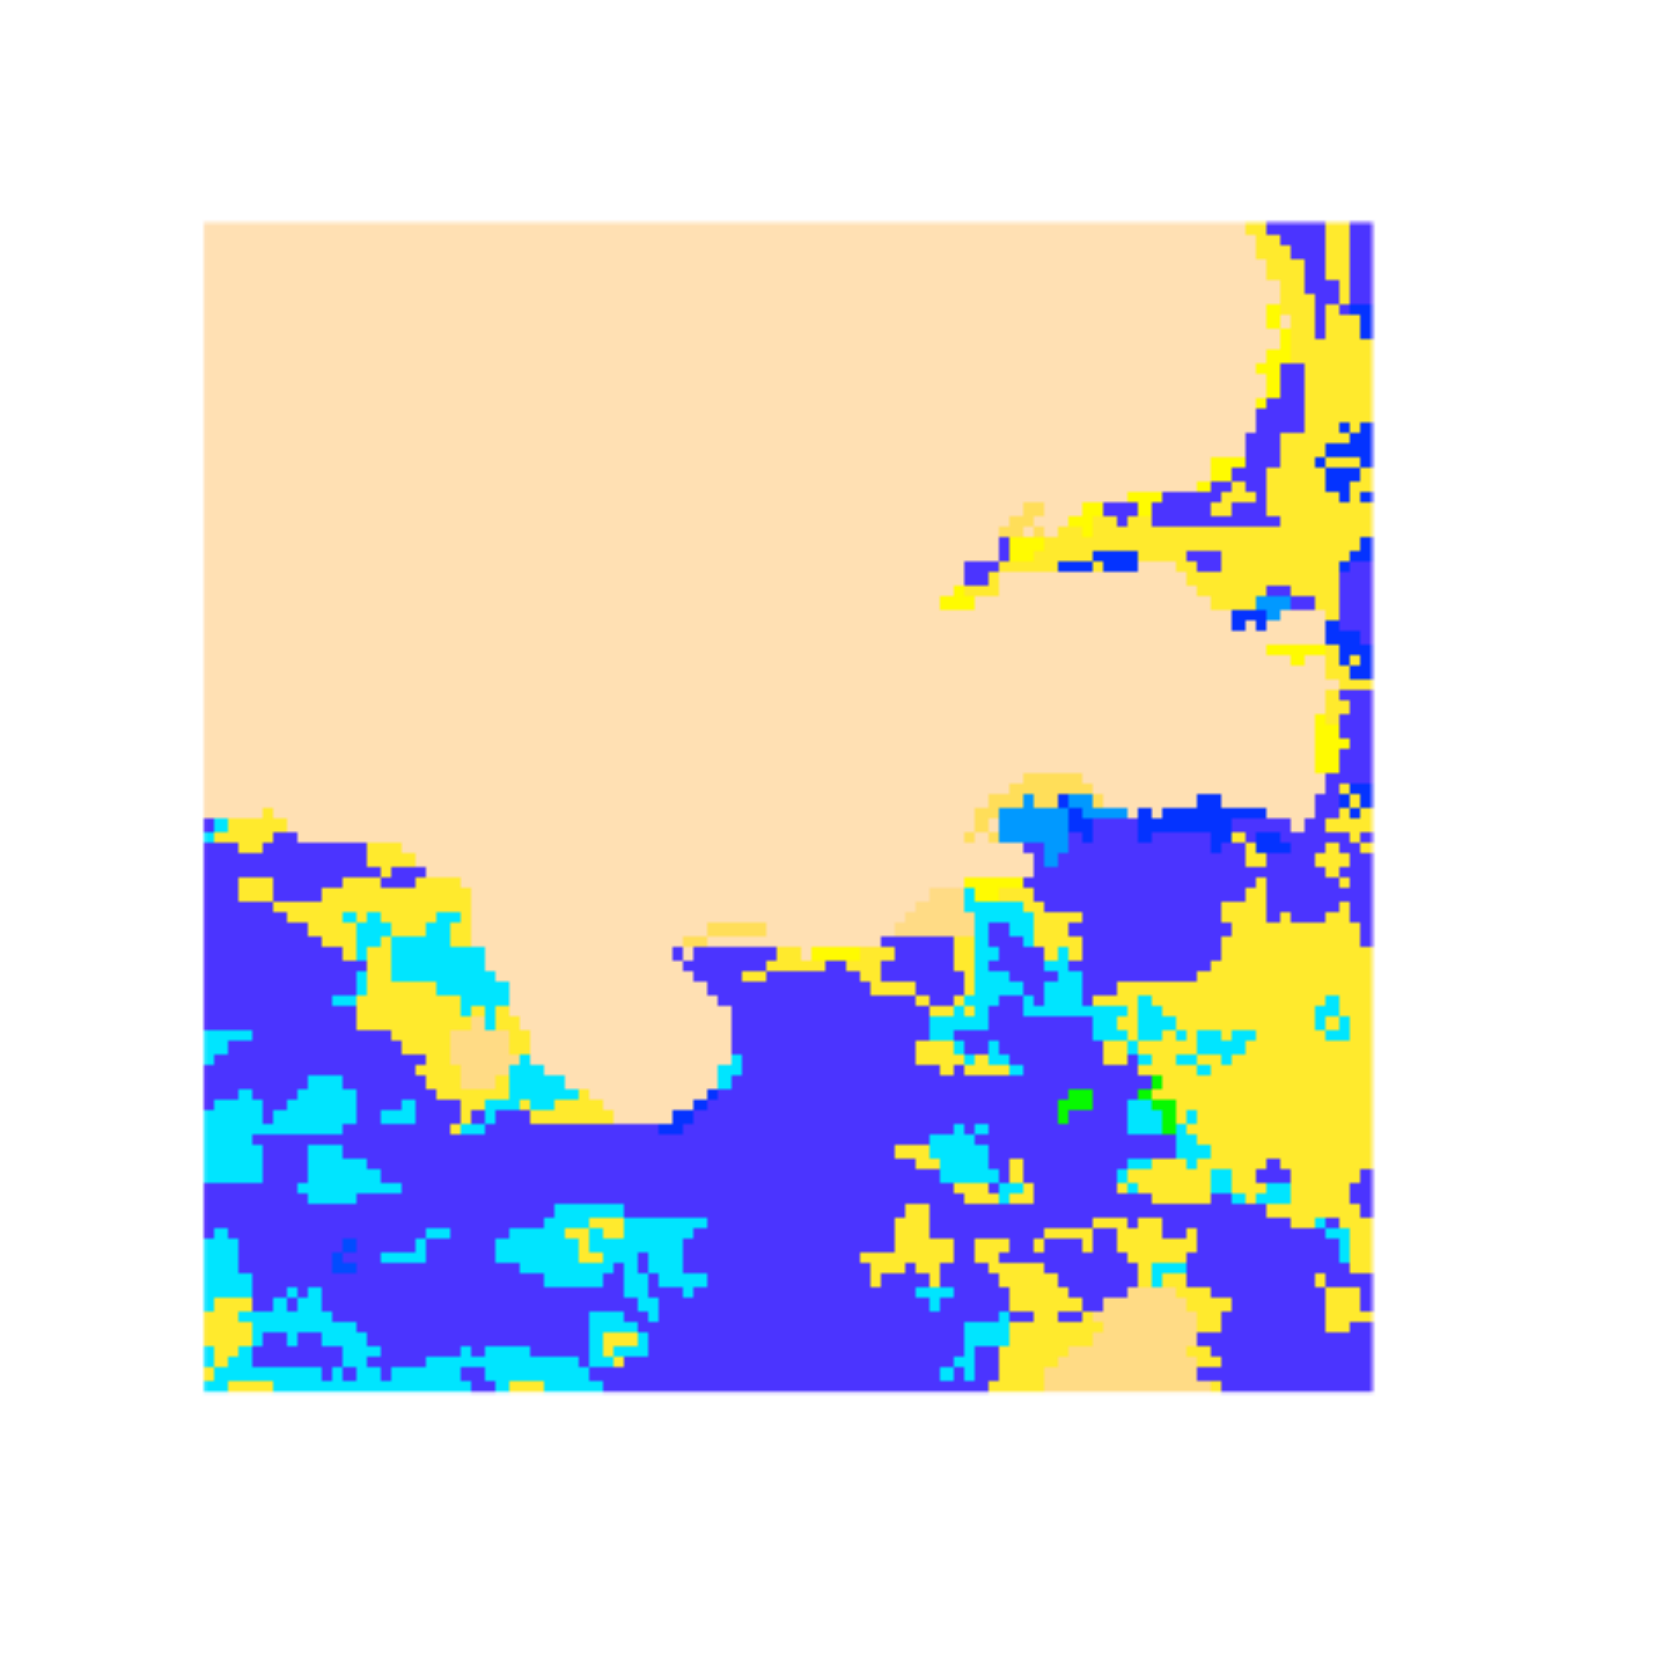}
      	     \caption{Land-use 2010}
      	     \label{fig:sfig1b}
      	   \end{subfigure}
      	   \begin{subfigure}{.4\textwidth}
      	     \centering
      	     \includegraphics[width=0.9\textwidth]{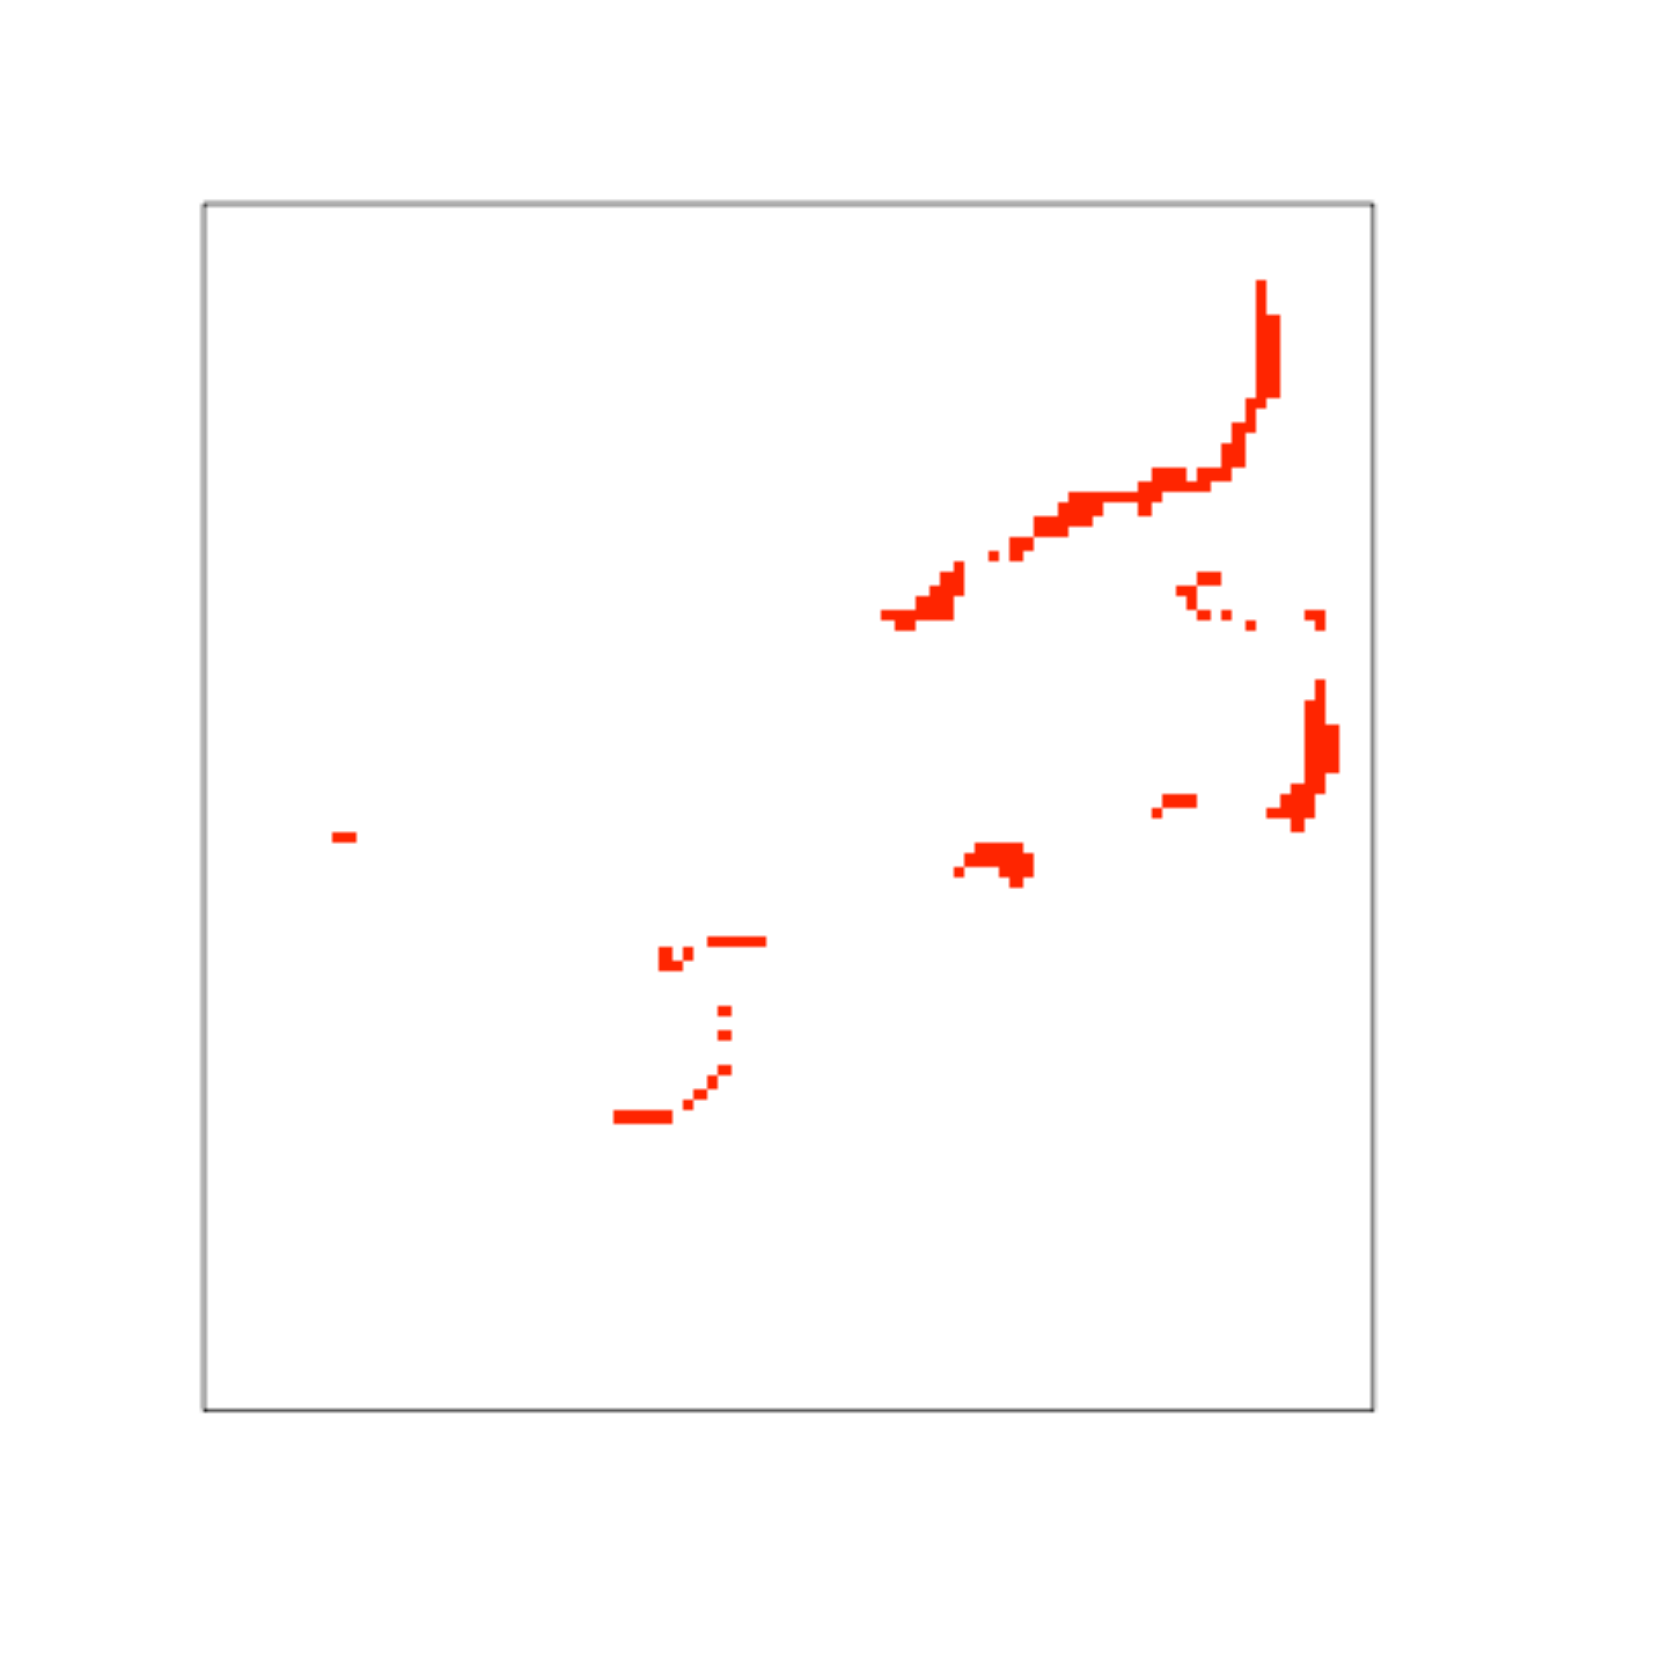}
      	     \caption{Deforestation 2005-2010}
      	     \label{fig:sfig1c}
      	   \end{subfigure}
      	   \begin{subfigure}{.4\textwidth}
      	     \centering
      	     \includegraphics[width=0.9\textwidth]{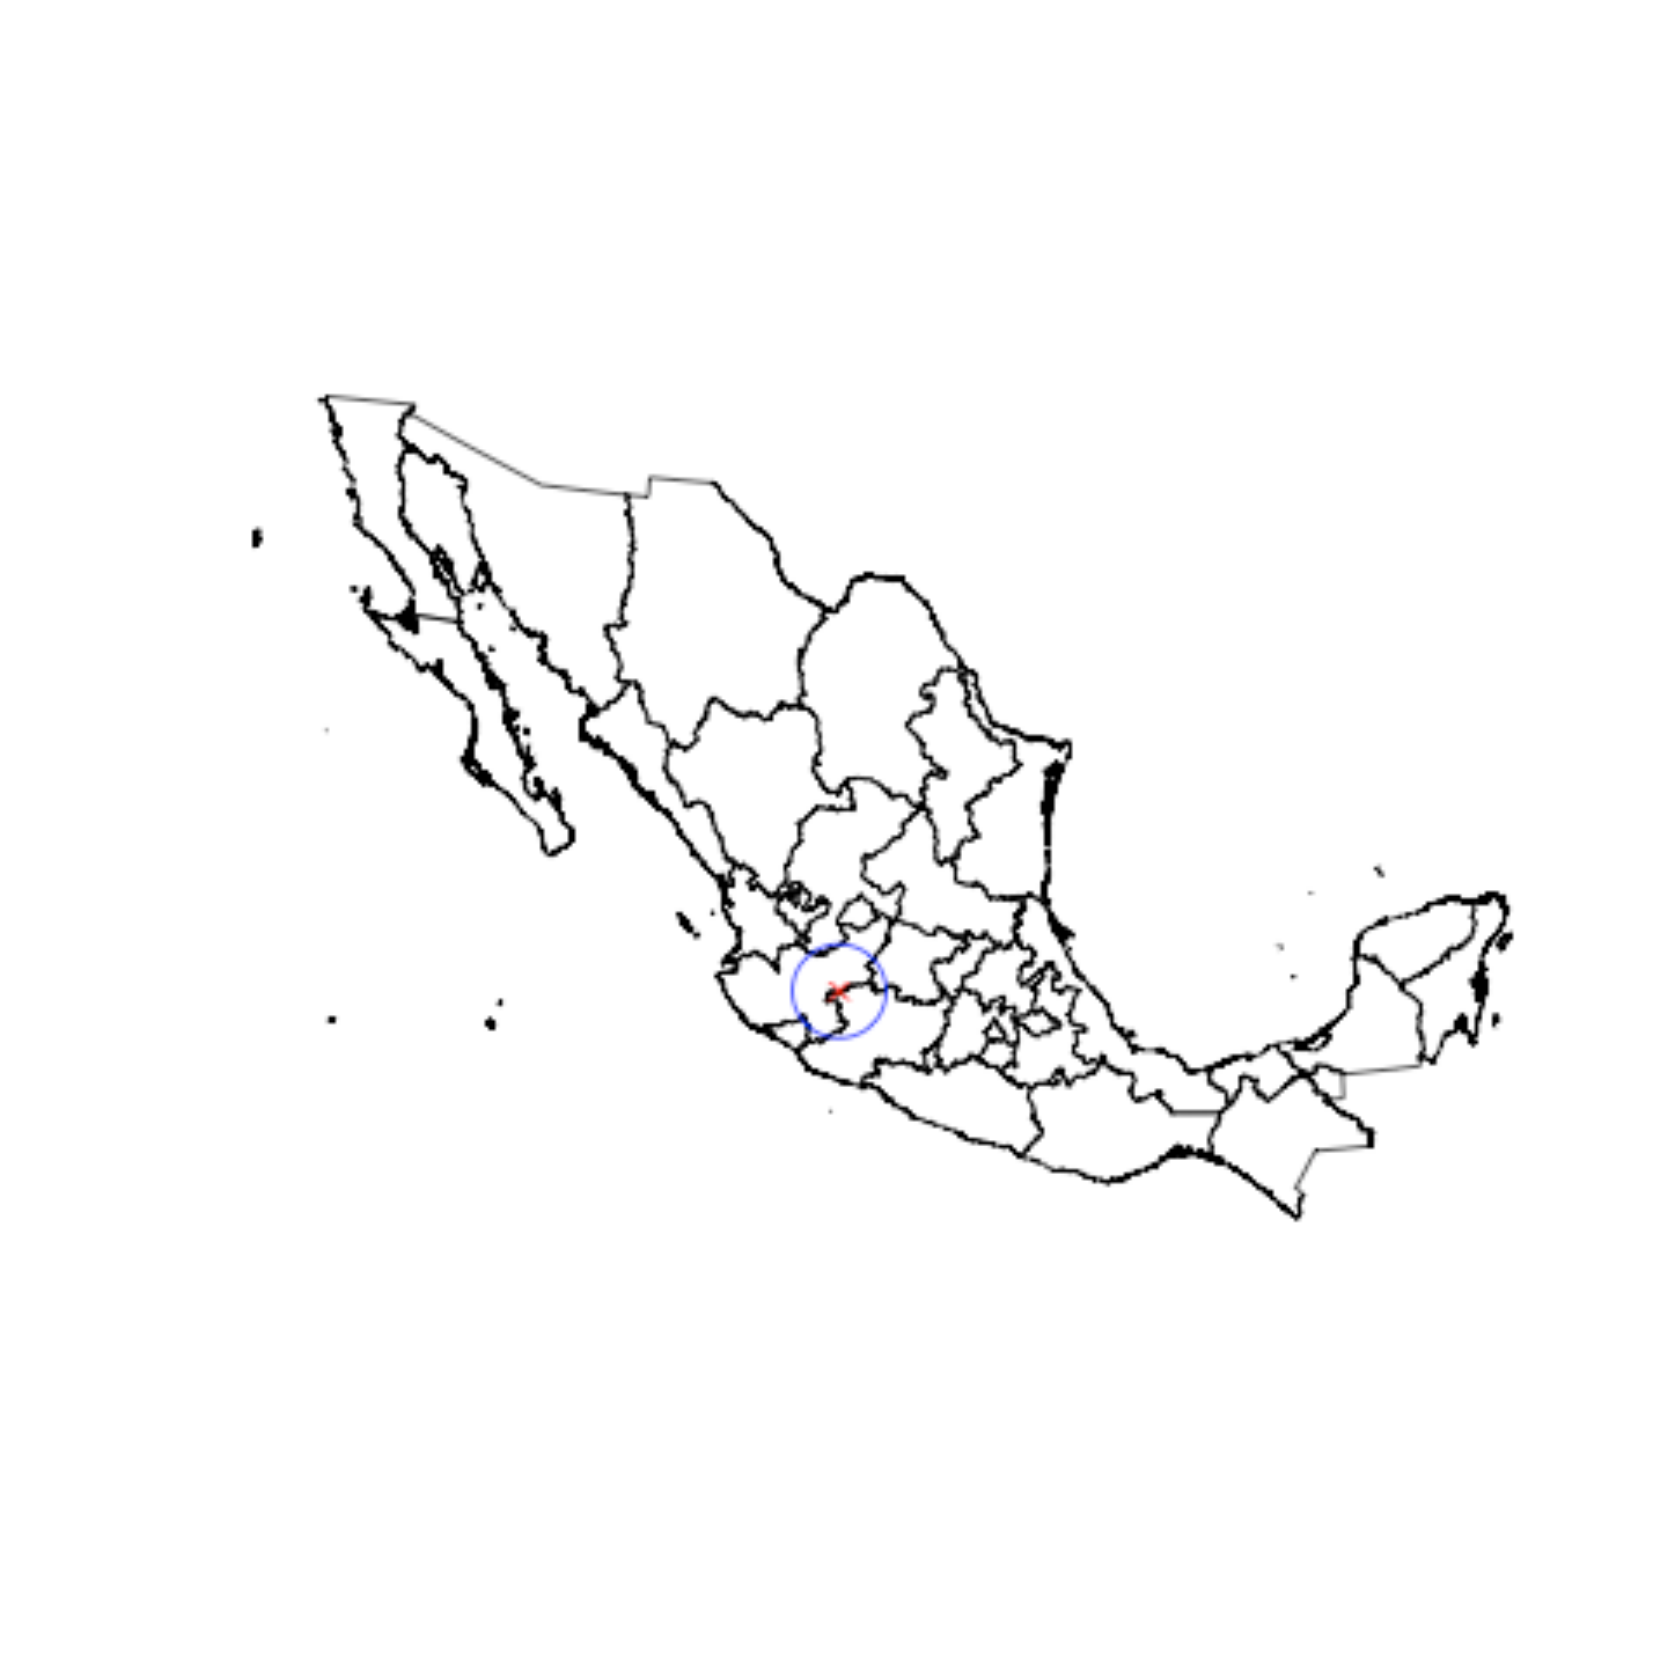}
      	     \caption{Location}
      	     \label{fig:sfig1d}
      	   \end{subfigure}   
         \begin{subfigure}{.5\textwidth}
           \centering
           \includegraphics[width=1\textwidth]{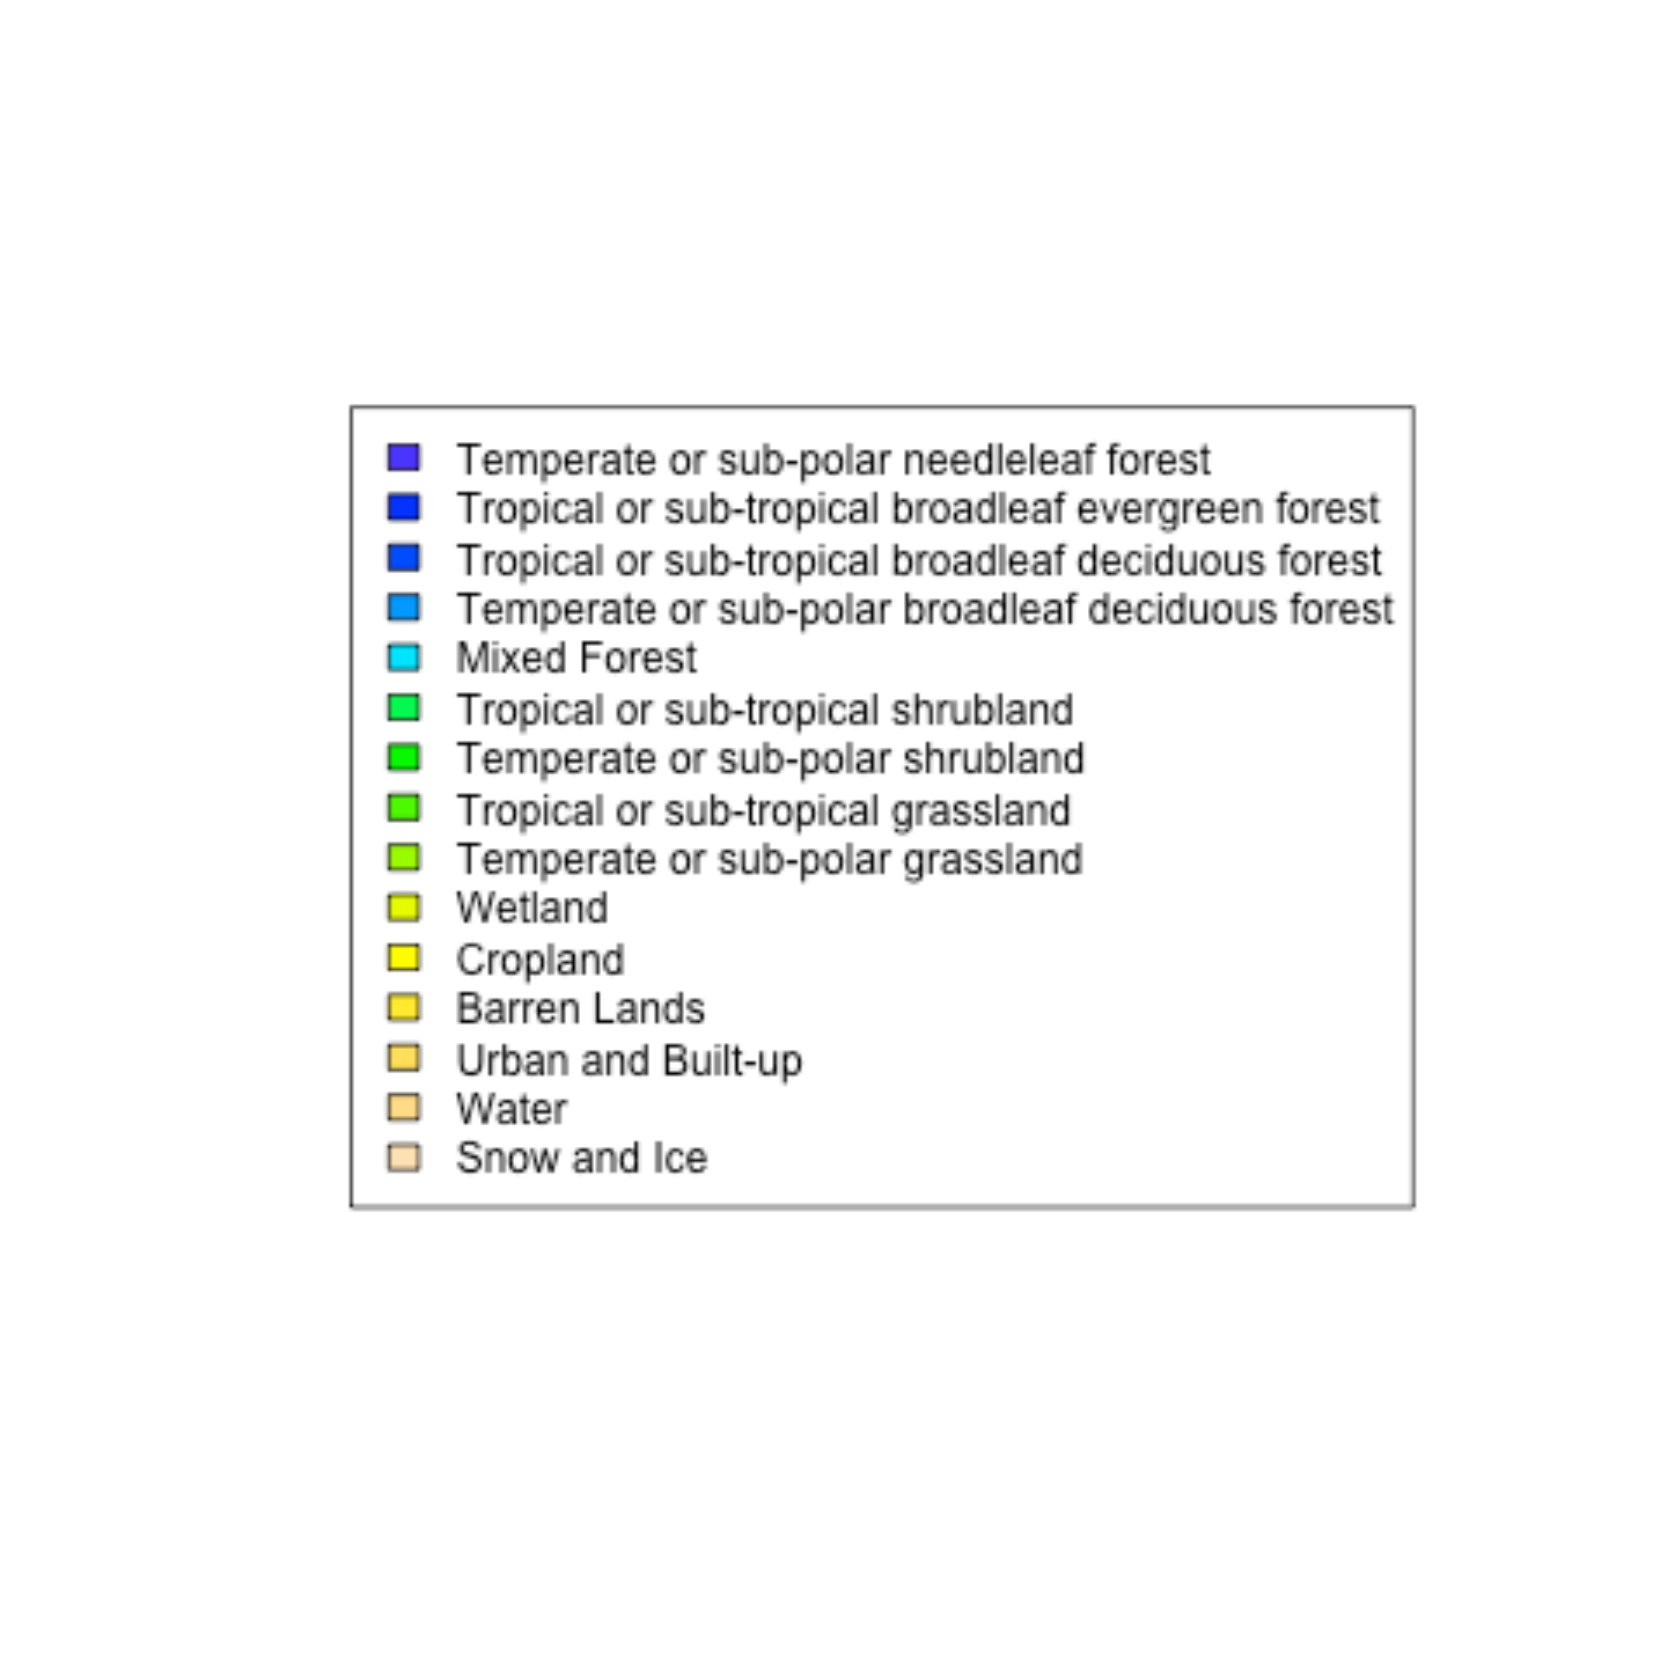}
           \caption{Land use legend}
           \label{fig:legend}
         \end{subfigure}
      	   %%         --- .5\textwidth stands for 50% of text width
      	   \caption[NALCMS land-use classification of Jalisco164 site, 2005 and 2010 at 250m resolution.]%<<-- Legend for the list of figures at the beginning of you thesis
      	   {NALCMS land-use classification of Jalisco164 site, 2005 and 2010 at 250m resolution.}% legend displayed below the graph.
      	   \label{fig:landUseJalisco164}
      	 \end{figure}
		
   		\begin{center}
   			\footnotesize\addtolength{\tabcolsep}{-2pt}
   			% latex table generated in R 3.3.1 by xtable 1.8-2 package
% Sun Mar  5 15:55:50 2017
\begin{table}[ht]
\centering
\begingroup\tiny
\begin{tabular}{rrrrrrrrrrrrrrrrrrrrr}
  & \begin{sideways} Temperate or sub-polar needleleaf forest \end{sideways} & \begin{sideways} Sub-polar taiga needleleaf forest \end{sideways} & \begin{sideways} Tropical or sub-tropical broadleaf evergreen forest \end{sideways} & \begin{sideways} Tropical or sub-tropical broadleaf deciduous forest \end{sideways} & \begin{sideways} Temperate or sub-polar broadleaf deciduous forest \end{sideways} & \begin{sideways} Mixed Forest \end{sideways} & \begin{sideways} Tropical or sub-tropical shrubland \end{sideways} & \begin{sideways} Temperate or sub-polar shrubland \end{sideways} & \begin{sideways} Tropical or sub-tropical grassland \end{sideways} & \begin{sideways} Temperate or sub-polar grassland \end{sideways} & \begin{sideways} Sub-polar or polar shrubland-lichen-moss \end{sideways} & \begin{sideways} Sub-polar or polar grassland-lichen-moss \end{sideways} & \begin{sideways} Sub-polar or polar barren-lichen-moss \end{sideways} & \begin{sideways} Wetland \end{sideways} & \begin{sideways} Cropland \end{sideways} & \begin{sideways} Barren Lands \end{sideways} & \begin{sideways} Urban and Built-up \end{sideways} & \begin{sideways} Water \end{sideways} & \begin{sideways} Snow and Ice \end{sideways} & \begin{sideways} Total \end{sideways} \\ 
  \hline
Temperate or sub-polar needleleaf forest &    0 &    0 &    0 &    0 &    0 &    0 &    0 &    0 &    0 &    0 &    0 &    0 &    0 &    2 &    0 &    0 &    0 &    4 &    0 &    6 \\ 
  Sub-polar taiga needleleaf forest &    0 &    0 &    0 &    0 &    0 &    0 &    0 &    0 &    0 &    0 &    0 &    0 &    0 &    0 &    0 &    0 &    0 &    0 &    0 &    0 \\ 
  Tropical or sub-tropical broadleaf evergreen forest &    0 &    0 &    0 &    0 &    0 &    0 &    0 &    0 &    0 &    0 &    0 &    0 &    0 &    0 &    0 &    0 &    0 &    0 &    0 &    0 \\ 
  Tropical or sub-tropical broadleaf deciduous forest &    0 &    0 &    0 & 2631 &    0 &    0 &    0 &    0 &    0 &    0 &    0 &    0 &    0 &   21 &    1 &    0 &    0 &   58 &    0 & 2711 \\ 
  Temperate or sub-polar broadleaf deciduous forest &    0 &    0 &    0 &    3 &   96 &    0 &    0 &    1 &    0 &    0 &    0 &    0 &    0 &   12 &    2 &    1 &    0 &   62 &    0 &  177 \\ 
  Mixed Forest &    0 &    0 &    0 &    0 &    0 &    4 &    0 &    0 &    0 &    0 &    0 &    0 &    0 &    0 &    0 &    0 &    0 &    0 &    0 &    4 \\ 
   \hline
Tropical or sub-tropical shrubland &    0 &    0 &    0 &    0 &    0 &    0 &   32 &    0 &    0 &    0 &    0 &    0 &    0 &    0 &    0 &    0 &    0 &    0 &    0 &   32 \\ 
  Temperate or sub-polar shrubland &    0 &    0 &    0 &    3 &    0 &    0 &    0 &  601 &    0 &    0 &    0 &    0 &    0 &    1 &    0 &    0 &    0 &    1 &    0 &  606 \\ 
  Tropical or sub-tropical grassland &    0 &    0 &    0 &    0 &    0 &    0 &    0 &    0 &    0 &    0 &    0 &    0 &    0 &    0 &    0 &    0 &    0 &    0 &    0 &    0 \\ 
  Temperate or sub-polar grassland &    0 &    0 &    0 &    0 &    0 &    0 &    0 &    0 &    0 &   12 &    0 &    0 &    0 &    0 &    0 &    0 &    0 &    0 &    0 &   12 \\ 
  Sub-polar or polar shrubland-lichen-moss &    0 &    0 &    0 &    0 &    0 &    0 &    0 &    0 &    0 &    0 &    0 &    0 &    0 &    0 &    0 &    0 &    0 &    0 &    0 &    0 \\ 
  Sub-polar or polar grassland-lichen-moss &    0 &    0 &    0 &    0 &    0 &    0 &    0 &    0 &    0 &    0 &    0 &    0 &    0 &    0 &    0 &    0 &    0 &    0 &    0 &    0 \\ 
  Sub-polar or polar barren-lichen-moss &    0 &    0 &    0 &    0 &    0 &    0 &    0 &    0 &    0 &    0 &    0 &    0 &    0 &    0 &    0 &    0 &    0 &    0 &    0 &    0 \\ 
  Wetland &    0 &    0 &    0 &    0 &    0 &    0 &    0 &    0 &    0 &    0 &    0 &    0 &    0 &    0 &    0 &    0 &    0 &    0 &    0 &    0 \\ 
  Cropland &    0 &    0 &    0 &    0 &    0 &    0 &    0 &    1 &    0 &    0 &    0 &    0 &    0 &   19 & 1183 &    1 &    0 &   39 &    0 & 1243 \\ 
  Barren Lands &    0 &    0 &    0 &    0 &    0 &    0 &    0 &    0 &    0 &    0 &    0 &    0 &    0 &    0 &    0 &   35 &    0 &   13 &    0 &   48 \\ 
  Urban and Built-up &    0 &    0 &    0 &    0 &    0 &    0 &    0 &    0 &    0 &    0 &    0 &    0 &    0 &    0 &    0 &    0 &  130 &    3 &    0 &  133 \\ 
  Water &    0 &    0 &    0 &    1 &    0 &    0 &    0 &    0 &    0 &    0 &    0 &    0 &    0 &    7 &    1 &    0 &    0 & 5019 &    0 & 5028 \\ 
  Snow and Ice &    0 &    0 &    0 &    0 &    0 &    0 &    0 &    0 &    0 &    0 &    0 &    0 &    0 &    0 &    0 &    0 &    0 &    0 &    0 &    0 \\ 
   \hline
Total &    0 &    0 &    0 & 2638 &   96 &    4 &   32 &  603 &    0 &   12 &    0 &    0 &    0 &   62 & 1187 &   37 &  130 & 5199 &    0 & 10000 \\ 
   \hline
\end{tabular}
\endgroup
\caption[NALCMS land-use distribution for site Jalisco164, 2005 and 2010.]{NALCMS land-use distribution for site Jalisco164, 2005 and 2010.} 
\end{table}

   			\label{tab:landUseSonora}
   		\end{center}
		
   		\begin{figure}[H]%--- Picture 'H'ere, 'B'ottom or 'T'op; '!' Try to
   		                    %impose your will to LaTeX
   		  \centering
   		  \includegraphics[width=.5\textwidth]{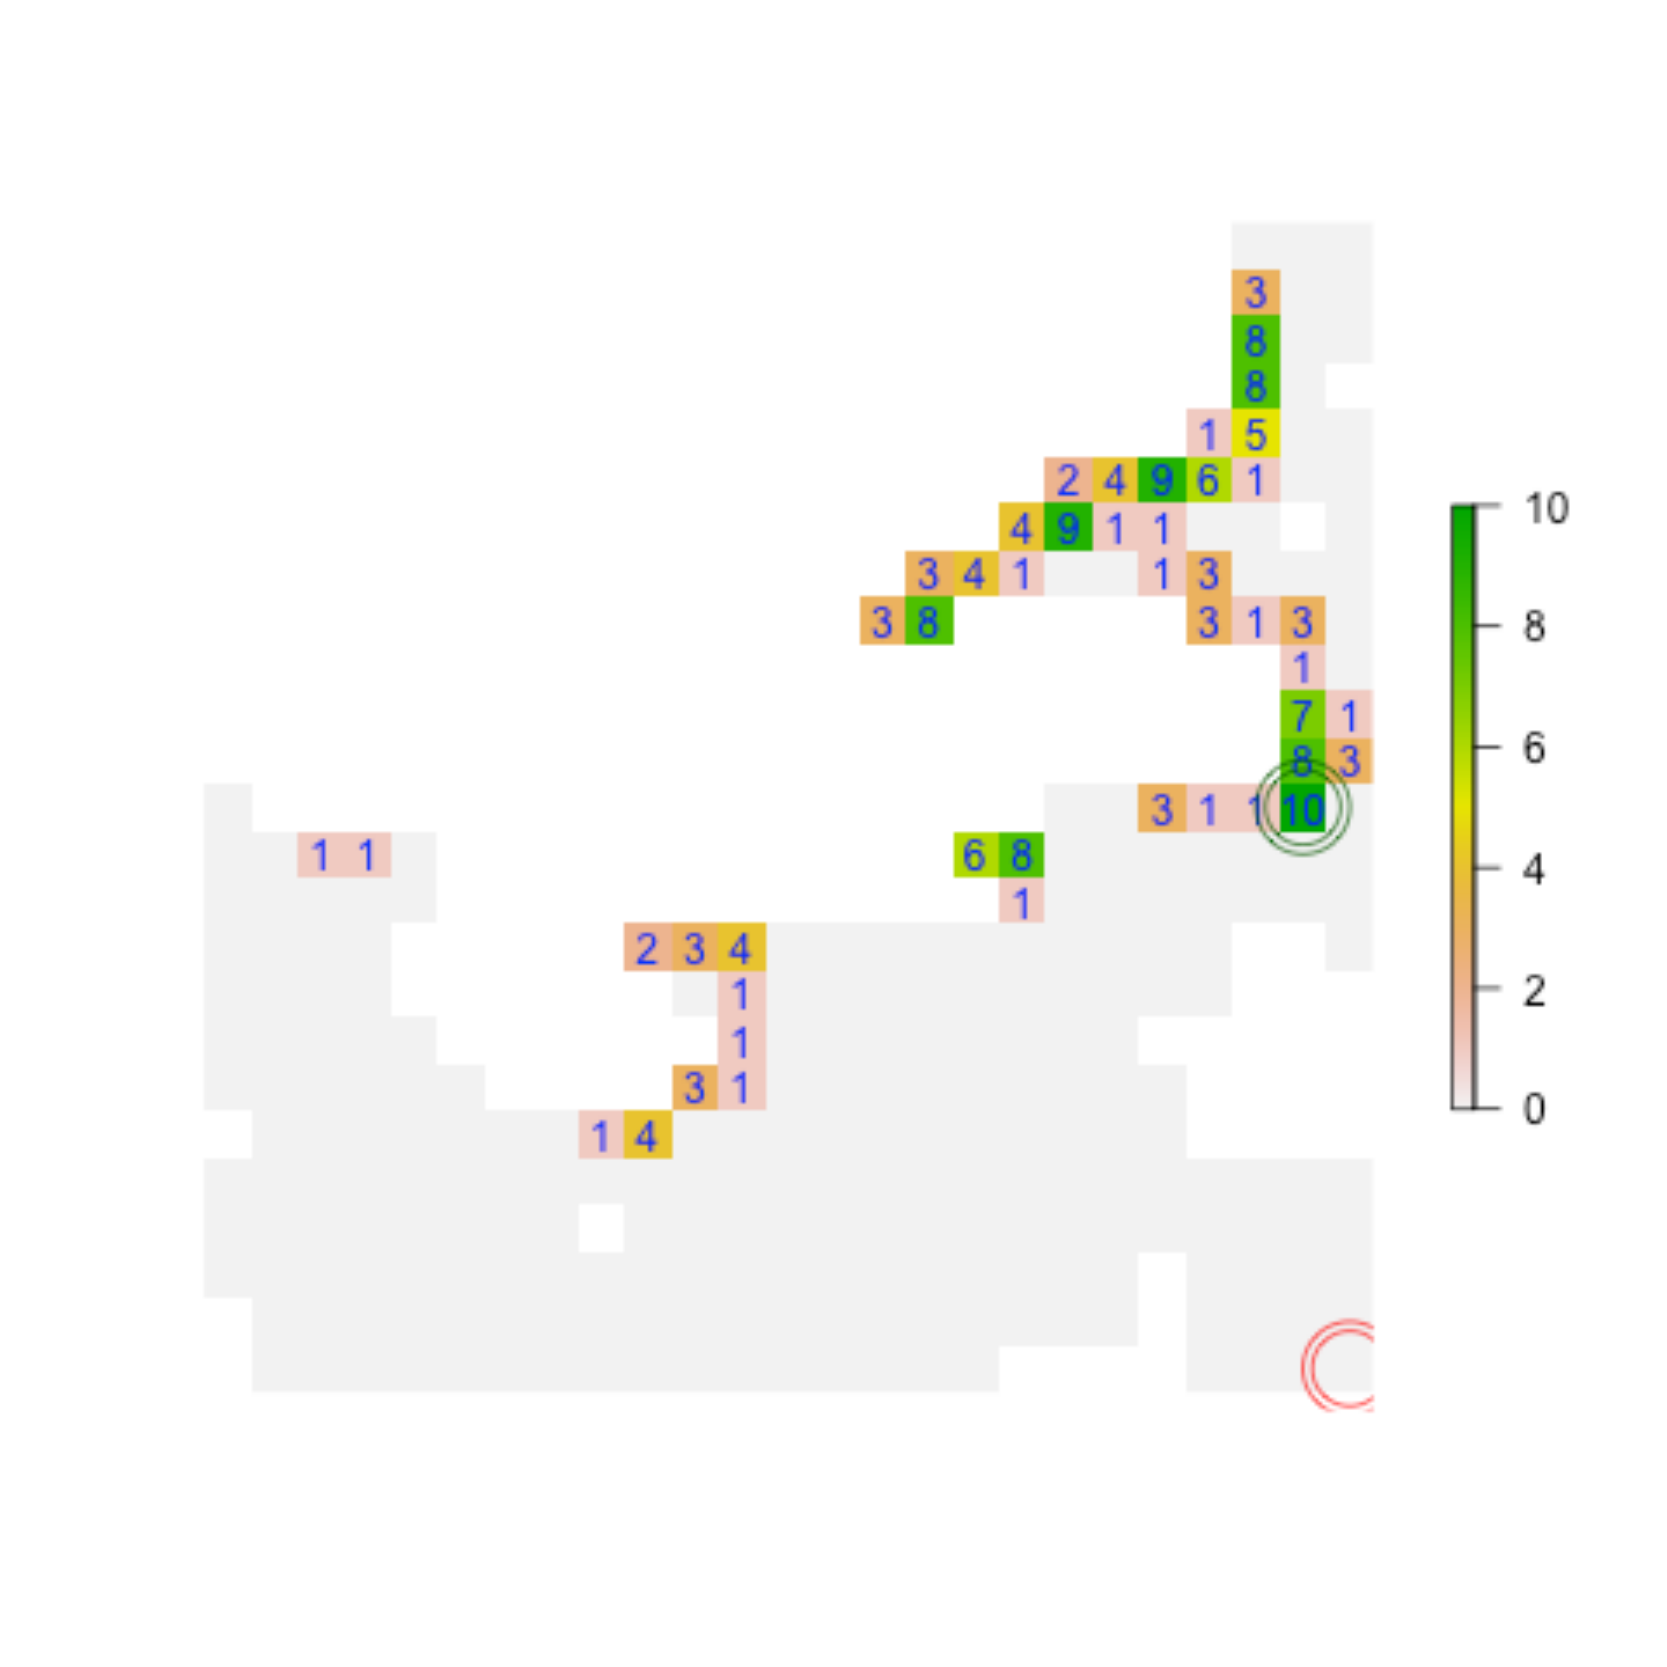} %<< no file extension
   		  %%         --- .5\textwidth stands for 50% of text width
   		  \caption[Deforestation in Jalisco164 site at 1km resolution]%<<-- Legend for the list of figures at the beginning of you thesis
   		  {Deforestation in Jalisco164 site at 1km resolution: number of 250m pixels deforested out of 16}% legend displayed below the graph.
   		  \label{fig:defoJalisco164}
   		\end{figure}
		
   		 \begin{figure}[H]
   	      \begin{subfigure}{.5\textwidth}
   	        \centering
   	    	\includegraphics[width=1\textwidth]{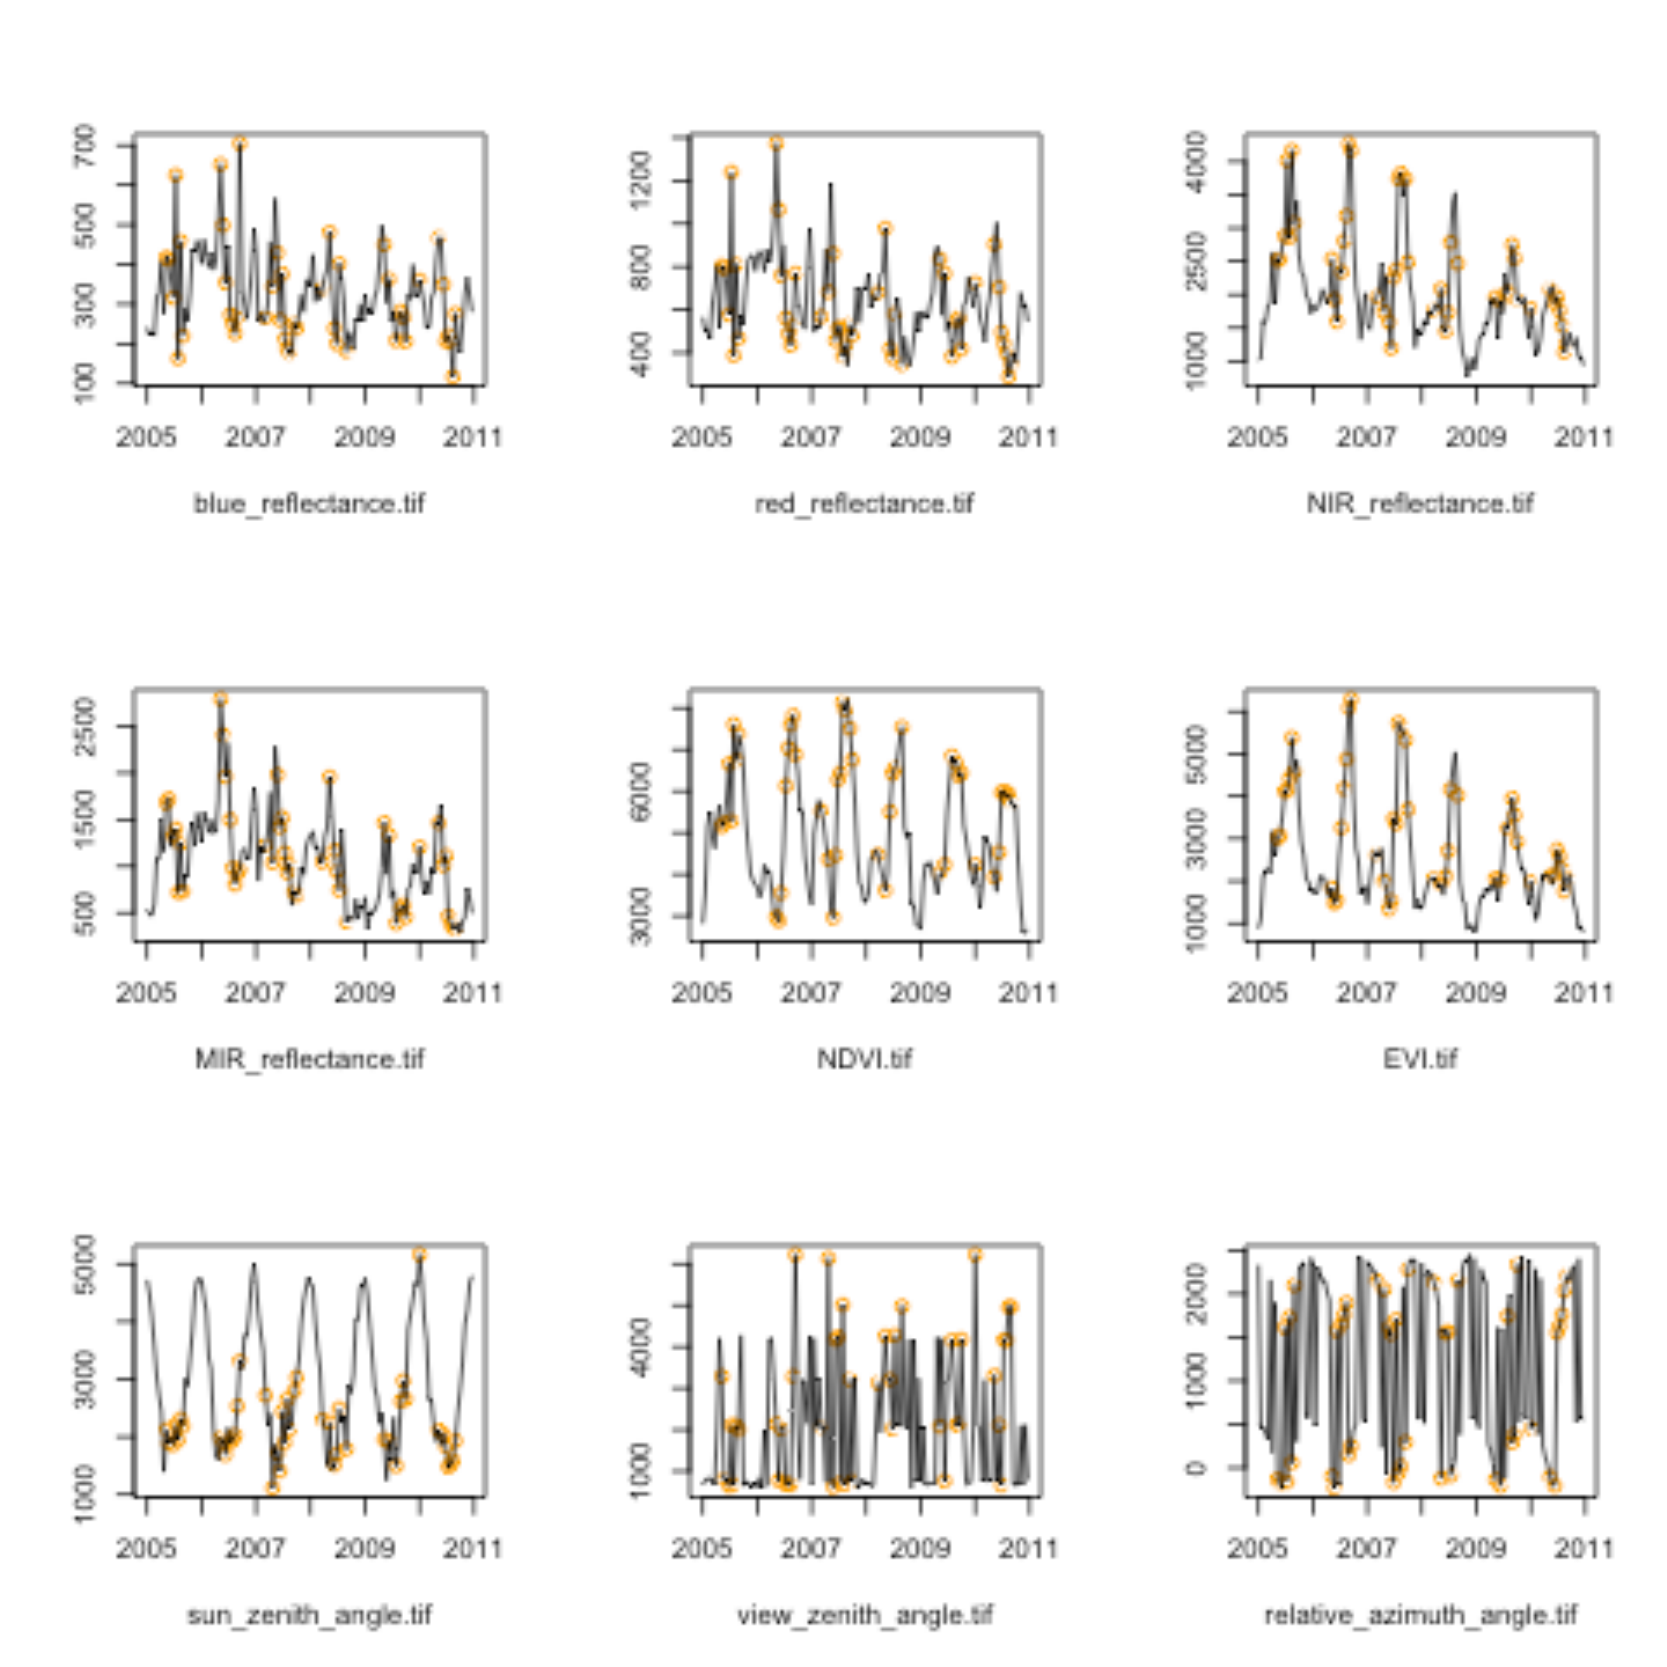} 
   	        \caption{deforested pixel}
   	        \label{fig:defo_pix}
   	      \end{subfigure}%
   	      \begin{subfigure}{.5\textwidth}
   	        \centering
   	        \includegraphics[width=1\textwidth]{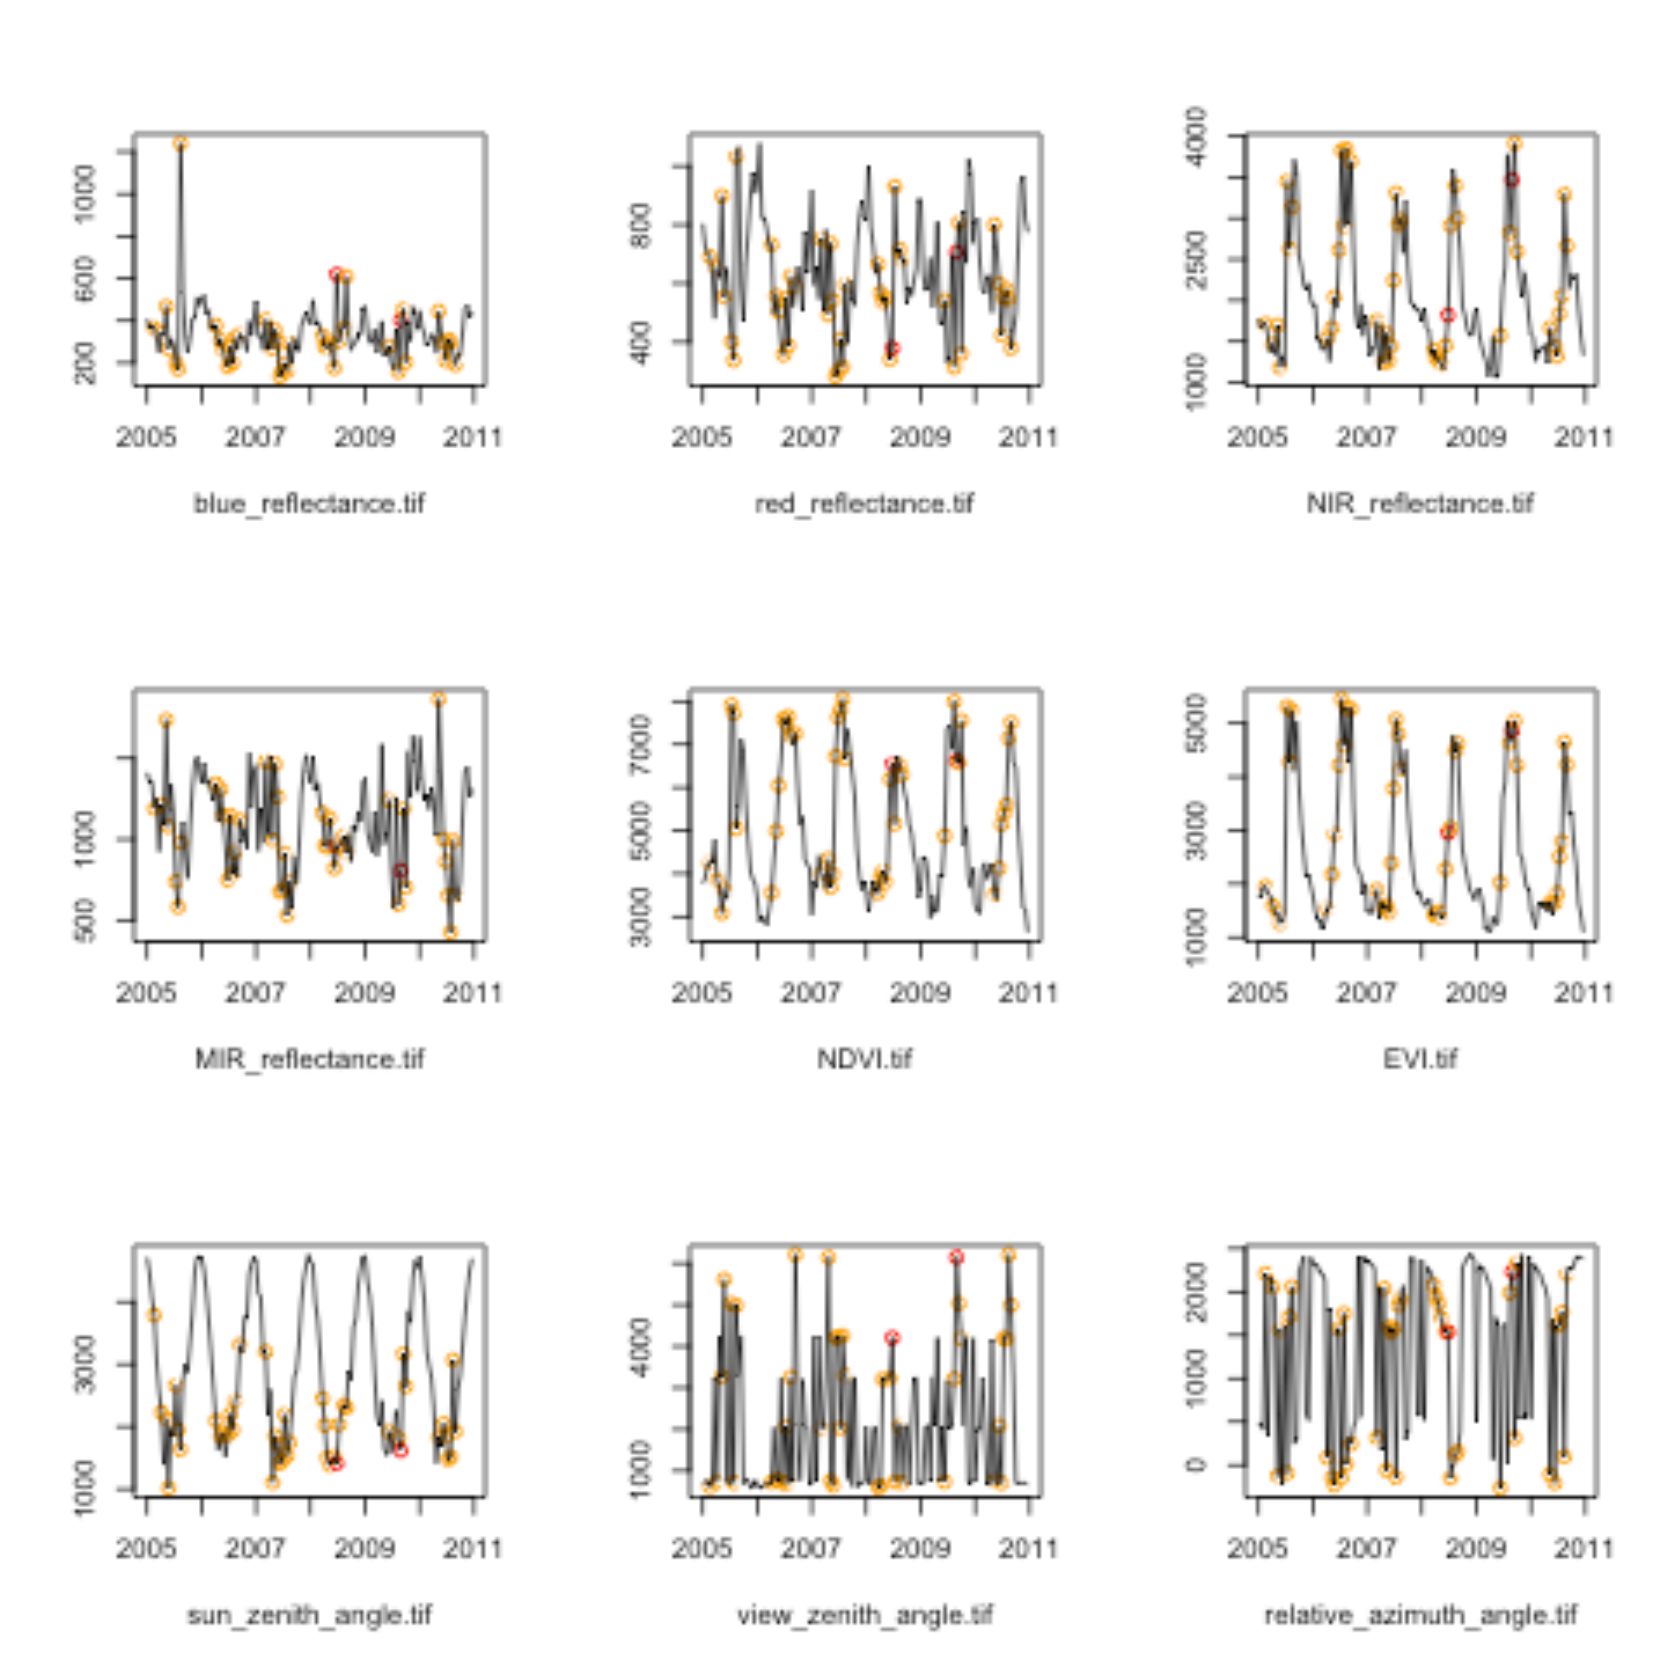}
   	        \caption{non-deforested pixel}
   	        \label{fig:non_defo_pix}
   	      \end{subfigure}
   	      %%         --- .5\textwidth stands for 50% of text width
   	      \caption[Reflectance, vegetation indices and sun-sensor geometry time series for deforested and non-deforested pixel in Yucatan 180 site.]%<<-- Legend for the list of figures at the beginning of you thesis
   	      {Reflectance, vegetation indices and sun-sensor geometry time series for deforested and non-deforested pixel in Jalisco164 site, identified in figure \ref{fig:defoJalisco164} with green and red circles respectively. Orange marked points are \emph{marginal data} and red marked points are \emph{cloudy} or \emph{not processed}}% legend displayed below the graph.
   	      \label{fig:timeSeries}
   	    \end{figure}
		
		\subsubsection{Nayarit151}
		
      	 \begin{figure}[H]  %--- Picture 'H'ere, 'B'ottom or 'T'op; '!' Try to
      	                     %impose your will to LaTeX
      	  % \centering 
  
      	   \begin{subfigure}{.5\textwidth}
      	     \centering
      	 	\includegraphics[width=0.7\textwidth]{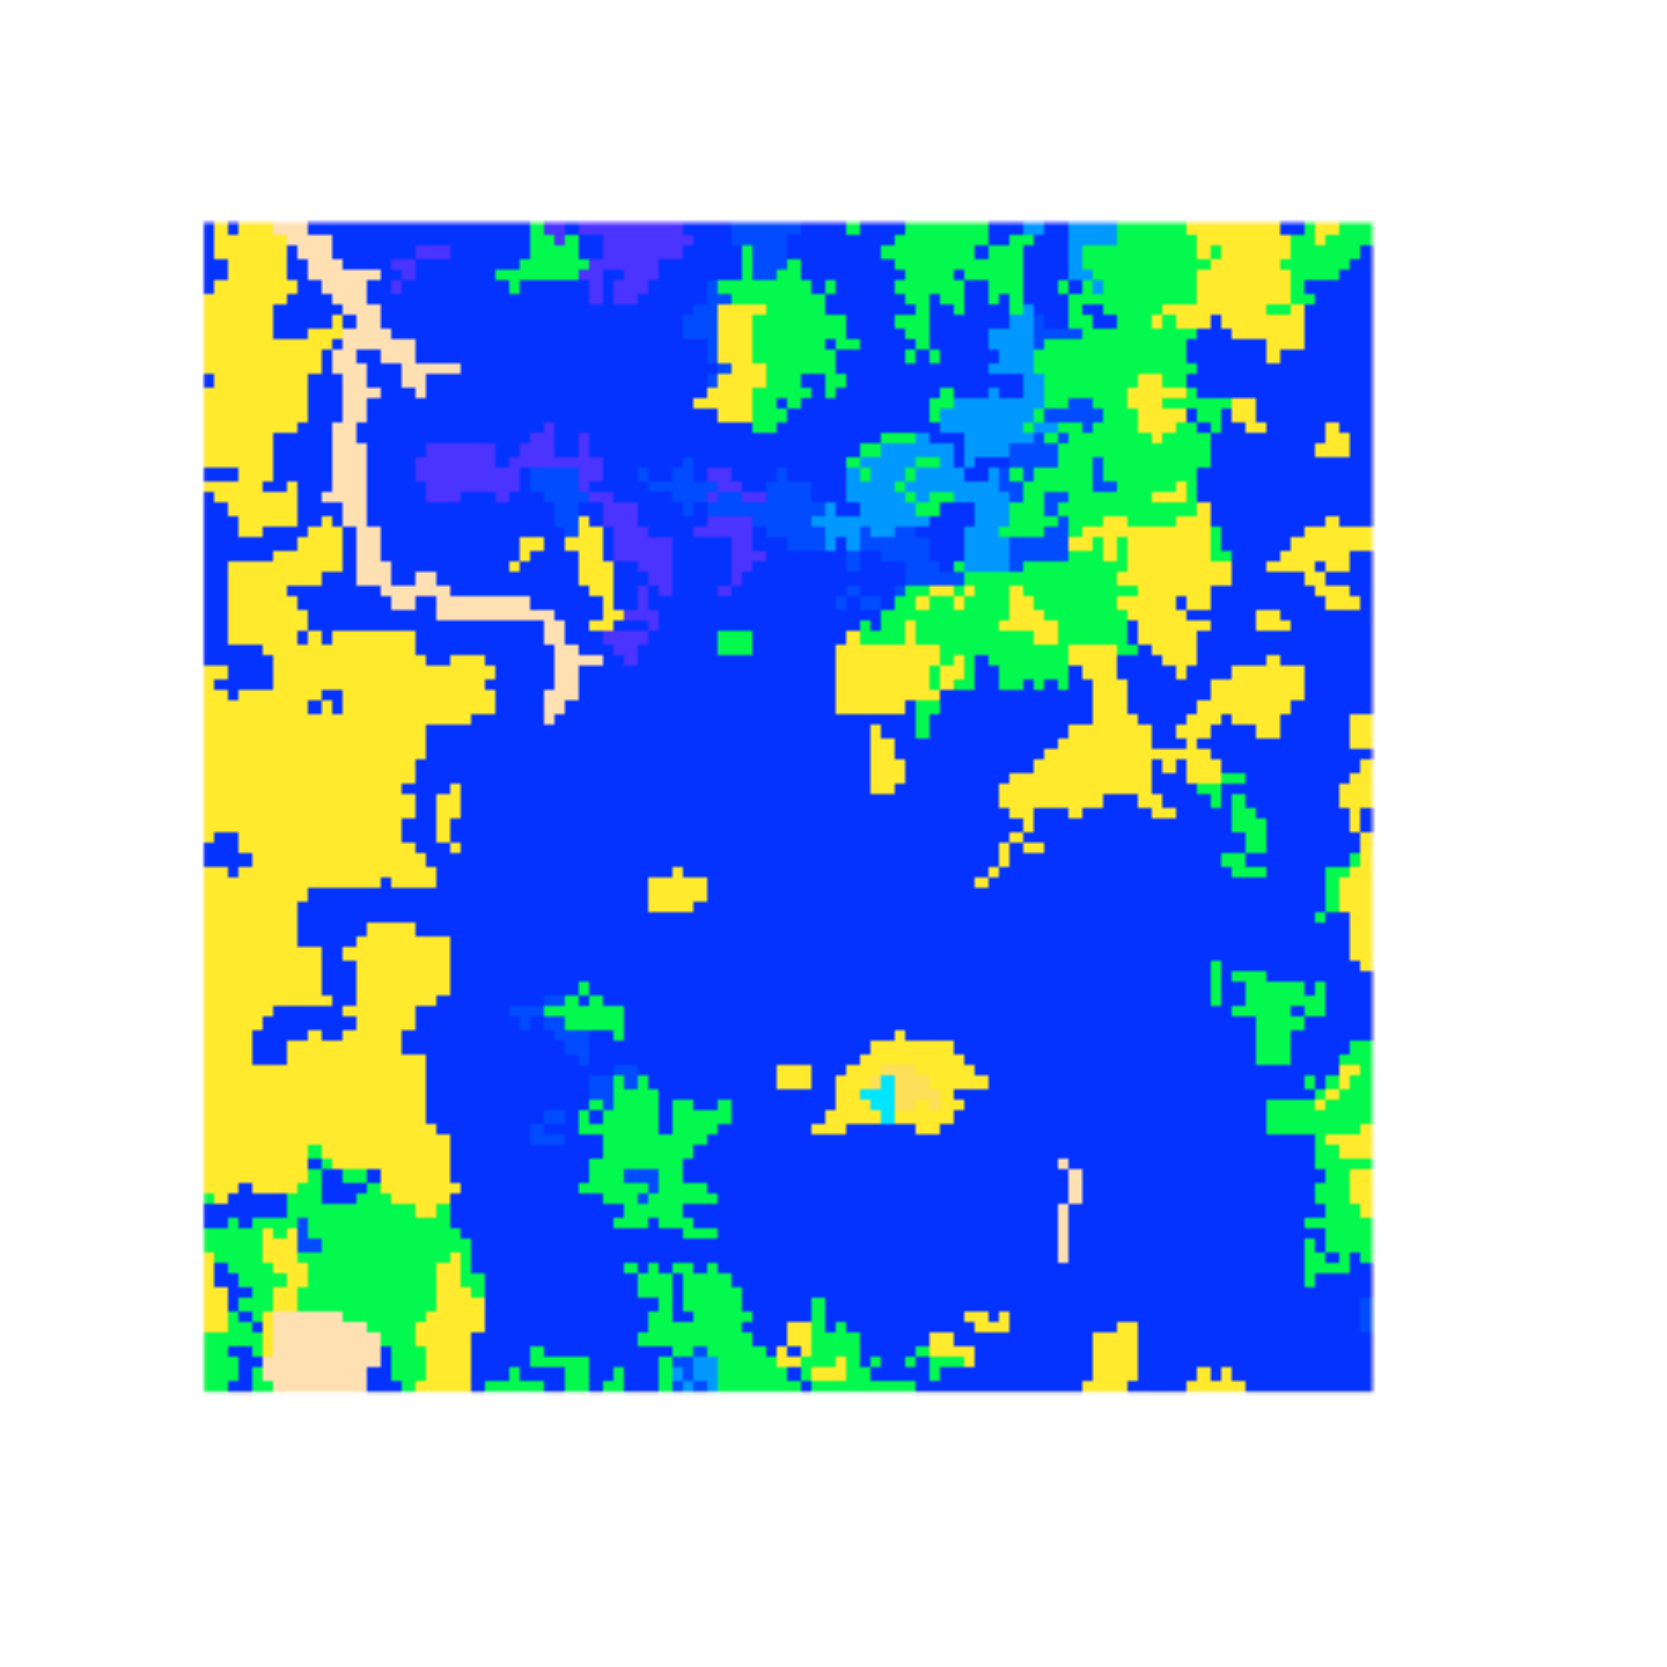} 
      	     \caption{Land-use 2005}
      	     \label{fig:sfig1a}
      	   \end{subfigure}%
      	   \begin{subfigure}{.5\textwidth}
      	     \centering
      	     \includegraphics[width=0.7\textwidth]{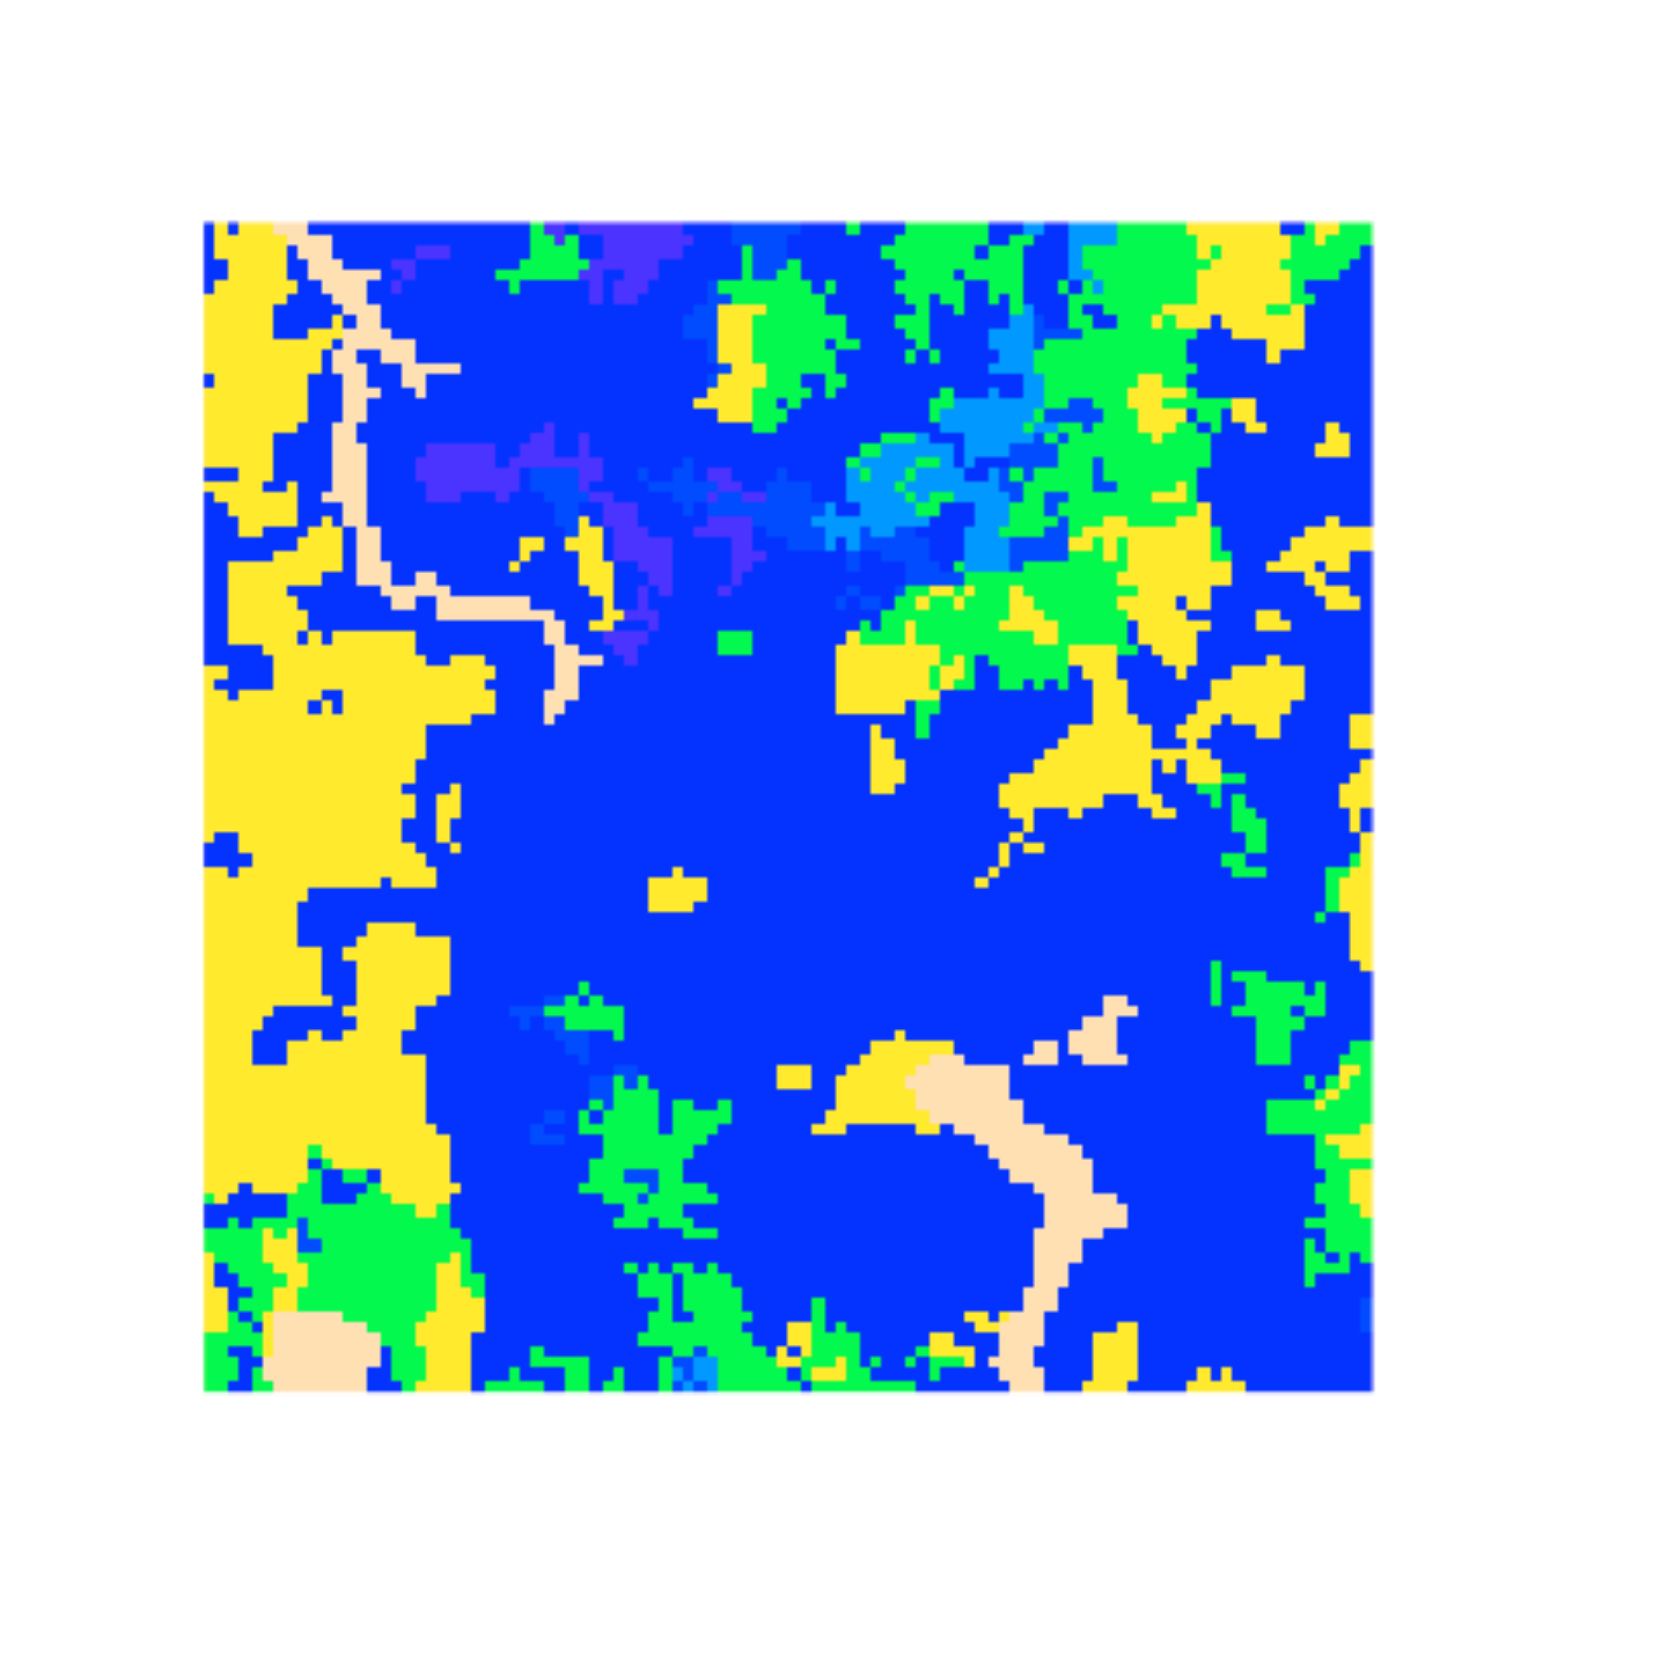}
      	     \caption{Land-use 2010}
      	     \label{fig:sfig1b}
      	   \end{subfigure}
      	   \begin{subfigure}{.4\textwidth}
      	     \centering
      	     \includegraphics[width=0.9\textwidth]{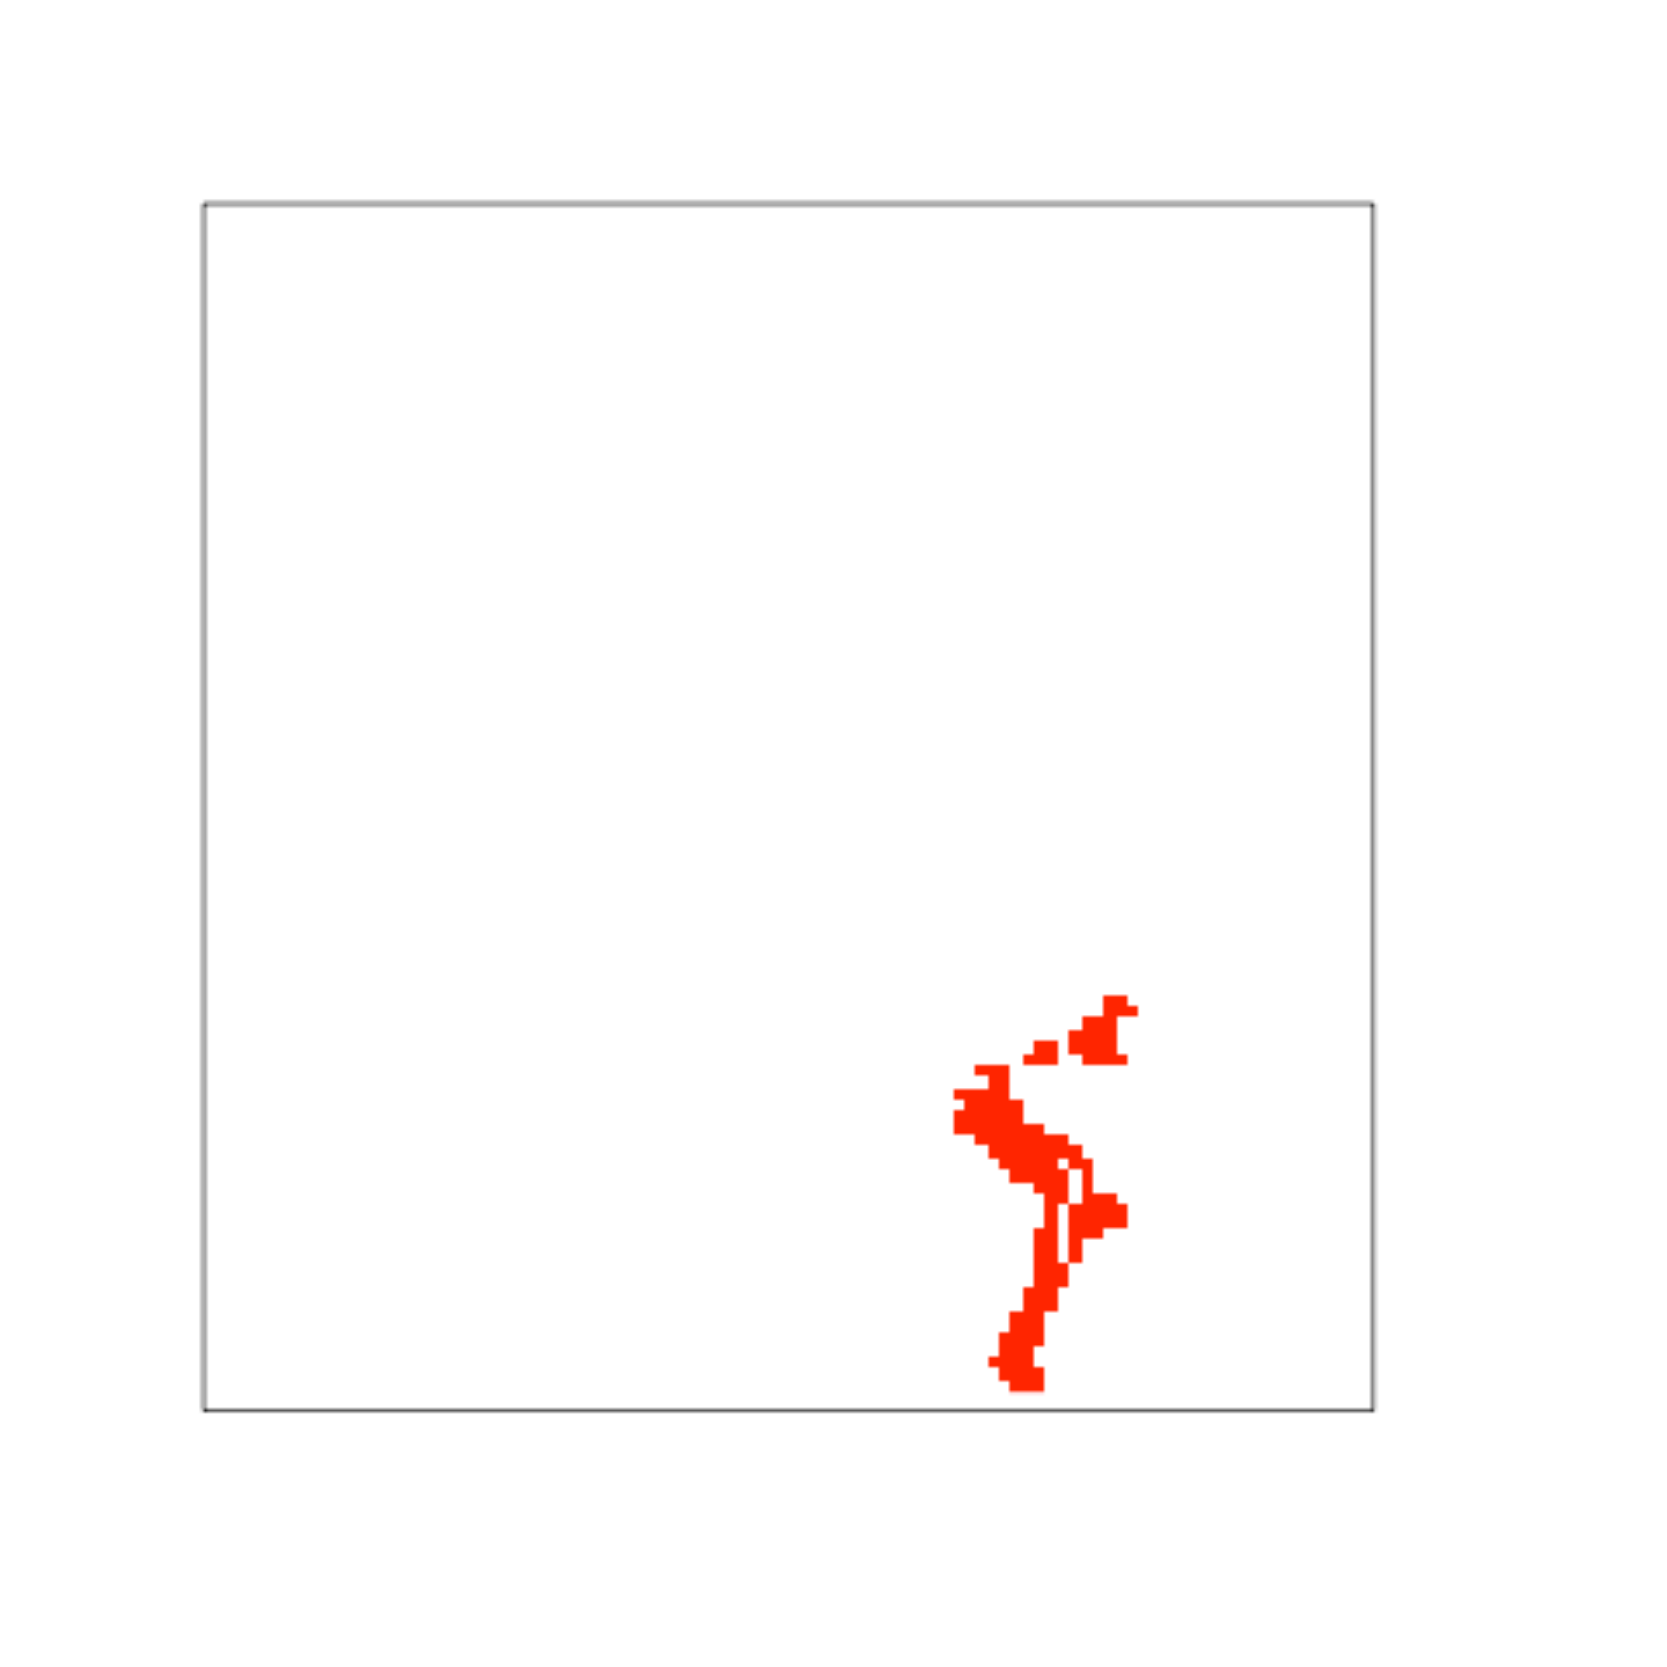}
      	     \caption{Deforestation 2005-2010}
      	     \label{fig:sfig1c}
      	   \end{subfigure}
      	   \begin{subfigure}{.4\textwidth}
      	     \centering
      	     \includegraphics[width=0.9\textwidth]{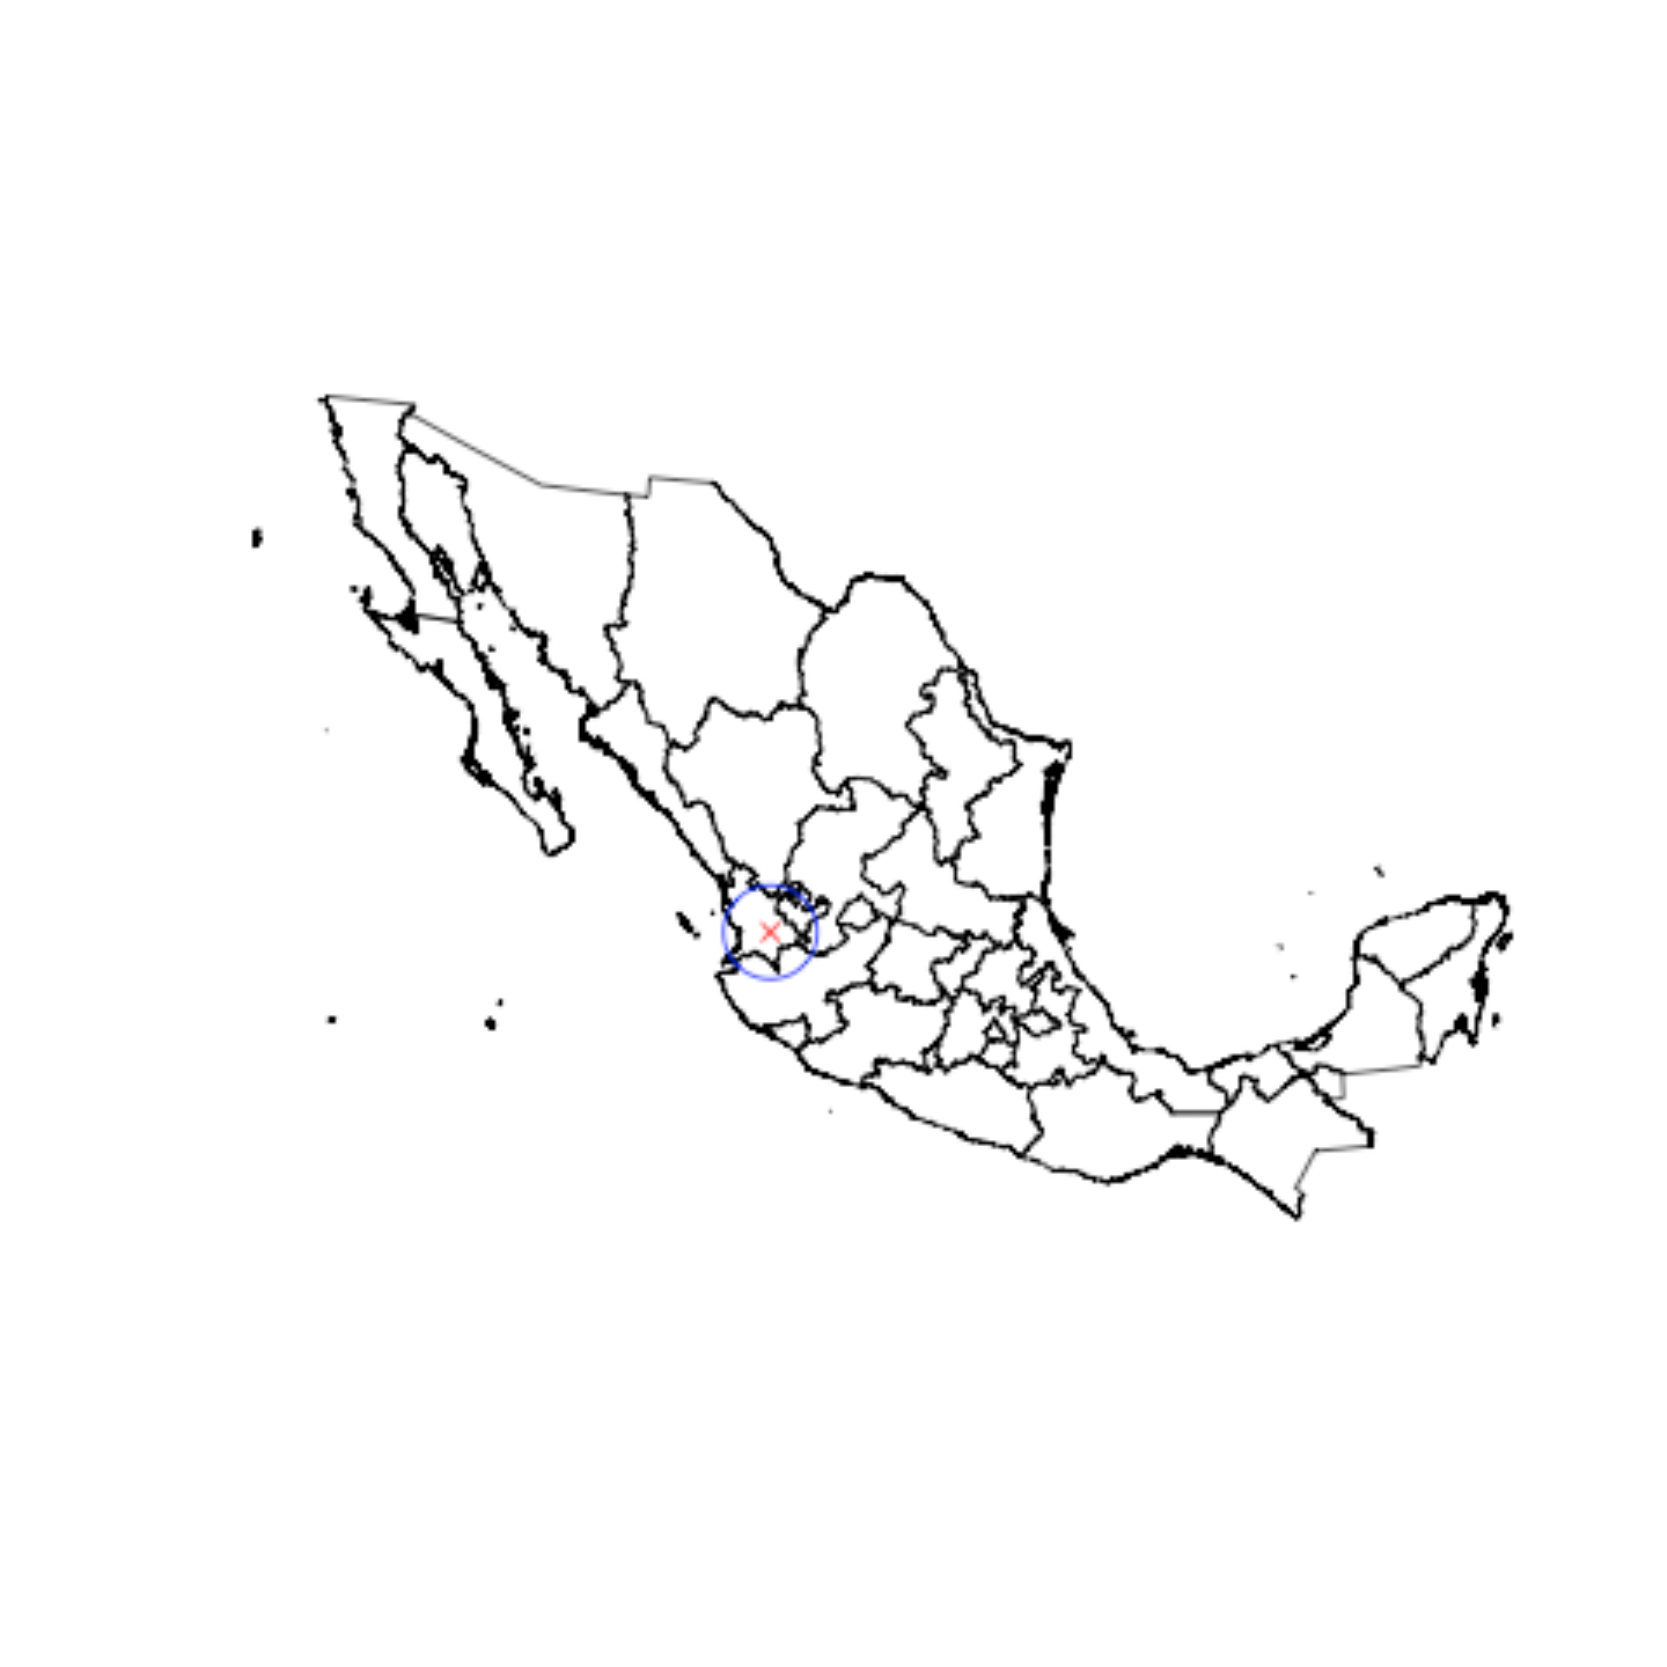}
      	     \caption{Location}
      	     \label{fig:sfig1d}
      	   \end{subfigure}   
         \begin{subfigure}{.5\textwidth}
           \centering
           \includegraphics[width=1\textwidth]{./2_Data/legend_landUse}
           \caption{Land use legend}
           \label{fig:legend}
         \end{subfigure}
      	   %%         --- .5\textwidth stands for 50% of text width
      	   \caption[NALCMS land-use classification of Nayarit151 site, 2005 and 2010 at 250m resolution.]%<<-- Legend for the list of figures at the beginning of you thesis
      	   {NALCMS land-use classification of Nayarit151 site, 2005 and 2010 at 250m resolution.}% legend displayed below the graph.
      	   \label{fig:landUseNayarit151}
      	 \end{figure}
		
   		\begin{center}
   			\footnotesize\addtolength{\tabcolsep}{-2pt}
   			% latex table generated in R 3.3.1 by xtable 1.8-2 package
% Sun Mar  5 15:58:58 2017
\begin{table}[ht]
\centering
\begingroup\tiny
\begin{tabular}{rrrrrrrrrrrrrrrrrrrrr}
  & \begin{sideways} Temperate or sub-polar needleleaf forest \end{sideways} & \begin{sideways} Sub-polar taiga needleleaf forest \end{sideways} & \begin{sideways} Tropical or sub-tropical broadleaf evergreen forest \end{sideways} & \begin{sideways} Tropical or sub-tropical broadleaf deciduous forest \end{sideways} & \begin{sideways} Temperate or sub-polar broadleaf deciduous forest \end{sideways} & \begin{sideways} Mixed Forest \end{sideways} & \begin{sideways} Tropical or sub-tropical shrubland \end{sideways} & \begin{sideways} Temperate or sub-polar shrubland \end{sideways} & \begin{sideways} Tropical or sub-tropical grassland \end{sideways} & \begin{sideways} Temperate or sub-polar grassland \end{sideways} & \begin{sideways} Sub-polar or polar shrubland-lichen-moss \end{sideways} & \begin{sideways} Sub-polar or polar grassland-lichen-moss \end{sideways} & \begin{sideways} Sub-polar or polar barren-lichen-moss \end{sideways} & \begin{sideways} Wetland \end{sideways} & \begin{sideways} Cropland \end{sideways} & \begin{sideways} Barren Lands \end{sideways} & \begin{sideways} Urban and Built-up \end{sideways} & \begin{sideways} Water \end{sideways} & \begin{sideways} Snow and Ice \end{sideways} & \begin{sideways} Total \end{sideways} \\ 
  \hline
Temperate or sub-polar needleleaf forest &    0 &    0 &    0 &    0 &    0 &    0 &    0 &    0 &    0 &    0 &    0 &    0 &    0 &    0 &    0 &    0 &    0 &    0 &    0 &    0 \\ 
  Sub-polar taiga needleleaf forest &    0 &    0 &    0 &    0 &    0 &    0 &    0 &    0 &    0 &    0 &    0 &    0 &    0 &    0 &    0 &    0 &    0 &    0 &    0 &    0 \\ 
  Tropical or sub-tropical broadleaf evergreen forest &    0 &    0 &  170 &    0 &    0 &    0 &    0 &    0 &    0 &    0 &    0 &    0 &    0 &    0 &    0 &    0 &    0 &    0 &    0 &  170 \\ 
  Tropical or sub-tropical broadleaf deciduous forest &    0 &    0 &    0 & 5876 &    0 &    0 &    0 &    0 &    0 &    0 &    0 &    0 &    0 &    0 &    0 &    0 &    0 &  151 &    0 & 6027 \\ 
  Temperate or sub-polar broadleaf deciduous forest &    0 &    0 &    0 &    0 &  223 &    0 &    0 &    0 &    0 &    0 &    0 &    0 &    0 &    0 &    0 &    0 &    0 &    0 &    0 &  223 \\ 
  Mixed Forest &    0 &    0 &    0 &    0 &    0 &  170 &    0 &    0 &    0 &    0 &    0 &    0 &    0 &    0 &    0 &    0 &    0 &    0 &    0 &  170 \\ 
   \hline
Tropical or sub-tropical shrubland &    0 &    0 &    0 &    0 &    0 &    0 &    0 &    0 &    0 &    0 &    0 &    0 &    0 &    0 &    7 &    0 &    0 &    0 &    0 &    7 \\ 
  Temperate or sub-polar shrubland &    0 &    0 &    0 &    0 &    0 &    0 &    0 & 1278 &    0 &    0 &    0 &    0 &    0 &    0 &    0 &    0 &    0 &    0 &    0 & 1278 \\ 
  Tropical or sub-tropical grassland &    0 &    0 &    0 &    0 &    0 &    0 &    0 &    0 &    0 &    0 &    0 &    0 &    0 &    0 &    0 &    0 &    0 &    0 &    0 &    0 \\ 
  Temperate or sub-polar grassland &    0 &    0 &    0 &    0 &    0 &    0 &    0 &    0 &    0 &    0 &    0 &    0 &    0 &    0 &    0 &    0 &    0 &    0 &    0 &    0 \\ 
  Sub-polar or polar shrubland-lichen-moss &    0 &    0 &    0 &    0 &    0 &    0 &    0 &    0 &    0 &    0 &    0 &    0 &    0 &    0 &    0 &    0 &    0 &    0 &    0 &    0 \\ 
  Sub-polar or polar grassland-lichen-moss &    0 &    0 &    0 &    0 &    0 &    0 &    0 &    0 &    0 &    0 &    0 &    0 &    0 &    0 &    0 &    0 &    0 &    0 &    0 &    0 \\ 
  Sub-polar or polar barren-lichen-moss &    0 &    0 &    0 &    0 &    0 &    0 &    0 &    0 &    0 &    0 &    0 &    0 &    0 &    0 &    0 &    0 &    0 &    0 &    0 &    0 \\ 
  Wetland &    0 &    0 &    0 &    0 &    0 &    0 &    0 &    0 &    0 &    0 &    0 &    0 &    0 &    0 &    0 &    0 &    0 &    0 &    0 &    0 \\ 
  Cropland &    0 &    0 &    0 &    0 &    0 &    0 &    0 &    0 &    0 &    0 &    0 &    0 &    0 &    0 & 1873 &    0 &    0 &   20 &    0 & 1893 \\ 
  Barren Lands &    0 &    0 &    0 &    0 &    0 &    0 &    0 &    0 &    0 &    0 &    0 &    0 &    0 &    0 &    9 &    0 &    0 &    5 &    0 &   14 \\ 
  Urban and Built-up &    0 &    0 &    0 &    0 &    0 &    0 &    0 &    0 &    0 &    0 &    0 &    0 &    0 &    0 &    0 &    0 &    0 &    0 &    0 &    0 \\ 
  Water &    0 &    0 &    0 &    0 &    0 &    0 &    0 &    0 &    0 &    0 &    0 &    0 &    0 &    0 &    0 &    0 &    0 &  218 &    0 &  218 \\ 
  Snow and Ice &    0 &    0 &    0 &    0 &    0 &    0 &    0 &    0 &    0 &    0 &    0 &    0 &    0 &    0 &    0 &    0 &    0 &    0 &    0 &    0 \\ 
   \hline
Total &    0 &    0 &  170 & 5876 &  223 &  170 &    0 & 1278 &    0 &    0 &    0 &    0 &    0 &    0 & 1889 &    0 &    0 &  394 &    0 & 10000 \\ 
   \hline
\end{tabular}
\endgroup
\caption[NALCMS land-use distribution for site Nayarit151, 2005 and 2010.]{NALCMS land-use distribution for site Nayarit151, 2005 and 2010.} 
\end{table}

   			\label{tab:landUseSonora}
   		\end{center}
		
   		\begin{figure}[H]%--- Picture 'H'ere, 'B'ottom or 'T'op; '!' Try to
   		                    %impose your will to LaTeX
   		  \centering
   		  \includegraphics[width=.5\textwidth]{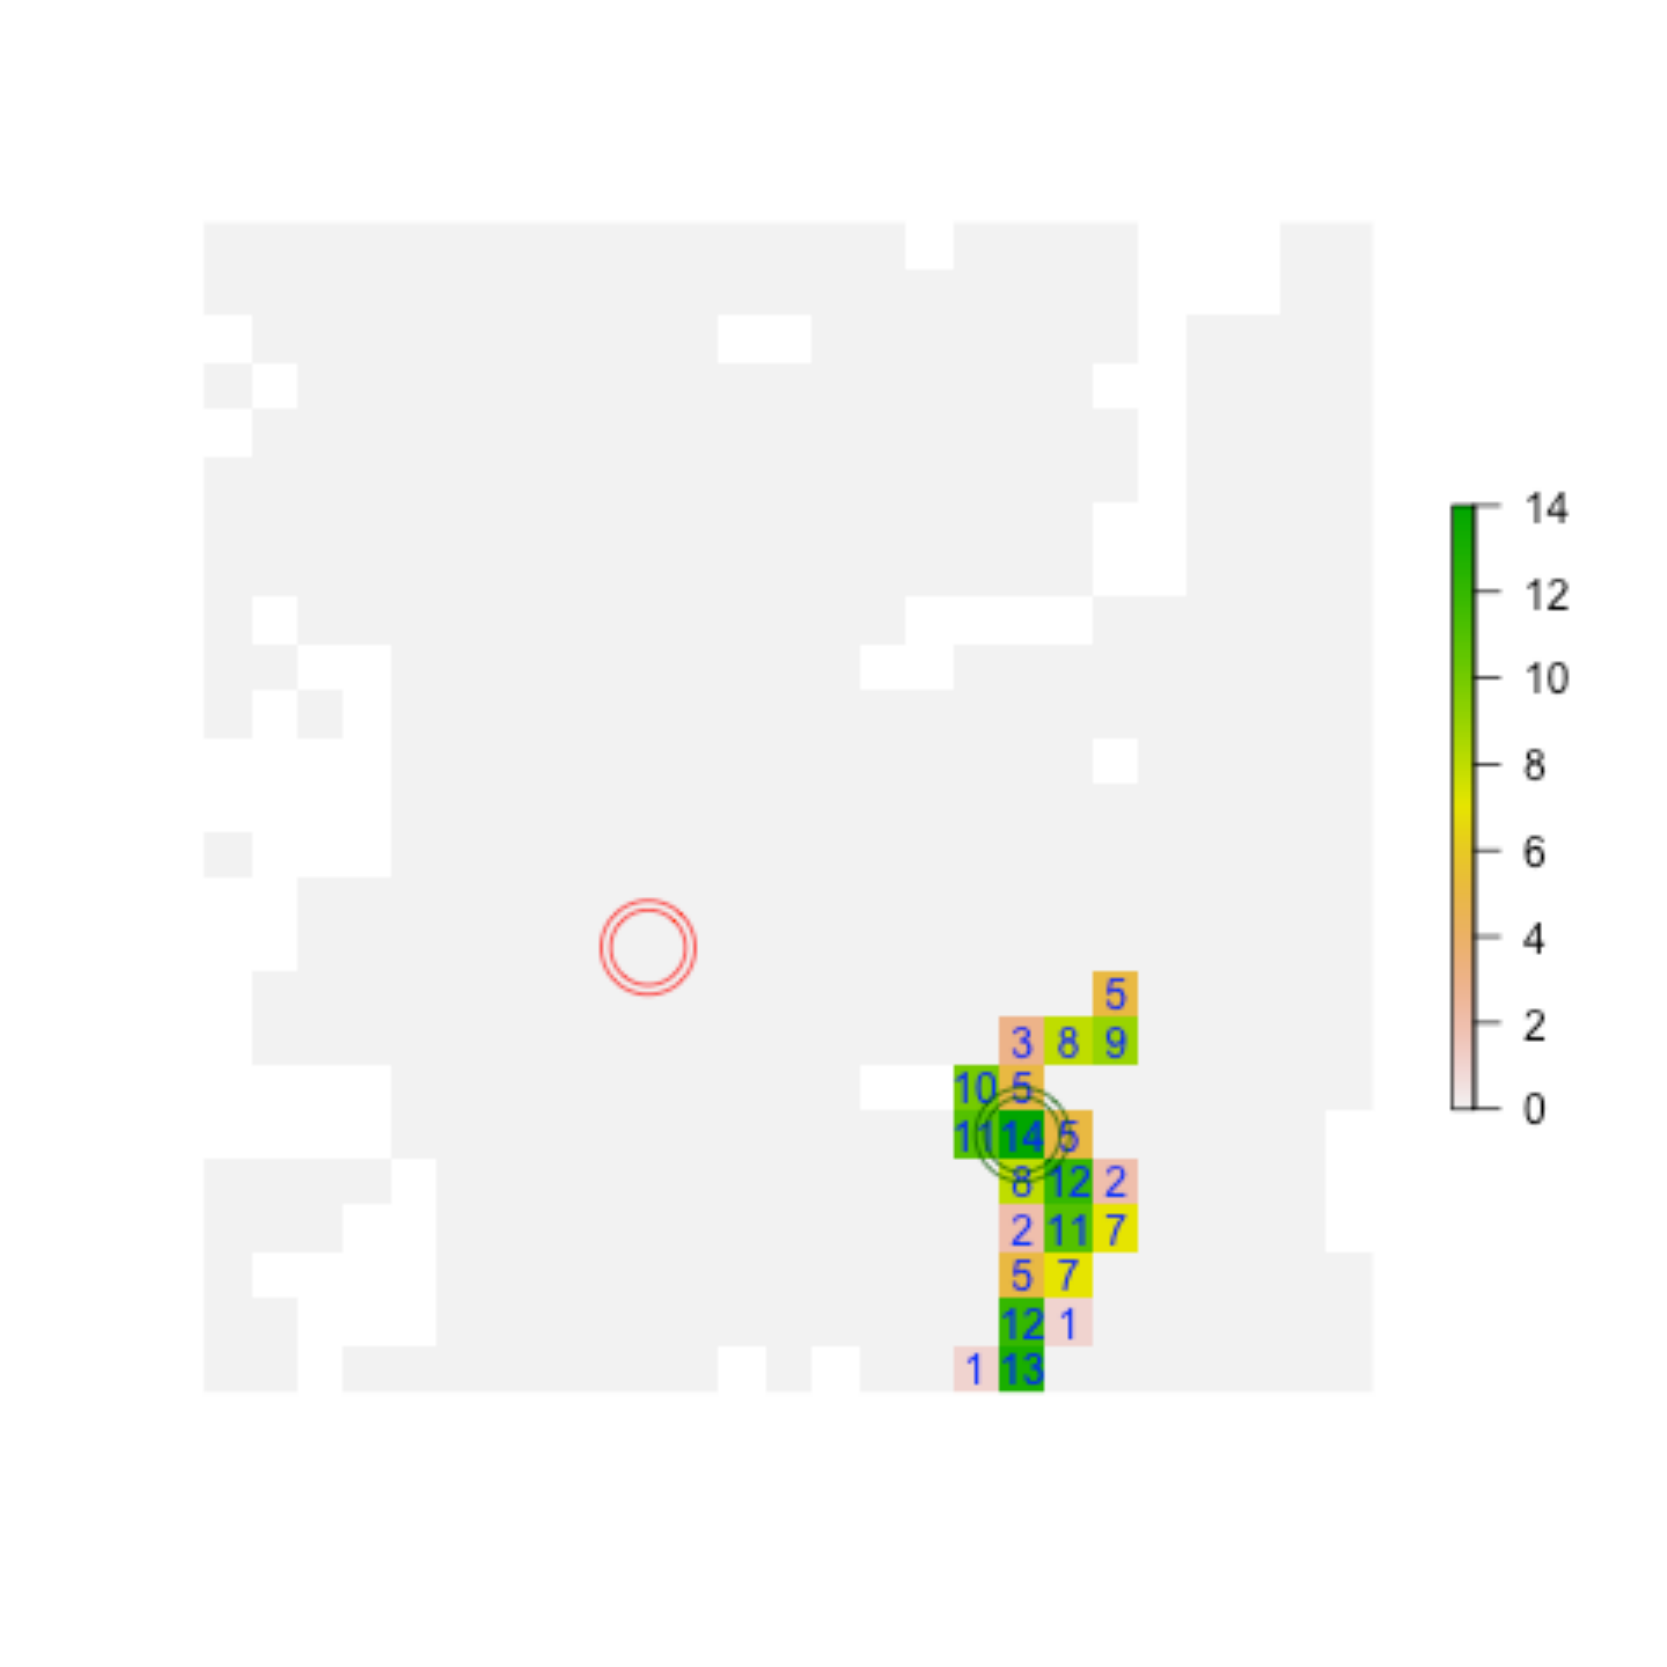} %<< no file extension
   		  %%         --- .5\textwidth stands for 50% of text width
   		  \caption[Deforestation in Nayarit151 site at 1km resolution]%<<-- Legend for the list of figures at the beginning of you thesis
   		  {Deforestation in Nayarit151 site at 1km resolution: number of 250m pixels deforested out of 16}% legend displayed below the graph.
   		  \label{fig:defoNayarit151}
   		\end{figure}
		
   		 \begin{figure}[H]
   	      \begin{subfigure}{.5\textwidth}
   	        \centering
   	    	\includegraphics[width=1\textwidth]{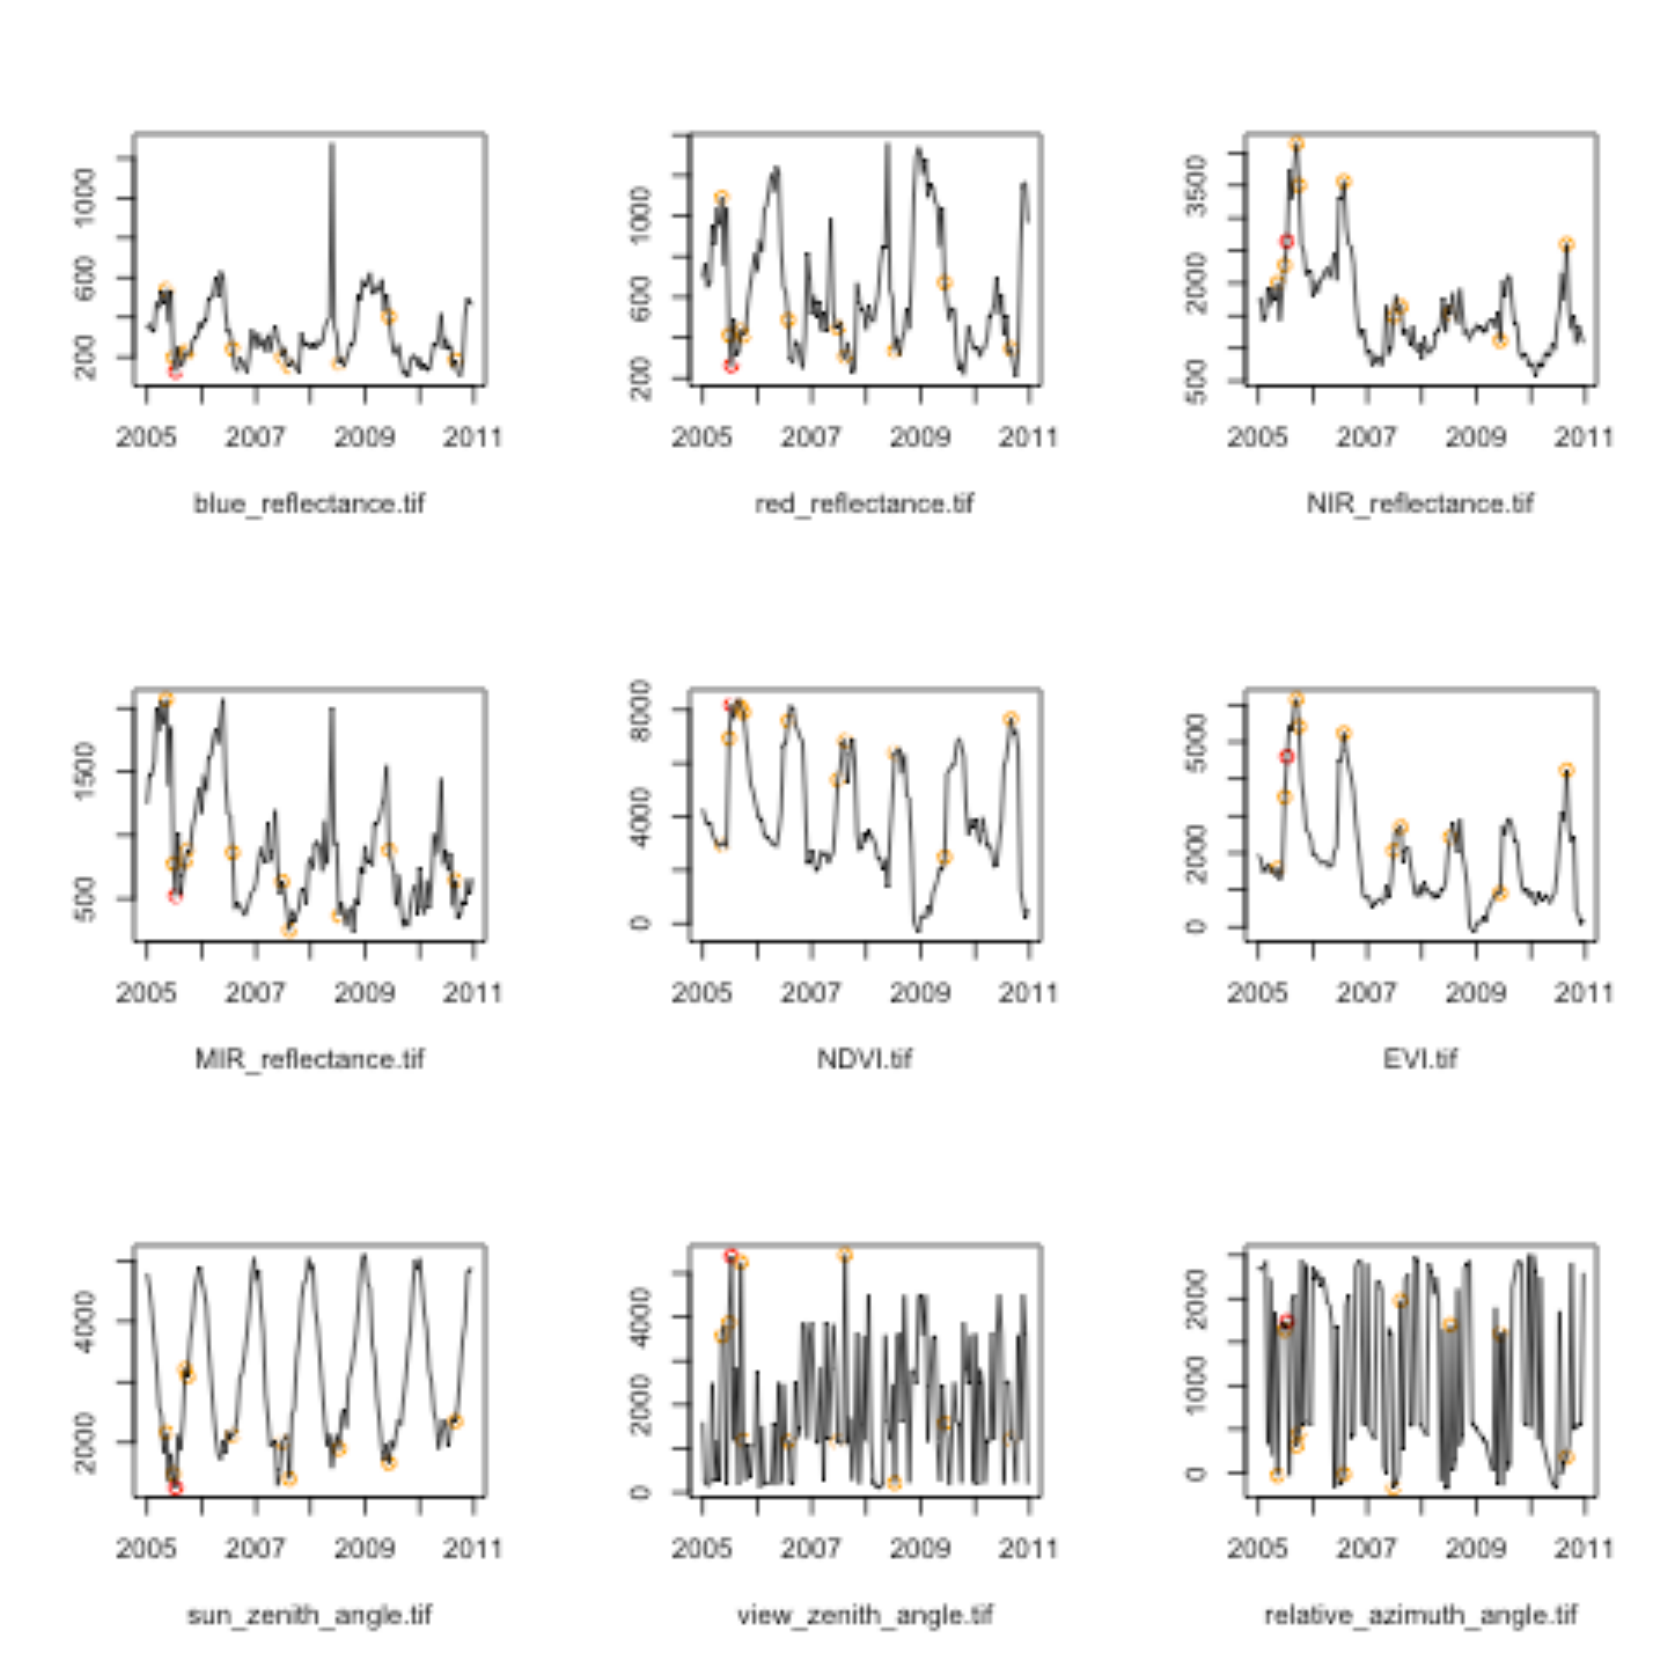} 
   	        \caption{deforested pixel}
   	        \label{fig:defo_pix}
   	      \end{subfigure}%
   	      \begin{subfigure}{.5\textwidth}
   	        \centering
   	        \includegraphics[width=1\textwidth]{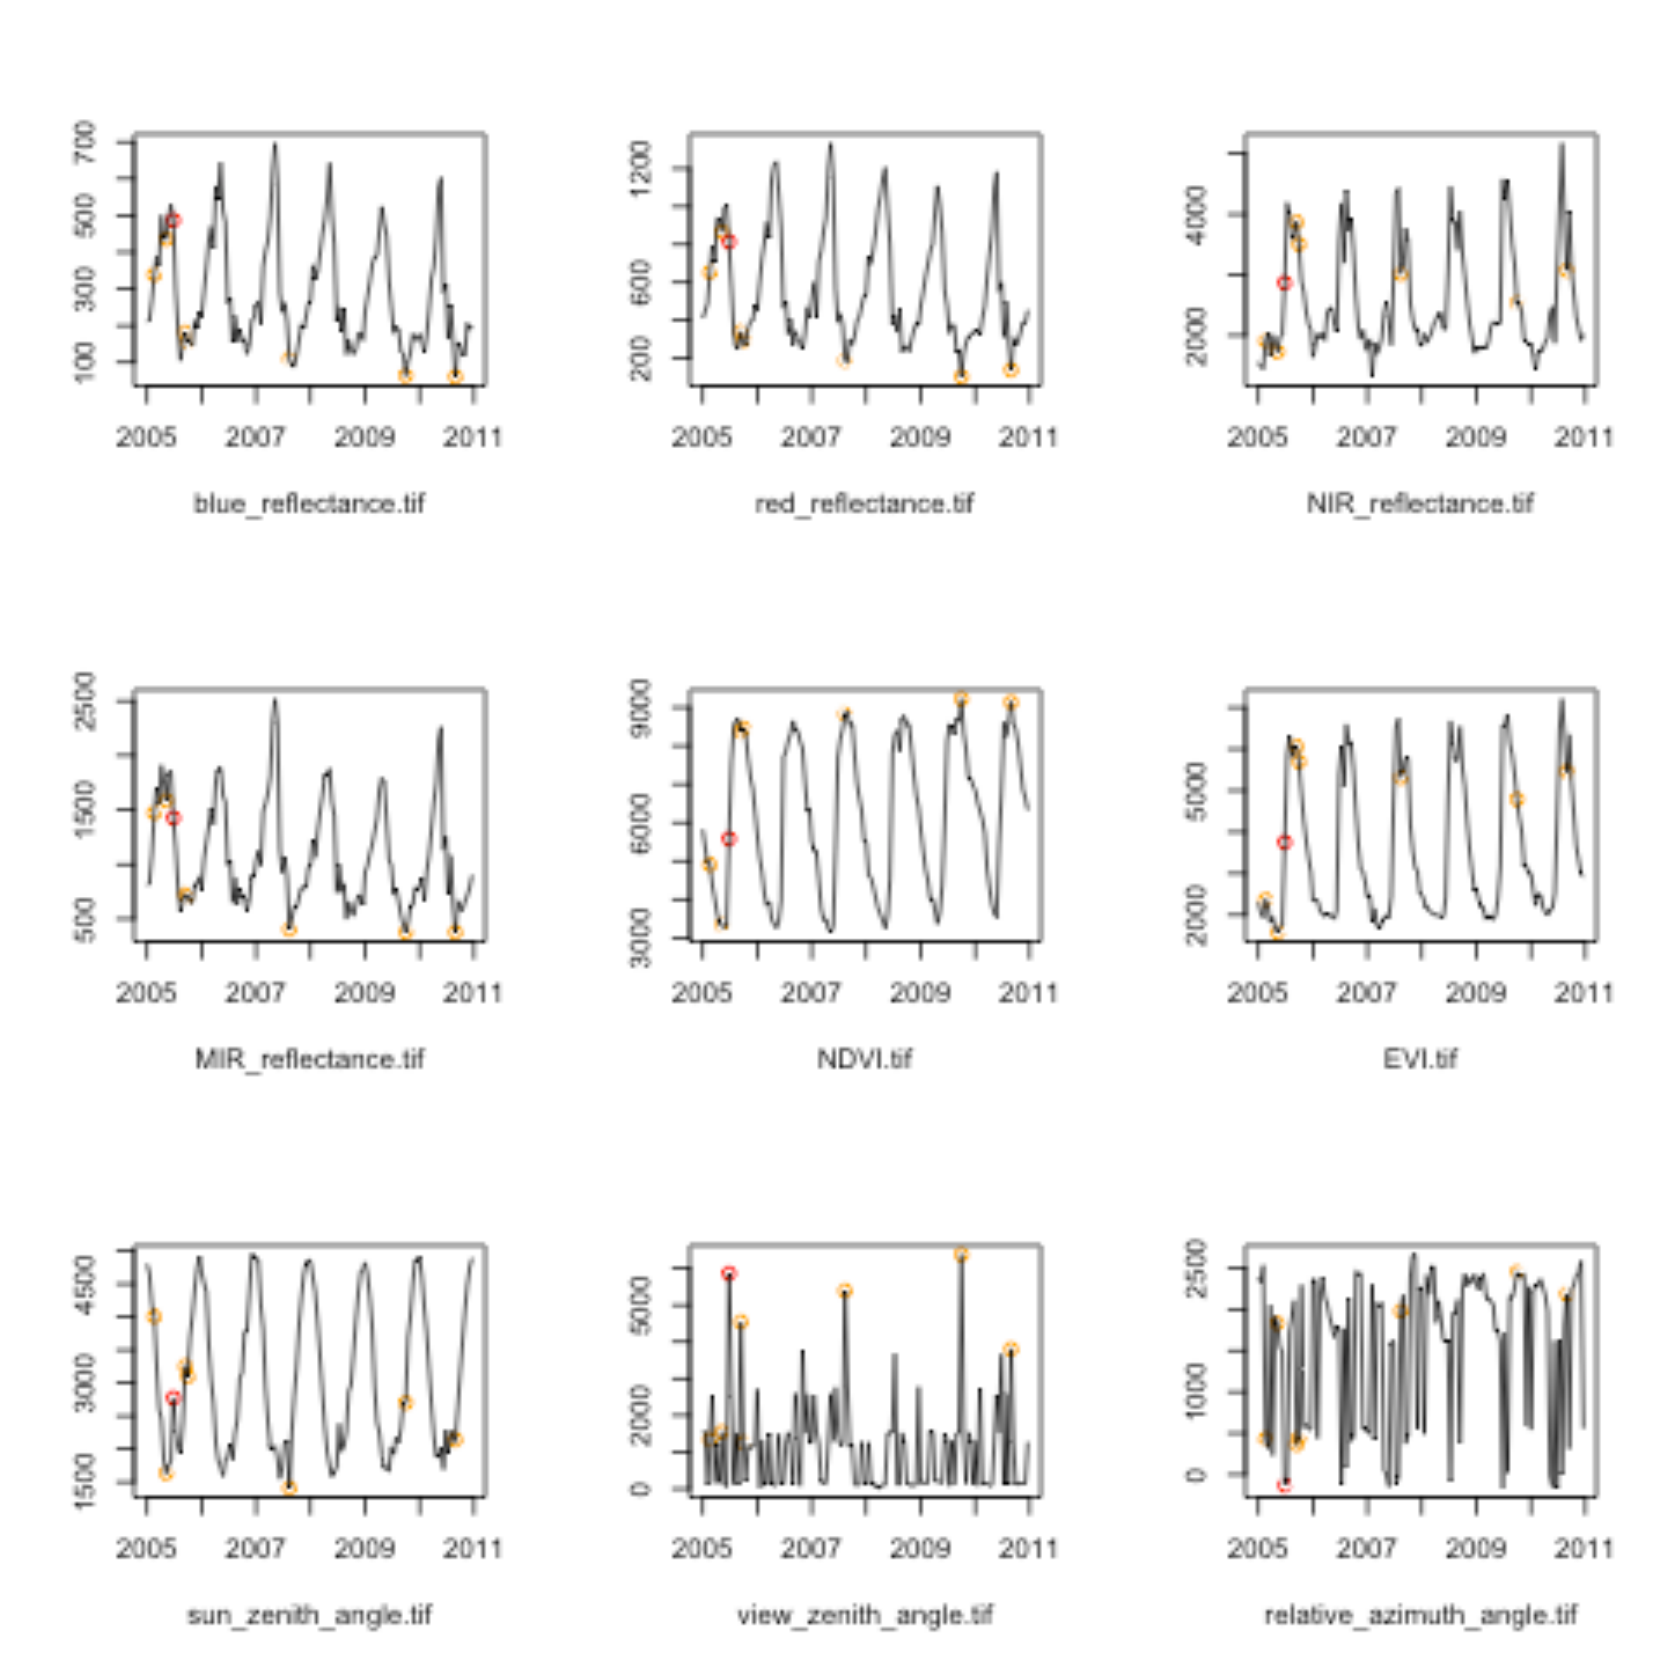}
   	        \caption{non-deforested pixel}
   	        \label{fig:non_defo_pix}
   	      \end{subfigure}
   	      %%         --- .5\textwidth stands for 50% of text width
   	      \caption[Reflectance, vegetation indices and sun-sensor geometry time series for deforested and non-deforested pixel in Yucatan 180 site.]%<<-- Legend for the list of figures at the beginning of you thesis
   	      {Reflectance, vegetation indices and sun-sensor geometry time series for deforested and non-deforested pixel in Nayarit151 site, identified in figure \ref{fig:defoNayarit151} with green and red circles respectively. Orange marked points are \emph{marginal data} and red marked points are \emph{cloudy} or \emph{not processed}}% legend displayed below the graph.
   	      \label{fig:timeSeries}
   	    \end{figure}
		
		\subsubsection{Nayarit109}
		
      	 \begin{figure}[H]  %--- Picture 'H'ere, 'B'ottom or 'T'op; '!' Try to
      	                     %impose your will to LaTeX
      	  % \centering 
  
      	   \begin{subfigure}{.5\textwidth}
      	     \centering
      	 	\includegraphics[width=0.7\textwidth]{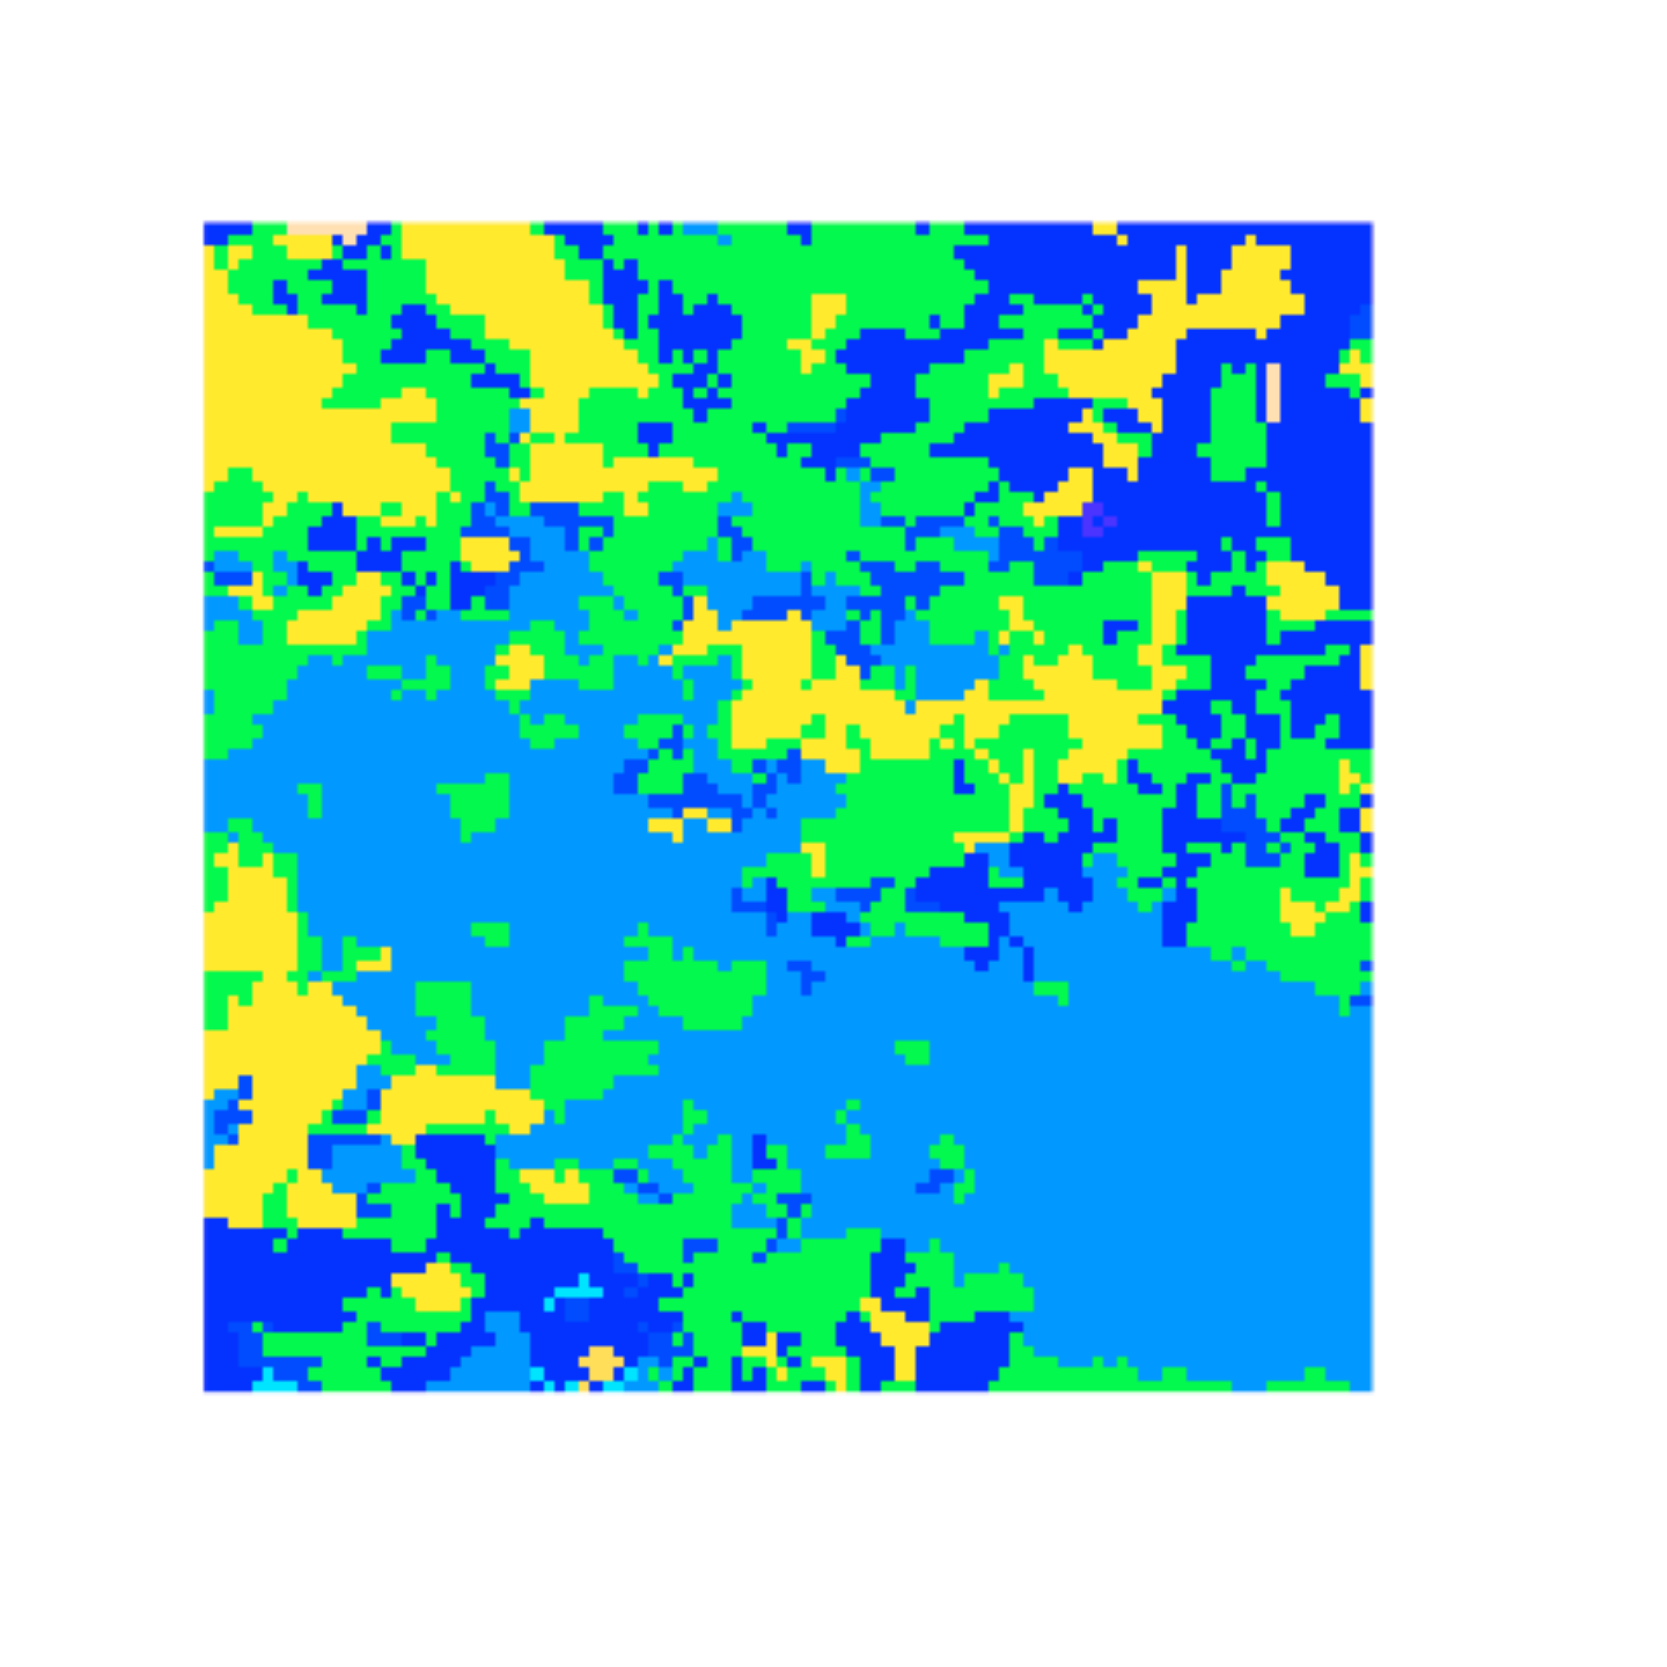} 
      	     \caption{Land-use 2005}
      	     \label{fig:sfig1a}
      	   \end{subfigure}%
      	   \begin{subfigure}{.5\textwidth}
      	     \centering
      	     \includegraphics[width=0.7\textwidth]{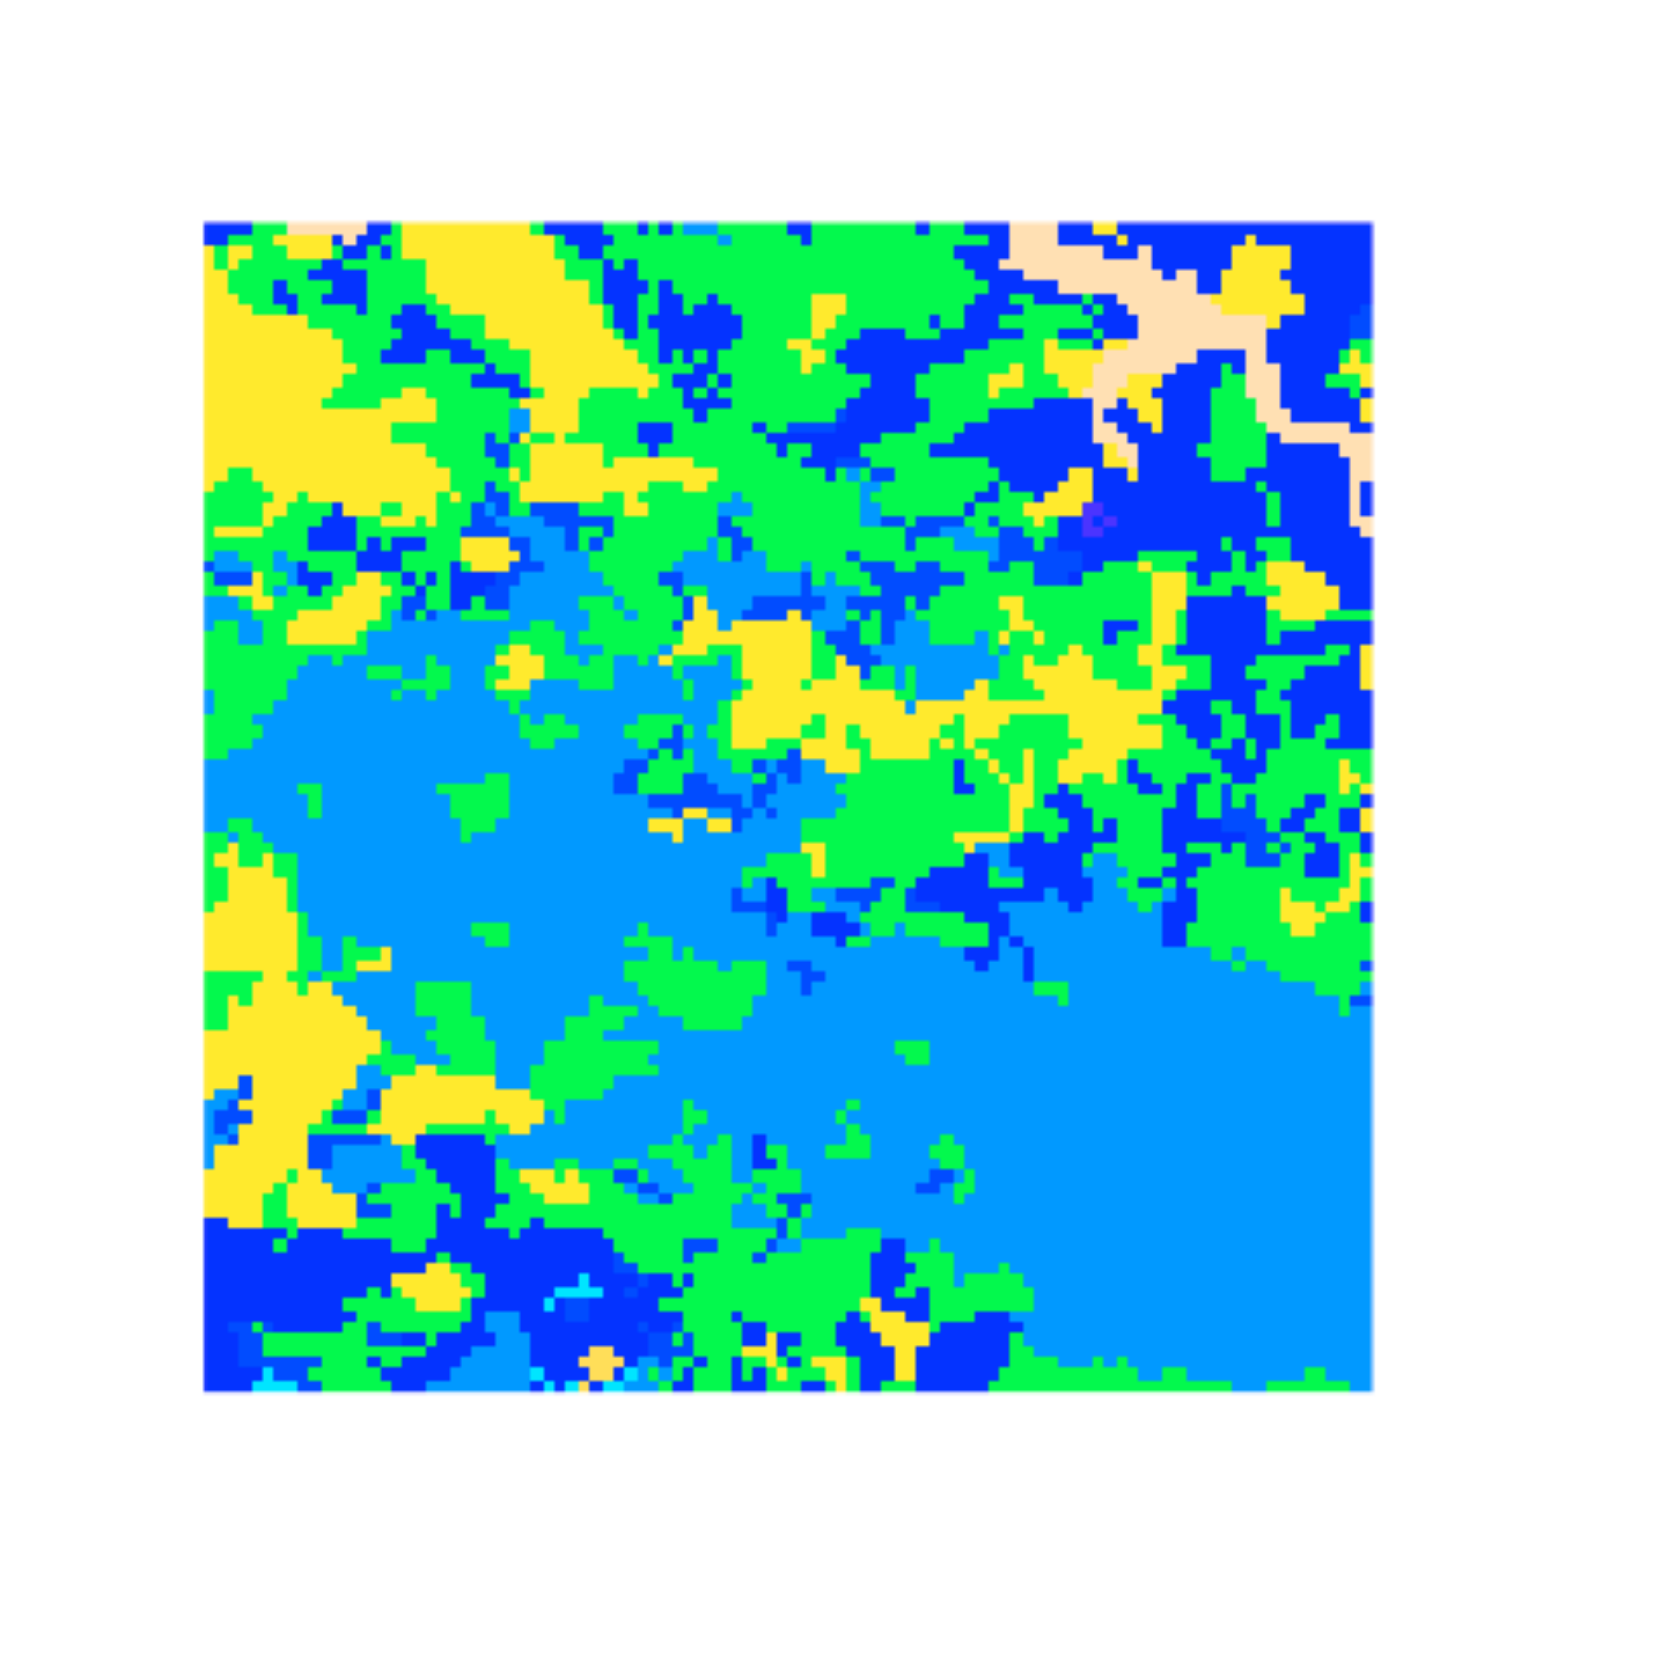}
      	     \caption{Land-use 2010}
      	     \label{fig:sfig1b}
      	   \end{subfigure}
      	   \begin{subfigure}{.4\textwidth}
      	     \centering
      	     \includegraphics[width=0.9\textwidth]{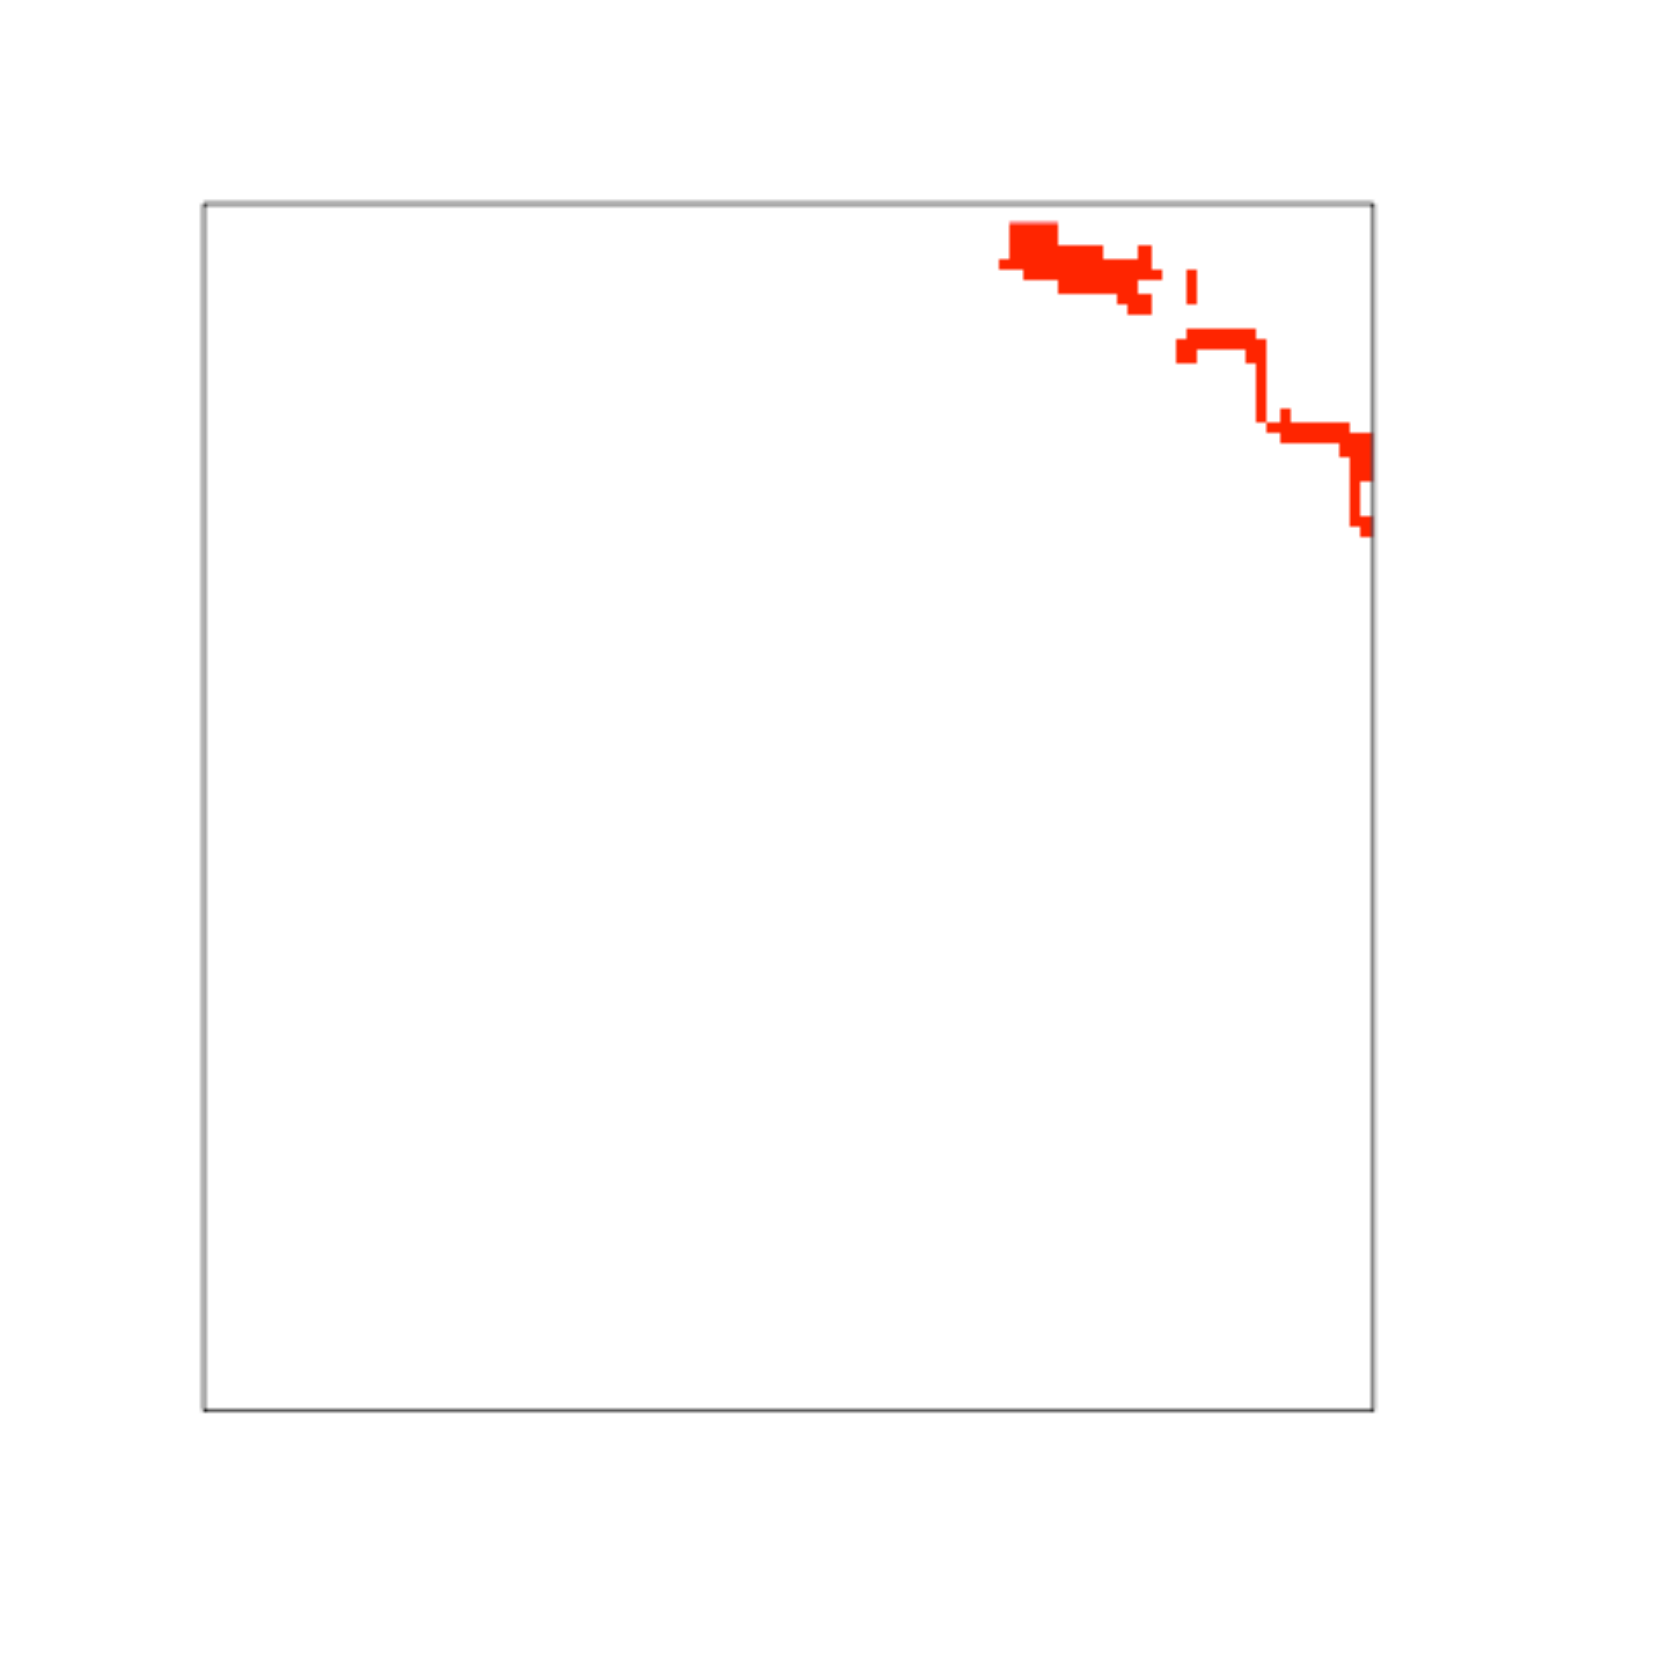}
      	     \caption{Deforestation 2005-2010}
      	     \label{fig:sfig1c}
      	   \end{subfigure}
      	   \begin{subfigure}{.4\textwidth}
      	     \centering
      	     \includegraphics[width=0.9\textwidth]{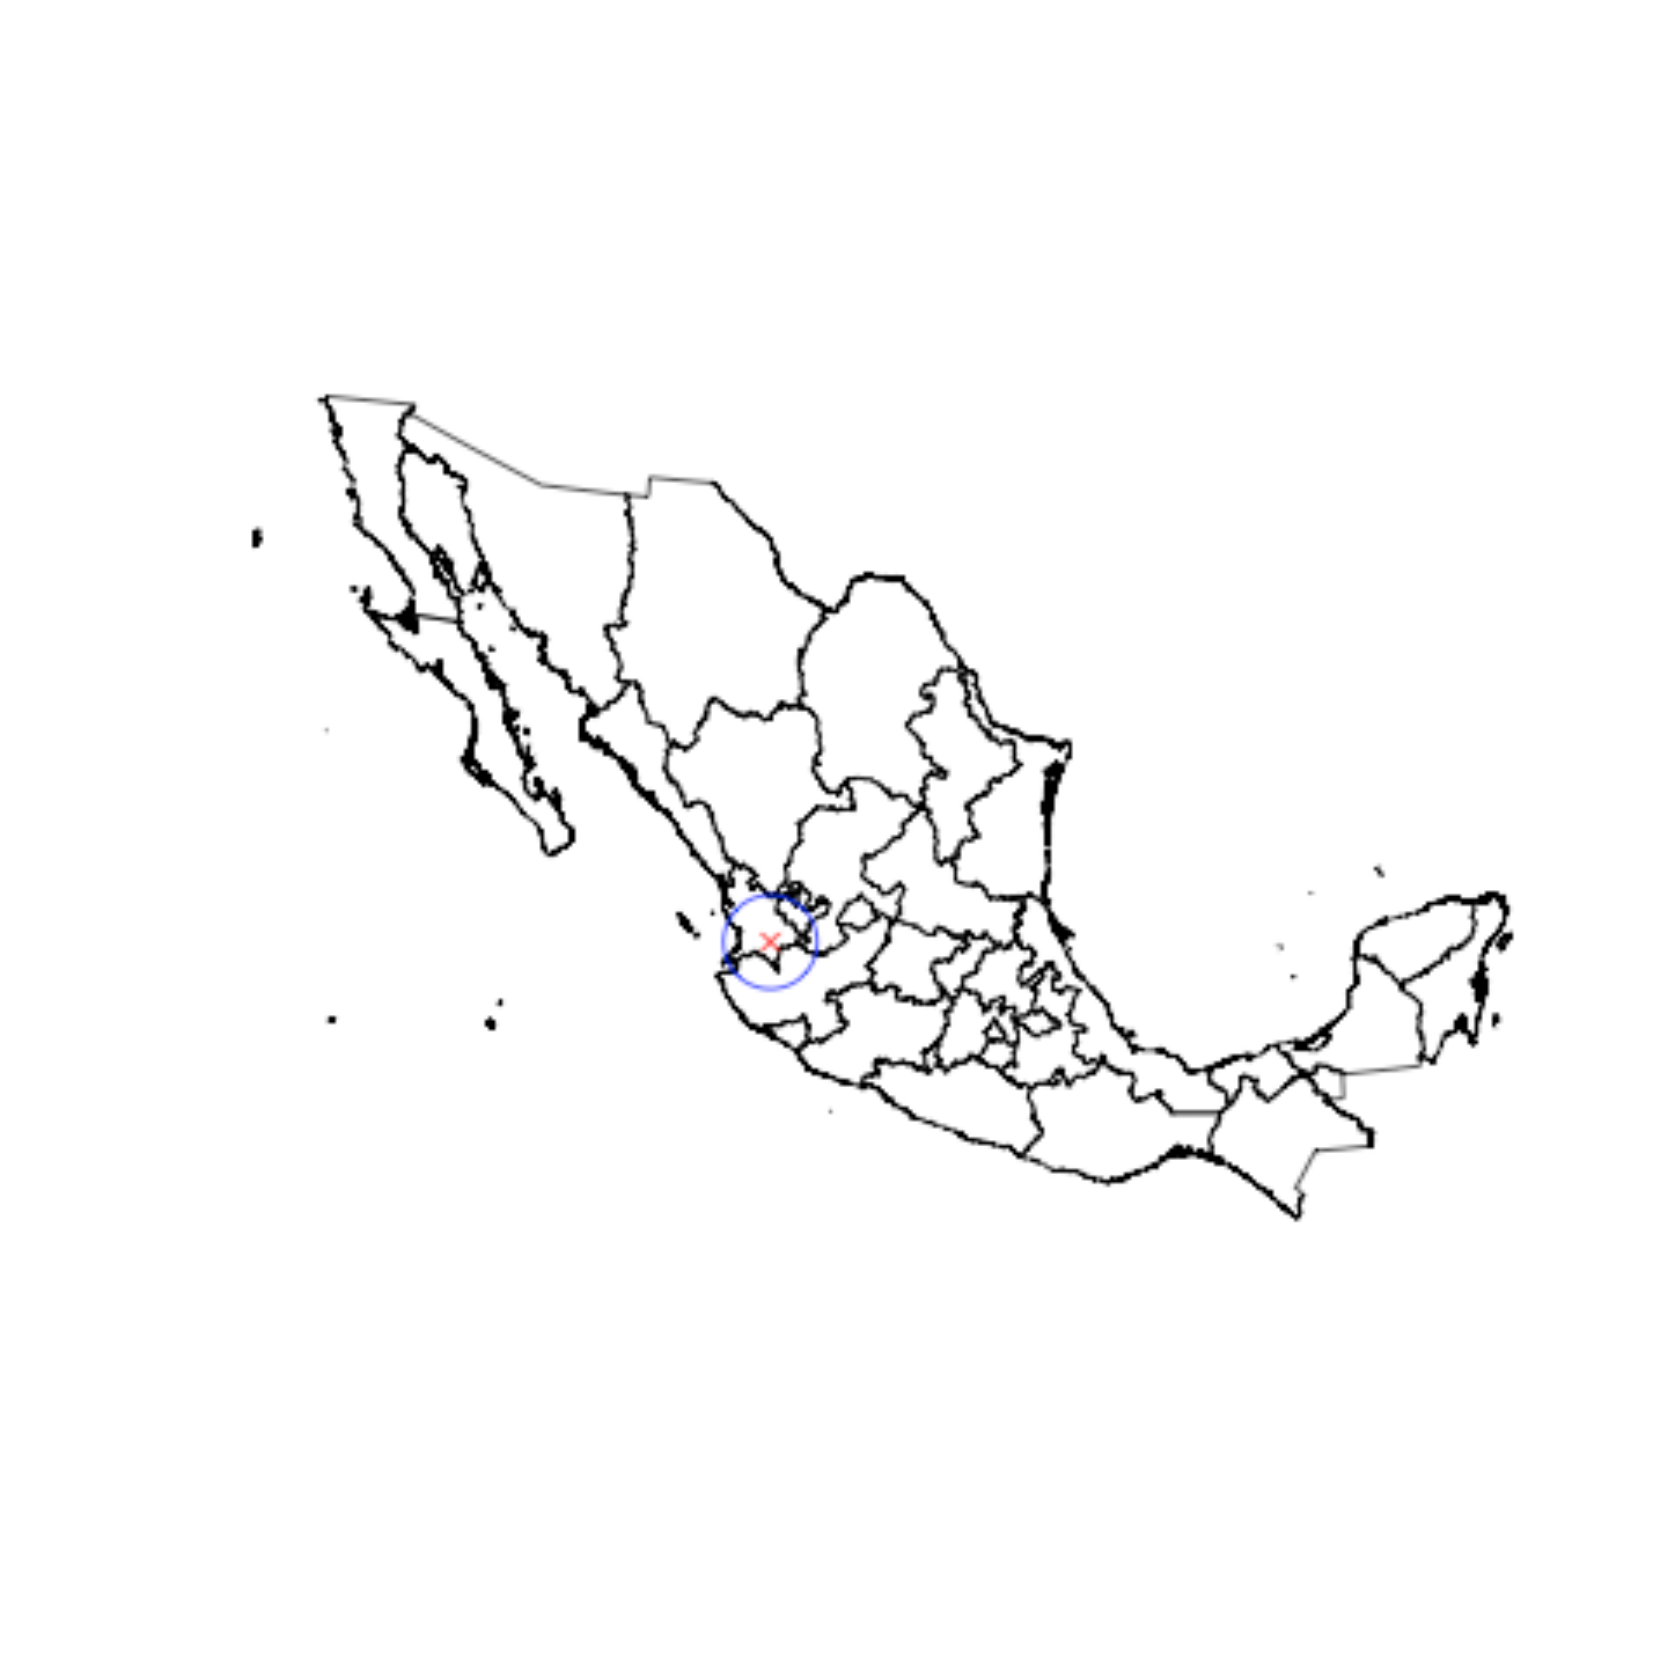}
      	     \caption{Location}
      	     \label{fig:sfig1d}
      	   \end{subfigure}   
         \begin{subfigure}{.5\textwidth}
           \centering
           \includegraphics[width=1\textwidth]{./2_Data/legend_landUse}
           \caption{Land use legend}
           \label{fig:legend}
         \end{subfigure}
      	   %%         --- .5\textwidth stands for 50% of text width
      	   \caption[NALCMS land-use classification of Nayarit109 site, 2005 and 2010 at 250m resolution.]%<<-- Legend for the list of figures at the beginning of you thesis
      	   {NALCMS land-use classification of Nayarit109 site, 2005 and 2010 at 250m resolution.}% legend displayed below the graph.
      	   \label{fig:landUseNayarit109}
      	 \end{figure}
		
   		\begin{center}
   			\footnotesize\addtolength{\tabcolsep}{-2pt}
   			% latex table generated in R 3.3.1 by xtable 1.8-2 package
% Sun Mar  5 15:59:41 2017
\begin{table}[ht]
\centering
\begingroup\tiny
\begin{tabular}{rrrrrrrrrrrrrrrrrrrrr}
  & \begin{sideways} Temperate or sub-polar needleleaf forest \end{sideways} & \begin{sideways} Sub-polar taiga needleleaf forest \end{sideways} & \begin{sideways} Tropical or sub-tropical broadleaf evergreen forest \end{sideways} & \begin{sideways} Tropical or sub-tropical broadleaf deciduous forest \end{sideways} & \begin{sideways} Temperate or sub-polar broadleaf deciduous forest \end{sideways} & \begin{sideways} Mixed Forest \end{sideways} & \begin{sideways} Tropical or sub-tropical shrubland \end{sideways} & \begin{sideways} Temperate or sub-polar shrubland \end{sideways} & \begin{sideways} Tropical or sub-tropical grassland \end{sideways} & \begin{sideways} Temperate or sub-polar grassland \end{sideways} & \begin{sideways} Sub-polar or polar shrubland-lichen-moss \end{sideways} & \begin{sideways} Sub-polar or polar grassland-lichen-moss \end{sideways} & \begin{sideways} Sub-polar or polar barren-lichen-moss \end{sideways} & \begin{sideways} Wetland \end{sideways} & \begin{sideways} Cropland \end{sideways} & \begin{sideways} Barren Lands \end{sideways} & \begin{sideways} Urban and Built-up \end{sideways} & \begin{sideways} Water \end{sideways} & \begin{sideways} Snow and Ice \end{sideways} & \begin{sideways} Total \end{sideways} \\ 
  \hline
Temperate or sub-polar needleleaf forest &    0 &    0 &    0 &    0 &    0 &    0 &    0 &    0 &    0 &    0 &    0 &    0 &    0 &    0 &    0 &    0 &    0 &    0 &    0 &    0 \\ 
  Sub-polar taiga needleleaf forest &    0 &    0 &    0 &    0 &    0 &    0 &    0 &    0 &    0 &    0 &    0 &    0 &    0 &    0 &    0 &    0 &    0 &    0 &    0 &    0 \\ 
  Tropical or sub-tropical broadleaf evergreen forest &    0 &    0 &    6 &    0 &    0 &    0 &    0 &    0 &    0 &    0 &    0 &    0 &    0 &    0 &    0 &    0 &    0 &    0 &    0 &    6 \\ 
  Tropical or sub-tropical broadleaf deciduous forest &    0 &    0 &    0 & 1658 &    0 &    0 &    0 &    0 &    0 &    0 &    0 &    0 &    0 &    0 &    0 &    0 &    0 &  109 &    0 & 1767 \\ 
  Temperate or sub-polar broadleaf deciduous forest &    0 &    0 &    0 &    0 &  337 &    0 &    0 &    0 &    0 &    0 &    0 &    0 &    0 &    0 &    0 &    0 &    0 &    0 &    0 &  337 \\ 
  Mixed Forest &    0 &    0 &    0 &    0 &    0 & 3266 &    0 &    0 &    0 &    0 &    0 &    0 &    0 &    0 &    0 &    0 &    0 &    0 &    0 & 3266 \\ 
   \hline
Tropical or sub-tropical shrubland &    0 &    0 &    0 &    0 &    0 &    0 &   17 &    0 &    0 &    0 &    0 &    0 &    0 &    0 &    0 &    0 &    0 &    0 &    0 &   17 \\ 
  Temperate or sub-polar shrubland &    0 &    0 &    0 &    4 &    0 &    0 &    0 & 3059 &    0 &    0 &    0 &    0 &    0 &    0 &    0 &    0 &    0 &    8 &    0 & 3071 \\ 
  Tropical or sub-tropical grassland &    0 &    0 &    0 &    0 &    0 &    0 &    0 &    0 &    0 &    0 &    0 &    0 &    0 &    0 &    0 &    0 &    0 &    0 &    0 &    0 \\ 
  Temperate or sub-polar grassland &    0 &    0 &    0 &    0 &    0 &    0 &    0 &    0 &    0 &    0 &    0 &    0 &    0 &    0 &    0 &    0 &    0 &    0 &    0 &    0 \\ 
  Sub-polar or polar shrubland-lichen-moss &    0 &    0 &    0 &    0 &    0 &    0 &    0 &    0 &    0 &    0 &    0 &    0 &    0 &    0 &    0 &    0 &    0 &    0 &    0 &    0 \\ 
  Sub-polar or polar grassland-lichen-moss &    0 &    0 &    0 &    0 &    0 &    0 &    0 &    0 &    0 &    0 &    0 &    0 &    0 &    0 &    0 &    0 &    0 &    0 &    0 &    0 \\ 
  Sub-polar or polar barren-lichen-moss &    0 &    0 &    0 &    0 &    0 &    0 &    0 &    0 &    0 &    0 &    0 &    0 &    0 &    0 &    0 &    0 &    0 &    0 &    0 &    0 \\ 
  Wetland &    0 &    0 &    0 &    0 &    0 &    0 &    0 &    0 &    0 &    0 &    0 &    0 &    0 &    0 &    0 &    0 &    0 &    0 &    0 &    0 \\ 
  Cropland &    0 &    0 &    0 &    6 &    0 &    0 &    0 &    0 &    0 &    0 &    0 &    0 &    0 &    0 & 1448 &    0 &    0 &   60 &    0 & 1514 \\ 
  Barren Lands &    0 &    0 &    0 &    0 &    0 &    0 &    0 &    0 &    0 &    0 &    0 &    0 &    0 &    0 &    0 &    9 &    0 &    0 &    0 &    9 \\ 
  Urban and Built-up &    0 &    0 &    0 &    0 &    0 &    0 &    0 &    0 &    0 &    0 &    0 &    0 &    0 &    0 &    0 &    0 &    0 &    0 &    0 &    0 \\ 
  Water &    0 &    0 &    0 &    0 &    0 &    0 &    0 &    0 &    0 &    0 &    0 &    0 &    0 &    0 &    0 &    0 &    0 &   13 &    0 &   13 \\ 
  Snow and Ice &    0 &    0 &    0 &    0 &    0 &    0 &    0 &    0 &    0 &    0 &    0 &    0 &    0 &    0 &    0 &    0 &    0 &    0 &    0 &    0 \\ 
   \hline
Total &    0 &    0 &    6 & 1668 &  337 & 3266 &   17 & 3059 &    0 &    0 &    0 &    0 &    0 &    0 & 1448 &    9 &    0 &  190 &    0 & 10000 \\ 
   \hline
\end{tabular}
\endgroup
\caption[NALCMS land-use distribution for site Nayarit109, 2005 and 2010.]{NALCMS land-use distribution for site Nayarit109, 2005 and 2010.} 
\end{table}

   			\label{tab:landUseSonora}
   		\end{center}
		
   		\begin{figure}[H]%--- Picture 'H'ere, 'B'ottom or 'T'op; '!' Try to
   		                    %impose your will to LaTeX
   		  \centering
   		  \includegraphics[width=.5\textwidth]{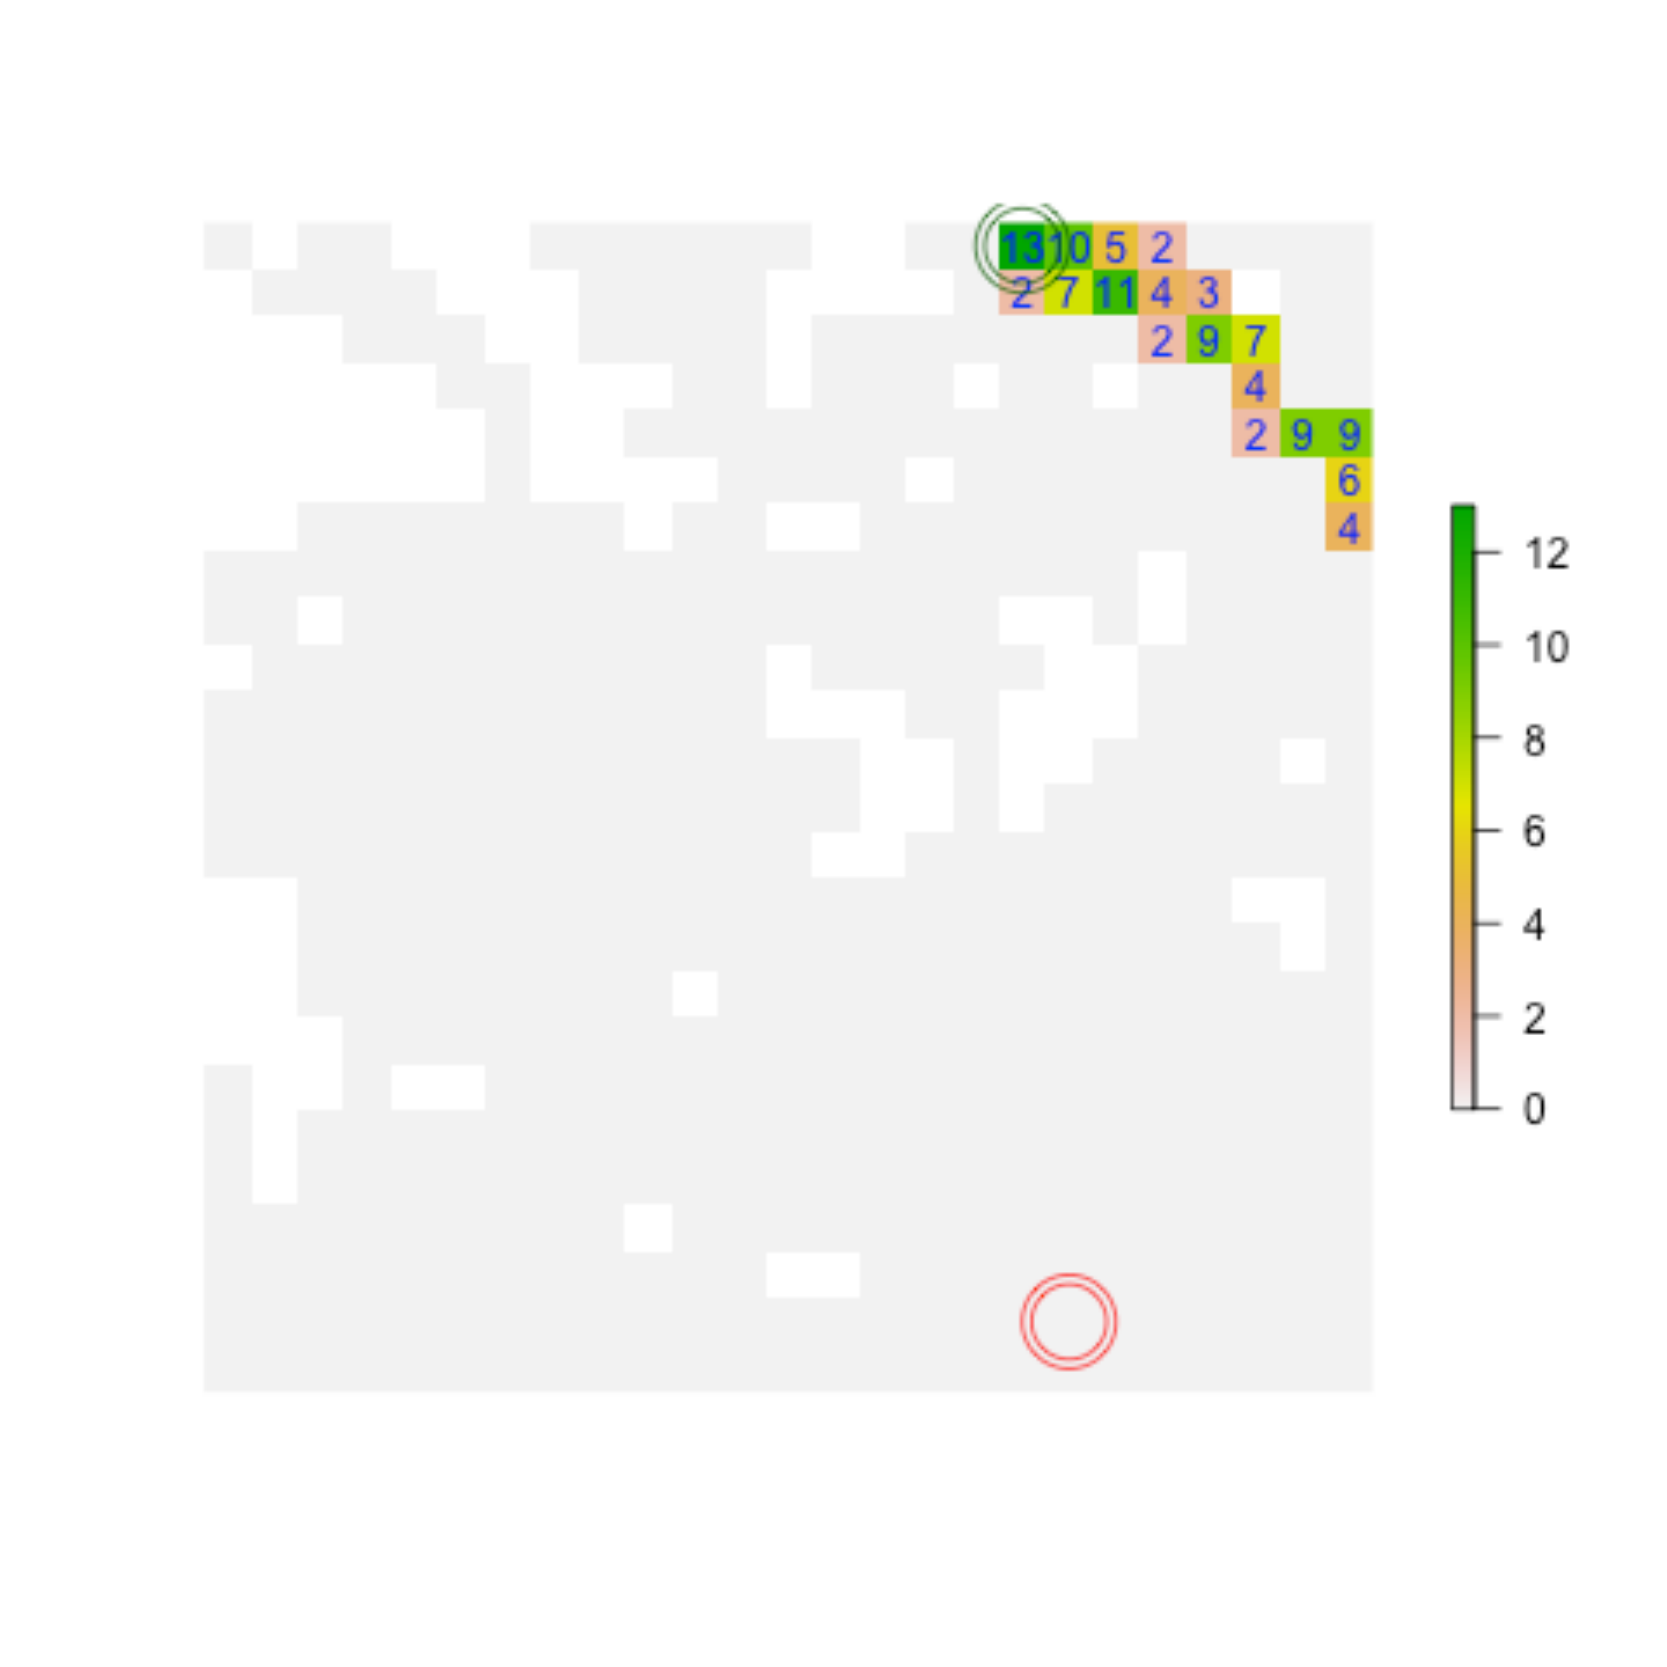} %<< no file extension
   		  %%         --- .5\textwidth stands for 50% of text width
   		  \caption[Deforestation in Nayarit109 site at 1km resolution]%<<-- Legend for the list of figures at the beginning of you thesis
   		  {Deforestation in Nayarit109 site at 1km resolution: number of 250m pixels deforested out of 16}% legend displayed below the graph.
   		  \label{fig:defoNayarit109}
   		\end{figure}
		
   		 \begin{figure}[H]
   	      \begin{subfigure}{.5\textwidth}
   	        \centering
   	    	\includegraphics[width=1\textwidth]{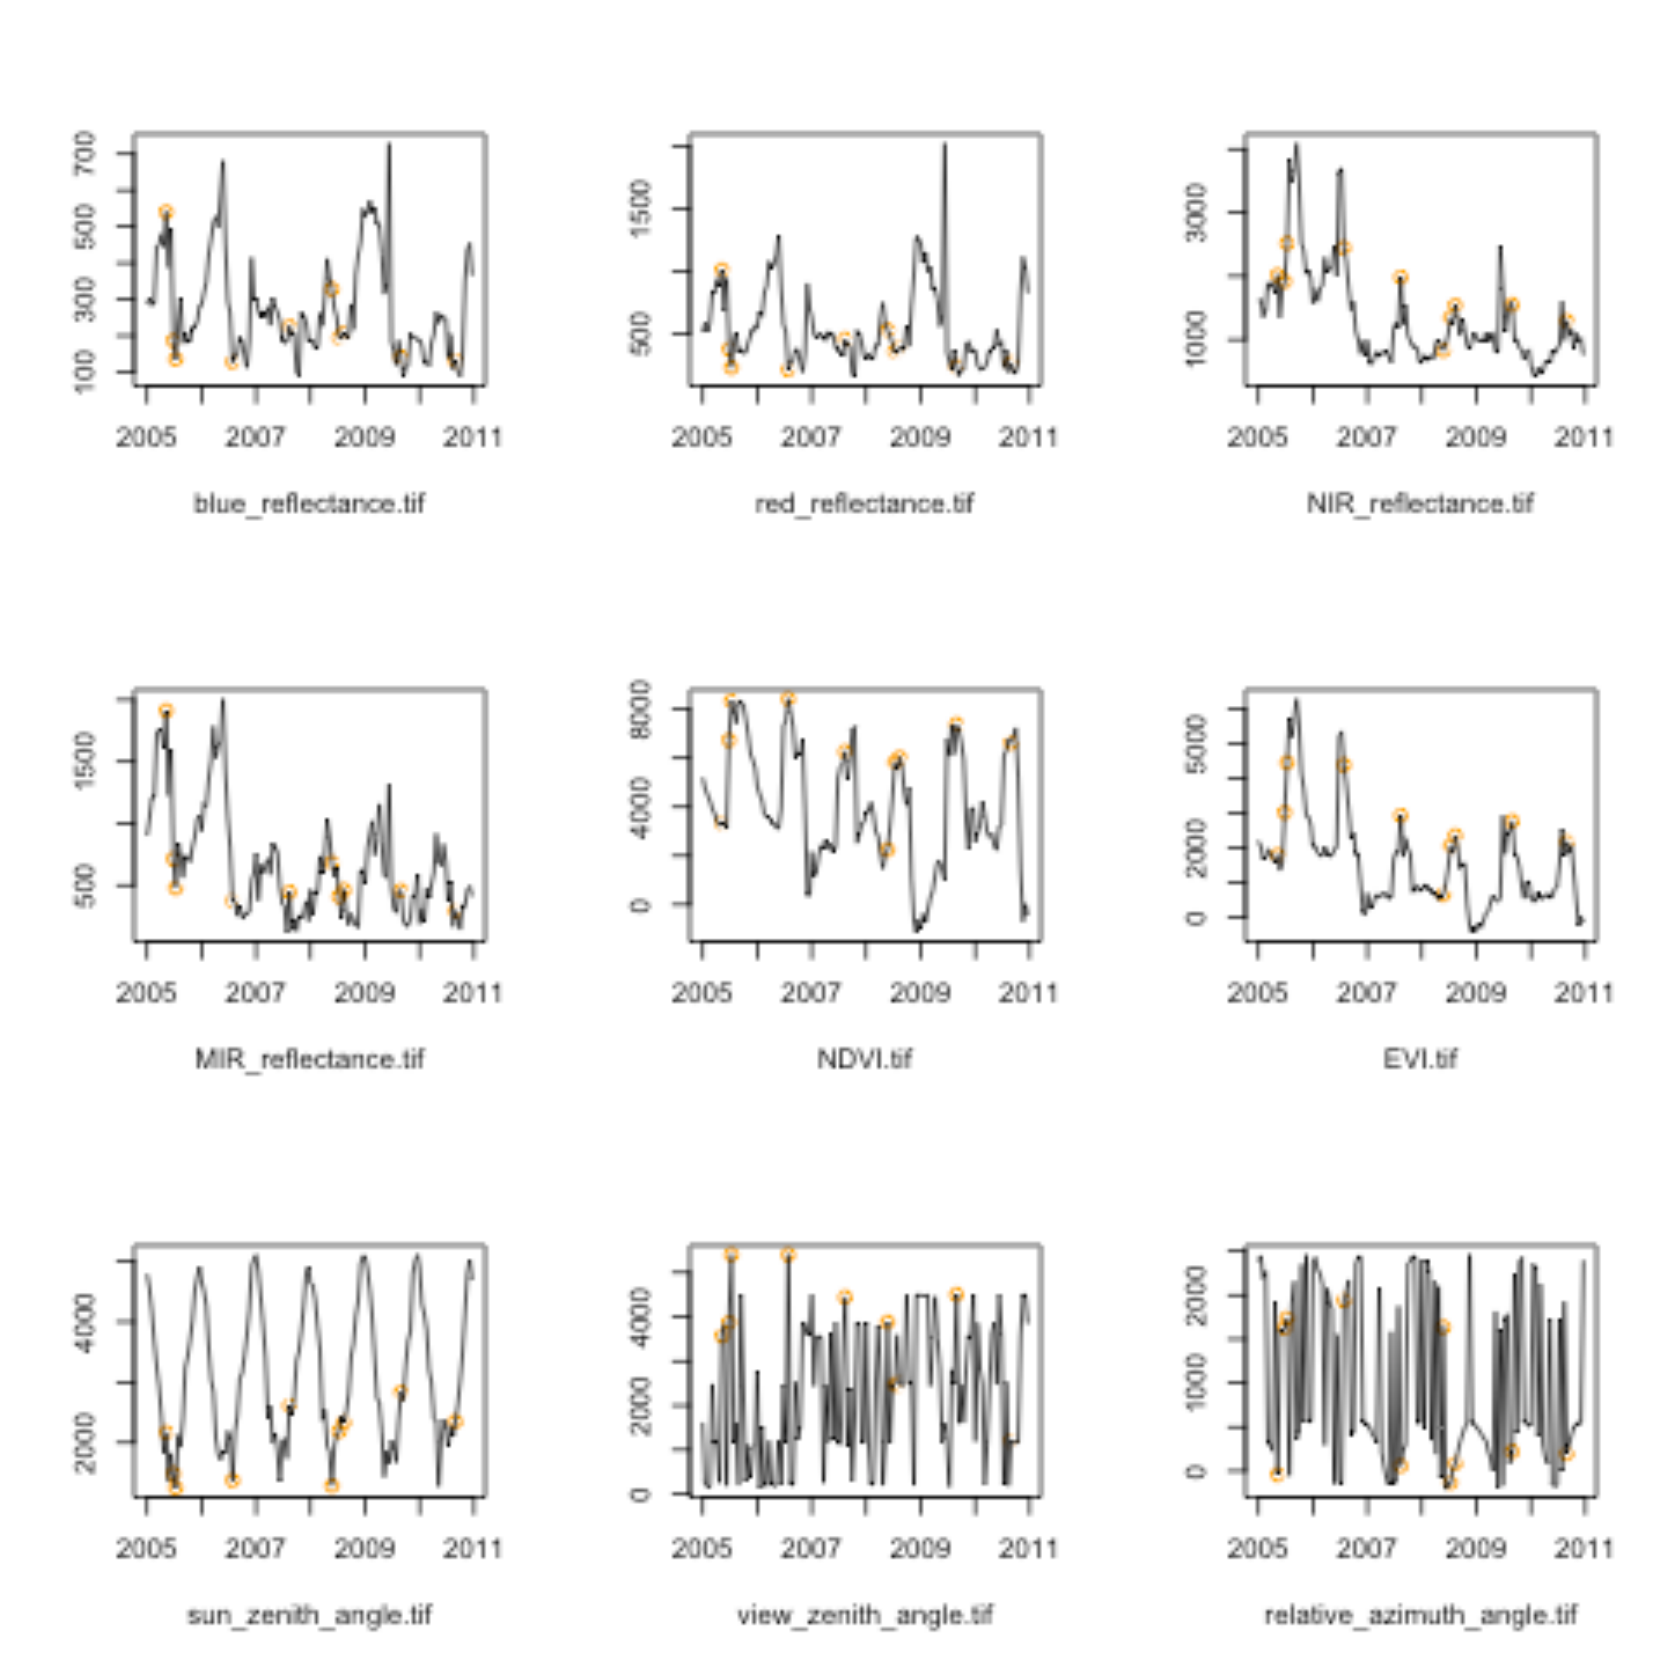} 
   	        \caption{deforested pixel}
   	        \label{fig:defo_pix}
   	      \end{subfigure}%
   	      \begin{subfigure}{.5\textwidth}
   	        \centering
   	        \includegraphics[width=1\textwidth]{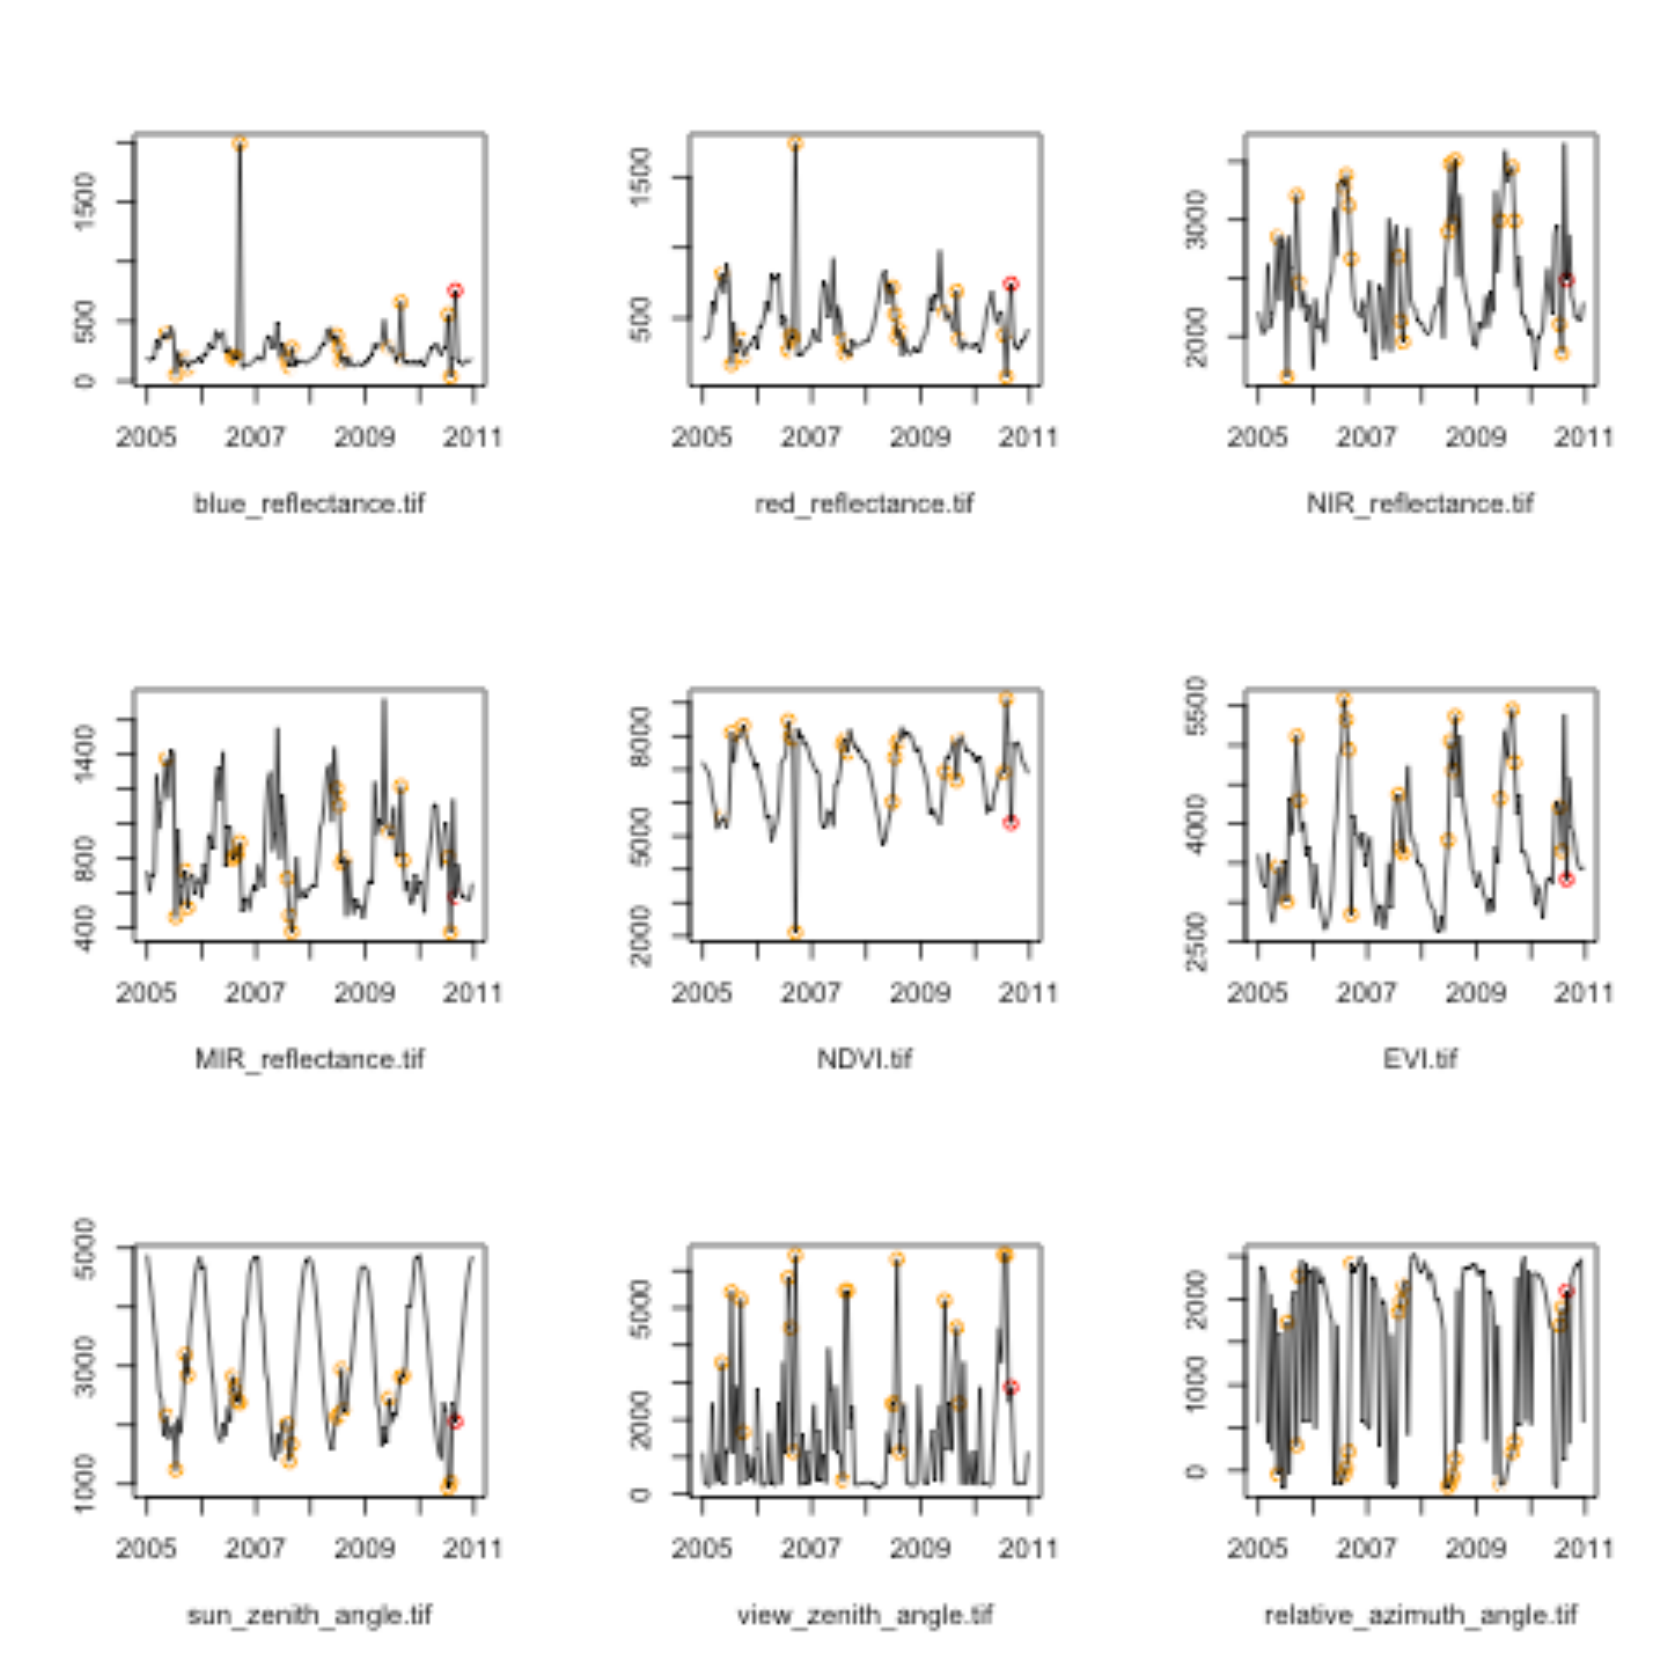}
   	        \caption{non-deforested pixel}
   	        \label{fig:non_defo_pix}
   	      \end{subfigure}
   	      %%         --- .5\textwidth stands for 50% of text width
   	      \caption[Reflectance, vegetation indices and sun-sensor geometry time series for deforested and non-deforested pixel in Yucatan 180 site.]%<<-- Legend for the list of figures at the beginning of you thesis
   	      {Reflectance, vegetation indices and sun-sensor geometry time series for deforested and non-deforested pixel in Nayarit109 site, identified in figure \ref{fig:defoNayarit109} with green and red circles respectively. Orange marked points are \emph{marginal data} and red marked points are \emph{cloudy} or \emph{not processed}}% legend displayed below the graph.
   	      \label{fig:timeSeries}
   	    \end{figure}
		
\subsection{Forest to urban or cropland sites}
		
		\subsubsection{QuintanaRoo100}
		
      	 \begin{figure}[H]  %--- Picture 'H'ere, 'B'ottom or 'T'op; '!' Try to
      	                     %impose your will to LaTeX
      	  % \centering 
  
      	   \begin{subfigure}{.5\textwidth}
      	     \centering
      	 	\includegraphics[width=0.7\textwidth]{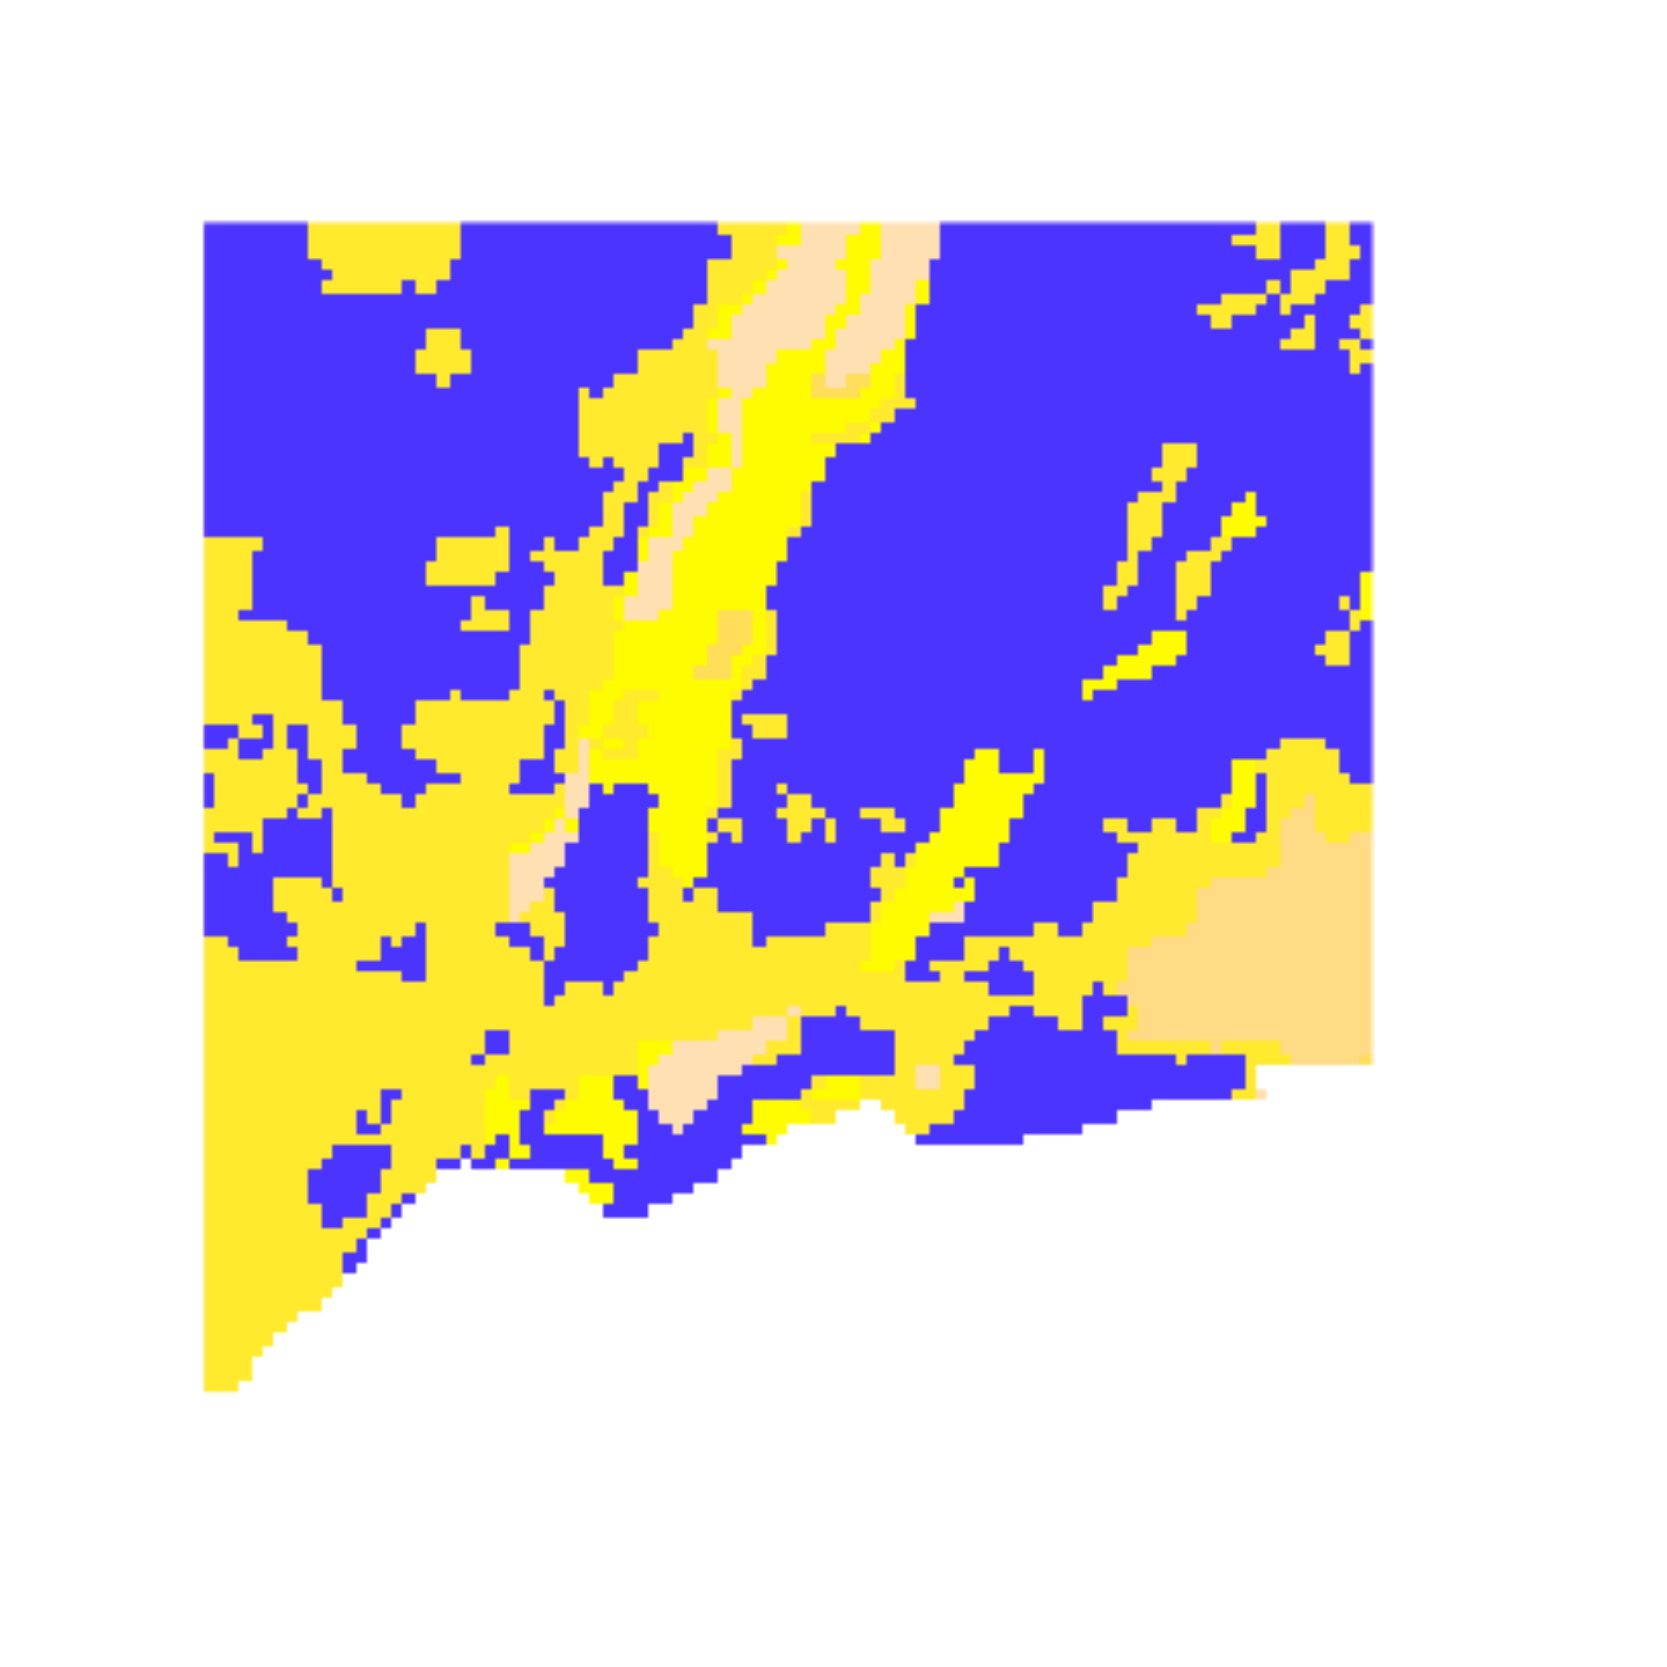} 
      	     \caption{Land-use 2005}
      	     \label{fig:sfig1a}
      	   \end{subfigure}%
      	   \begin{subfigure}{.5\textwidth}
      	     \centering
      	     \includegraphics[width=0.7\textwidth]{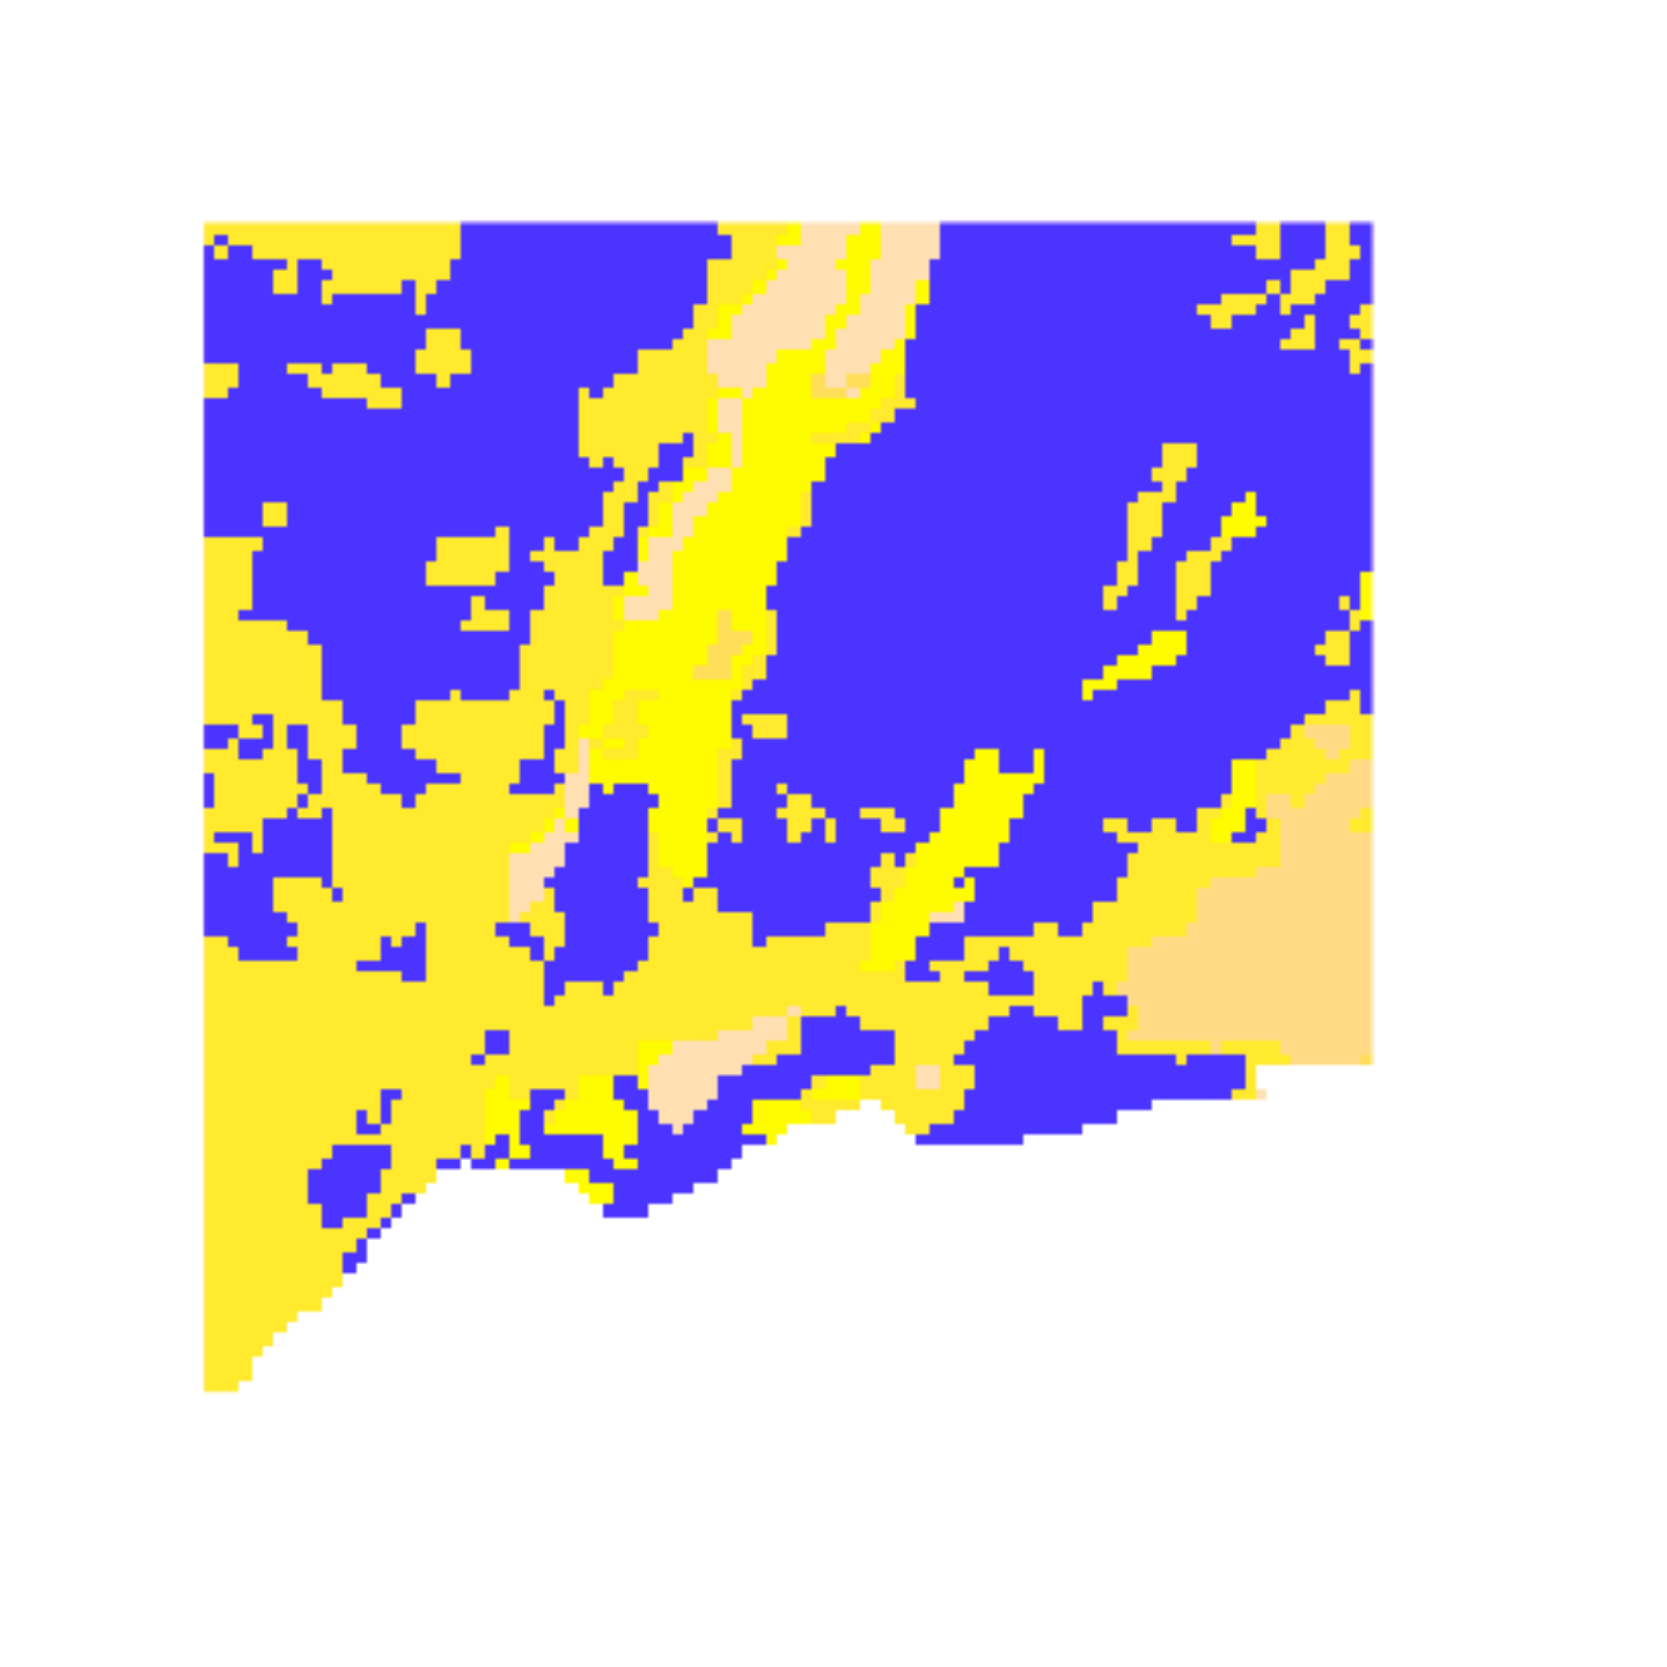}
      	     \caption{Land-use 2010}
      	     \label{fig:sfig1b}
      	   \end{subfigure}
      	   \begin{subfigure}{.4\textwidth}
      	     \centering
      	     \includegraphics[width=0.9\textwidth]{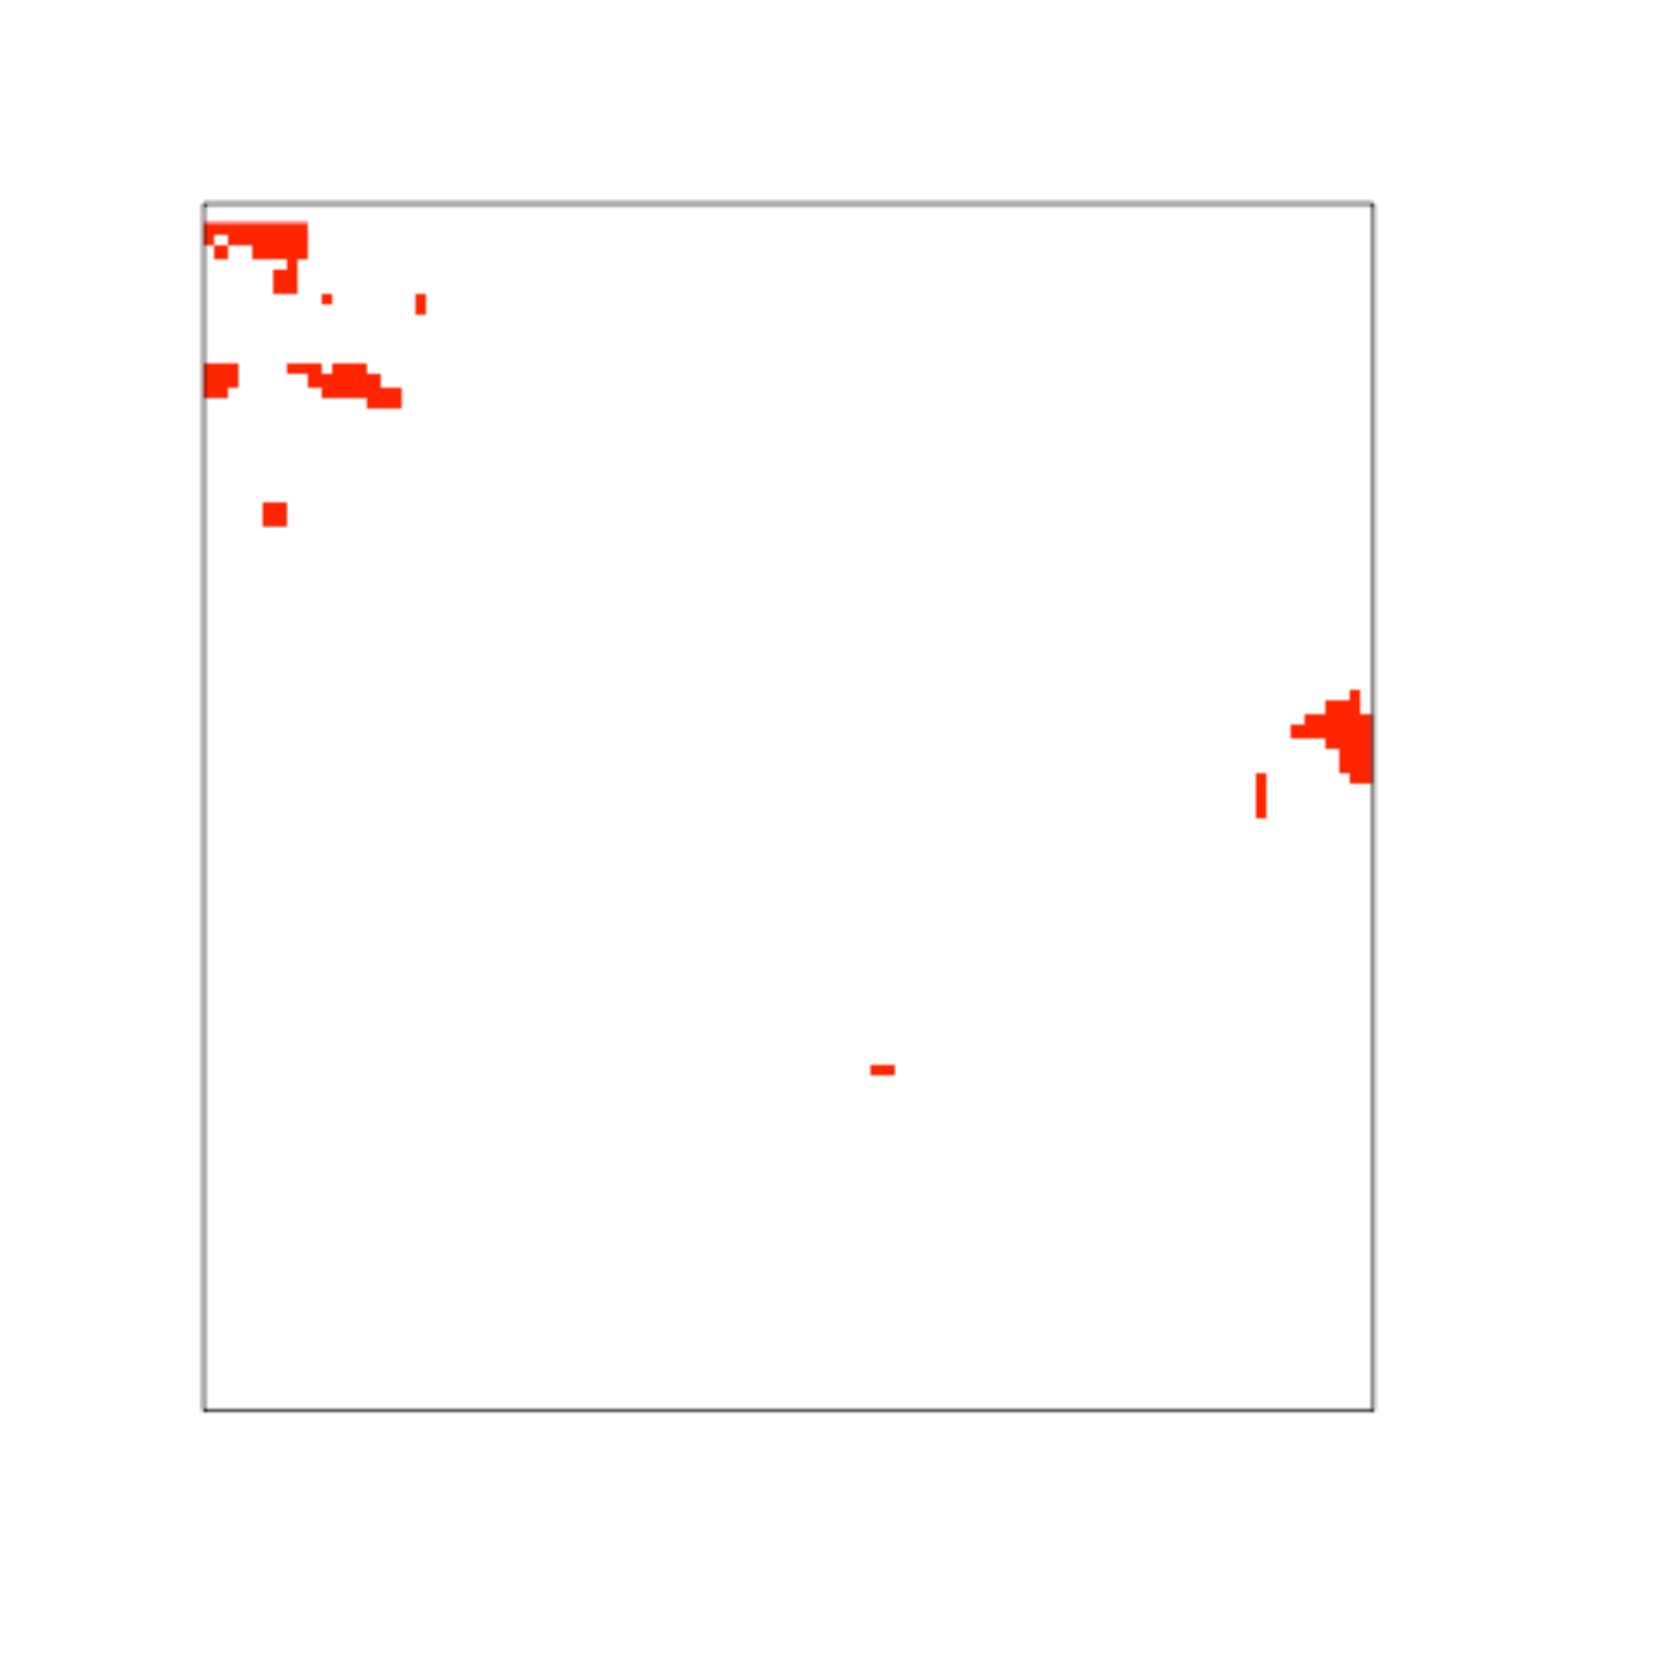}
      	     \caption{Deforestation 2005-2010}
      	     \label{fig:sfig1c}
      	   \end{subfigure}
      	   \begin{subfigure}{.4\textwidth}
      	     \centering
      	     \includegraphics[width=0.9\textwidth]{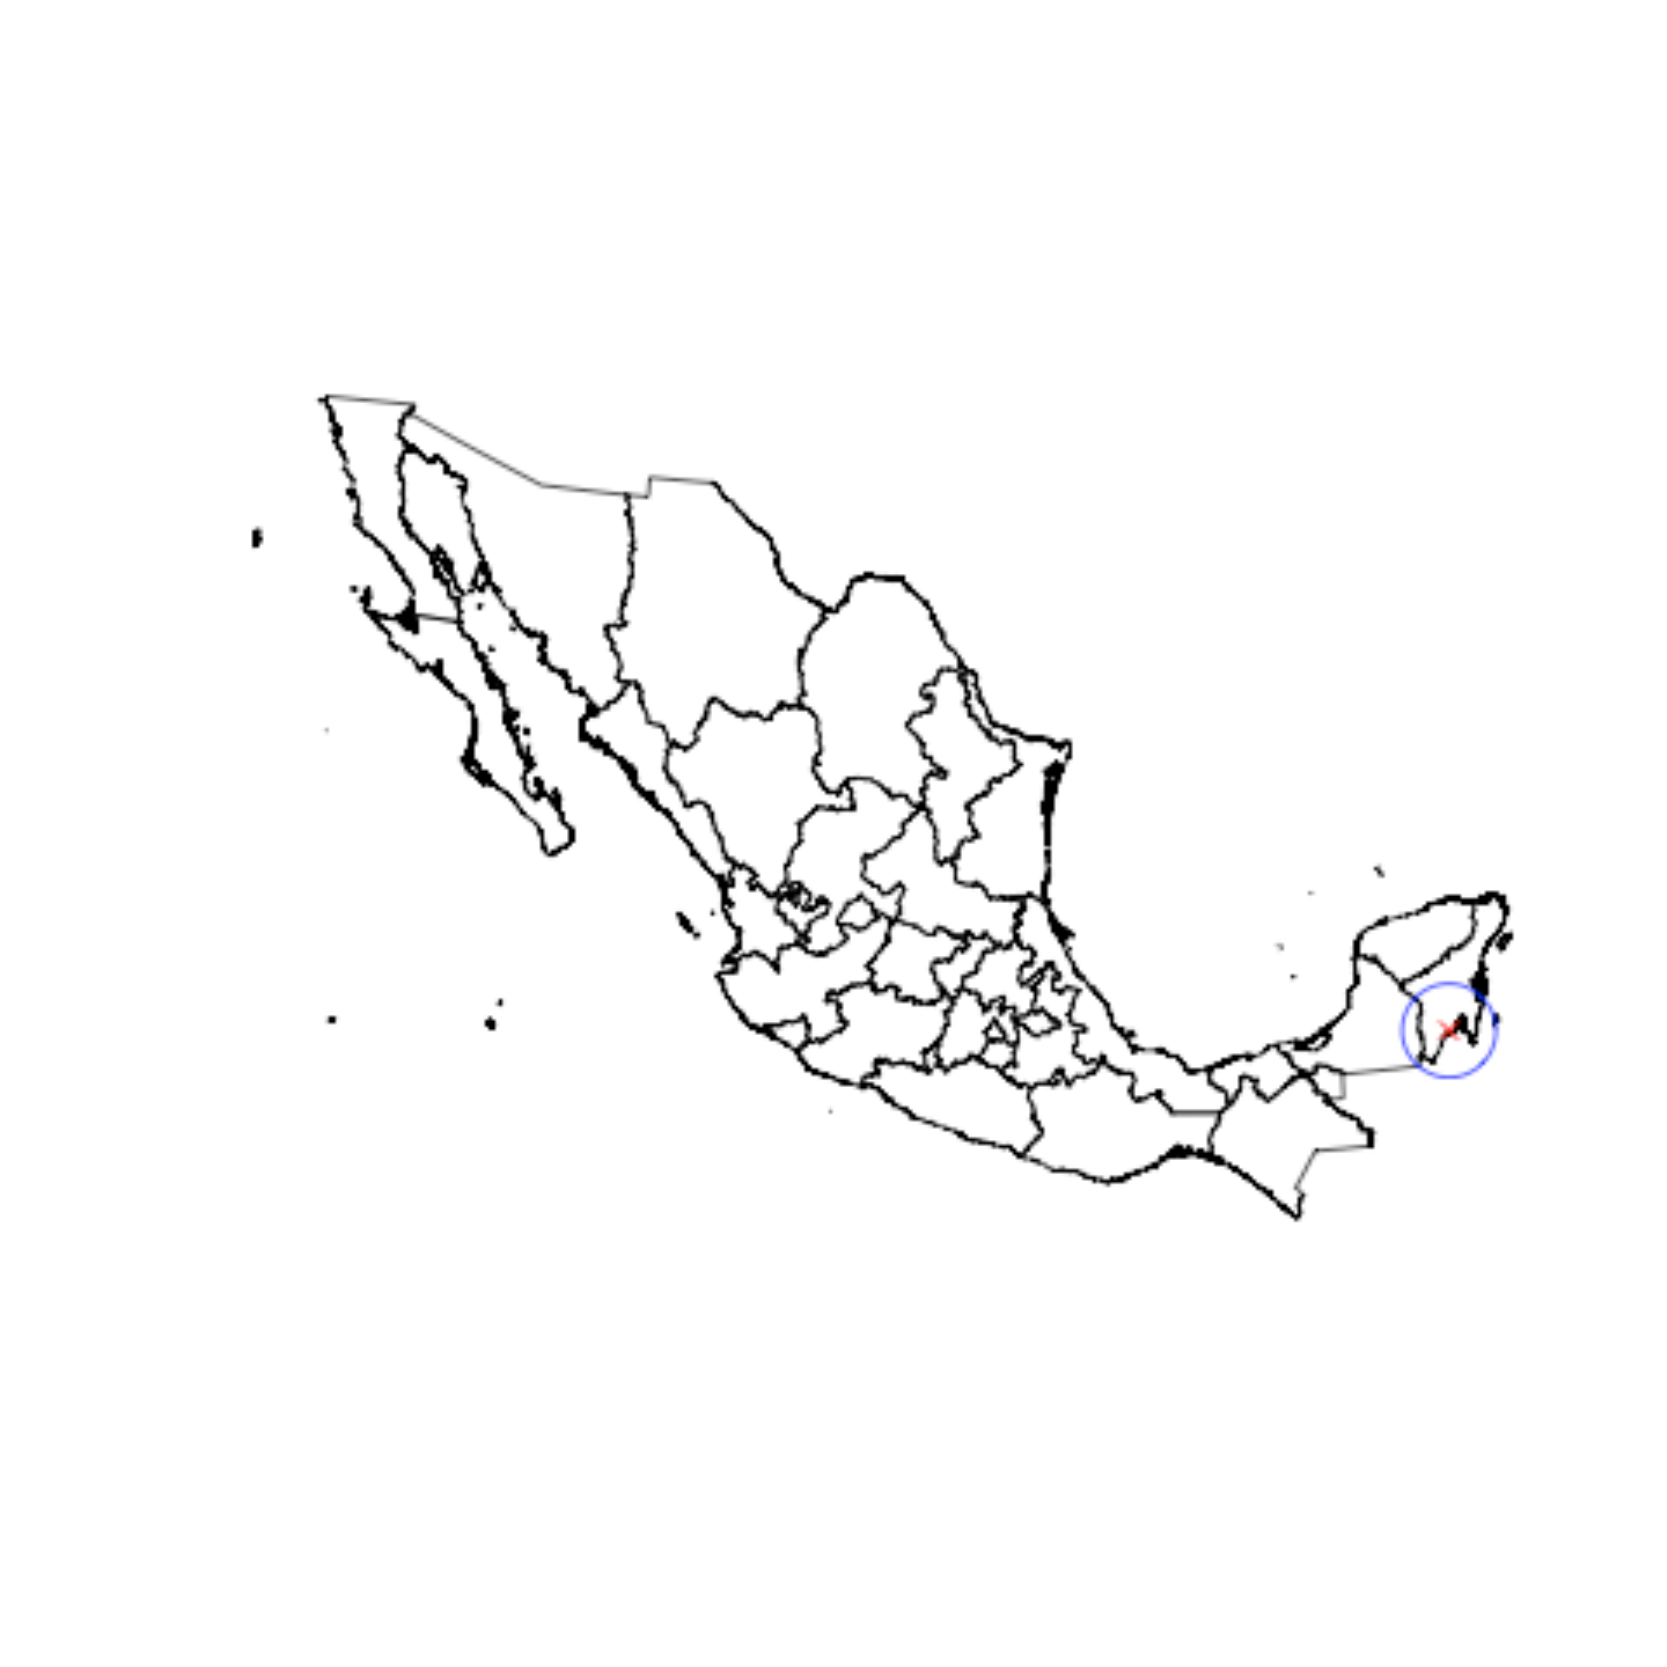}
      	     \caption{Location}
      	     \label{fig:sfig1d}
      	   \end{subfigure}   
         \begin{subfigure}{.5\textwidth}
           \centering
           \includegraphics[width=1\textwidth]{./2_Data/legend_landUse}
           \caption{Land use legend}
           \label{fig:legend}
         \end{subfigure}
      	   %%         --- .5\textwidth stands for 50% of text width
      	   \caption[NALCMS land-use classification of QuintanaRoo100 site, 2005 and 2010 at 250m resolution.]%<<-- Legend for the list of figures at the beginning of you thesis
      	   {NALCMS land-use classification of QuintanaRoo100 site, 2005 and 2010 at 250m resolution.}% legend displayed below the graph.
      	   \label{fig:landUseQuintanaRoo100}
      	 \end{figure}
		
   		\begin{center}
   			\footnotesize\addtolength{\tabcolsep}{-2pt}
   			% latex table generated in R 3.3.1 by xtable 1.8-2 package
% Sun Mar  5 16:01:40 2017
\begin{table}[ht]
\centering
\begingroup\tiny
\begin{tabular}{rrrrrrrrrrrrrrrrrrrrr}
  & \begin{sideways} Temperate or sub-polar needleleaf forest \end{sideways} & \begin{sideways} Sub-polar taiga needleleaf forest \end{sideways} & \begin{sideways} Tropical or sub-tropical broadleaf evergreen forest \end{sideways} & \begin{sideways} Tropical or sub-tropical broadleaf deciduous forest \end{sideways} & \begin{sideways} Temperate or sub-polar broadleaf deciduous forest \end{sideways} & \begin{sideways} Mixed Forest \end{sideways} & \begin{sideways} Tropical or sub-tropical shrubland \end{sideways} & \begin{sideways} Temperate or sub-polar shrubland \end{sideways} & \begin{sideways} Tropical or sub-tropical grassland \end{sideways} & \begin{sideways} Temperate or sub-polar grassland \end{sideways} & \begin{sideways} Sub-polar or polar shrubland-lichen-moss \end{sideways} & \begin{sideways} Sub-polar or polar grassland-lichen-moss \end{sideways} & \begin{sideways} Sub-polar or polar barren-lichen-moss \end{sideways} & \begin{sideways} Wetland \end{sideways} & \begin{sideways} Cropland \end{sideways} & \begin{sideways} Barren Lands \end{sideways} & \begin{sideways} Urban and Built-up \end{sideways} & \begin{sideways} Water \end{sideways} & \begin{sideways} Snow and Ice \end{sideways} & \begin{sideways} Total \end{sideways} \\ 
  \hline
Temperate or sub-polar needleleaf forest &    0 &    0 &    0 &    0 &    0 &    0 &    0 &    0 &    0 &    0 &    0 &    0 &    0 &    0 &    0 &    0 &    0 &    0 &    0 &    0 \\ 
  Sub-polar taiga needleleaf forest &    0 &    0 &    0 &    0 &    0 &    0 &    0 &    0 &    0 &    0 &    0 &    0 &    0 &    0 &    0 &    0 &    0 &    0 &    0 &    0 \\ 
  Tropical or sub-tropical broadleaf evergreen forest &    0 &    0 & 4286 &    0 &    0 &    0 &    0 &    0 &    0 &    0 &    0 &    0 &    0 &    0 &   90 &    0 &   10 &    0 &    0 & 4386 \\ 
  Tropical or sub-tropical broadleaf deciduous forest &    0 &    0 &    0 &    0 &    0 &    0 &    0 &    0 &    0 &    0 &    0 &    0 &    0 &    0 &    0 &    0 &    0 &    0 &    0 &    0 \\ 
  Temperate or sub-polar broadleaf deciduous forest &    0 &    0 &    0 &    0 &    0 &    0 &    0 &    0 &    0 &    0 &    0 &    0 &    0 &    0 &    0 &    0 &    0 &    0 &    0 &    0 \\ 
  Mixed Forest &    0 &    0 &    0 &    0 &    0 &    0 &    0 &    0 &    0 &    0 &    0 &    0 &    0 &    0 &    0 &    0 &    0 &    0 &    0 &    0 \\ 
   \hline
Tropical or sub-tropical shrubland &    0 &    0 &    0 &    0 &    0 &    0 &    0 &    0 &    0 &    0 &    0 &    0 &    0 &    0 &    0 &    0 &    0 &    0 &    0 &    0 \\ 
  Temperate or sub-polar shrubland &    0 &    0 &    0 &    0 &    0 &    0 &    0 &    0 &    0 &    0 &    0 &    0 &    0 &    0 &    0 &    0 &    0 &    0 &    0 &    0 \\ 
  Tropical or sub-tropical grassland &    0 &    0 &    0 &    0 &    0 &    0 &    0 &    0 &    0 &    0 &    0 &    0 &    0 &    0 &    0 &    0 &    0 &    0 &    0 &    0 \\ 
  Temperate or sub-polar grassland &    0 &    0 &    0 &    0 &    0 &    0 &    0 &    0 &    0 &    0 &    0 &    0 &    0 &    0 &    0 &    0 &    0 &    0 &    0 &    0 \\ 
  Sub-polar or polar shrubland-lichen-moss &    0 &    0 &    0 &    0 &    0 &    0 &    0 &    0 &    0 &    0 &    0 &    0 &    0 &    0 &    0 &    0 &    0 &    0 &    0 &    0 \\ 
  Sub-polar or polar grassland-lichen-moss &    0 &    0 &    0 &    0 &    0 &    0 &    0 &    0 &    0 &    0 &    0 &    0 &    0 &    0 &    0 &    0 &    0 &    0 &    0 &    0 \\ 
  Sub-polar or polar barren-lichen-moss &    0 &    0 &    0 &    0 &    0 &    0 &    0 &    0 &    0 &    0 &    0 &    0 &    0 &    0 &    0 &    0 &    0 &    0 &    0 &    0 \\ 
  Wetland &    0 &    0 &    0 &    0 &    0 &    0 &    0 &    0 &    0 &    0 &    0 &    0 &    0 &  674 &    0 &    0 &    0 &    0 &    0 &  674 \\ 
  Cropland &    0 &    0 &    0 &    0 &    0 &    0 &    0 &    0 &    0 &    0 &    0 &    0 &    0 &    0 & 2361 &    0 &   28 &    2 &    0 & 2391 \\ 
  Barren Lands &    0 &    0 &    0 &    0 &    0 &    0 &    0 &    0 &    0 &    0 &    0 &    0 &    0 &    4 &    0 &   20 &    0 &    1 &    0 &   25 \\ 
  Urban and Built-up &    0 &    0 &    0 &    0 &    0 &    0 &    0 &    0 &    0 &    0 &    0 &    0 &    0 &    0 &    0 &    0 &  313 &    0 &    0 &  313 \\ 
  Water &    0 &    0 &    0 &    0 &    0 &    0 &    0 &    0 &    0 &    0 &    0 &    0 &    0 &    2 &    0 &    0 &    0 &  295 &    0 &  297 \\ 
  Snow and Ice &    0 &    0 &    0 &    0 &    0 &    0 &    0 &    0 &    0 &    0 &    0 &    0 &    0 &    0 &    0 &    0 &    0 &    0 &    0 &    0 \\ 
   \hline
Total &    0 &    0 & 4286 &    0 &    0 &    0 &    0 &    0 &    0 &    0 &    0 &    0 &    0 &  680 & 2451 &   20 &  351 &  298 &    0 & 8086 \\ 
   \hline
\end{tabular}
\endgroup
\caption[NALCMS land-use distribution for site QuintanaRoo100, 2005 and 2010.]{NALCMS land-use distribution for site QuintanaRoo100, 2005 and 2010.} 
\end{table}

   			\label{tab:landUseSonora}
   		\end{center}
		
   		\begin{figure}[H]%--- Picture 'H'ere, 'B'ottom or 'T'op; '!' Try to
   		                    %impose your will to LaTeX
   		  \centering
   		  \includegraphics[width=.5\textwidth]{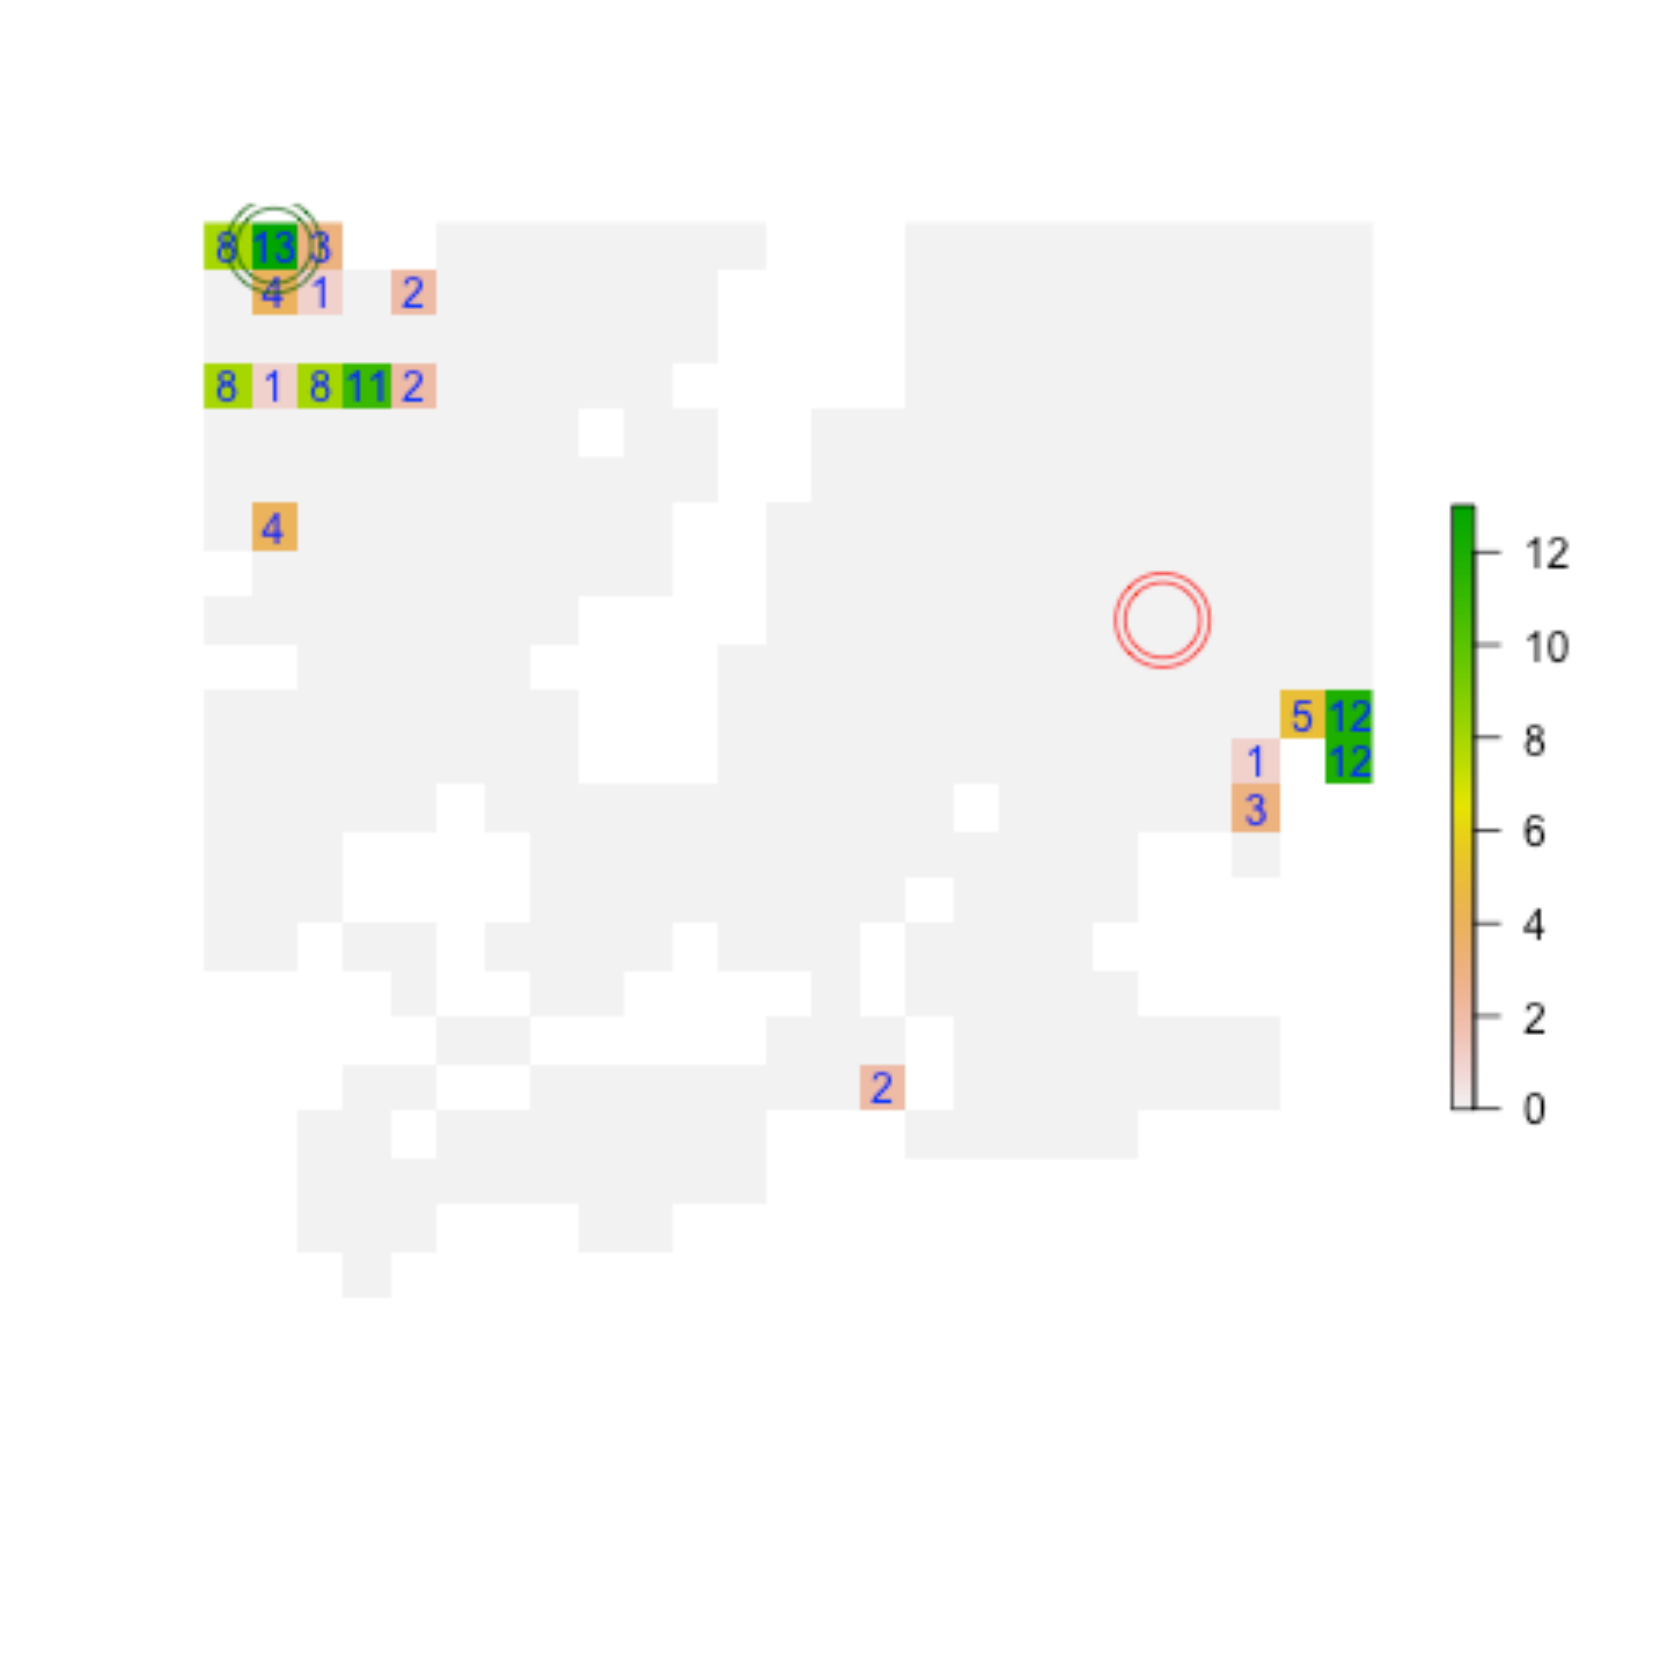} %<< no file extension
   		  %%         --- .5\textwidth stands for 50% of text width
   		  \caption[Deforestation in QuintanaRoo100 site at 1km resolution]%<<-- Legend for the list of figures at the beginning of you thesis
   		  {Deforestation in QuintanaRoo100 site at 1km resolution: number of 250m pixels deforested out of 16}% legend displayed below the graph.
   		  \label{fig:defoQuintanaRoo100}
   		\end{figure}
		
   		 \begin{figure}[H]
   	      \begin{subfigure}{.5\textwidth}
   	        \centering
   	    	\includegraphics[width=1\textwidth]{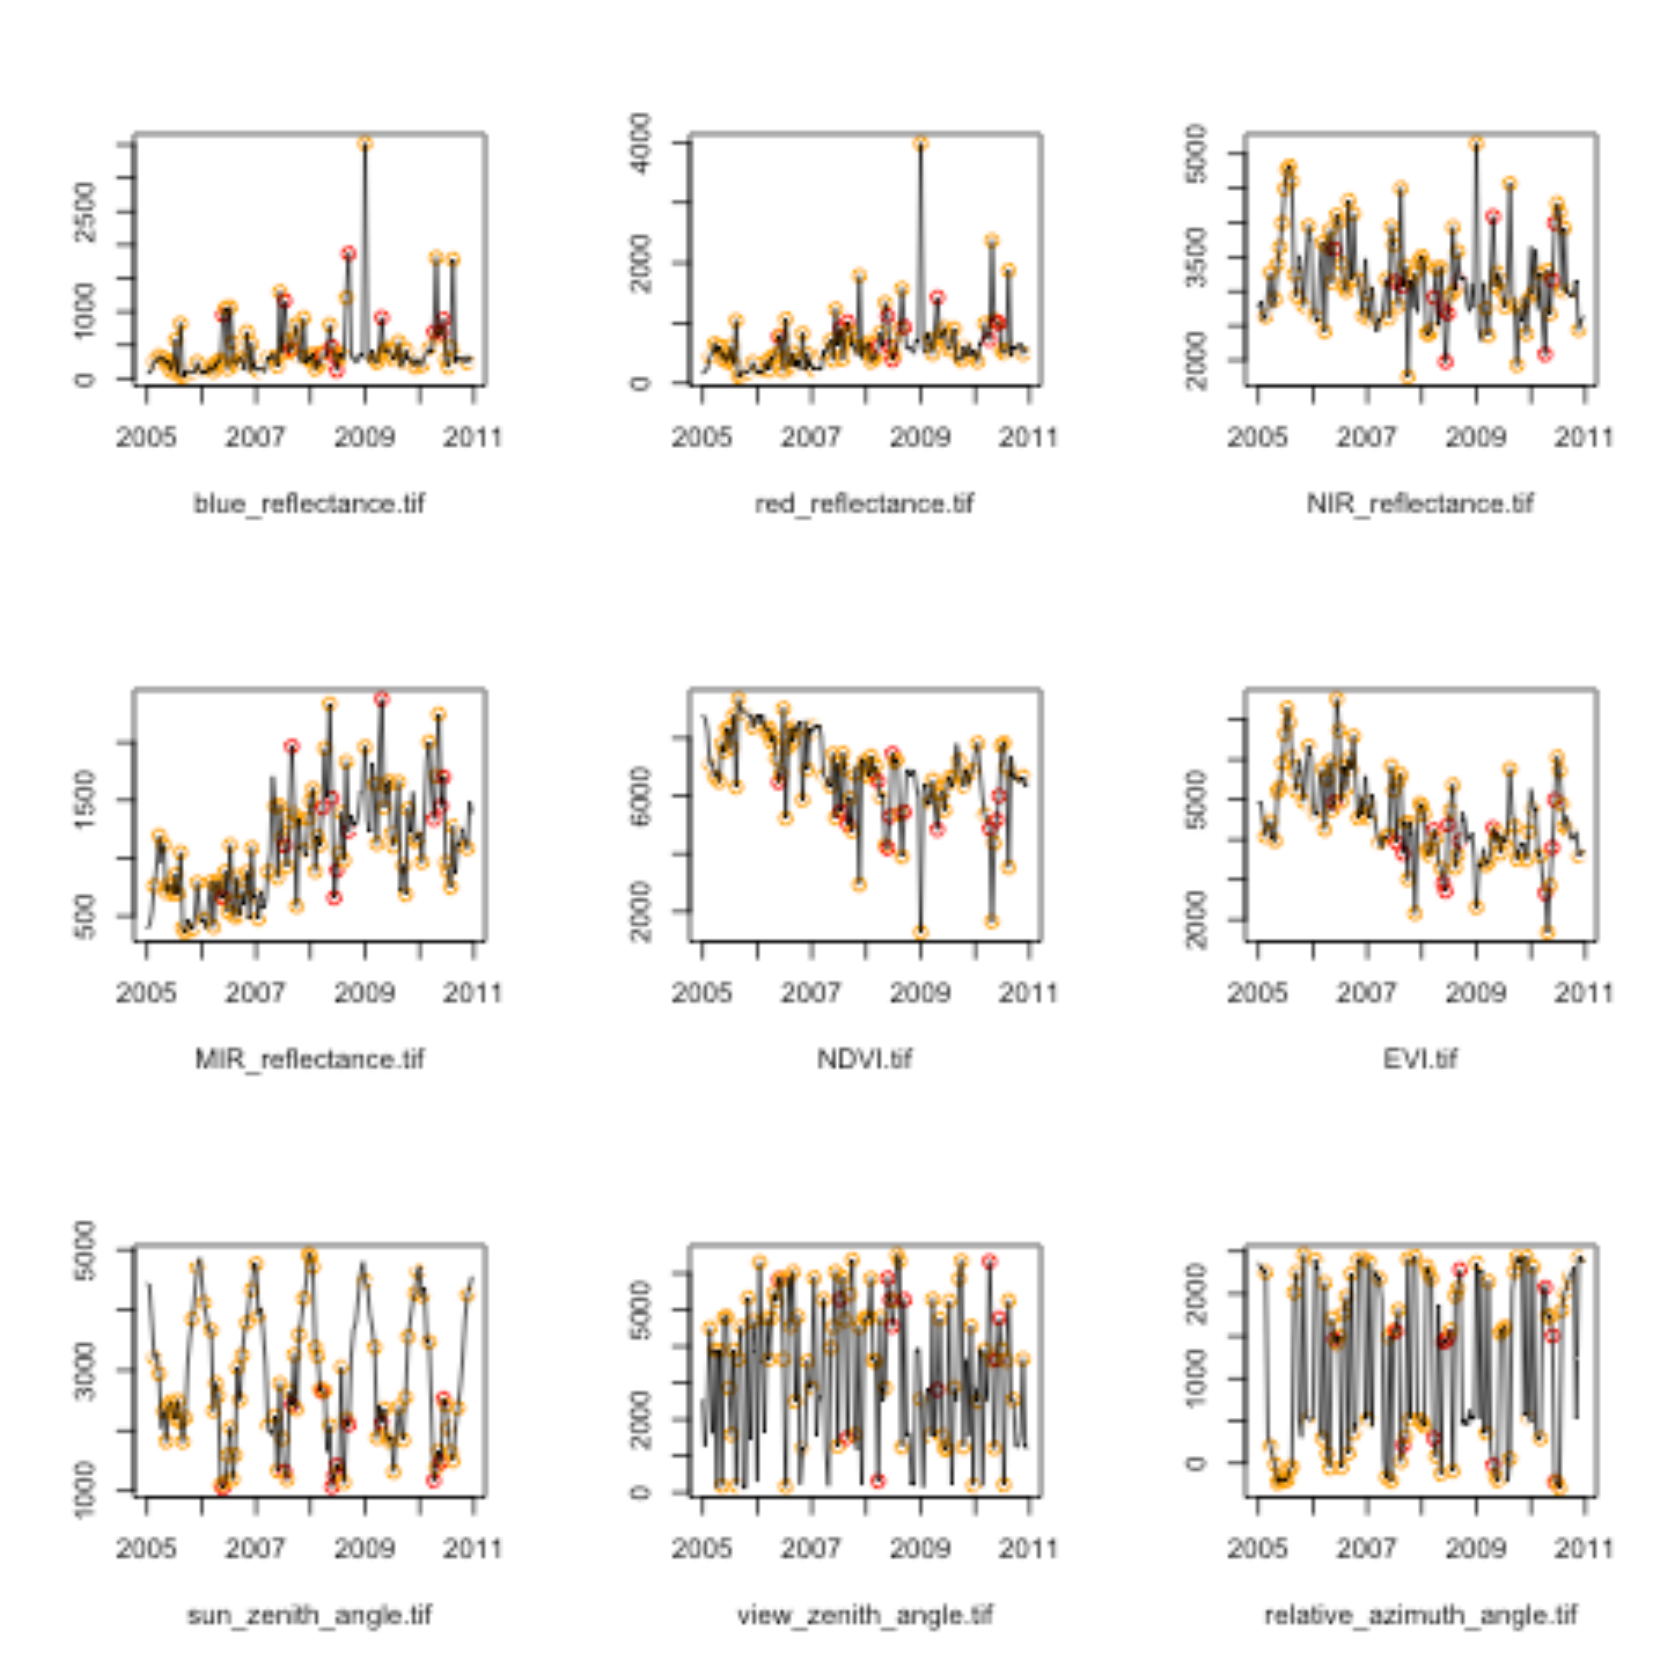} 
   	        \caption{deforested pixel}
   	        \label{fig:defo_pix}
   	      \end{subfigure}%
   	      \begin{subfigure}{.5\textwidth}
   	        \centering
   	        \includegraphics[width=1\textwidth]{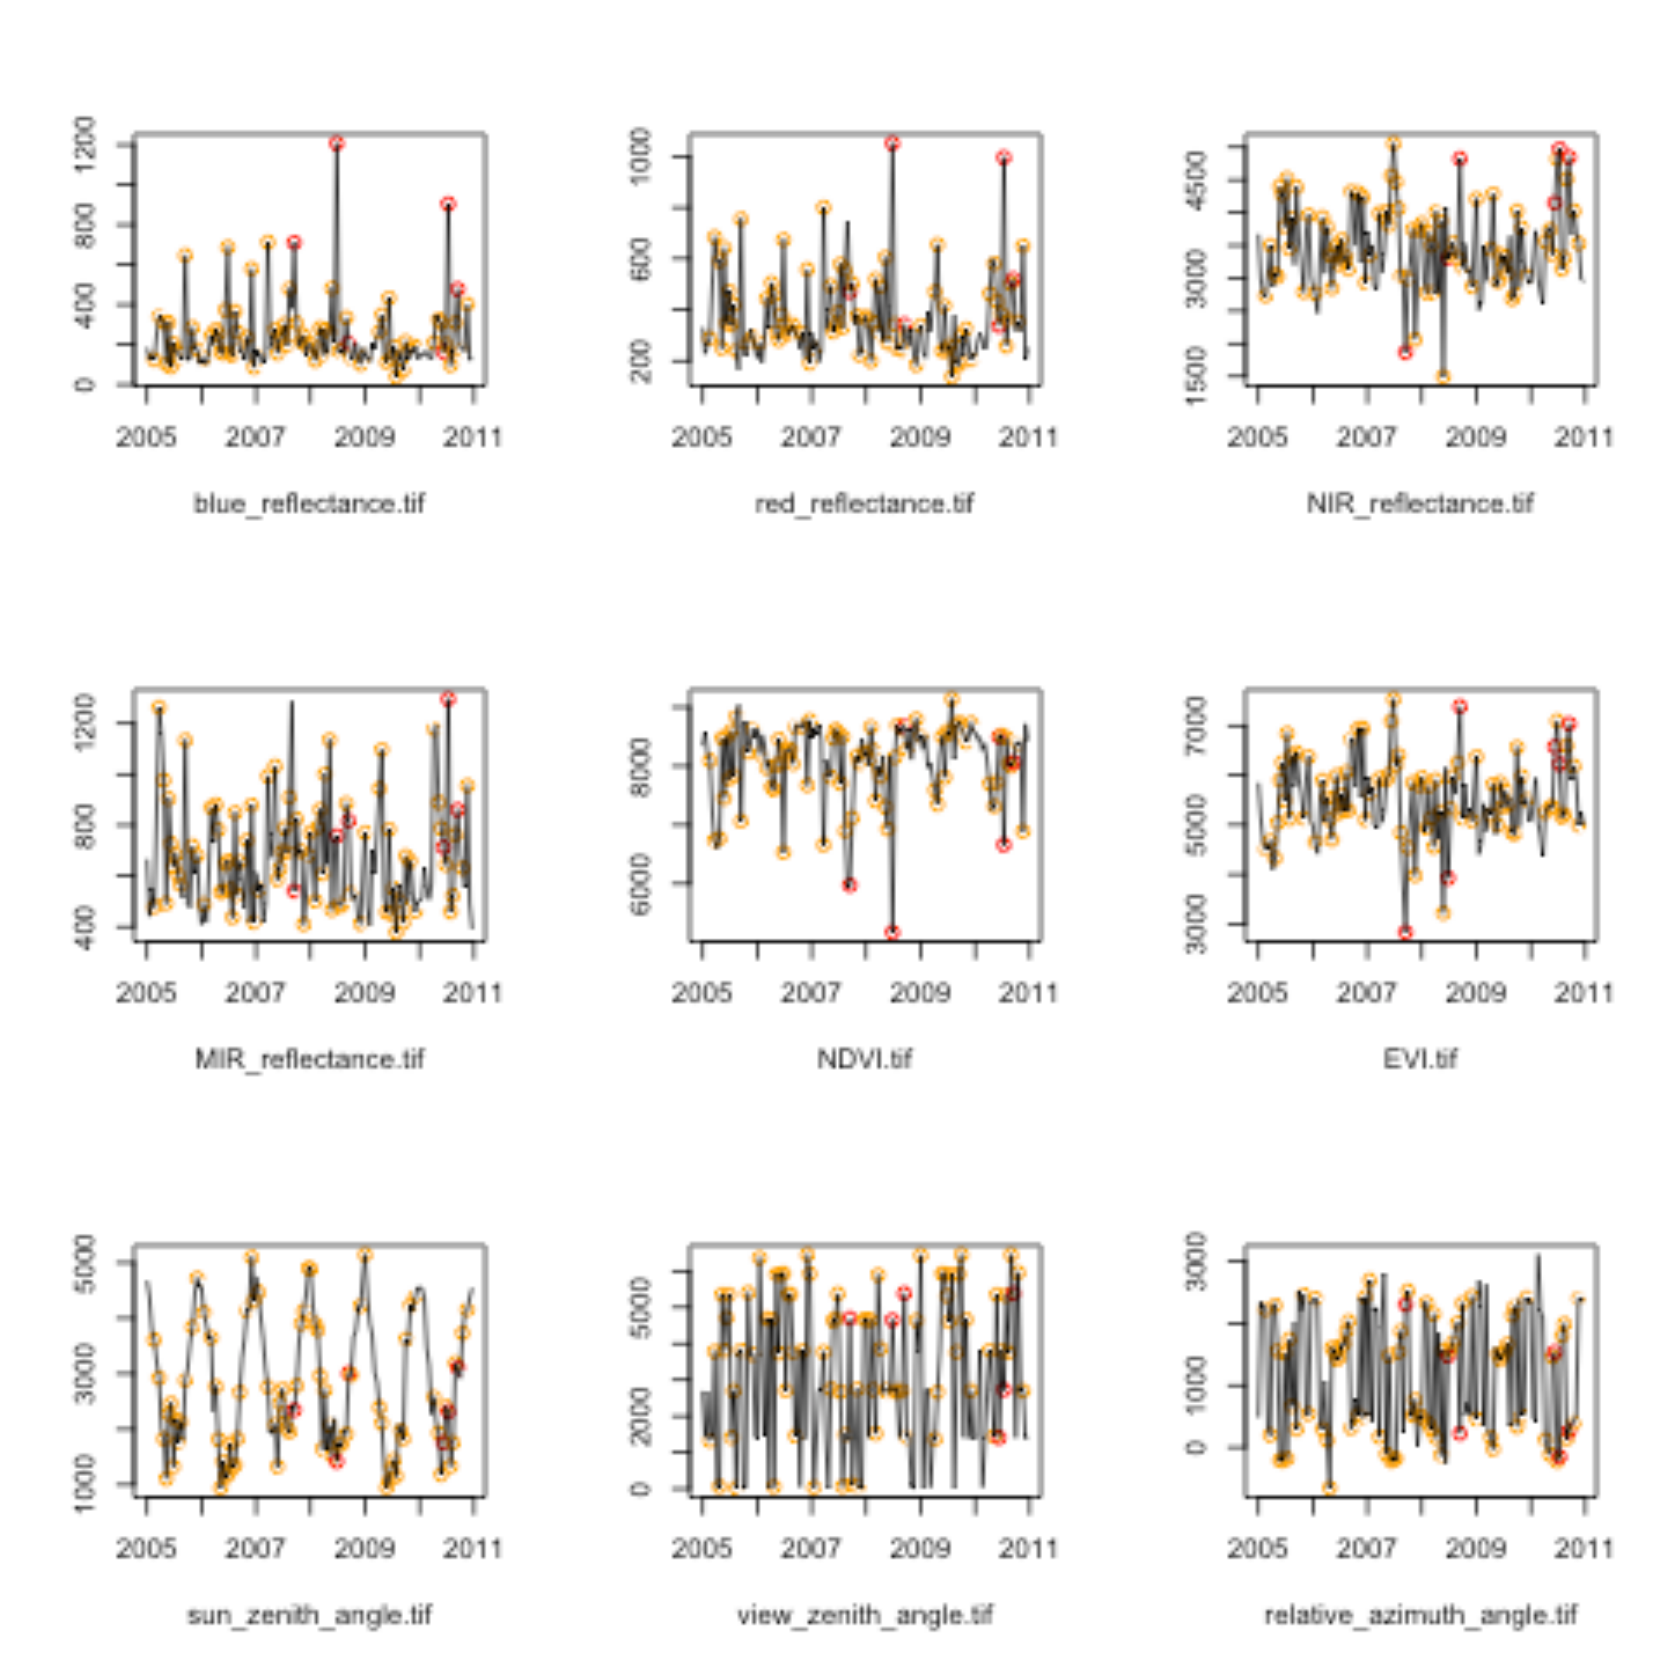}
   	        \caption{non-deforested pixel}
   	        \label{fig:non_defo_pix}
   	      \end{subfigure}
   	      %%         --- .5\textwidth stands for 50% of text width
   	      \caption[Reflectance, vegetation indices and sun-sensor geometry time series for deforested and non-deforested pixel in Yucatan 180 site.]%<<-- Legend for the list of figures at the beginning of you thesis
   	      {Reflectance, vegetation indices and sun-sensor geometry time series for deforested and non-deforested pixel in QuintanaRoo100 site, identified in figure \ref{fig:defoQuintanaRoo100} with green and red circles respectively. Orange marked points are \emph{marginal data} and red marked points are \emph{cloudy} or \emph{not processed}}% legend displayed below the graph.
   	      \label{fig:timeSeries}
   	    \end{figure}
		
		\subsubsection{Michoacan98}
		
      	 \begin{figure}[H]  %--- Picture 'H'ere, 'B'ottom or 'T'op; '!' Try to
      	                     %impose your will to LaTeX
      	  % \centering 
  
      	   \begin{subfigure}{.5\textwidth}
      	     \centering
      	 	\includegraphics[width=0.7\textwidth]{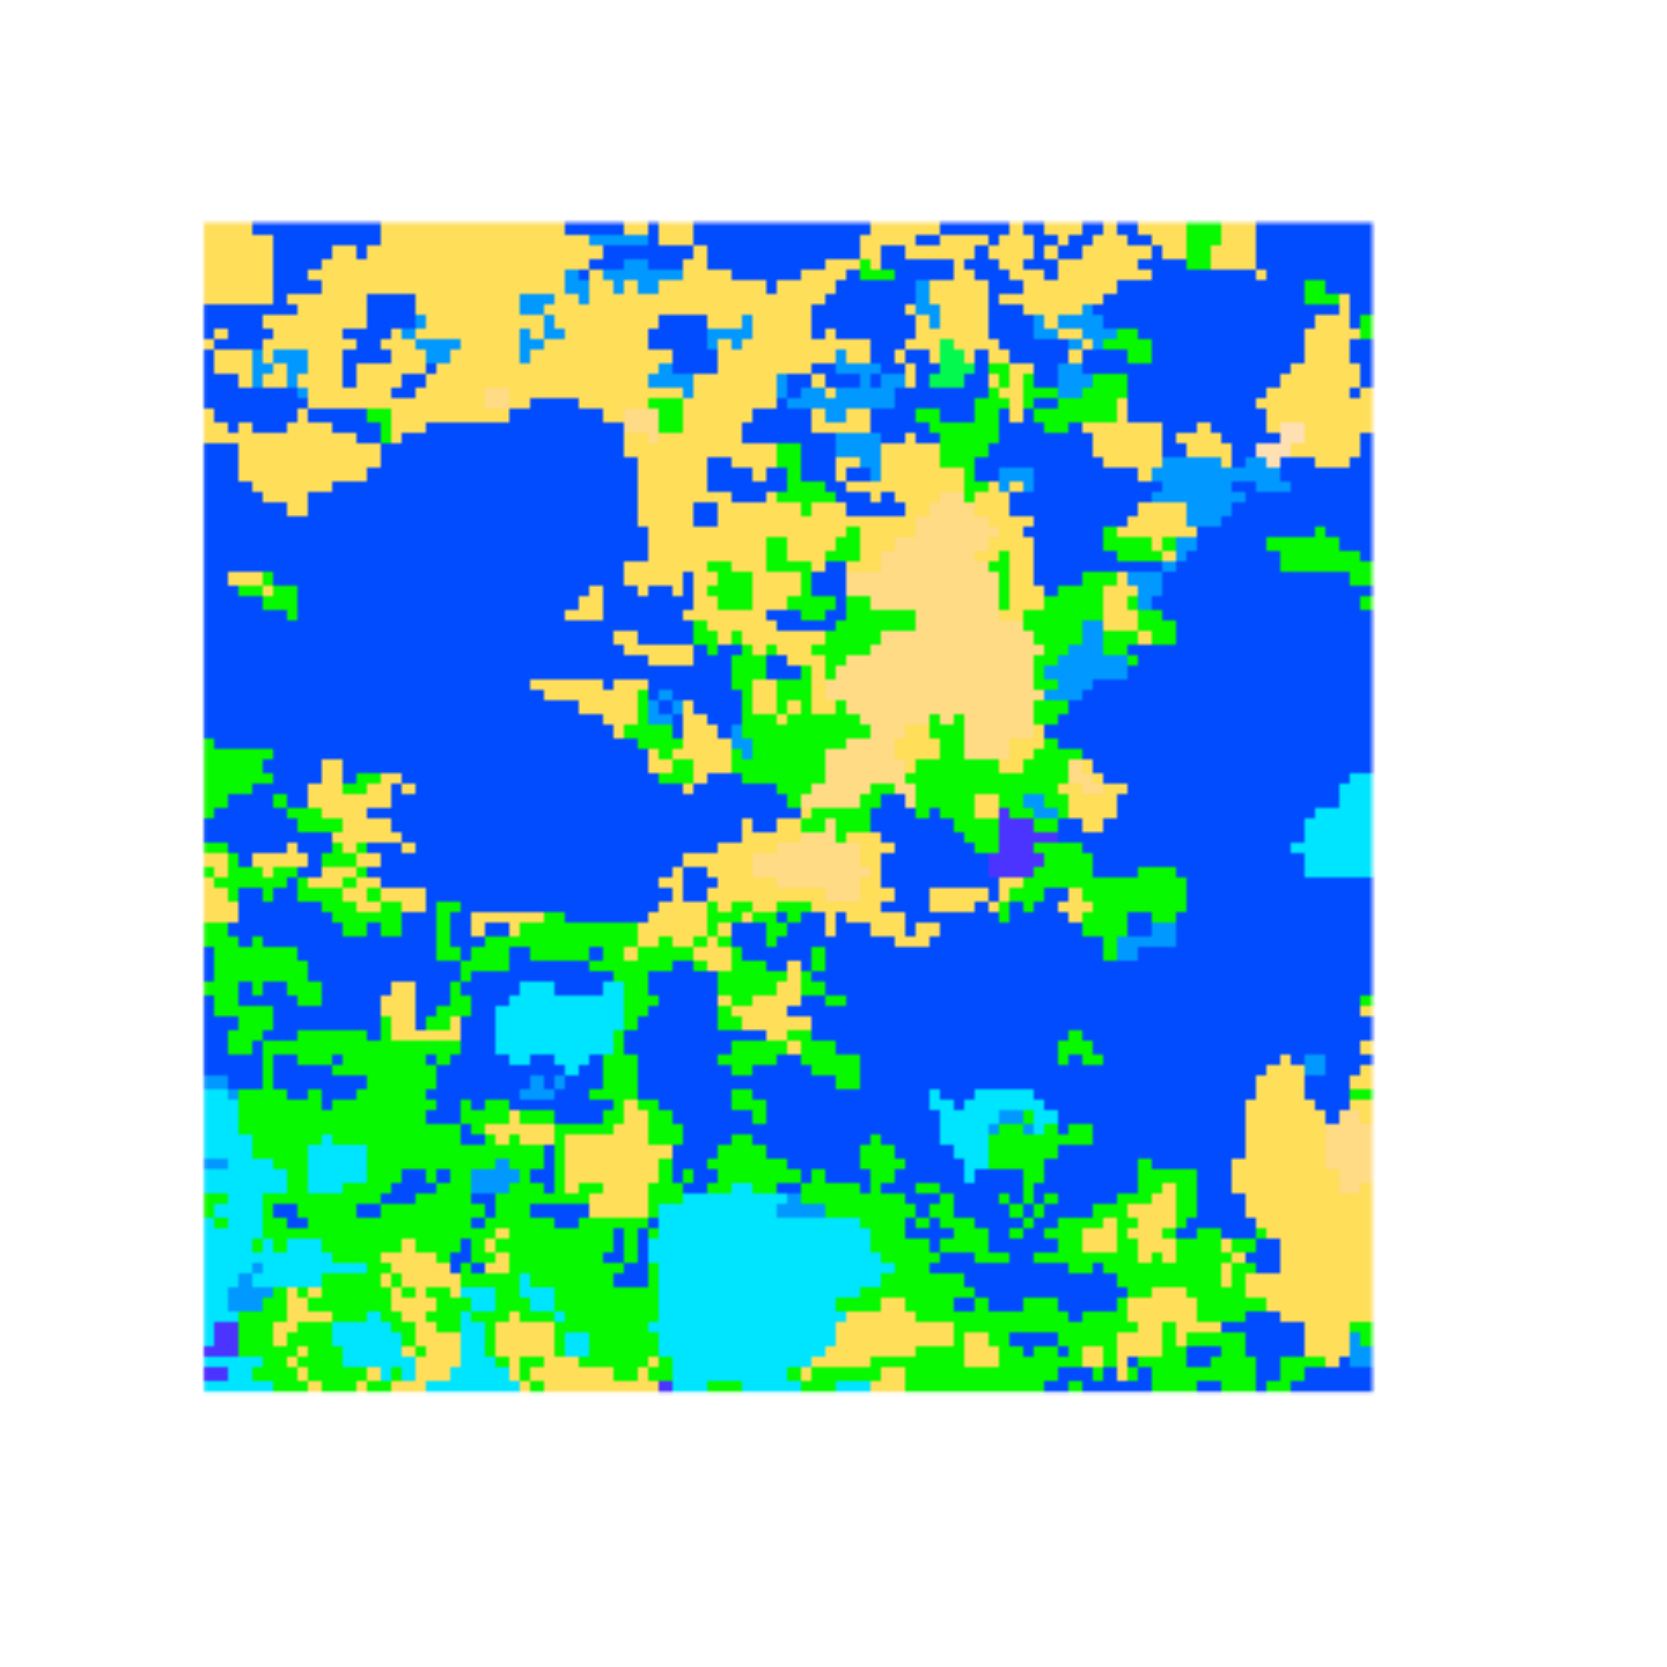} 
      	     \caption{Land-use 2005}
      	     \label{fig:sfig1a}
      	   \end{subfigure}%
      	   \begin{subfigure}{.5\textwidth}
      	     \centering
      	     \includegraphics[width=0.7\textwidth]{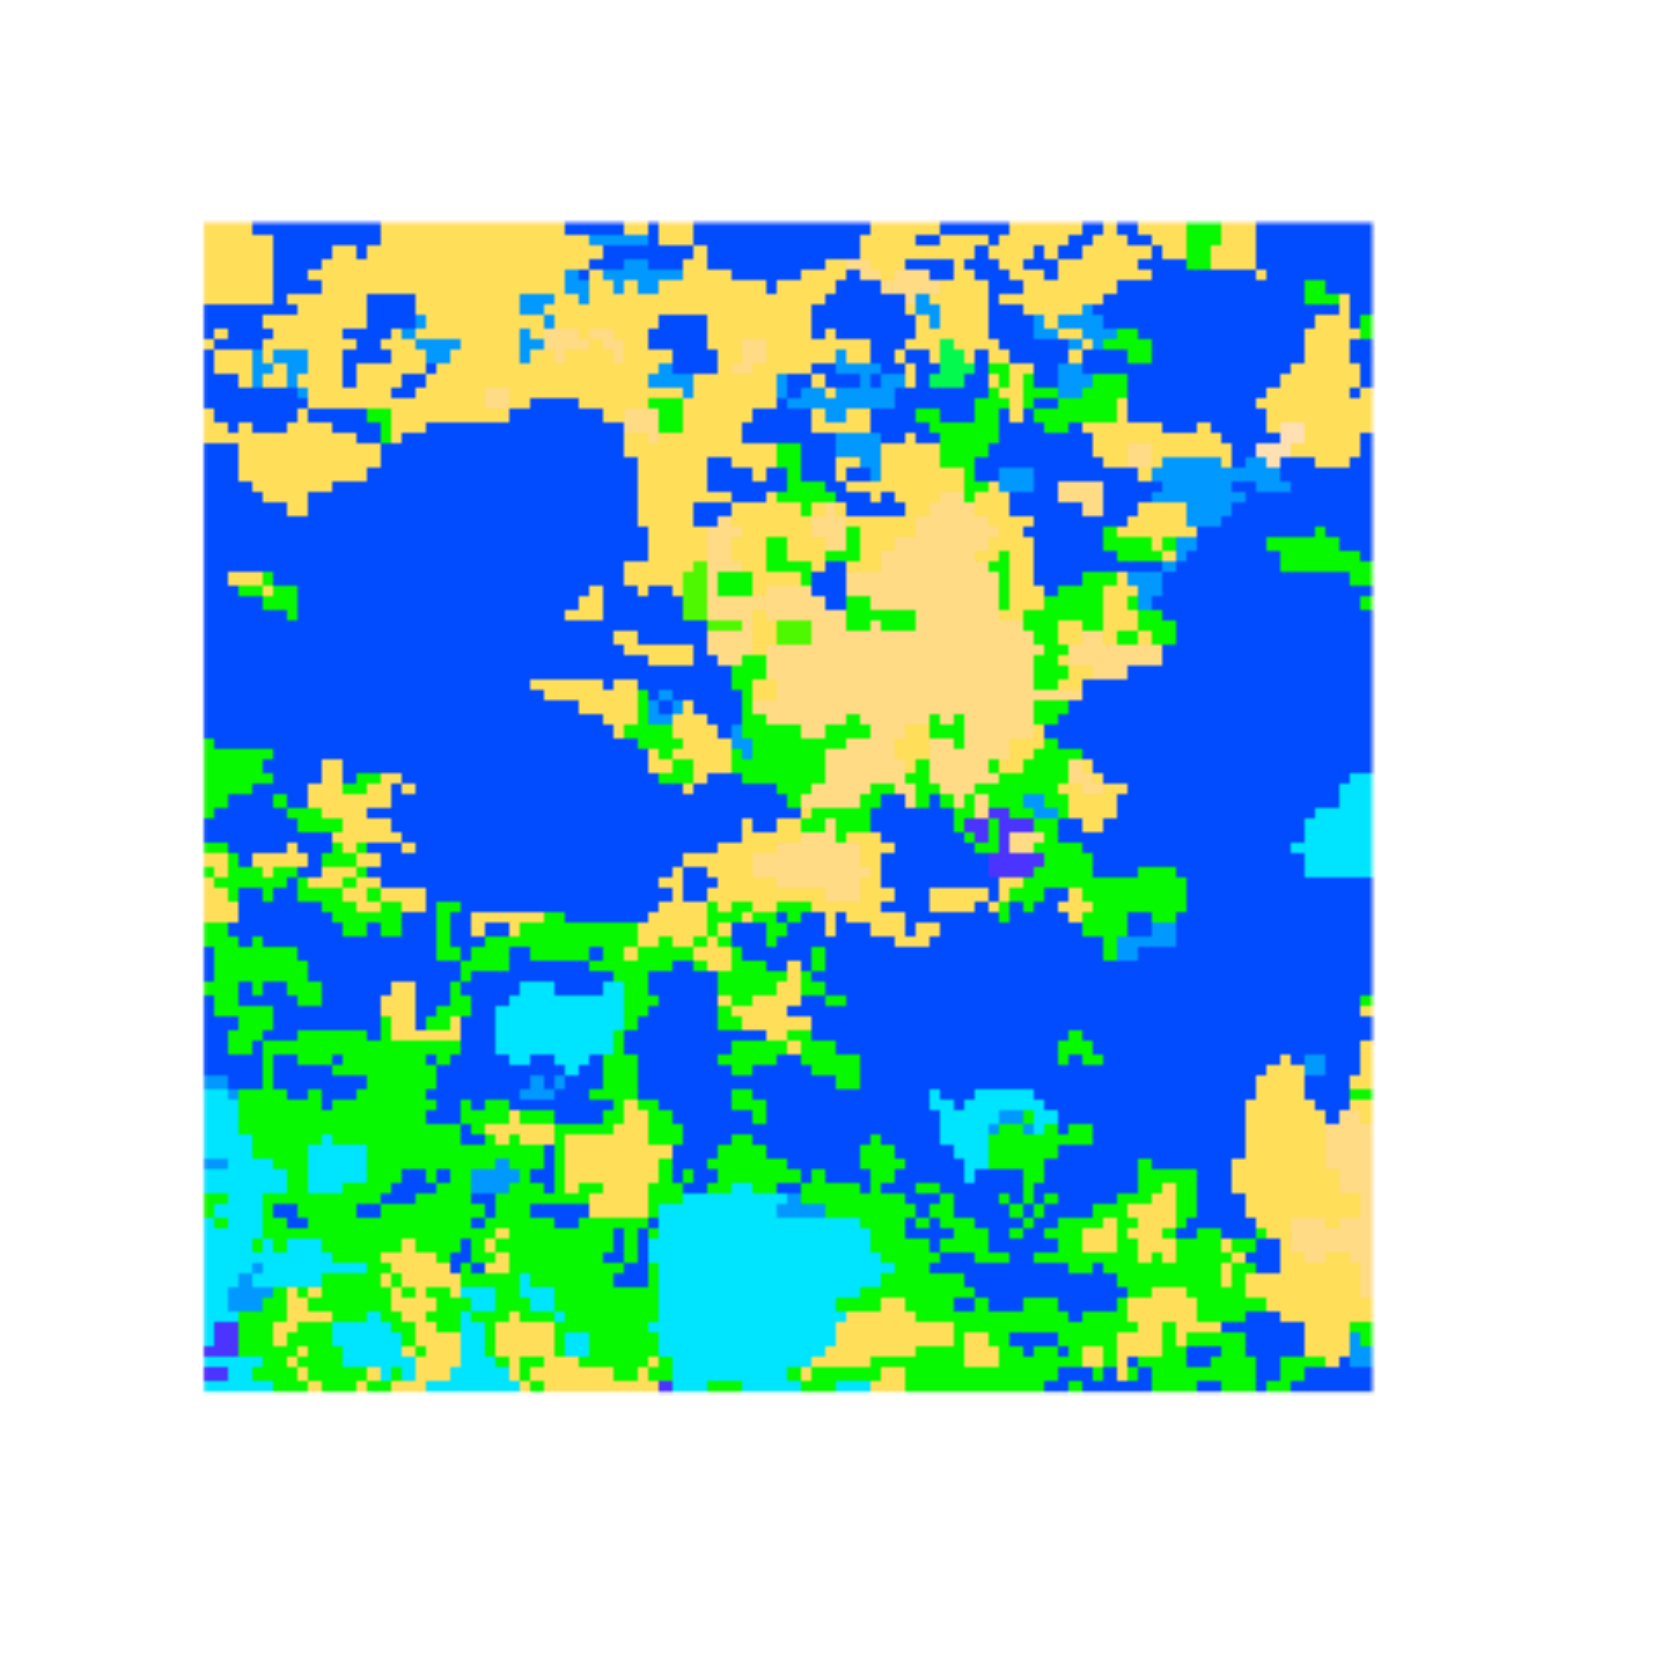}
      	     \caption{Land-use 2010}
      	     \label{fig:sfig1b}
      	   \end{subfigure}
      	   \begin{subfigure}{.4\textwidth}
      	     \centering
      	     \includegraphics[width=0.9\textwidth]{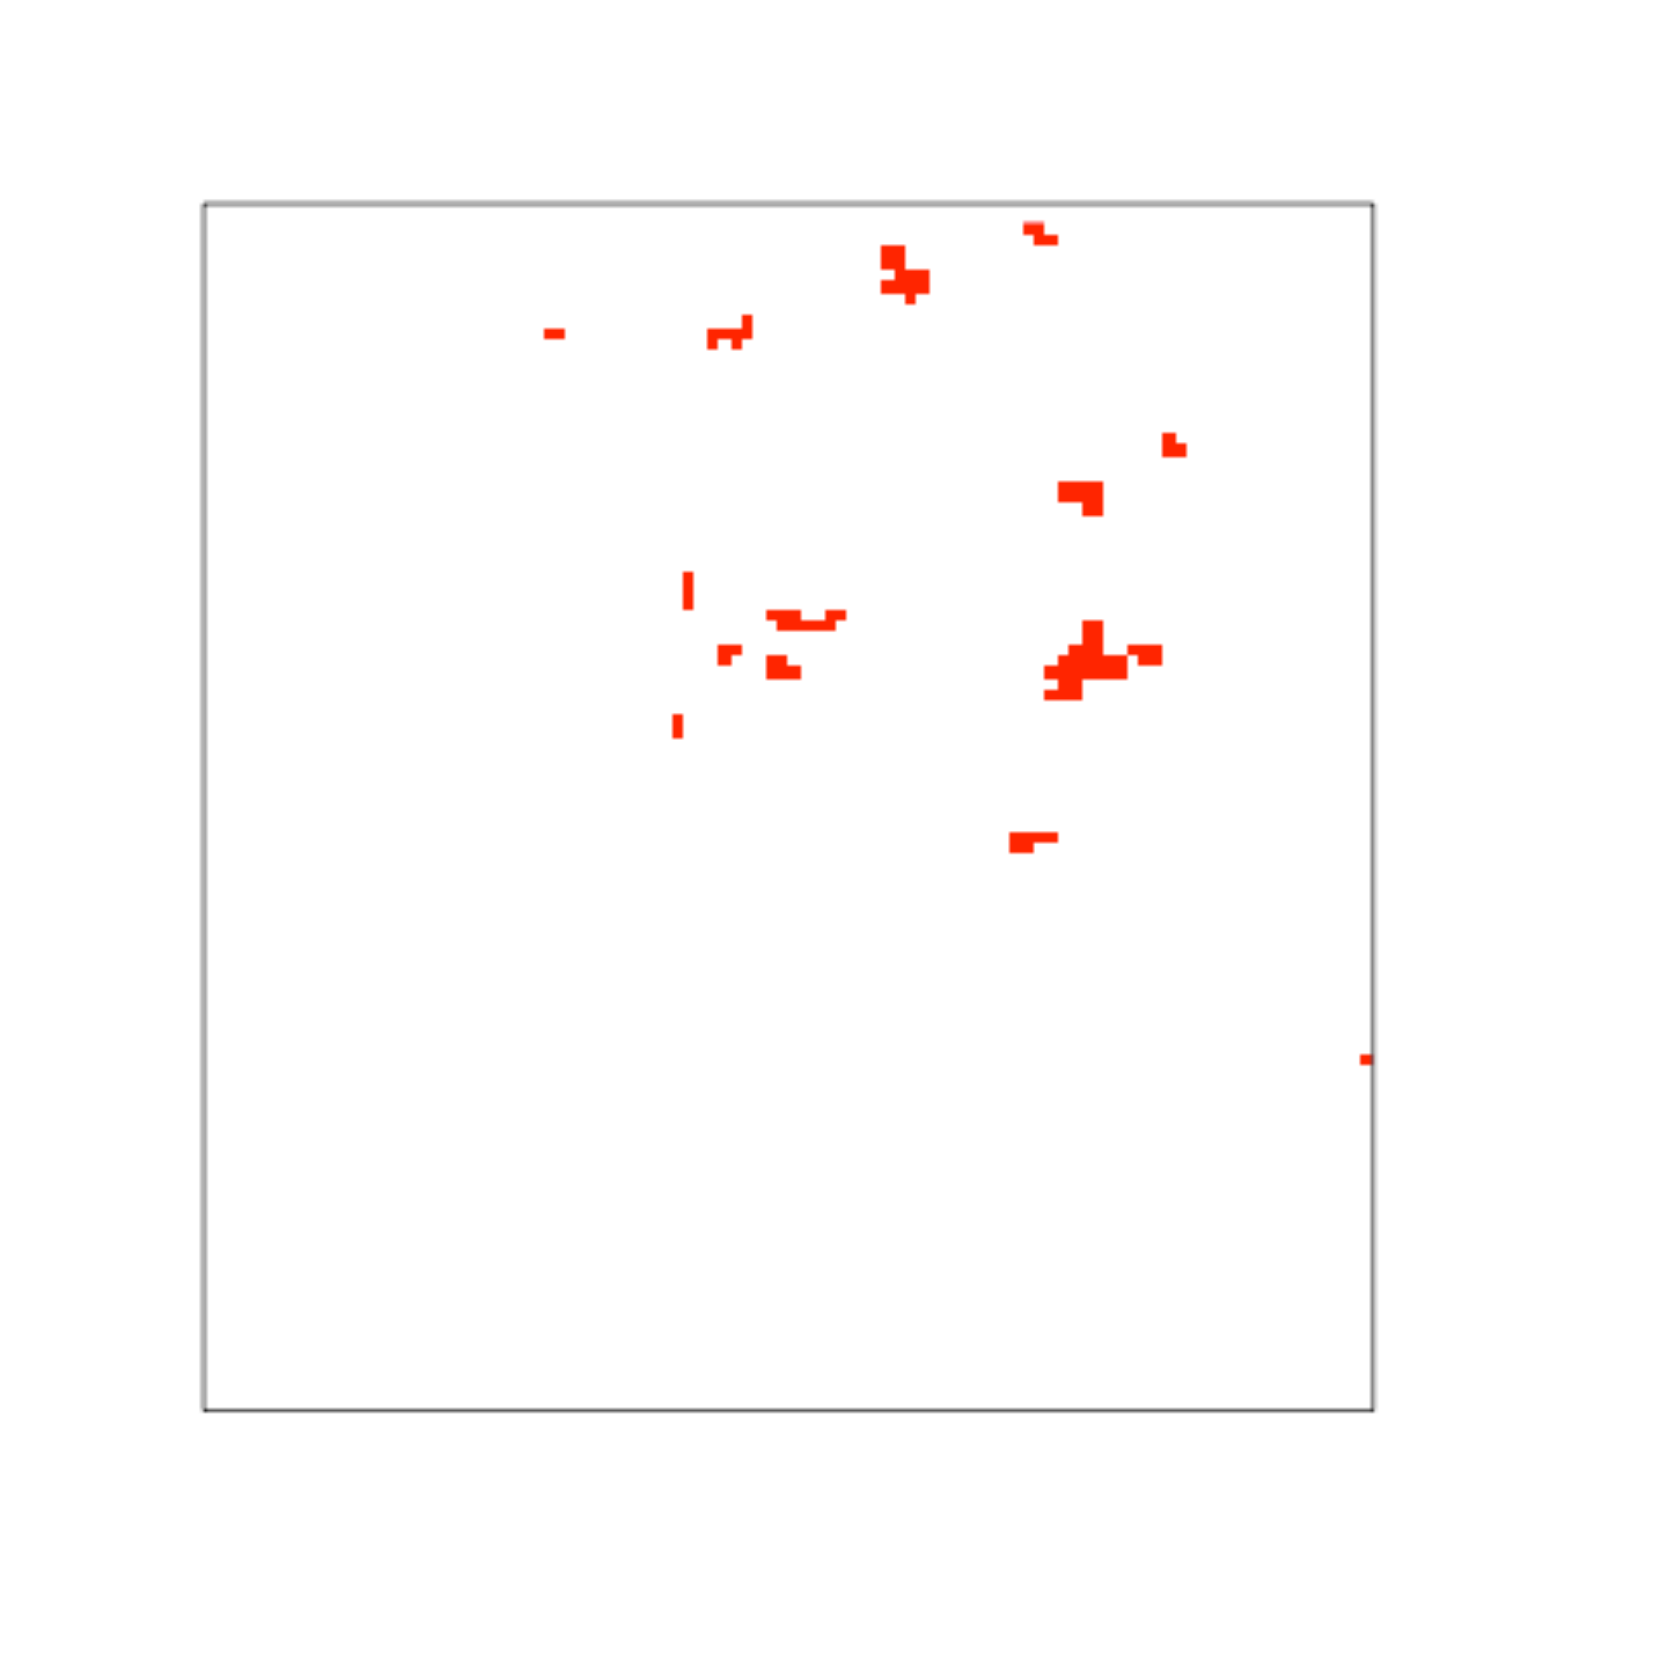}
      	     \caption{Deforestation 2005-2010}
      	     \label{fig:sfig1c}
      	   \end{subfigure}
      	   \begin{subfigure}{.4\textwidth}
      	     \centering
      	     \includegraphics[width=0.9\textwidth]{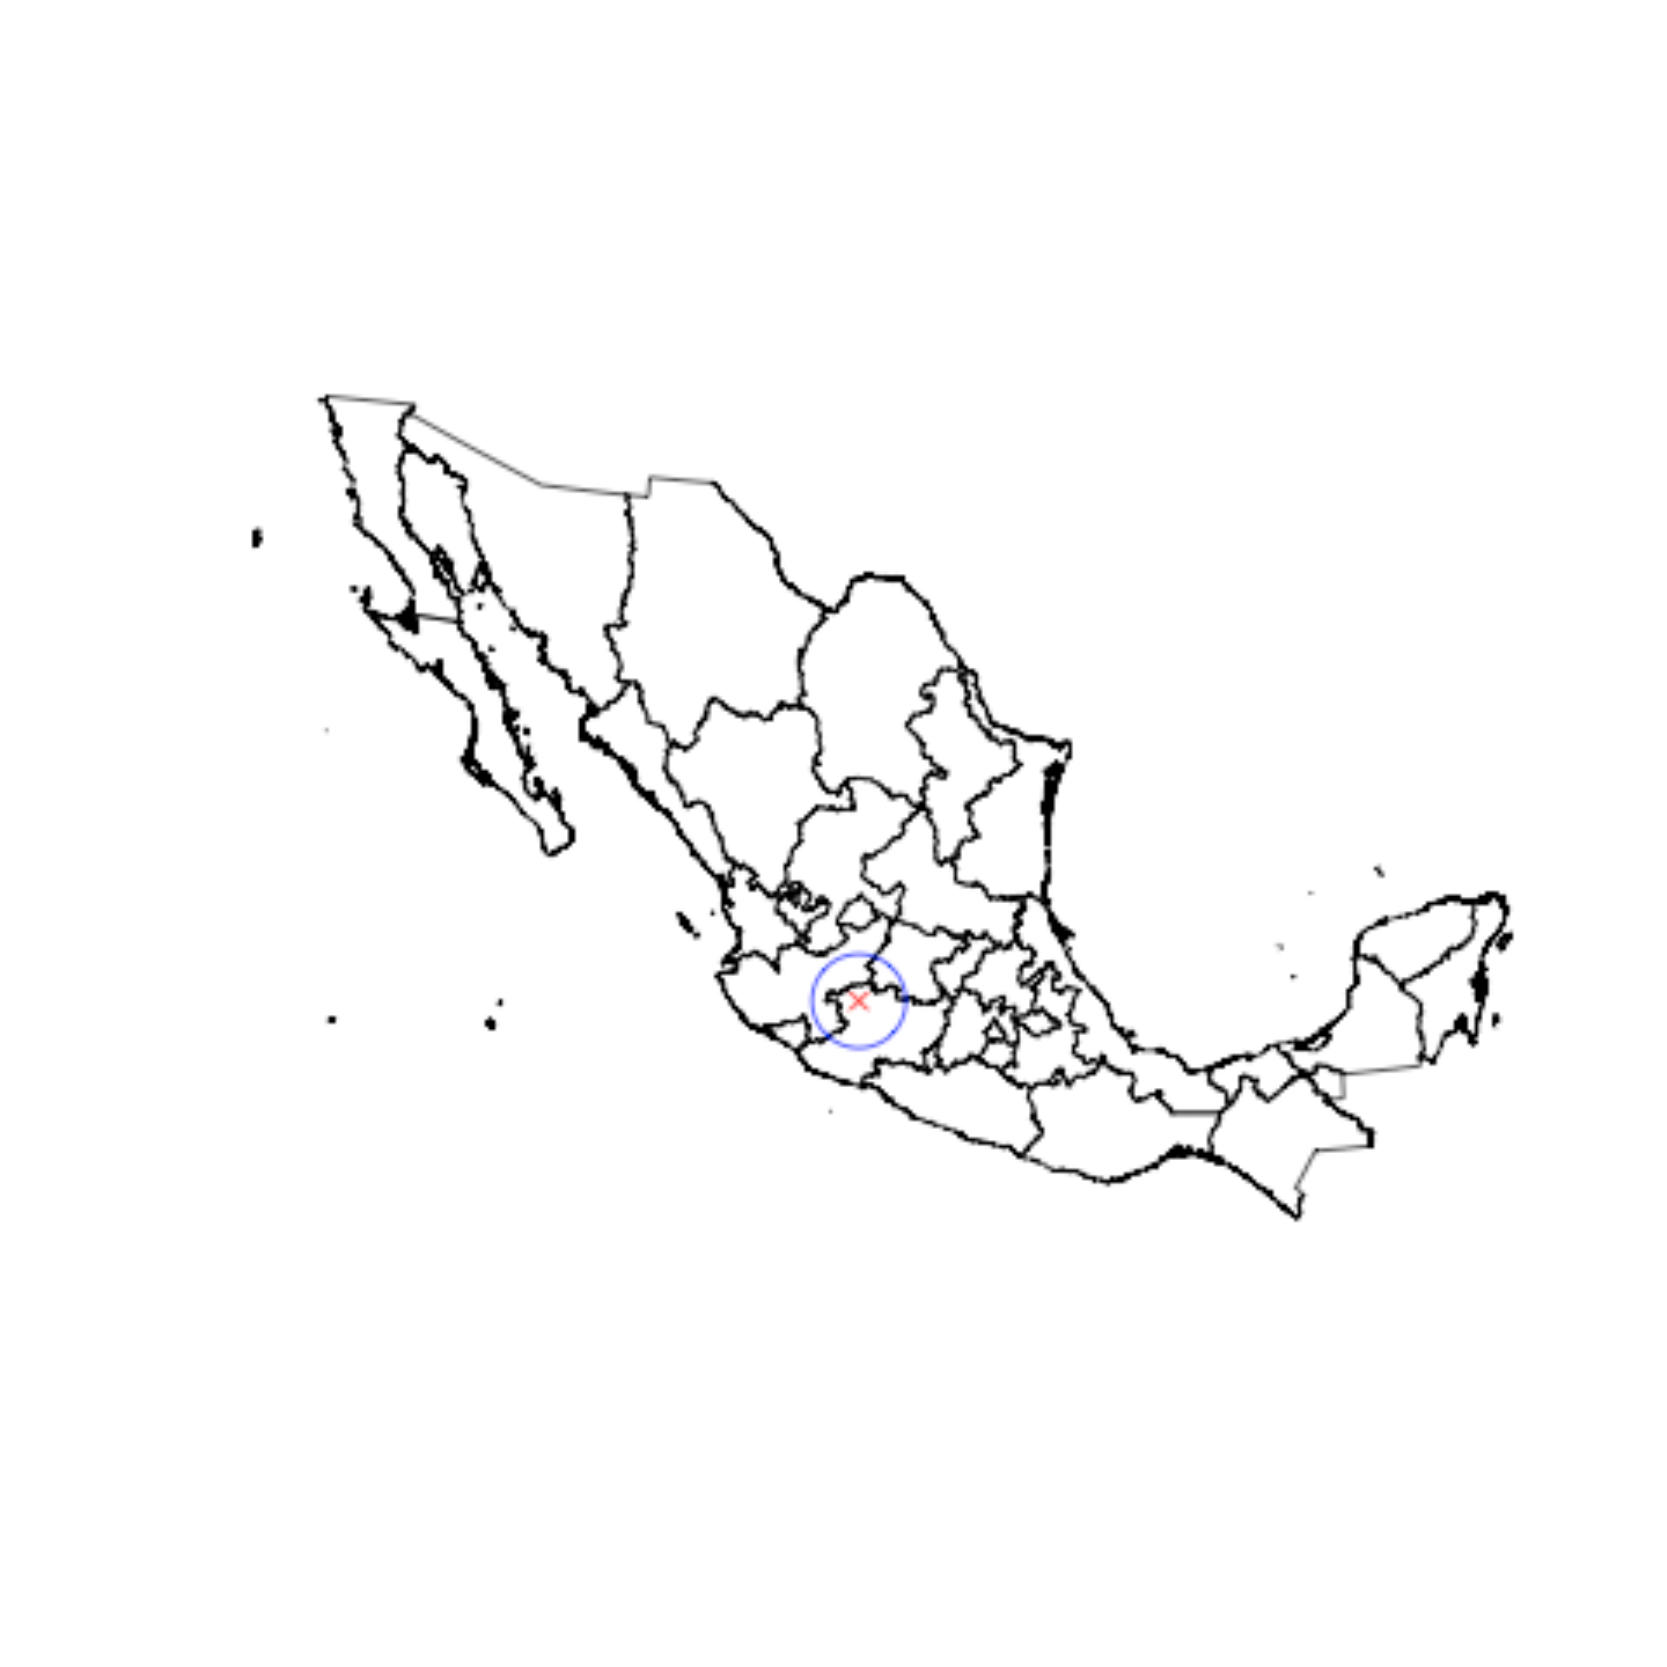}
      	     \caption{Location}
      	     \label{fig:sfig1d}
      	   \end{subfigure}   
         \begin{subfigure}{.5\textwidth}
           \centering
           \includegraphics[width=1\textwidth]{./2_Data/legend_landUse}
           \caption{Land use legend}
           \label{fig:legend}
         \end{subfigure}
      	   %%         --- .5\textwidth stands for 50% of text width
      	   \caption[NALCMS land-use classification of Michoacan98 site, 2005 and 2010 at 250m resolution.]%<<-- Legend for the list of figures at the beginning of you thesis
      	   {NALCMS land-use classification of Michoacan98 site, 2005 and 2010 at 250m resolution.}% legend displayed below the graph.
      	   \label{fig:landUseMichoacan98}
      	 \end{figure}
		
   		\begin{center}
   			\footnotesize\addtolength{\tabcolsep}{-2pt}
   			% latex table generated in R 3.3.1 by xtable 1.8-2 package
% Sun Mar  5 16:02:10 2017
\begin{table}[ht]
\centering
\begingroup\tiny
\begin{tabular}{rrrrrrrrrrrrrrrrrrrrr}
  & \begin{sideways} Temperate or sub-polar needleleaf forest \end{sideways} & \begin{sideways} Sub-polar taiga needleleaf forest \end{sideways} & \begin{sideways} Tropical or sub-tropical broadleaf evergreen forest \end{sideways} & \begin{sideways} Tropical or sub-tropical broadleaf deciduous forest \end{sideways} & \begin{sideways} Temperate or sub-polar broadleaf deciduous forest \end{sideways} & \begin{sideways} Mixed Forest \end{sideways} & \begin{sideways} Tropical or sub-tropical shrubland \end{sideways} & \begin{sideways} Temperate or sub-polar shrubland \end{sideways} & \begin{sideways} Tropical or sub-tropical grassland \end{sideways} & \begin{sideways} Temperate or sub-polar grassland \end{sideways} & \begin{sideways} Sub-polar or polar shrubland-lichen-moss \end{sideways} & \begin{sideways} Sub-polar or polar grassland-lichen-moss \end{sideways} & \begin{sideways} Sub-polar or polar barren-lichen-moss \end{sideways} & \begin{sideways} Wetland \end{sideways} & \begin{sideways} Cropland \end{sideways} & \begin{sideways} Barren Lands \end{sideways} & \begin{sideways} Urban and Built-up \end{sideways} & \begin{sideways} Water \end{sideways} & \begin{sideways} Snow and Ice \end{sideways} & \begin{sideways} Total \end{sideways} \\ 
  \hline
Temperate or sub-polar needleleaf forest &   25 &    0 &    0 &    0 &    0 &    0 &    0 &    1 &    0 &    0 &    0 &    0 &    0 &    0 &    0 &    0 &    5 &    0 &    0 &   31 \\ 
  Sub-polar taiga needleleaf forest &    0 &    0 &    0 &    0 &    0 &    0 &    0 &    0 &    0 &    0 &    0 &    0 &    0 &    0 &    0 &    0 &    0 &    0 &    0 &    0 \\ 
  Tropical or sub-tropical broadleaf evergreen forest &    0 &    0 &    0 &    0 &    0 &    0 &    0 &    0 &    0 &    0 &    0 &    0 &    0 &    0 &    0 &    0 &    0 &    0 &    0 &    0 \\ 
  Tropical or sub-tropical broadleaf deciduous forest &    0 &    0 &    0 & 4669 &    0 &    0 &    0 &    0 &    6 &    0 &    0 &    0 &    0 &    0 &   14 &    0 &   37 &    0 &    0 & 4726 \\ 
  Temperate or sub-polar broadleaf deciduous forest &    0 &    0 &    0 &    1 &  243 &    0 &    0 &    4 &    0 &    0 &    0 &    0 &    0 &    0 &   12 &    0 &   19 &    0 &    0 &  279 \\ 
  Mixed Forest &    0 &    0 &    0 &    0 &    0 &  603 &    0 &    0 &    0 &    0 &    0 &    0 &    0 &    0 &    0 &    0 &    0 &    0 &    0 &  603 \\ 
   \hline
Tropical or sub-tropical shrubland &    0 &    0 &    0 &    0 &    0 &    0 &    9 &    0 &    0 &    0 &    0 &    0 &    0 &    0 &    0 &    0 &    0 &    0 &    0 &    9 \\ 
  Temperate or sub-polar shrubland &    3 &    0 &    0 &    6 &    0 &    0 &    0 & 1762 &    0 &    0 &    0 &    0 &    0 &    0 &    6 &    0 &   76 &    0 &    0 & 1853 \\ 
  Tropical or sub-tropical grassland &    0 &    0 &    0 &    0 &    0 &    0 &    0 &    0 &    0 &    0 &    0 &    0 &    0 &    0 &    0 &    0 &    0 &    0 &    0 &    0 \\ 
  Temperate or sub-polar grassland &    0 &    0 &    0 &    0 &    0 &    0 &    0 &    0 &    0 &    0 &    0 &    0 &    0 &    0 &    0 &    0 &    0 &    0 &    0 &    0 \\ 
  Sub-polar or polar shrubland-lichen-moss &    0 &    0 &    0 &    0 &    0 &    0 &    0 &    0 &    0 &    0 &    0 &    0 &    0 &    0 &    0 &    0 &    0 &    0 &    0 &    0 \\ 
  Sub-polar or polar grassland-lichen-moss &    0 &    0 &    0 &    0 &    0 &    0 &    0 &    0 &    0 &    0 &    0 &    0 &    0 &    0 &    0 &    0 &    0 &    0 &    0 &    0 \\ 
  Sub-polar or polar barren-lichen-moss &    0 &    0 &    0 &    0 &    0 &    0 &    0 &    0 &    0 &    0 &    0 &    0 &    0 &    0 &    0 &    0 &    0 &    0 &    0 &    0 \\ 
  Wetland &    0 &    0 &    0 &    0 &    0 &    0 &    0 &    0 &    0 &    0 &    0 &    0 &    0 &    0 &    0 &    0 &    0 &    0 &    0 &    0 \\ 
  Cropland &    1 &    0 &    0 &    2 &    1 &    0 &    0 &    1 &   12 &    0 &    0 &    0 &    0 &    0 & 2012 &    0 &  105 &    0 &    0 & 2134 \\ 
  Barren Lands &    0 &    0 &    0 &    0 &    0 &    0 &    0 &    0 &    0 &    0 &    0 &    0 &    0 &    0 &    0 &    0 &    0 &    0 &    0 &    0 \\ 
  Urban and Built-up &    0 &    0 &    0 &    0 &    0 &    0 &    0 &    0 &    0 &    0 &    0 &    0 &    0 &    0 &    0 &    0 &  357 &    0 &    0 &  357 \\ 
  Water &    0 &    0 &    0 &    0 &    0 &    0 &    0 &    0 &    0 &    0 &    0 &    0 &    0 &    0 &    0 &    0 &    0 &    8 &    0 &    8 \\ 
  Snow and Ice &    0 &    0 &    0 &    0 &    0 &    0 &    0 &    0 &    0 &    0 &    0 &    0 &    0 &    0 &    0 &    0 &    0 &    0 &    0 &    0 \\ 
   \hline
Total &   29 &    0 &    0 & 4678 &  244 &  603 &    9 & 1768 &   18 &    0 &    0 &    0 &    0 &    0 & 2044 &    0 &  599 &    8 &    0 & 10000 \\ 
   \hline
\end{tabular}
\endgroup
\caption[NALCMS land-use distribution for site Michoacan98, 2005 and 2010.]{NALCMS land-use distribution for site Michoacan98, 2005 and 2010.} 
\end{table}

   			\label{tab:landUseSonora}
   		\end{center}
		
   		\begin{figure}[H]%--- Picture 'H'ere, 'B'ottom or 'T'op; '!' Try to
   		                    %impose your will to LaTeX
   		  \centering
   		  \includegraphics[width=.5\textwidth]{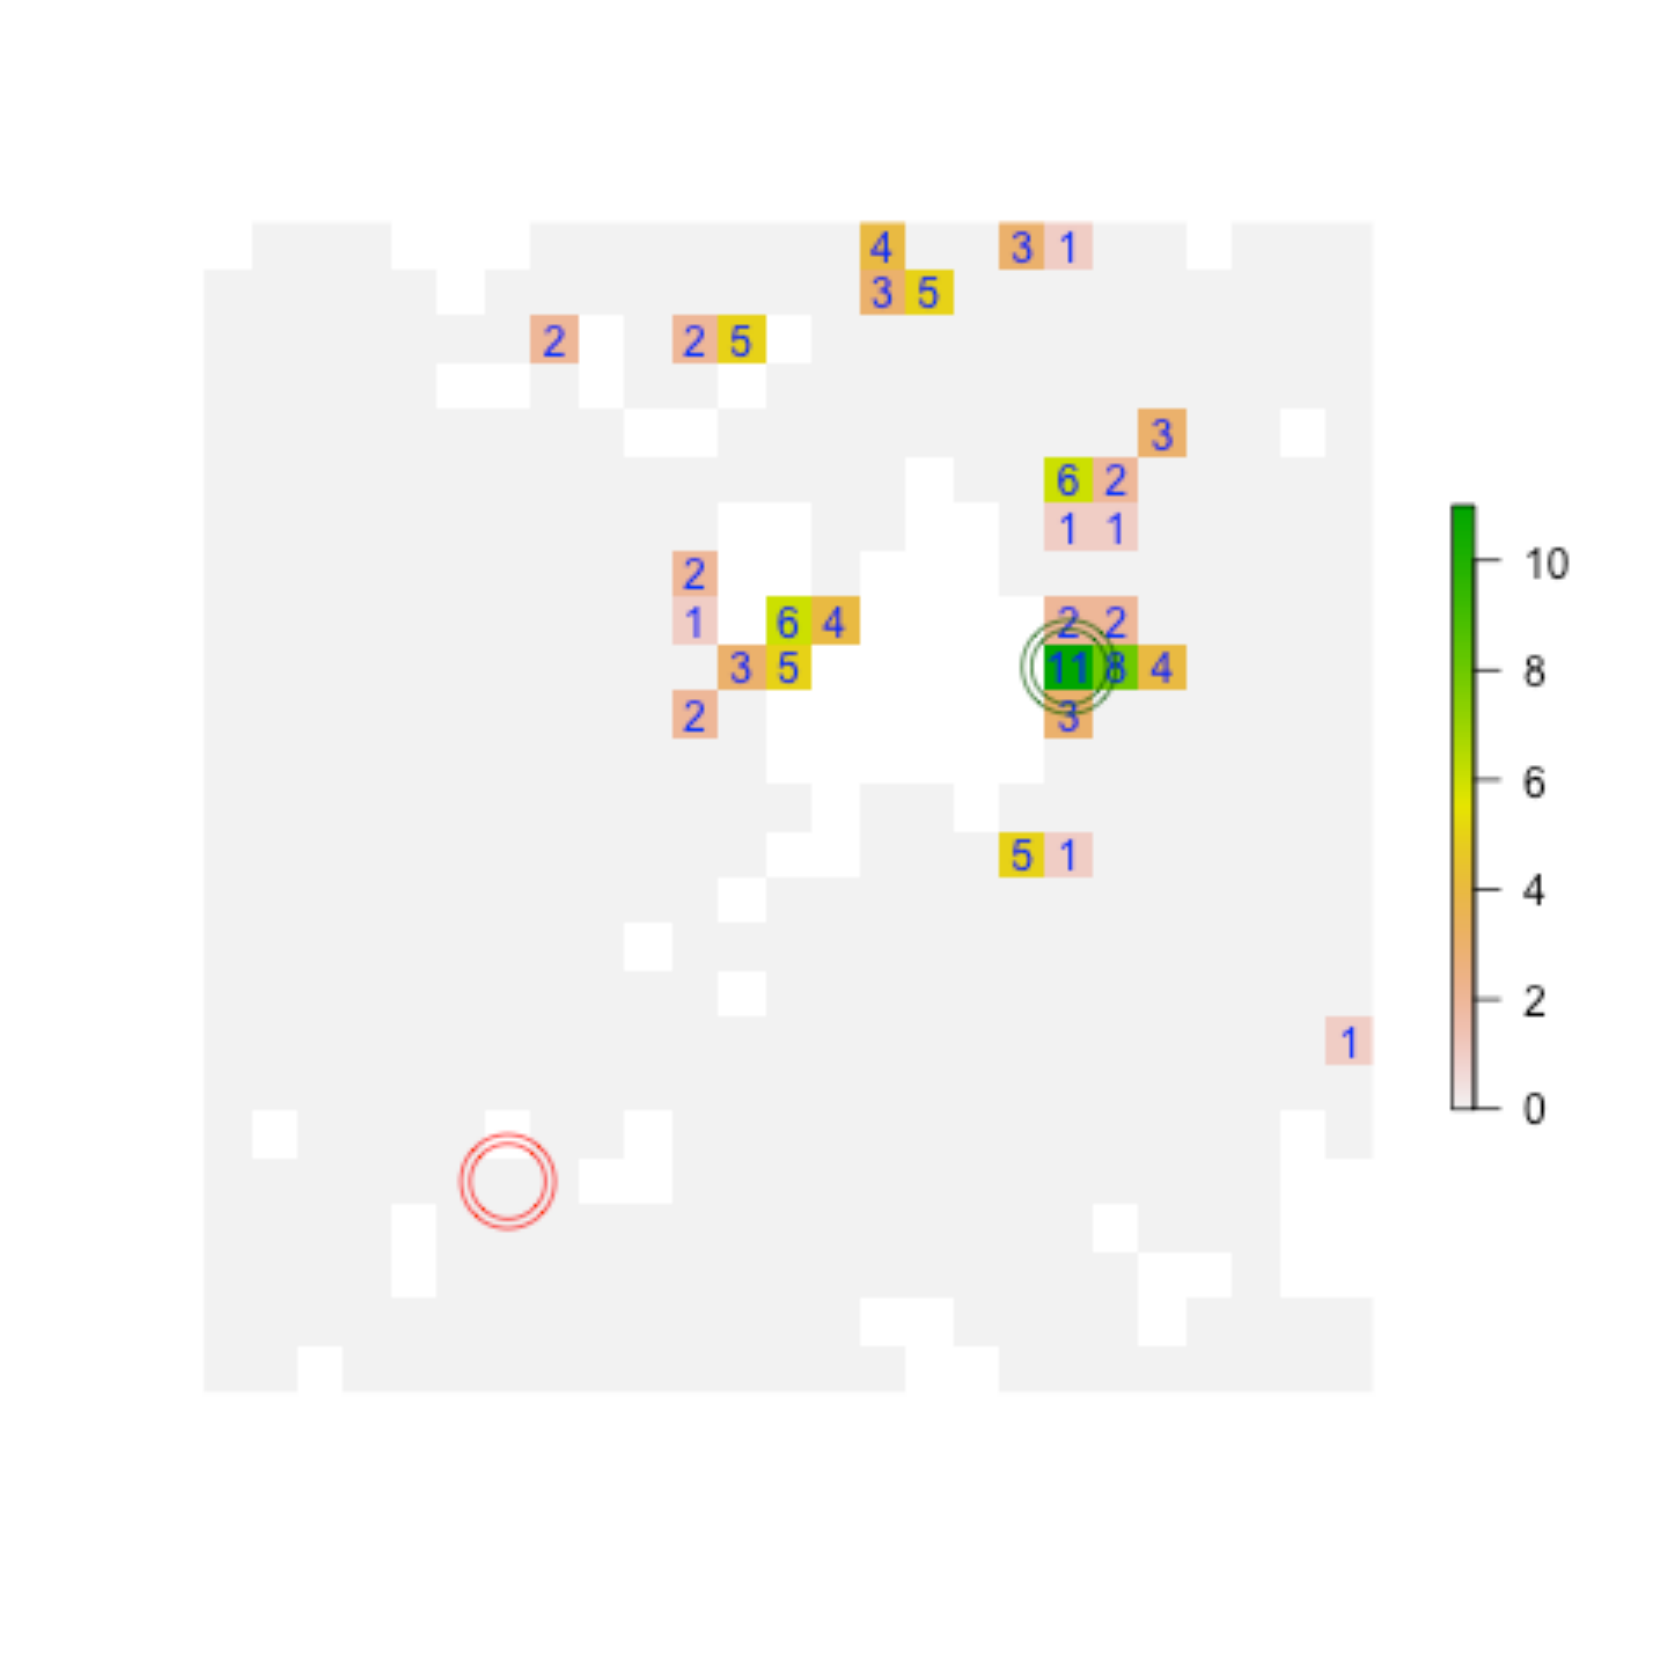} %<< no file extension
   		  %%         --- .5\textwidth stands for 50% of text width
   		  \caption[Deforestation in Michoacan98 site at 1km resolution]%<<-- Legend for the list of figures at the beginning of you thesis
   		  {Deforestation in Michoacan98 site at 1km resolution: number of 250m pixels deforested out of 16}% legend displayed below the graph.
   		  \label{fig:defoMichoacan98}
   		\end{figure}
		
   		 \begin{figure}[H]
   	      \begin{subfigure}{.5\textwidth}
   	        \centering
   	    	\includegraphics[width=1\textwidth]{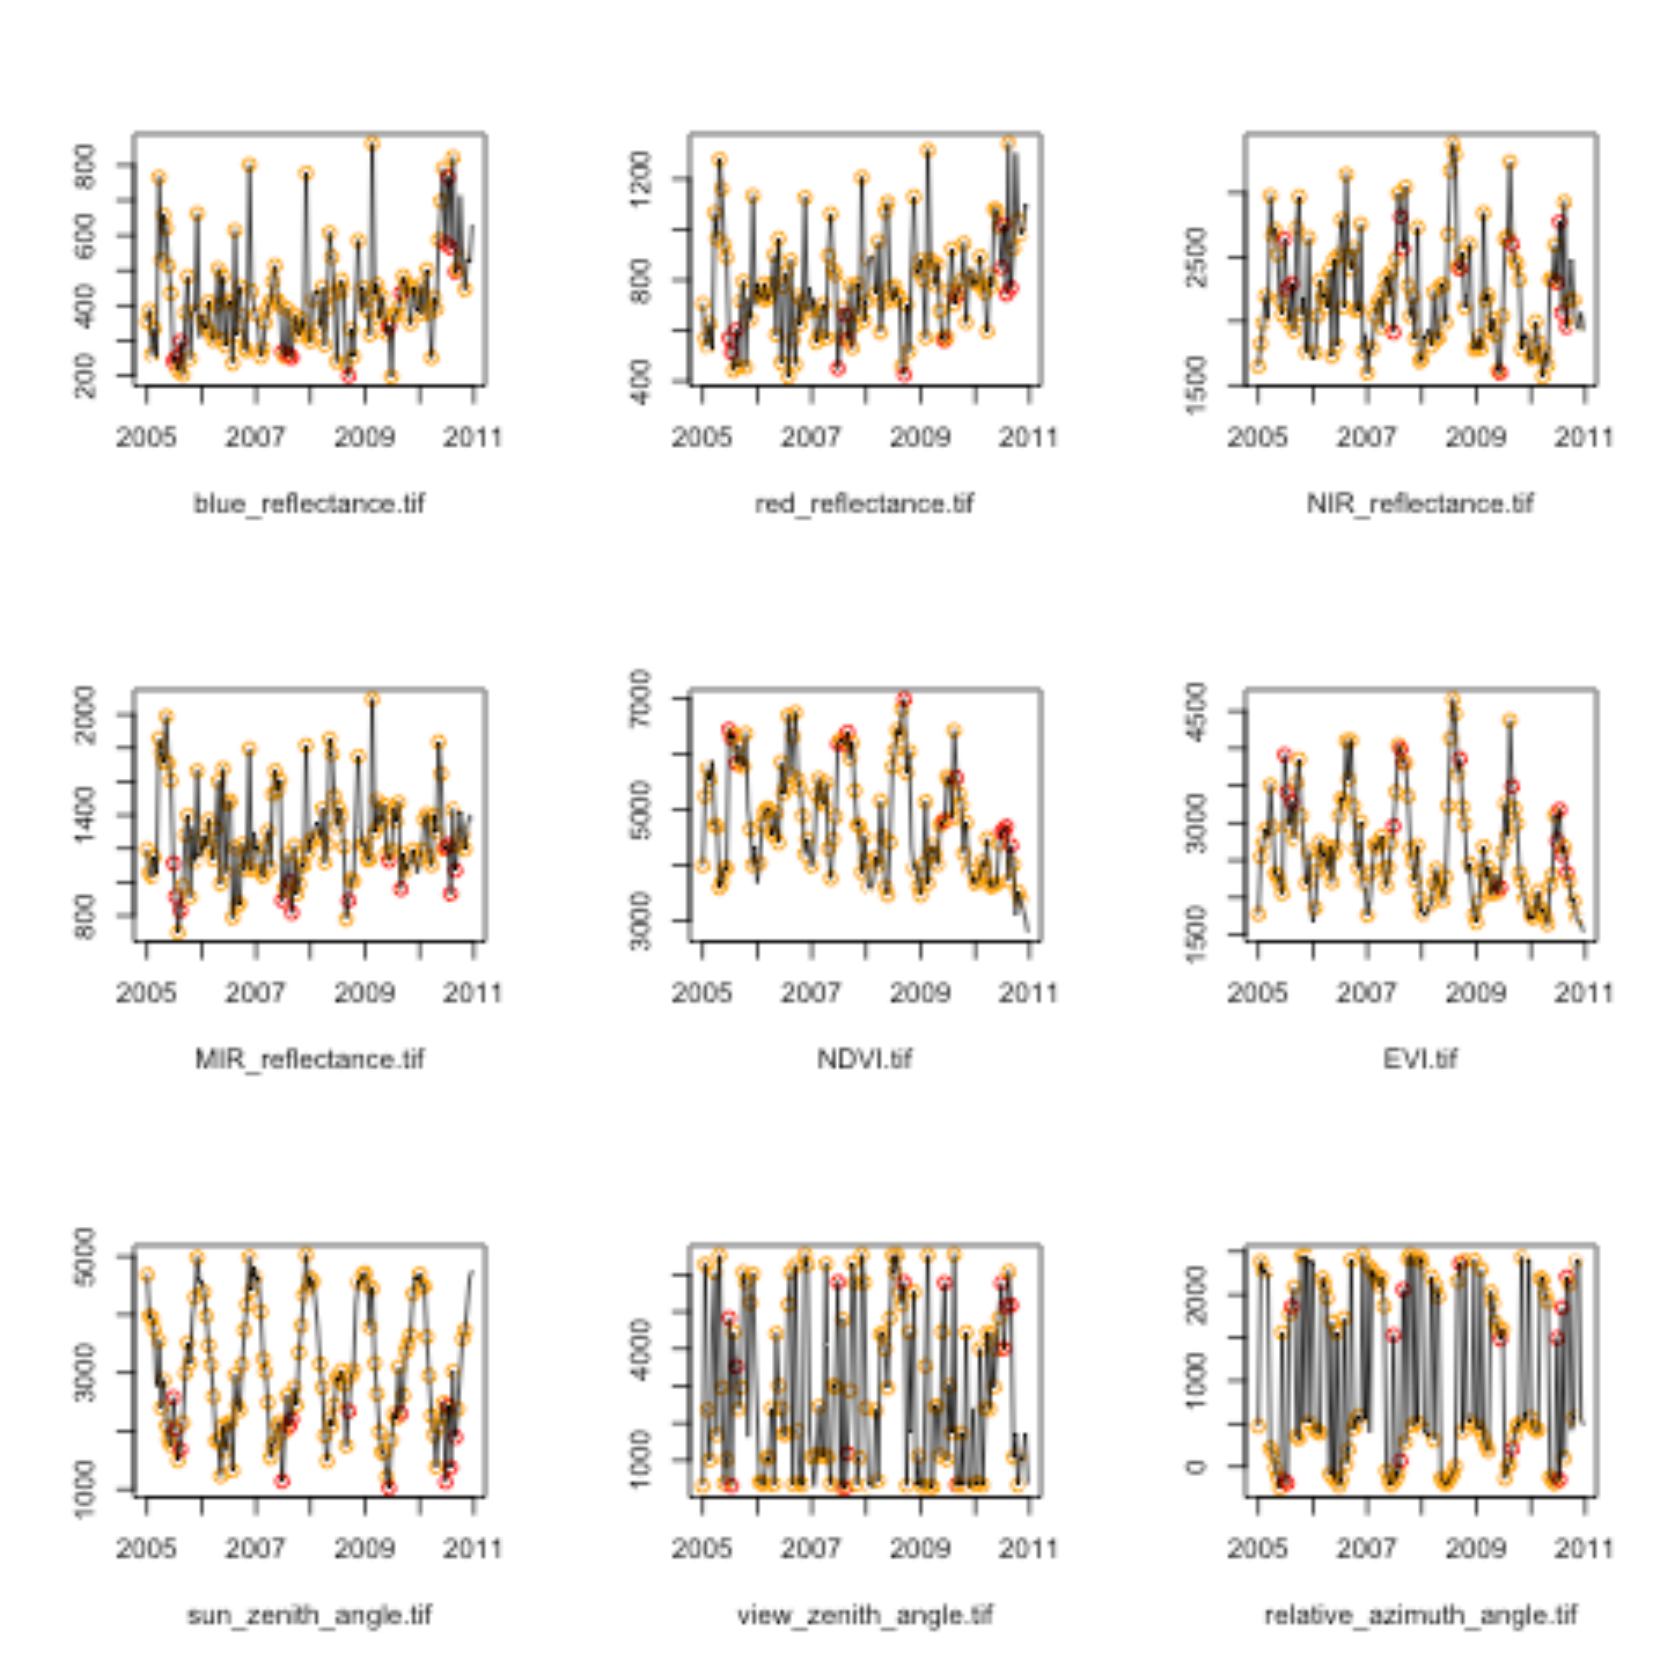} 
   	        \caption{deforested pixel}
   	        \label{fig:defo_pix}
   	      \end{subfigure}%
   	      \begin{subfigure}{.5\textwidth}
   	        \centering
   	        \includegraphics[width=1\textwidth]{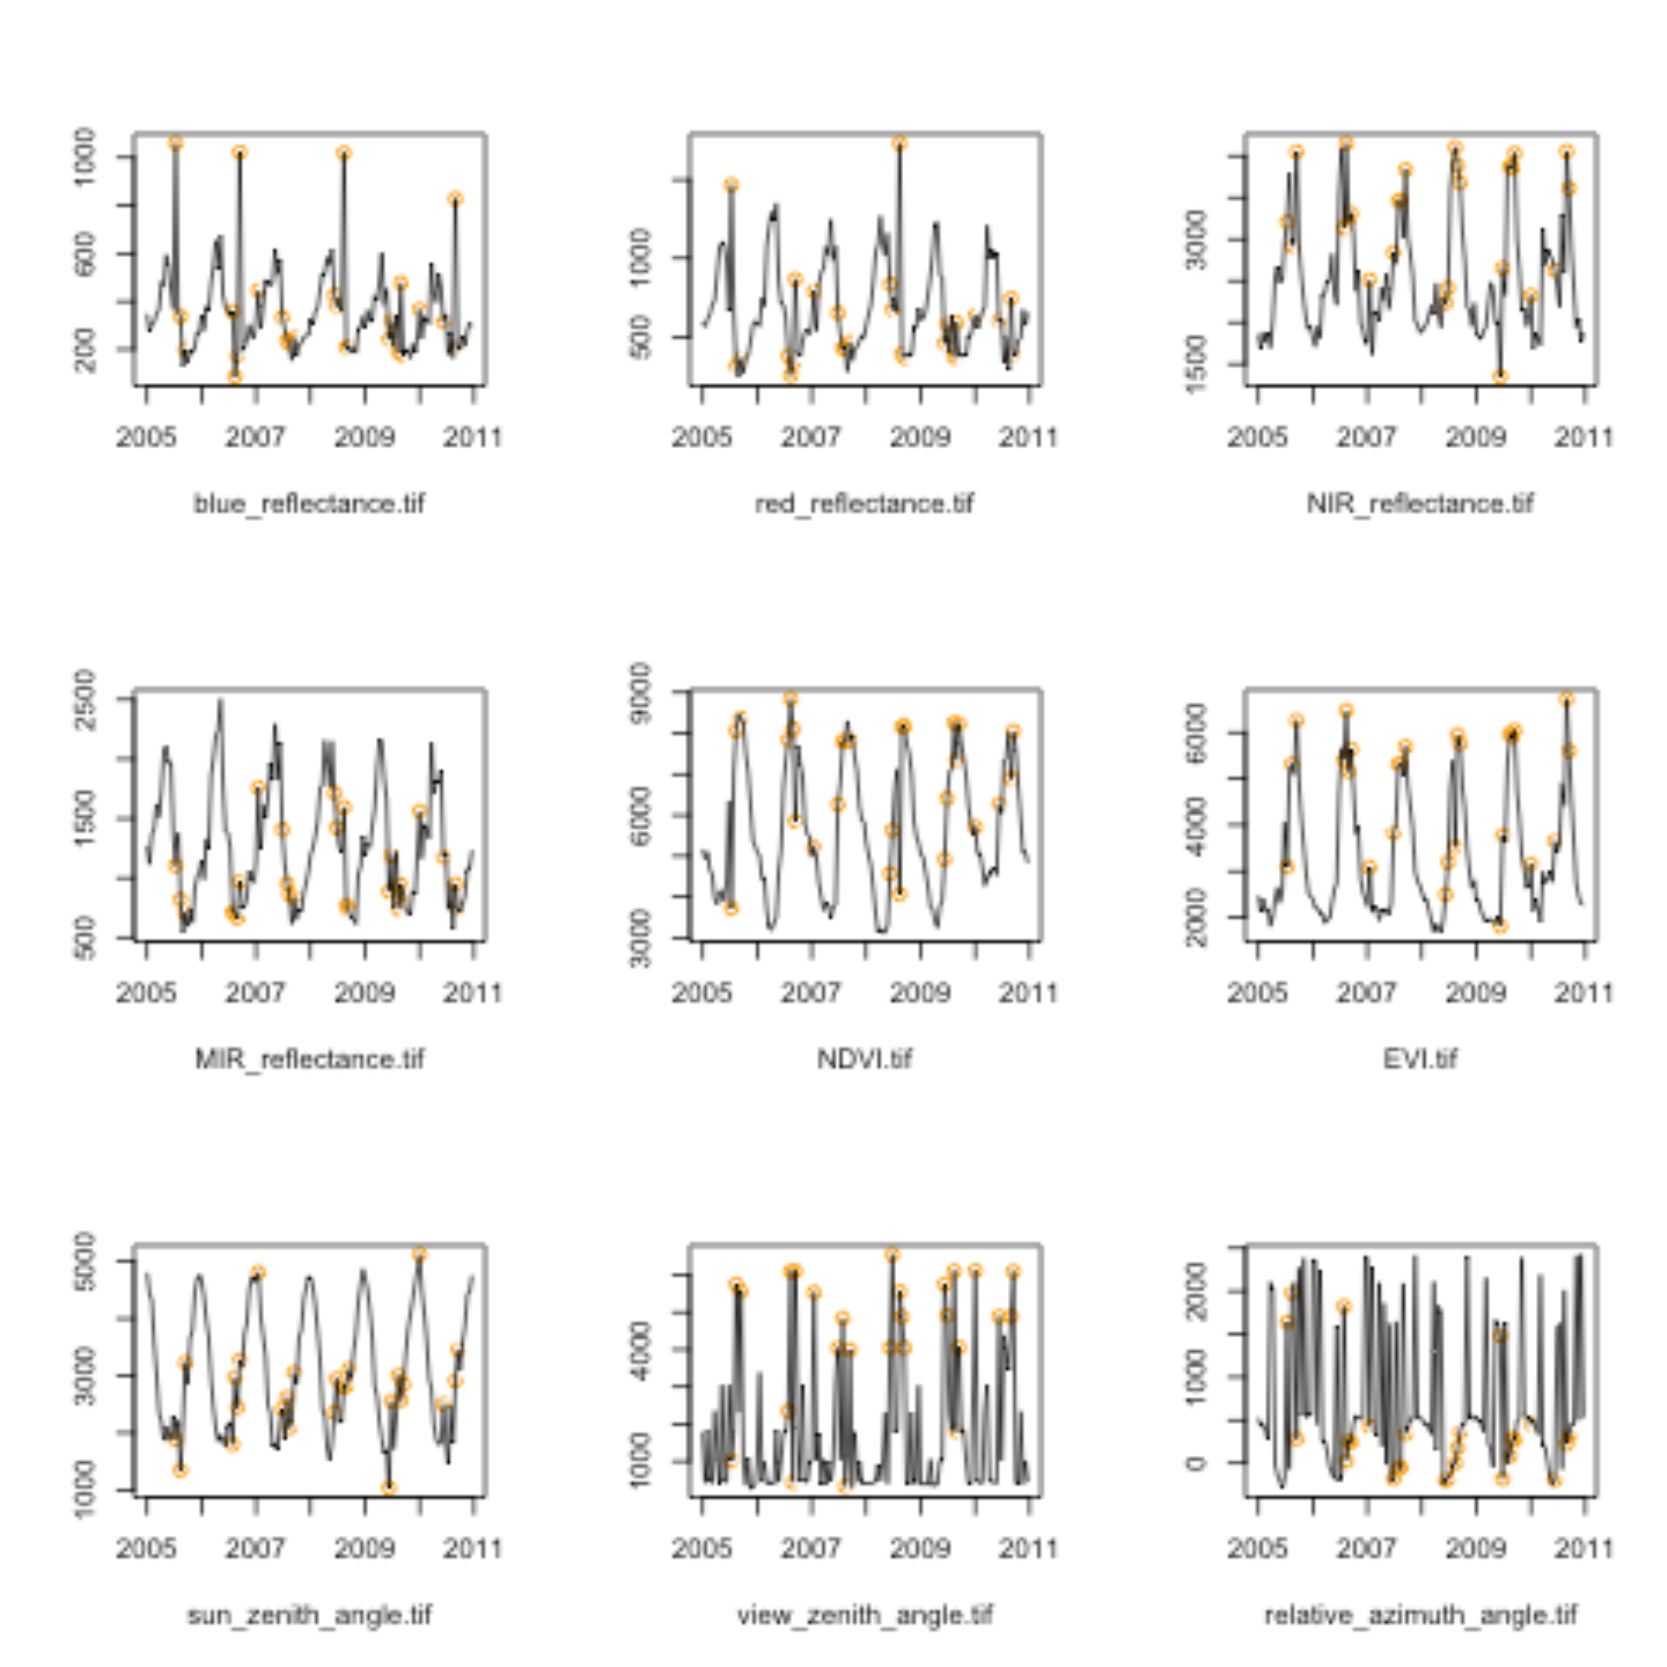}
   	        \caption{non-deforested pixel}
   	        \label{fig:non_defo_pix}
   	      \end{subfigure}
   	      %%         --- .5\textwidth stands for 50% of text width
   	      \caption[Reflectance, vegetation indices and sun-sensor geometry time series for deforested and non-deforested pixel in Yucatan 180 site.]%<<-- Legend for the list of figures at the beginning of you thesis
   	      {Reflectance, vegetation indices and sun-sensor geometry time series for deforested and non-deforested pixel in Michoacan98 site, identified in figure \ref{fig:defoMichoacan98} with green and red circles respectively. Orange marked points are \emph{marginal data} and red marked points are \emph{cloudy} or \emph{not processed}}% legend displayed below the graph.
   	      \label{fig:timeSeries}
   	    \end{figure}
		
		\subsubsection{QuintanaRoo77}
		
      	 \begin{figure}[H]  %--- Picture 'H'ere, 'B'ottom or 'T'op; '!' Try to
      	                     %impose your will to LaTeX
      	  % \centering 
  
      	   \begin{subfigure}{.5\textwidth}
      	     \centering
      	 	\includegraphics[width=0.7\textwidth]{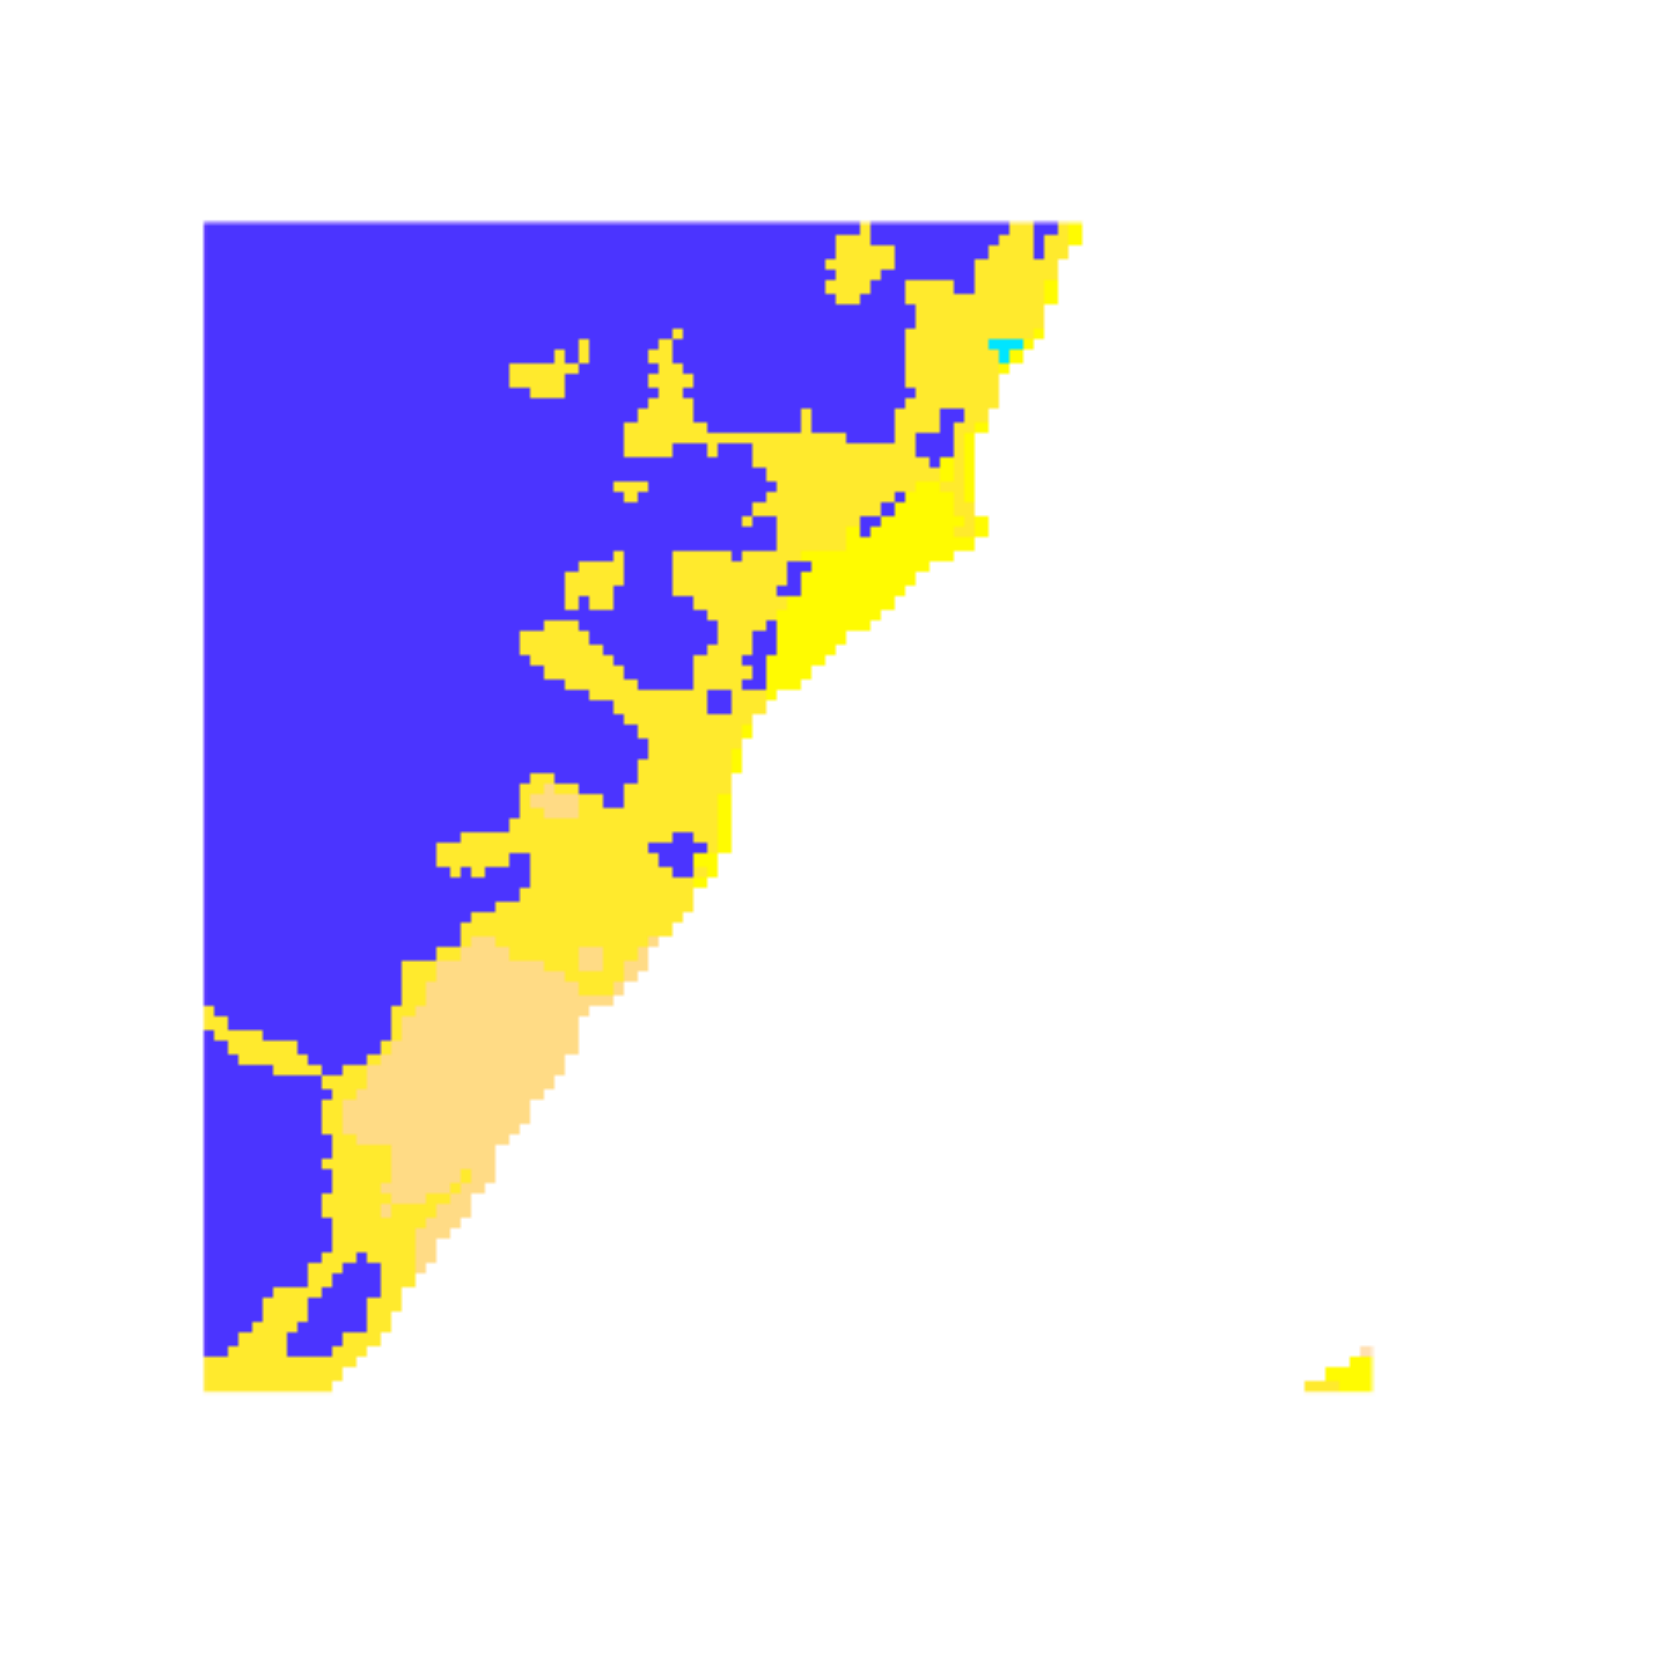} 
      	     \caption{Land-use 2005}
      	     \label{fig:sfig1a}
      	   \end{subfigure}%
      	   \begin{subfigure}{.5\textwidth}
      	     \centering
      	     \includegraphics[width=0.7\textwidth]{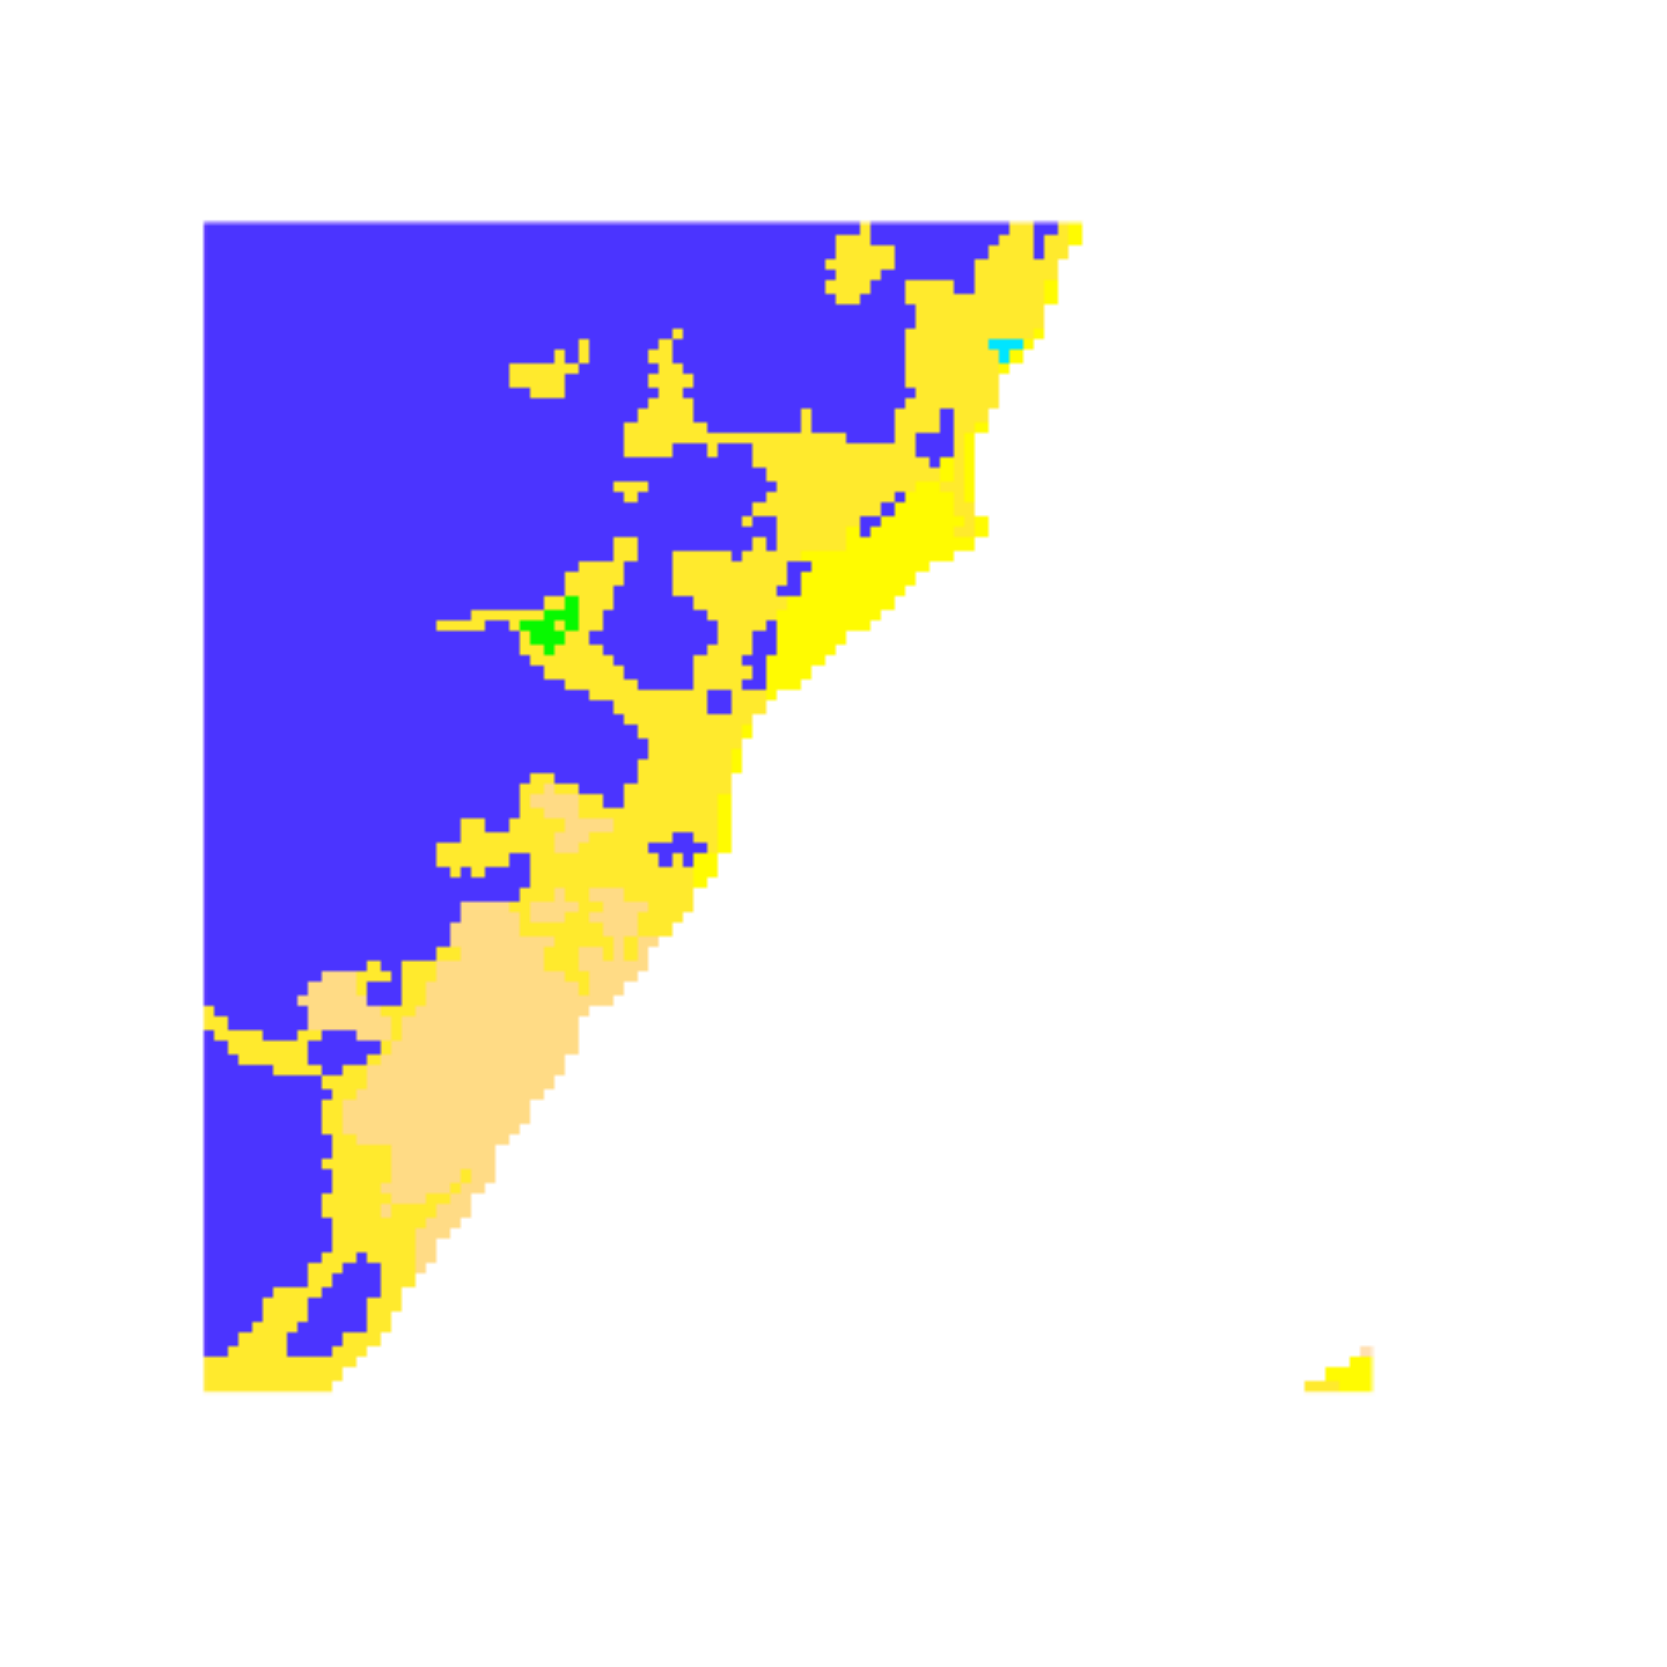}
      	     \caption{Land-use 2010}
      	     \label{fig:sfig1b}
      	   \end{subfigure}
      	   \begin{subfigure}{.4\textwidth}
      	     \centering
      	     \includegraphics[width=0.9\textwidth]{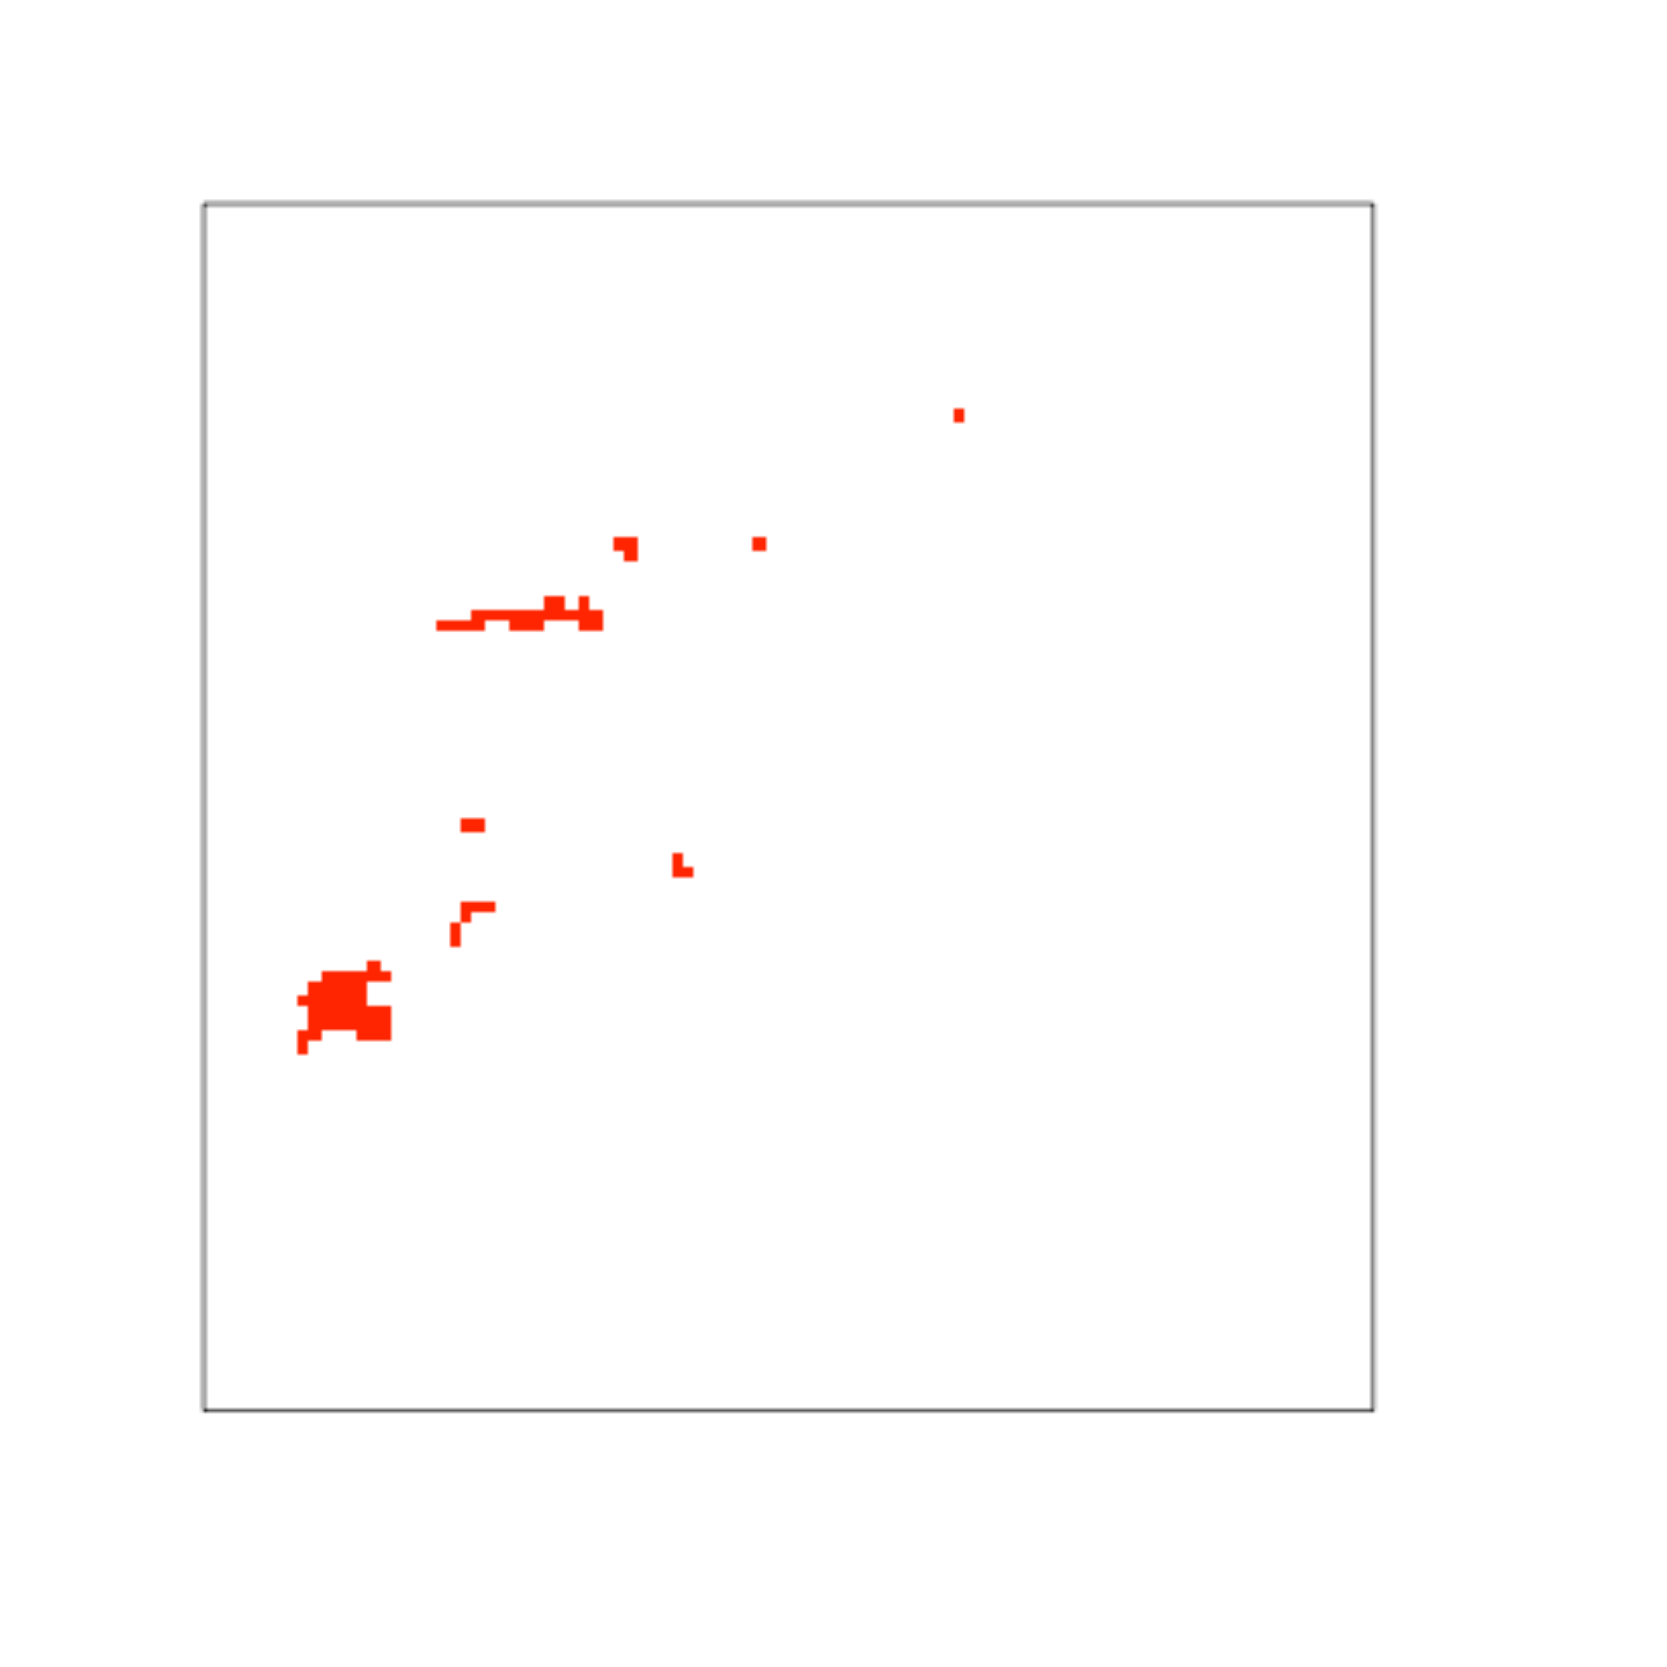}
      	     \caption{Deforestation 2005-2010}
      	     \label{fig:sfig1c}
      	   \end{subfigure}
      	   \begin{subfigure}{.4\textwidth}
      	     \centering
      	     \includegraphics[width=0.9\textwidth]{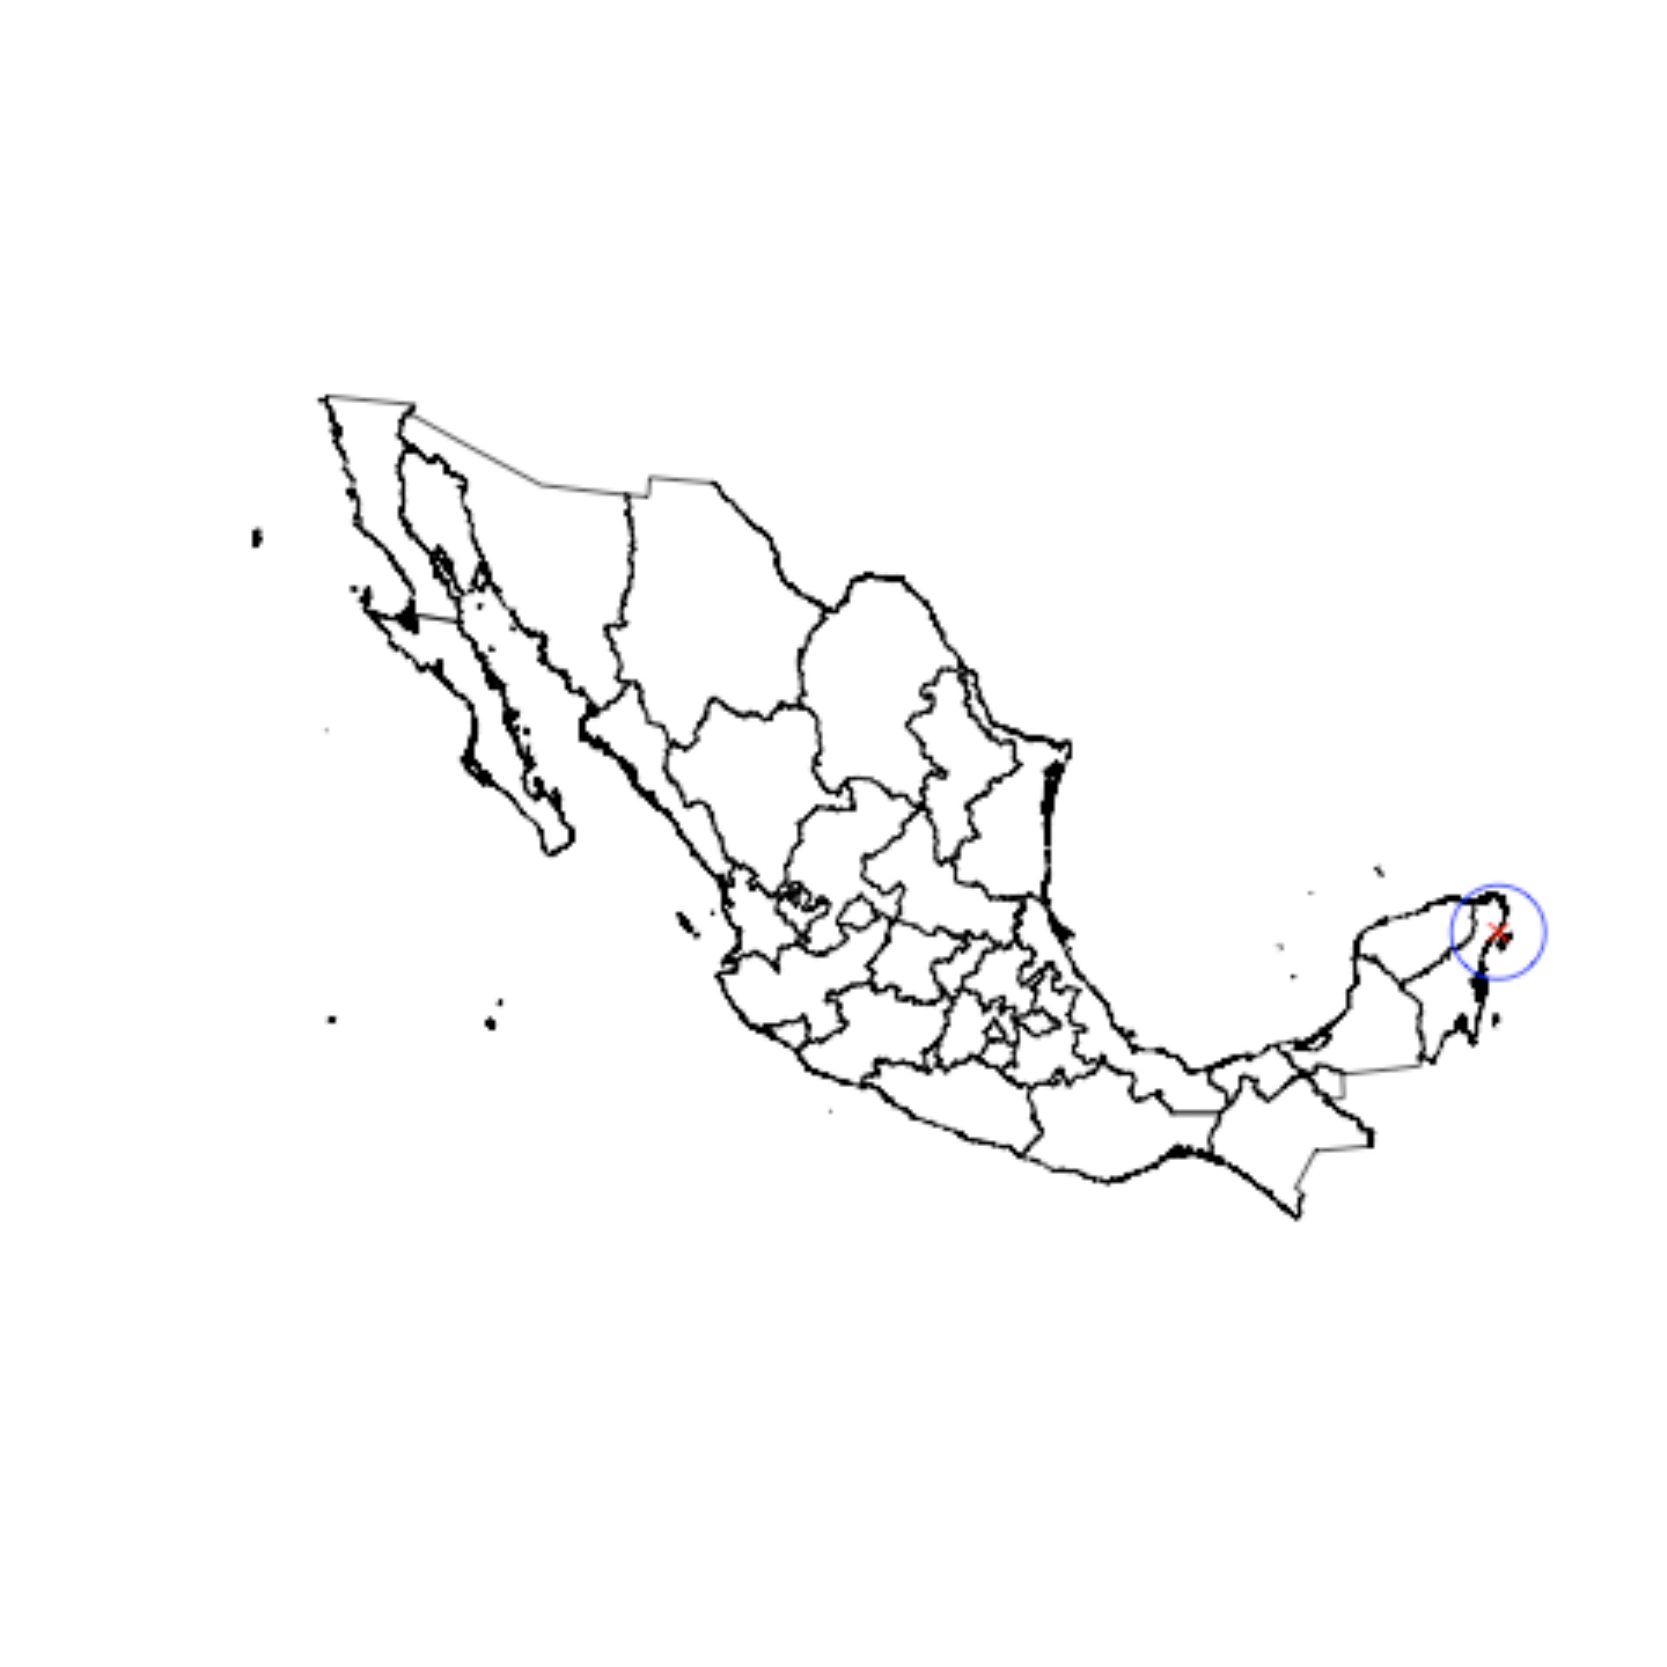}
      	     \caption{Location}
      	     \label{fig:sfig1d}
      	   \end{subfigure}   
         \begin{subfigure}{.5\textwidth}
           \centering
           \includegraphics[width=1\textwidth]{./2_Data/legend_landUse}
           \caption{Land use legend}
           \label{fig:legend}
         \end{subfigure}
      	   %%         --- .5\textwidth stands for 50% of text width
      	   \caption[NALCMS land-use classification of QuintanaRoo77 site, 2005 and 2010 at 250m resolution.]%<<-- Legend for the list of figures at the beginning of you thesis
      	   {NALCMS land-use classification of QuintanaRoo77 site, 2005 and 2010 at 250m resolution.}% legend displayed below the graph.
      	   \label{fig:landUseQuintanaRoo77}
      	 \end{figure}
		
   		\begin{center}
   			\footnotesize\addtolength{\tabcolsep}{-2pt}
   			% latex table generated in R 3.3.1 by xtable 1.8-2 package
% Sun Mar  5 16:02:46 2017
\begin{table}[ht]
\centering
\begingroup\tiny
\begin{tabular}{rrrrrrrrrrrrrrrrrrrrr}
  & \begin{sideways} Temperate or sub-polar needleleaf forest \end{sideways} & \begin{sideways} Sub-polar taiga needleleaf forest \end{sideways} & \begin{sideways} Tropical or sub-tropical broadleaf evergreen forest \end{sideways} & \begin{sideways} Tropical or sub-tropical broadleaf deciduous forest \end{sideways} & \begin{sideways} Temperate or sub-polar broadleaf deciduous forest \end{sideways} & \begin{sideways} Mixed Forest \end{sideways} & \begin{sideways} Tropical or sub-tropical shrubland \end{sideways} & \begin{sideways} Temperate or sub-polar shrubland \end{sideways} & \begin{sideways} Tropical or sub-tropical grassland \end{sideways} & \begin{sideways} Temperate or sub-polar grassland \end{sideways} & \begin{sideways} Sub-polar or polar shrubland-lichen-moss \end{sideways} & \begin{sideways} Sub-polar or polar grassland-lichen-moss \end{sideways} & \begin{sideways} Sub-polar or polar barren-lichen-moss \end{sideways} & \begin{sideways} Wetland \end{sideways} & \begin{sideways} Cropland \end{sideways} & \begin{sideways} Barren Lands \end{sideways} & \begin{sideways} Urban and Built-up \end{sideways} & \begin{sideways} Water \end{sideways} & \begin{sideways} Snow and Ice \end{sideways} & \begin{sideways} Total \end{sideways} \\ 
  \hline
Temperate or sub-polar needleleaf forest &    0 &    0 &    0 &    0 &    0 &    0 &    0 &    0 &    0 &    0 &    0 &    0 &    0 &    0 &    0 &    0 &    0 &    0 &    0 &    0 \\ 
  Sub-polar taiga needleleaf forest &    0 &    0 &    0 &    0 &    0 &    0 &    0 &    0 &    0 &    0 &    0 &    0 &    0 &    0 &    0 &    0 &    0 &    0 &    0 &    0 \\ 
  Tropical or sub-tropical broadleaf evergreen forest &    0 &    0 & 2975 &    0 &    0 &    0 &    0 &    0 &    5 &    0 &    0 &    0 &    0 &    0 &   37 &    0 &   35 &    0 &    0 & 3052 \\ 
  Tropical or sub-tropical broadleaf deciduous forest &    0 &    0 &    0 &    0 &    0 &    0 &    0 &    0 &    0 &    0 &    0 &    0 &    0 &    0 &    0 &    0 &    0 &    0 &    0 &    0 \\ 
  Temperate or sub-polar broadleaf deciduous forest &    0 &    0 &    0 &    0 &    0 &    0 &    0 &    0 &    0 &    0 &    0 &    0 &    0 &    0 &    0 &    0 &    0 &    0 &    0 &    0 \\ 
  Mixed Forest &    0 &    0 &    0 &    0 &    0 &    0 &    0 &    0 &    0 &    0 &    0 &    0 &    0 &    0 &    0 &    0 &    0 &    0 &    0 &    0 \\ 
   \hline
Tropical or sub-tropical shrubland &    0 &    0 &    0 &    0 &    0 &    0 &    4 &    0 &    0 &    0 &    0 &    0 &    0 &    0 &    0 &    0 &    0 &    0 &    0 &    4 \\ 
  Temperate or sub-polar shrubland &    0 &    0 &    0 &    0 &    0 &    0 &    0 &    0 &    0 &    0 &    0 &    0 &    0 &    0 &    0 &    0 &    0 &    0 &    0 &    0 \\ 
  Tropical or sub-tropical grassland &    0 &    0 &    0 &    0 &    0 &    0 &    0 &    0 &    0 &    0 &    0 &    0 &    0 &    0 &    0 &    0 &    0 &    0 &    0 &    0 \\ 
  Temperate or sub-polar grassland &    0 &    0 &    0 &    0 &    0 &    0 &    0 &    0 &    0 &    0 &    0 &    0 &    0 &    0 &    0 &    0 &    0 &    0 &    0 &    0 \\ 
  Sub-polar or polar shrubland-lichen-moss &    0 &    0 &    0 &    0 &    0 &    0 &    0 &    0 &    0 &    0 &    0 &    0 &    0 &    0 &    0 &    0 &    0 &    0 &    0 &    0 \\ 
  Sub-polar or polar grassland-lichen-moss &    0 &    0 &    0 &    0 &    0 &    0 &    0 &    0 &    0 &    0 &    0 &    0 &    0 &    0 &    0 &    0 &    0 &    0 &    0 &    0 \\ 
  Sub-polar or polar barren-lichen-moss &    0 &    0 &    0 &    0 &    0 &    0 &    0 &    0 &    0 &    0 &    0 &    0 &    0 &    0 &    0 &    0 &    0 &    0 &    0 &    0 \\ 
  Wetland &    0 &    0 &    0 &    0 &    0 &    0 &    0 &    0 &    0 &    0 &    0 &    0 &    0 &  169 &    0 &    0 &    0 &    0 &    0 &  169 \\ 
  Cropland &    0 &    0 &    0 &    0 &    0 &    0 &    0 &    0 &    7 &    0 &    0 &    0 &    0 &    1 &  952 &    0 &   60 &    0 &    0 & 1020 \\ 
  Barren Lands &    0 &    0 &    0 &    0 &    0 &    0 &    0 &    0 &    0 &    0 &    0 &    0 &    0 &    0 &    0 &    0 &    0 &    0 &    0 &    0 \\ 
  Urban and Built-up &    0 &    0 &    0 &    0 &    0 &    0 &    0 &    0 &    0 &    0 &    0 &    0 &    0 &    0 &    0 &    0 &  313 &    0 &    0 &  313 \\ 
  Water &    0 &    0 &    0 &    0 &    0 &    0 &    0 &    0 &    0 &    0 &    0 &    0 &    0 &    0 &    0 &    0 &    0 &    1 &    0 &    1 \\ 
  Snow and Ice &    0 &    0 &    0 &    0 &    0 &    0 &    0 &    0 &    0 &    0 &    0 &    0 &    0 &    0 &    0 &    0 &    0 &    0 &    0 &    0 \\ 
   \hline
Total &    0 &    0 & 2975 &    0 &    0 &    0 &    4 &    0 &   12 &    0 &    0 &    0 &    0 &  170 &  989 &    0 &  408 &    1 &    0 & 4559 \\ 
   \hline
\end{tabular}
\endgroup
\caption[NALCMS land-use distribution for site QuintanaRoo77, 2005 and 2010.]{NALCMS land-use distribution for site QuintanaRoo77, 2005 and 2010.} 
\end{table}

   			\label{tab:landUseSonora}
   		\end{center}
		
   		\begin{figure}[H]%--- Picture 'H'ere, 'B'ottom or 'T'op; '!' Try to
   		                    %impose your will to LaTeX
   		  \centering
   		  \includegraphics[width=.5\textwidth]{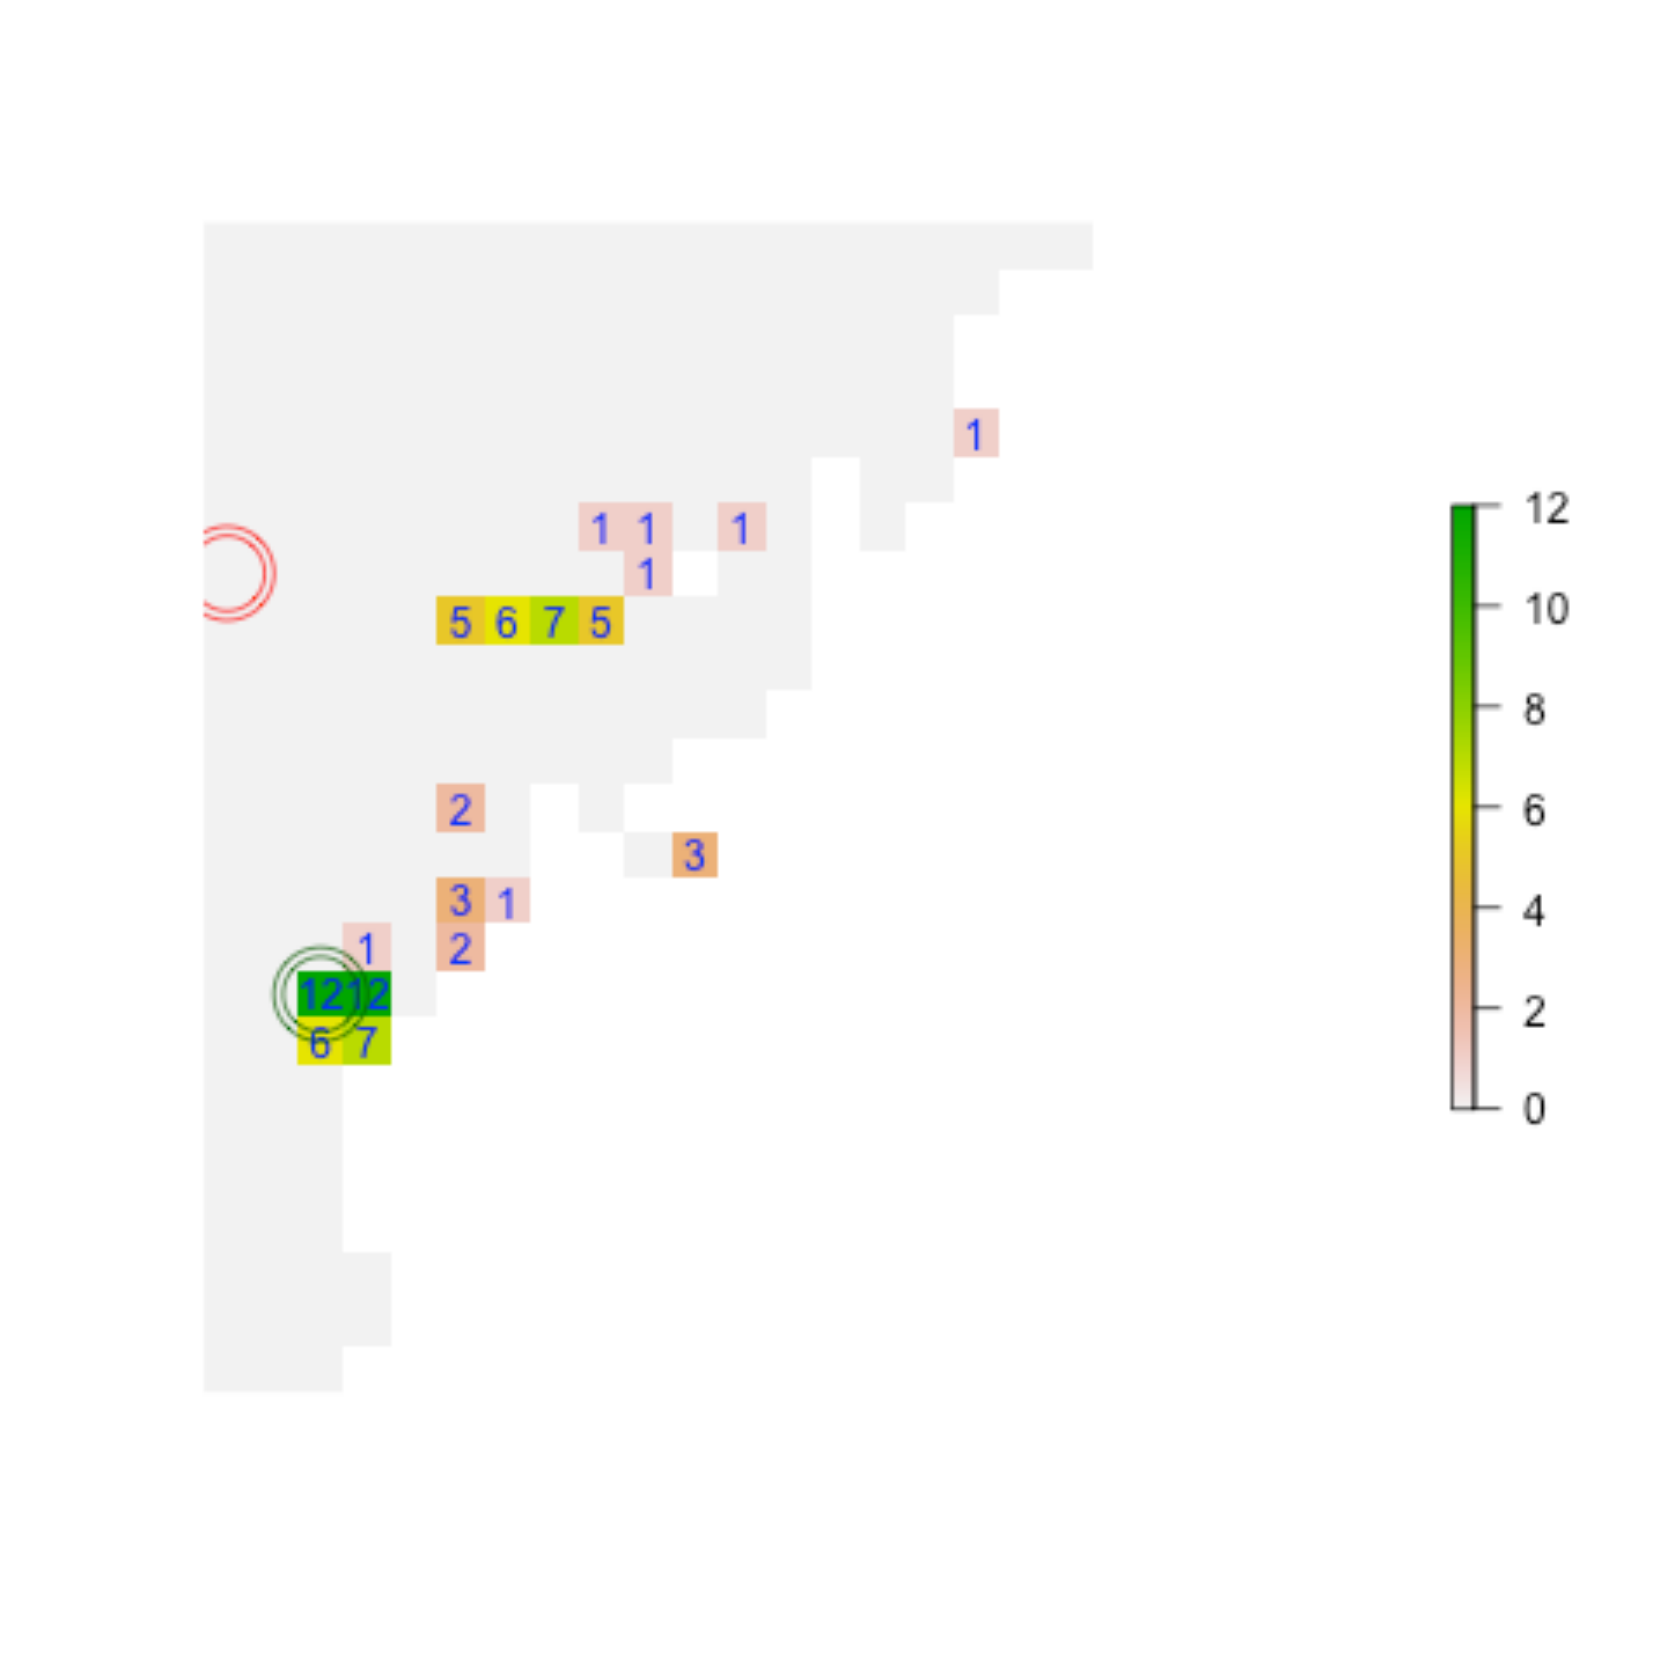} %<< no file extension
   		  %%         --- .5\textwidth stands for 50% of text width
   		  \caption[Deforestation in QuintanaRoo77 site at 1km resolution]%<<-- Legend for the list of figures at the beginning of you thesis
   		  {Deforestation in QuintanaRoo77 site at 1km resolution: number of 250m pixels deforested out of 16}% legend displayed below the graph.
   		  \label{fig:defoQuintanaRoo77}
   		\end{figure}
		
   		 \begin{figure}[H]
   	      \begin{subfigure}{.5\textwidth}
   	        \centering
   	    	\includegraphics[width=1\textwidth]{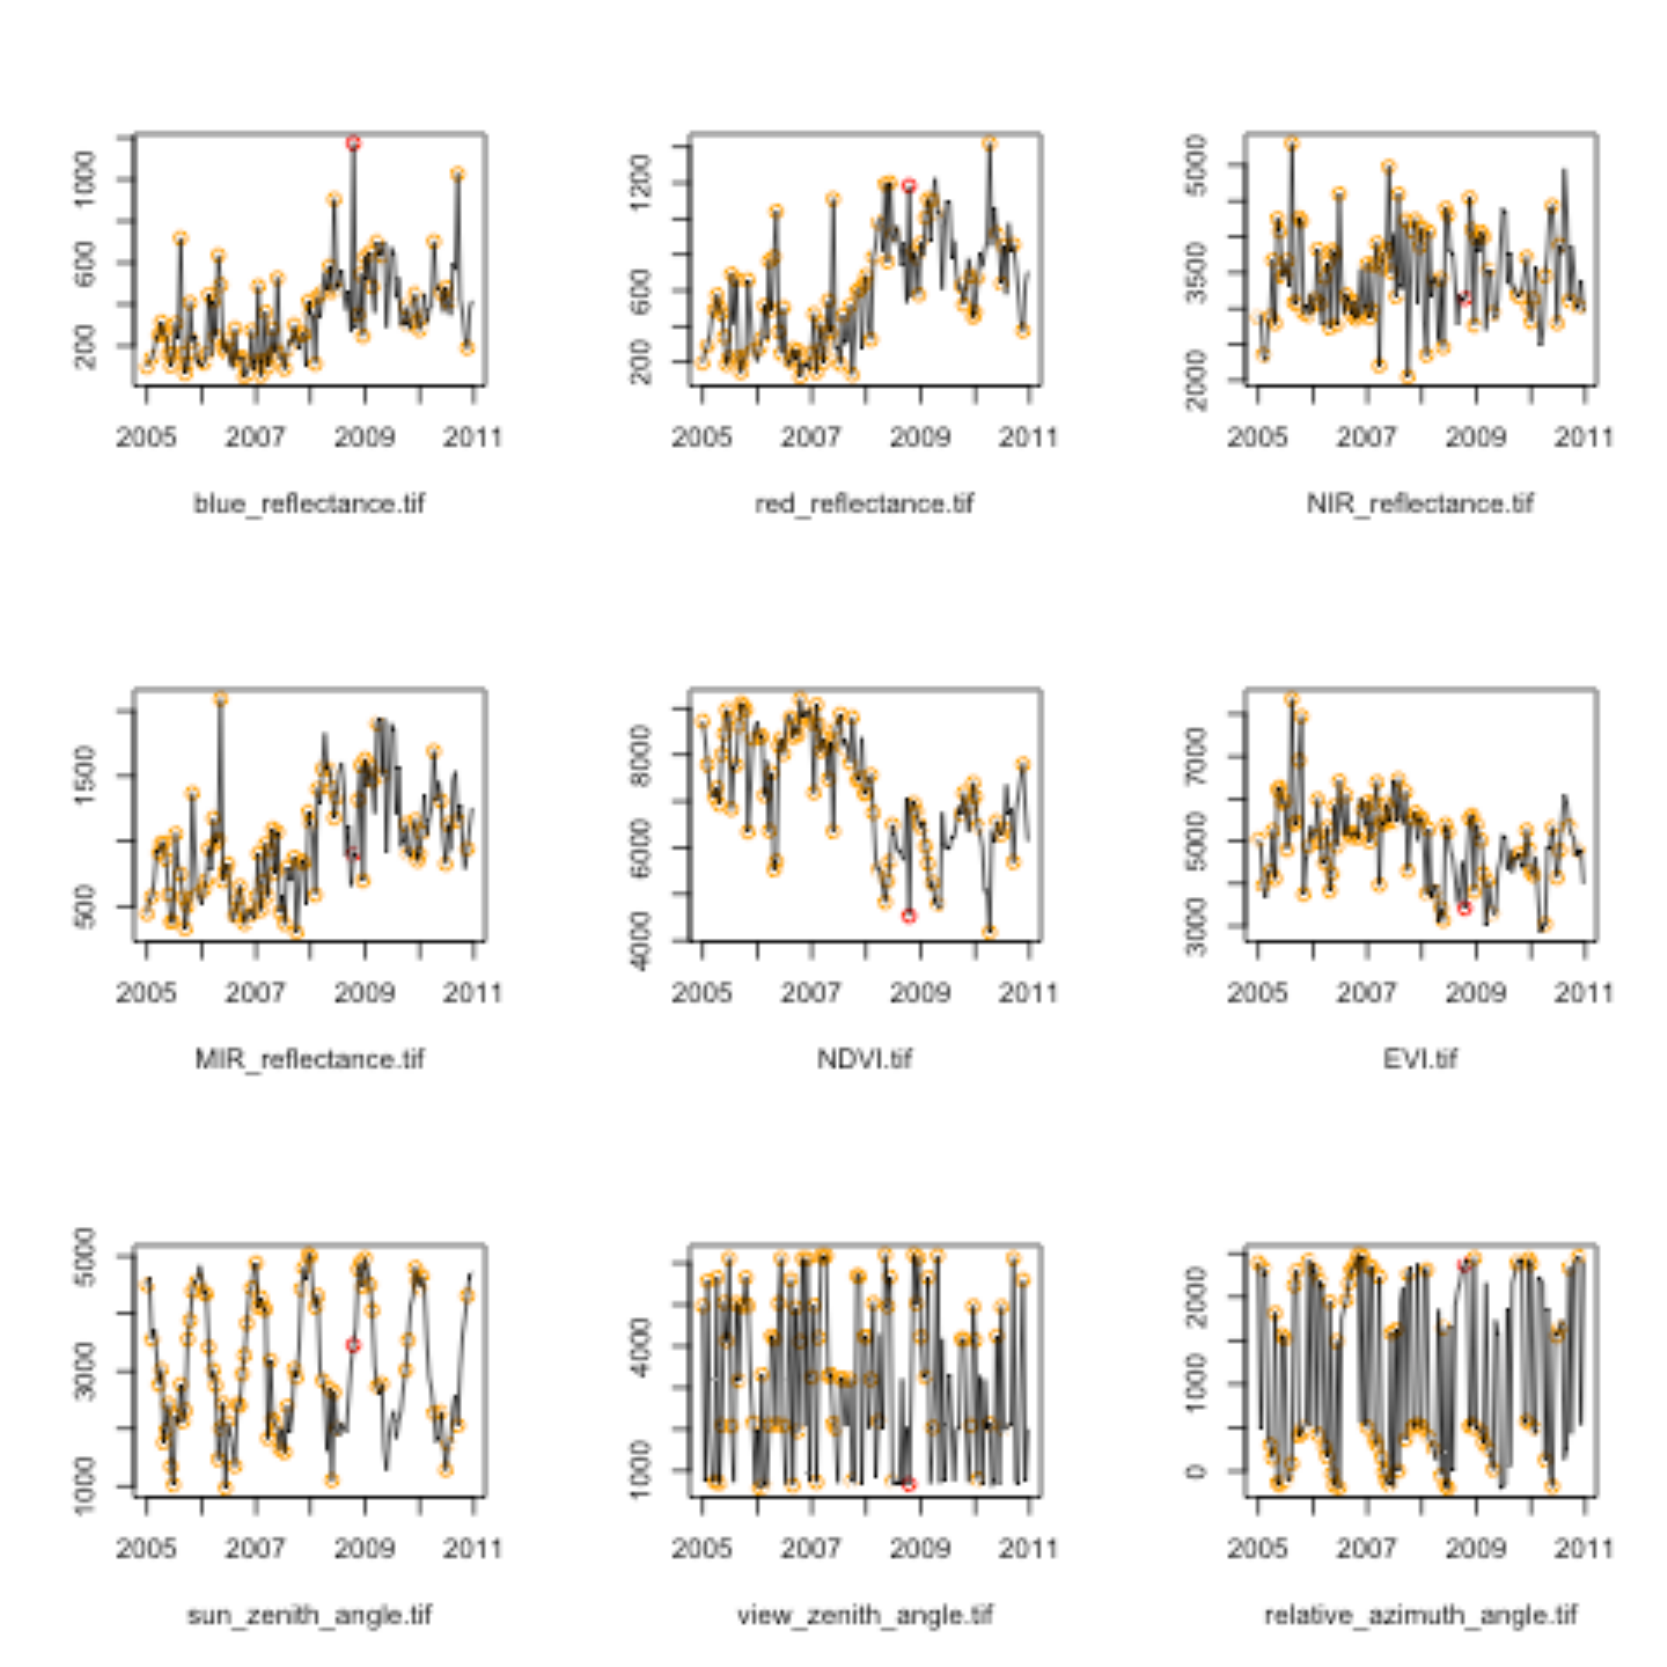} 
   	        \caption{deforested pixel}
   	        \label{fig:defo_pix}
   	      \end{subfigure}%
   	      \begin{subfigure}{.5\textwidth}
   	        \centering
   	        \includegraphics[width=1\textwidth]{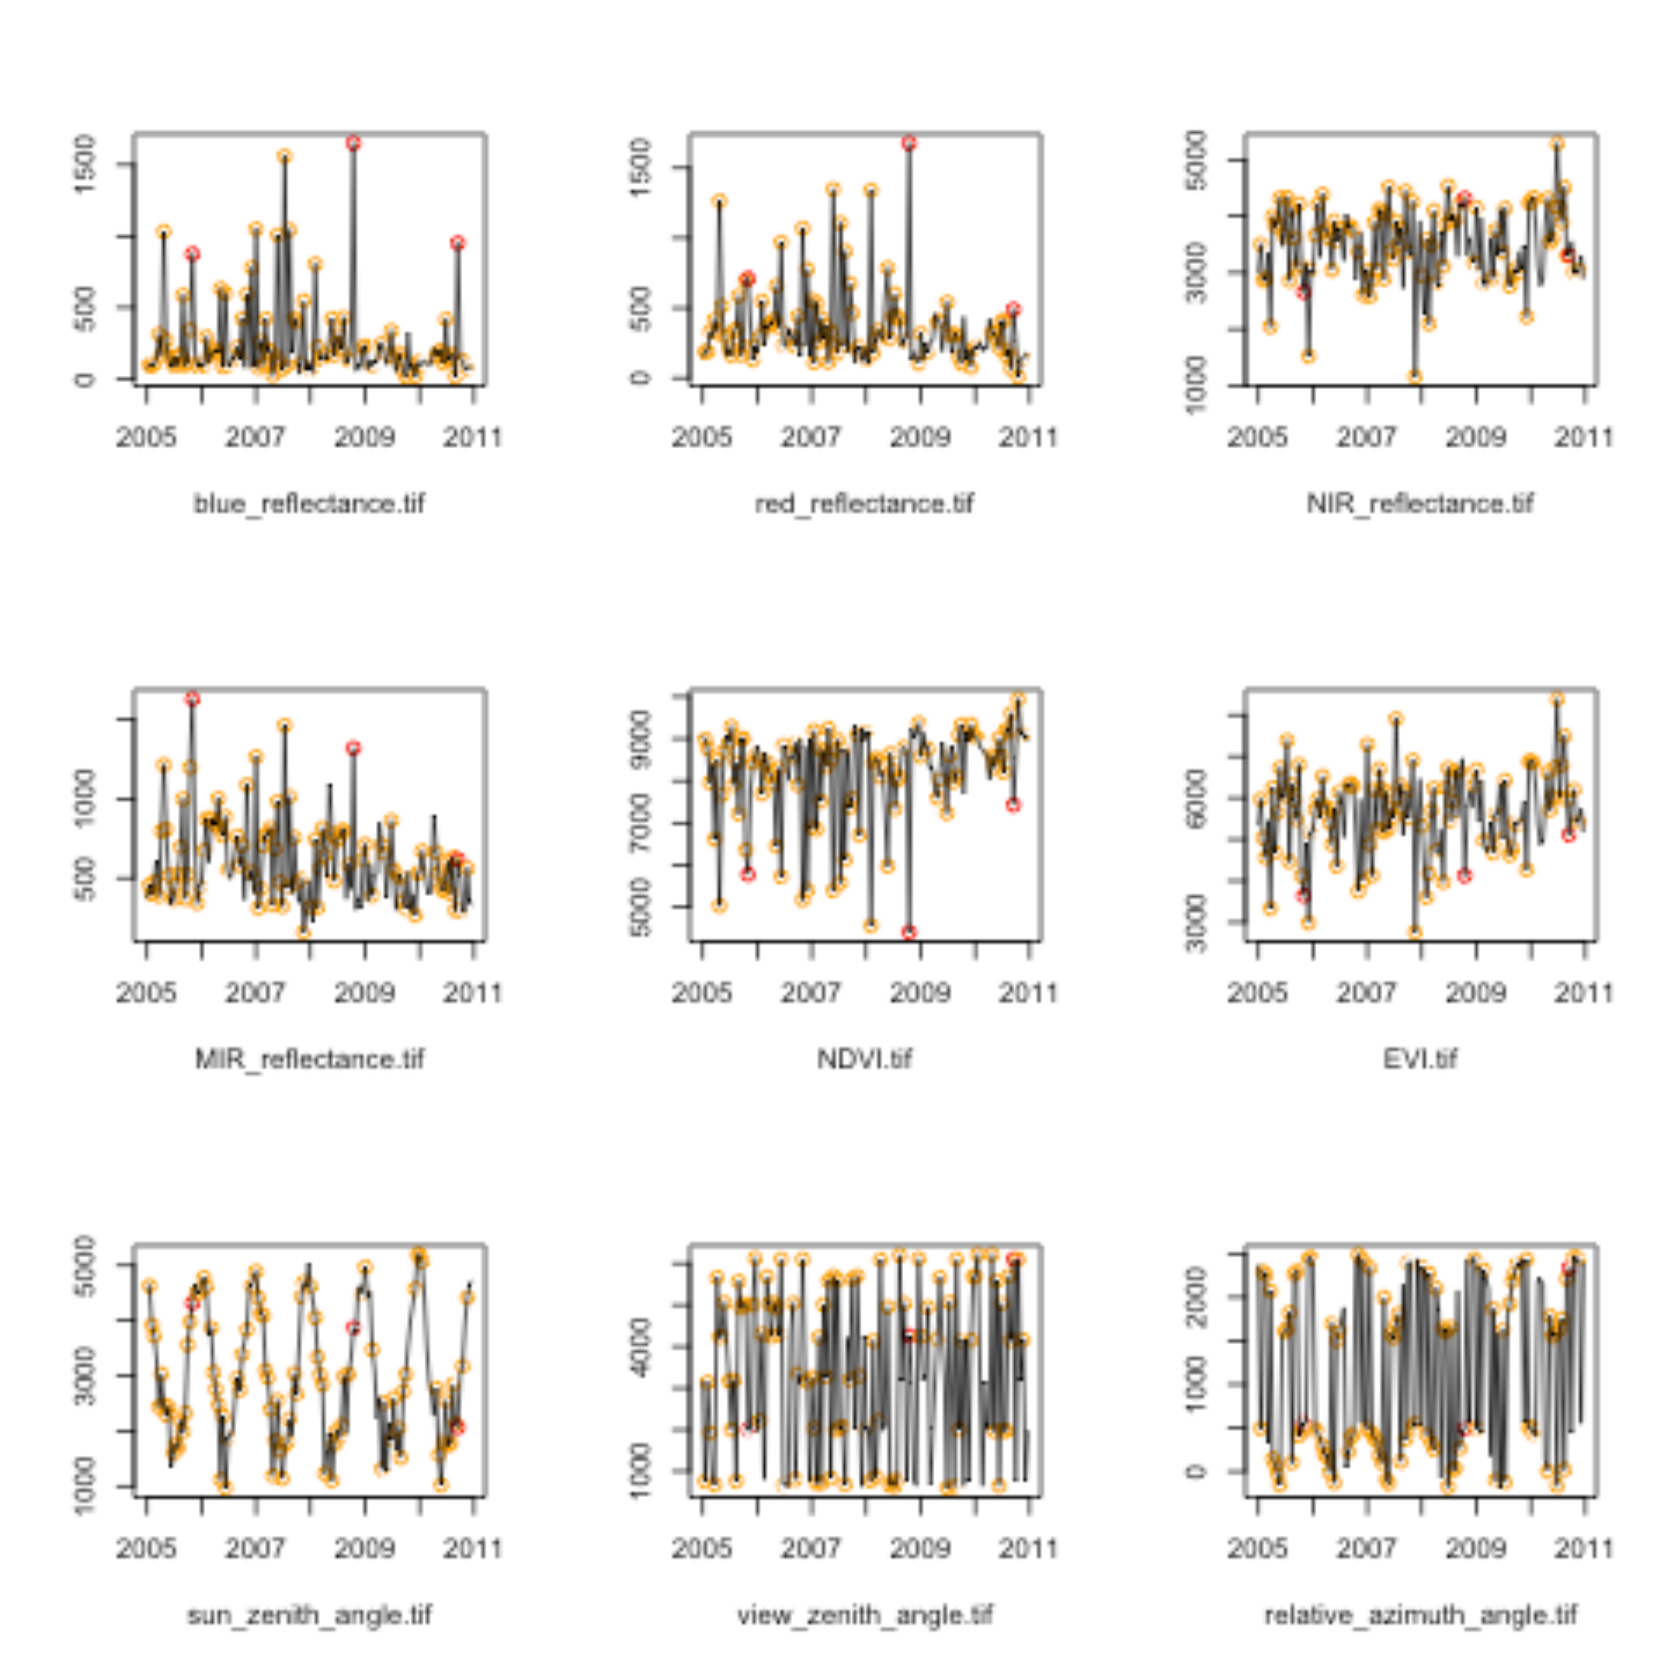}
   	        \caption{non-deforested pixel}
   	        \label{fig:non_defo_pix}
   	      \end{subfigure}
   	      %%         --- .5\textwidth stands for 50% of text width
   	      \caption[Reflectance, vegetation indices and sun-sensor geometry time series for deforested and non-deforested pixel in Yucatan 180 site.]%<<-- Legend for the list of figures at the beginning of you thesis
   	      {Reflectance, vegetation indices and sun-sensor geometry time series for deforested and non-deforested pixel in QuintanaRoo77 site, identified in figure \ref{fig:defoQuintanaRoo77} with green and red circles respectively. Orange marked points are \emph{marginal data} and red marked points are \emph{cloudy} or \emph{not processed}}% legend displayed below the graph.
   	      \label{fig:timeSeries}
   	    \end{figure}
		
		\subsubsection{Sonora74}
		
      	 \begin{figure}[H]  %--- Picture 'H'ere, 'B'ottom or 'T'op; '!' Try to
      	                     %impose your will to LaTeX
      	  % \centering 
  
      	   \begin{subfigure}{.5\textwidth}
      	     \centering
      	 	\includegraphics[width=0.7\textwidth]{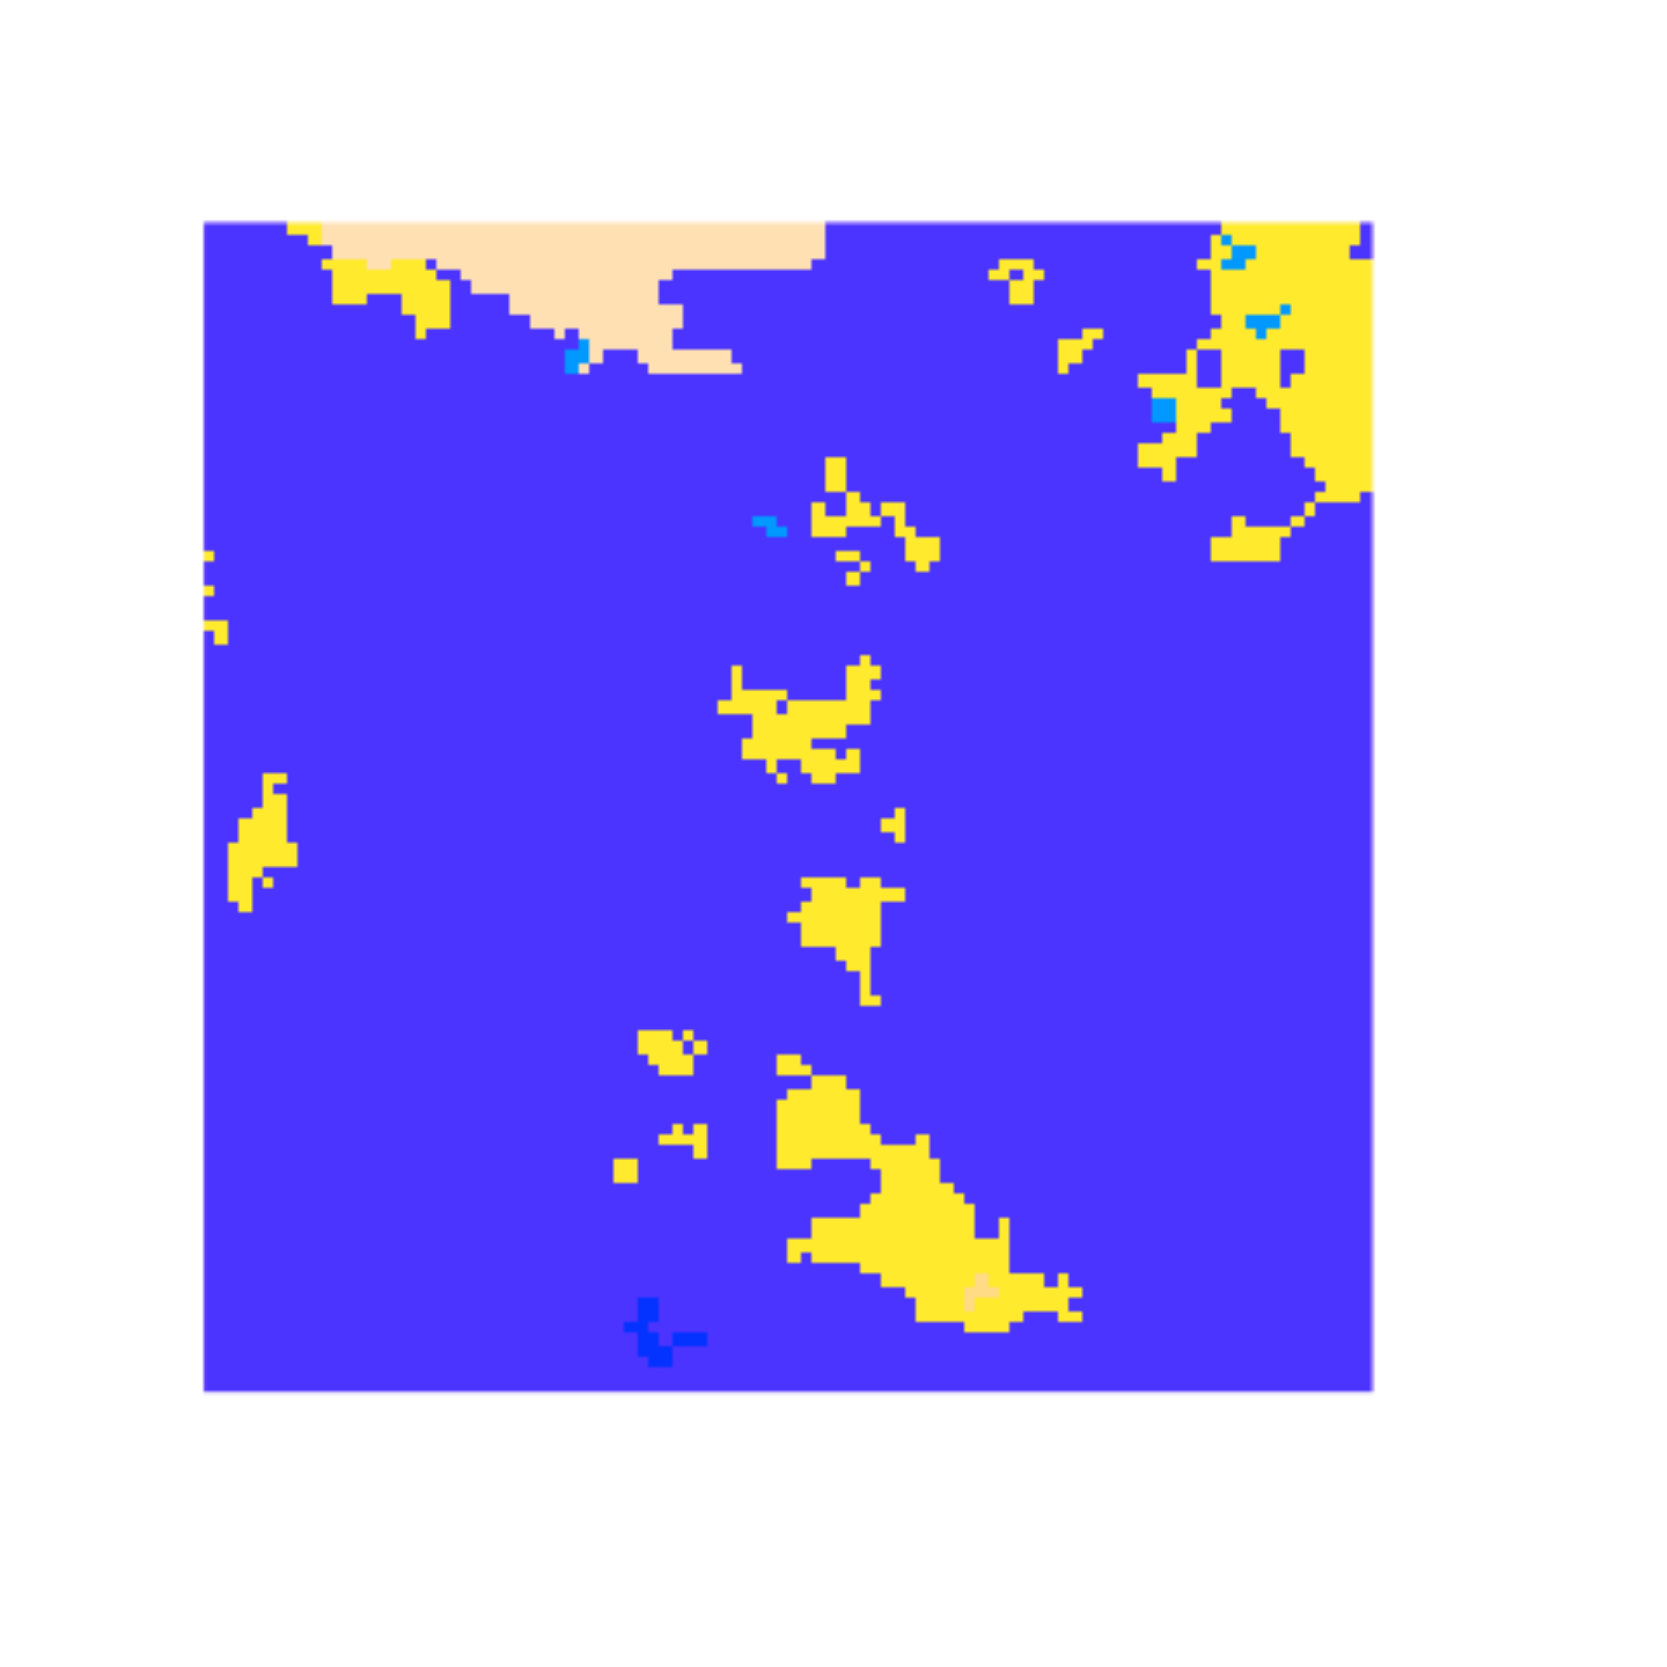} 
      	     \caption{Land-use 2005}
      	     \label{fig:sfig1a}
      	   \end{subfigure}%
      	   \begin{subfigure}{.5\textwidth}
      	     \centering
      	     \includegraphics[width=0.7\textwidth]{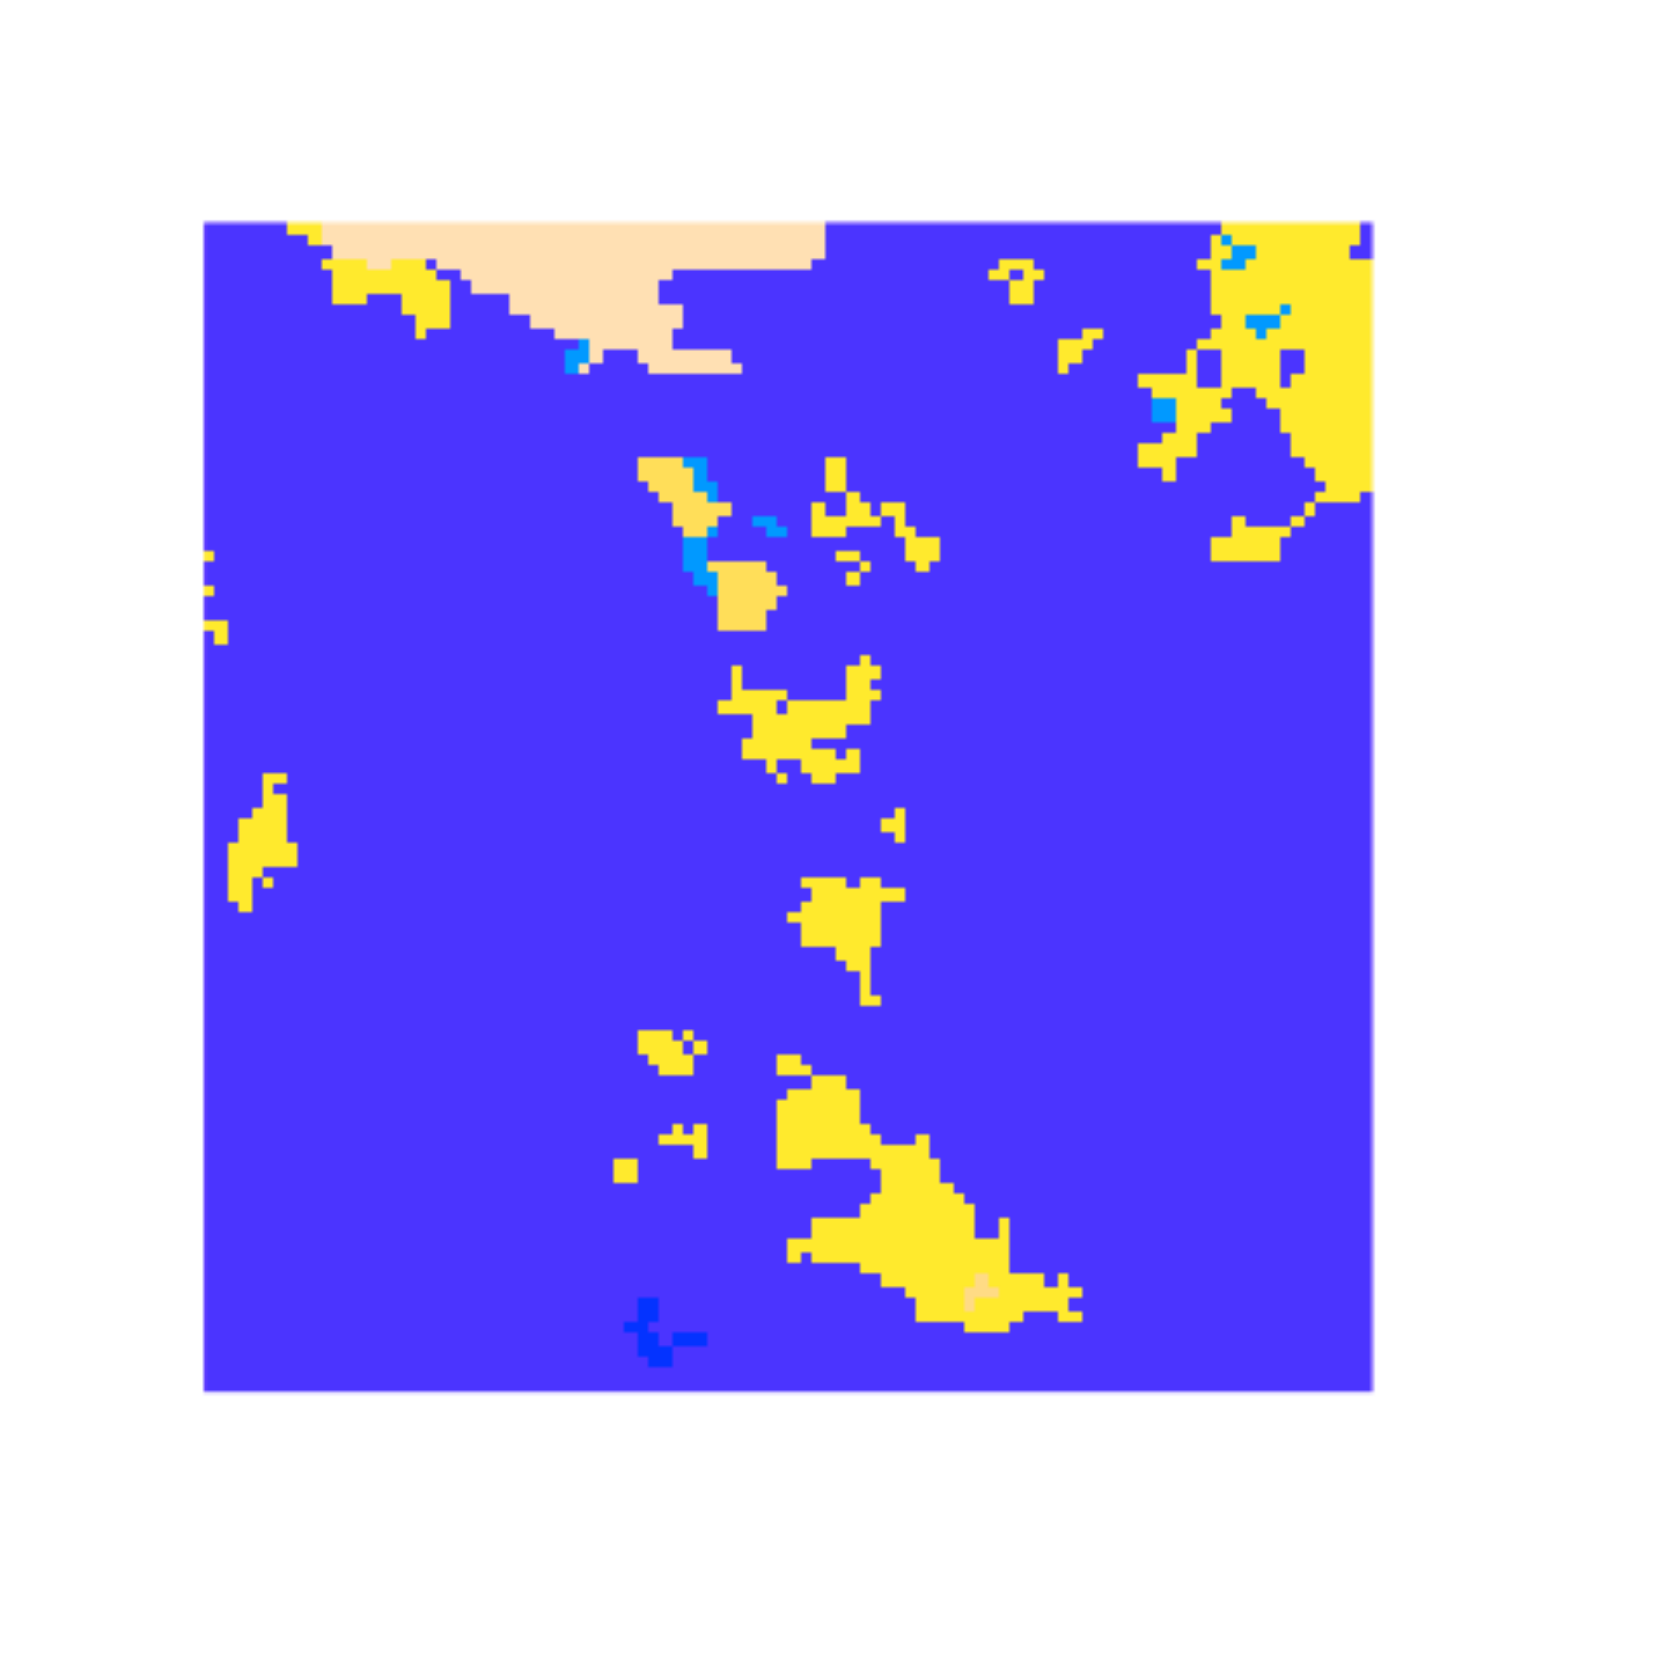}
      	     \caption{Land-use 2010}
      	     \label{fig:sfig1b}
      	   \end{subfigure}
      	   \begin{subfigure}{.4\textwidth}
      	     \centering
      	     \includegraphics[width=0.9\textwidth]{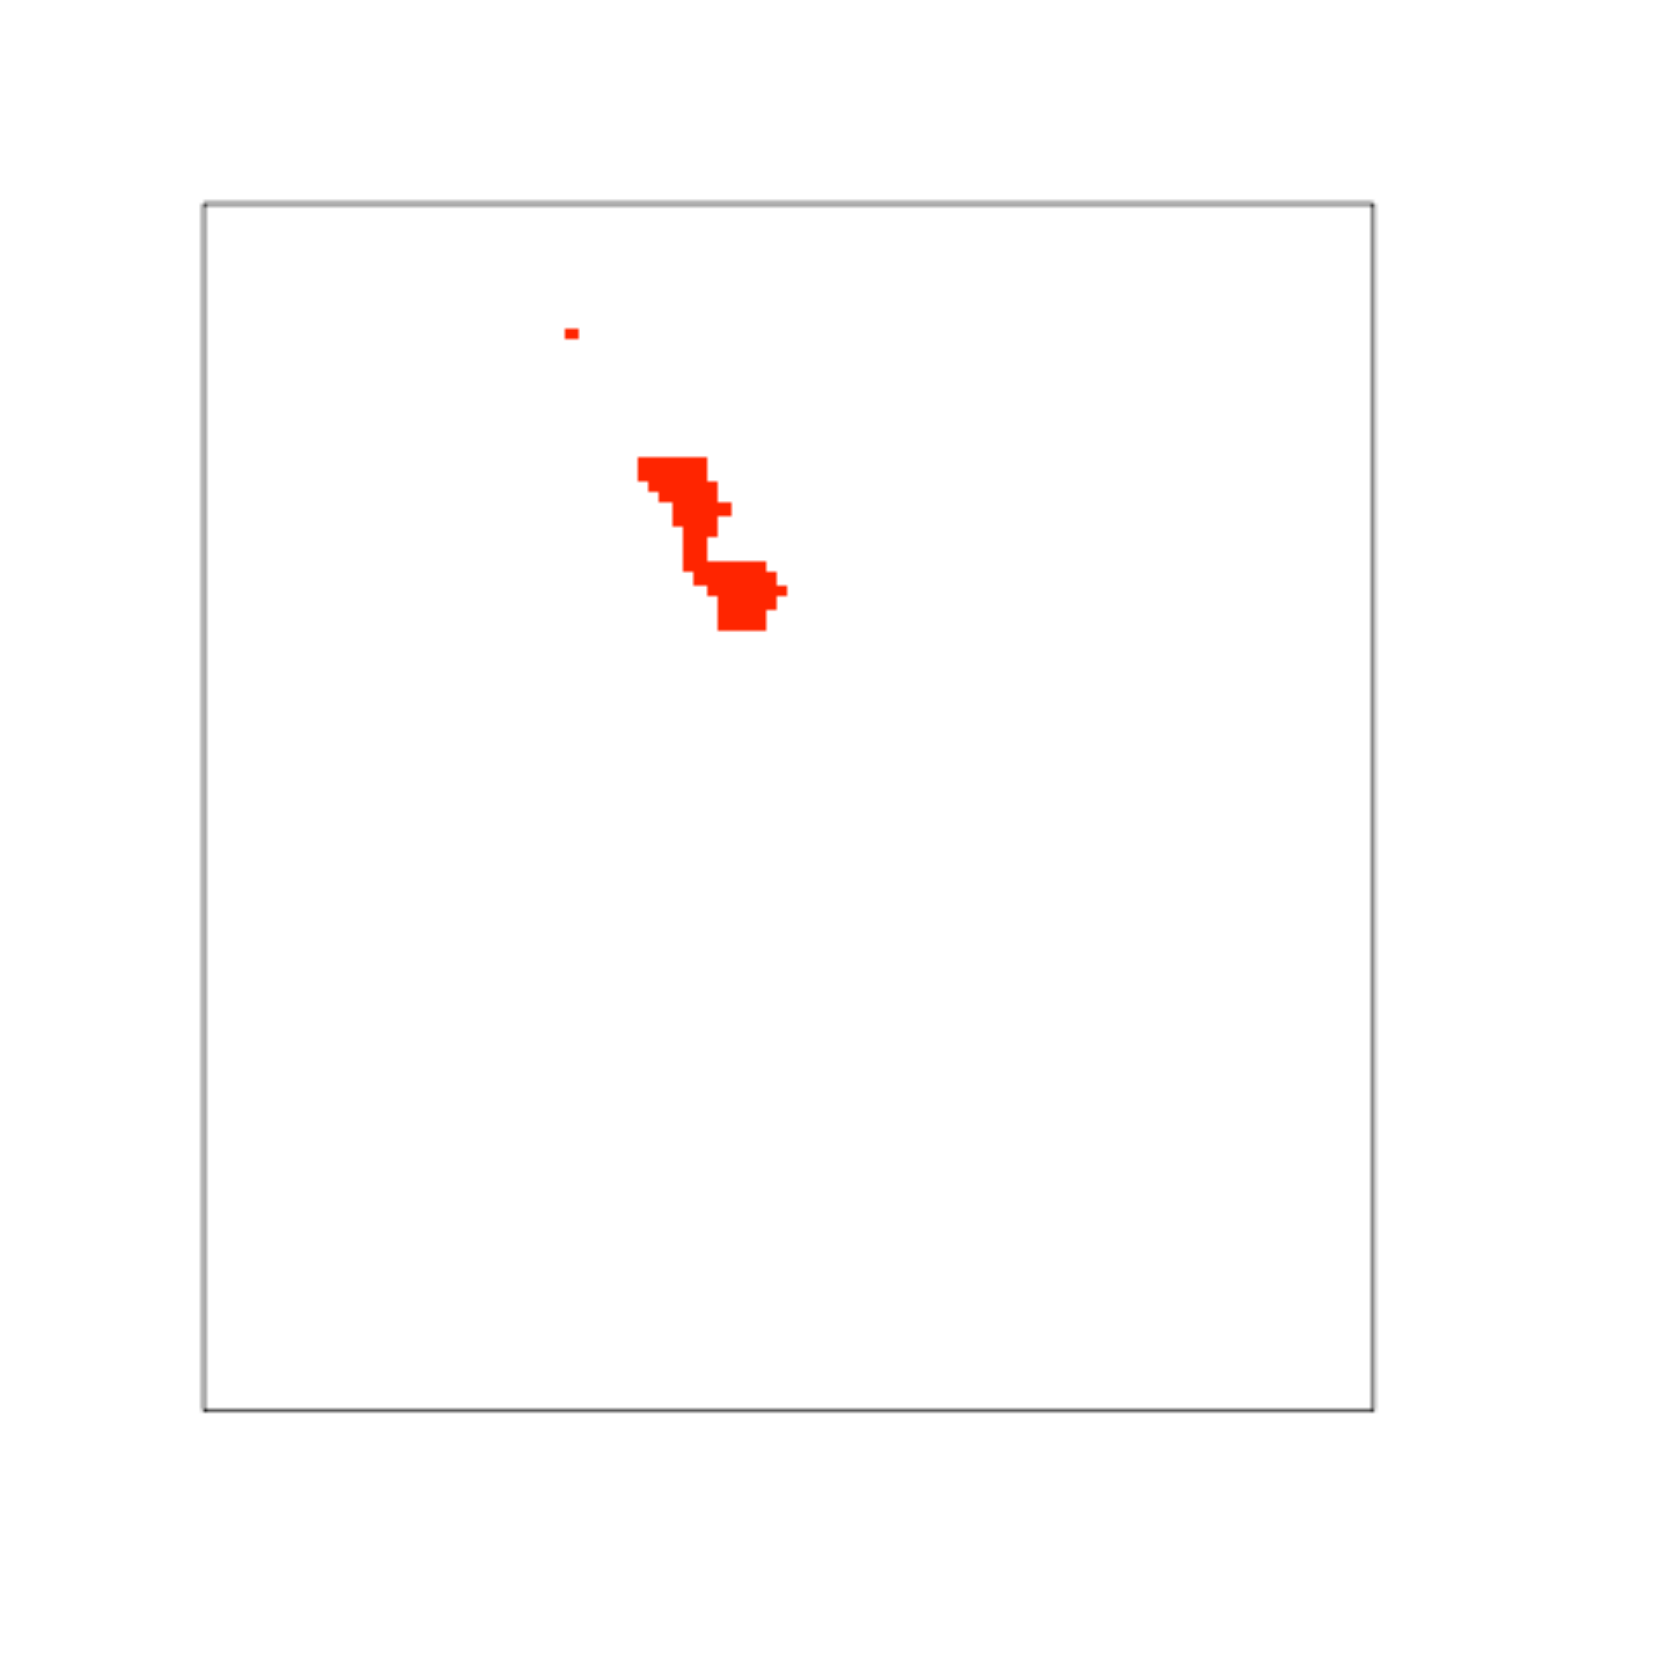}
      	     \caption{Deforestation 2005-2010}
      	     \label{fig:sfig1c}
      	   \end{subfigure}
      	   \begin{subfigure}{.4\textwidth}
      	     \centering
      	     \includegraphics[width=0.9\textwidth]{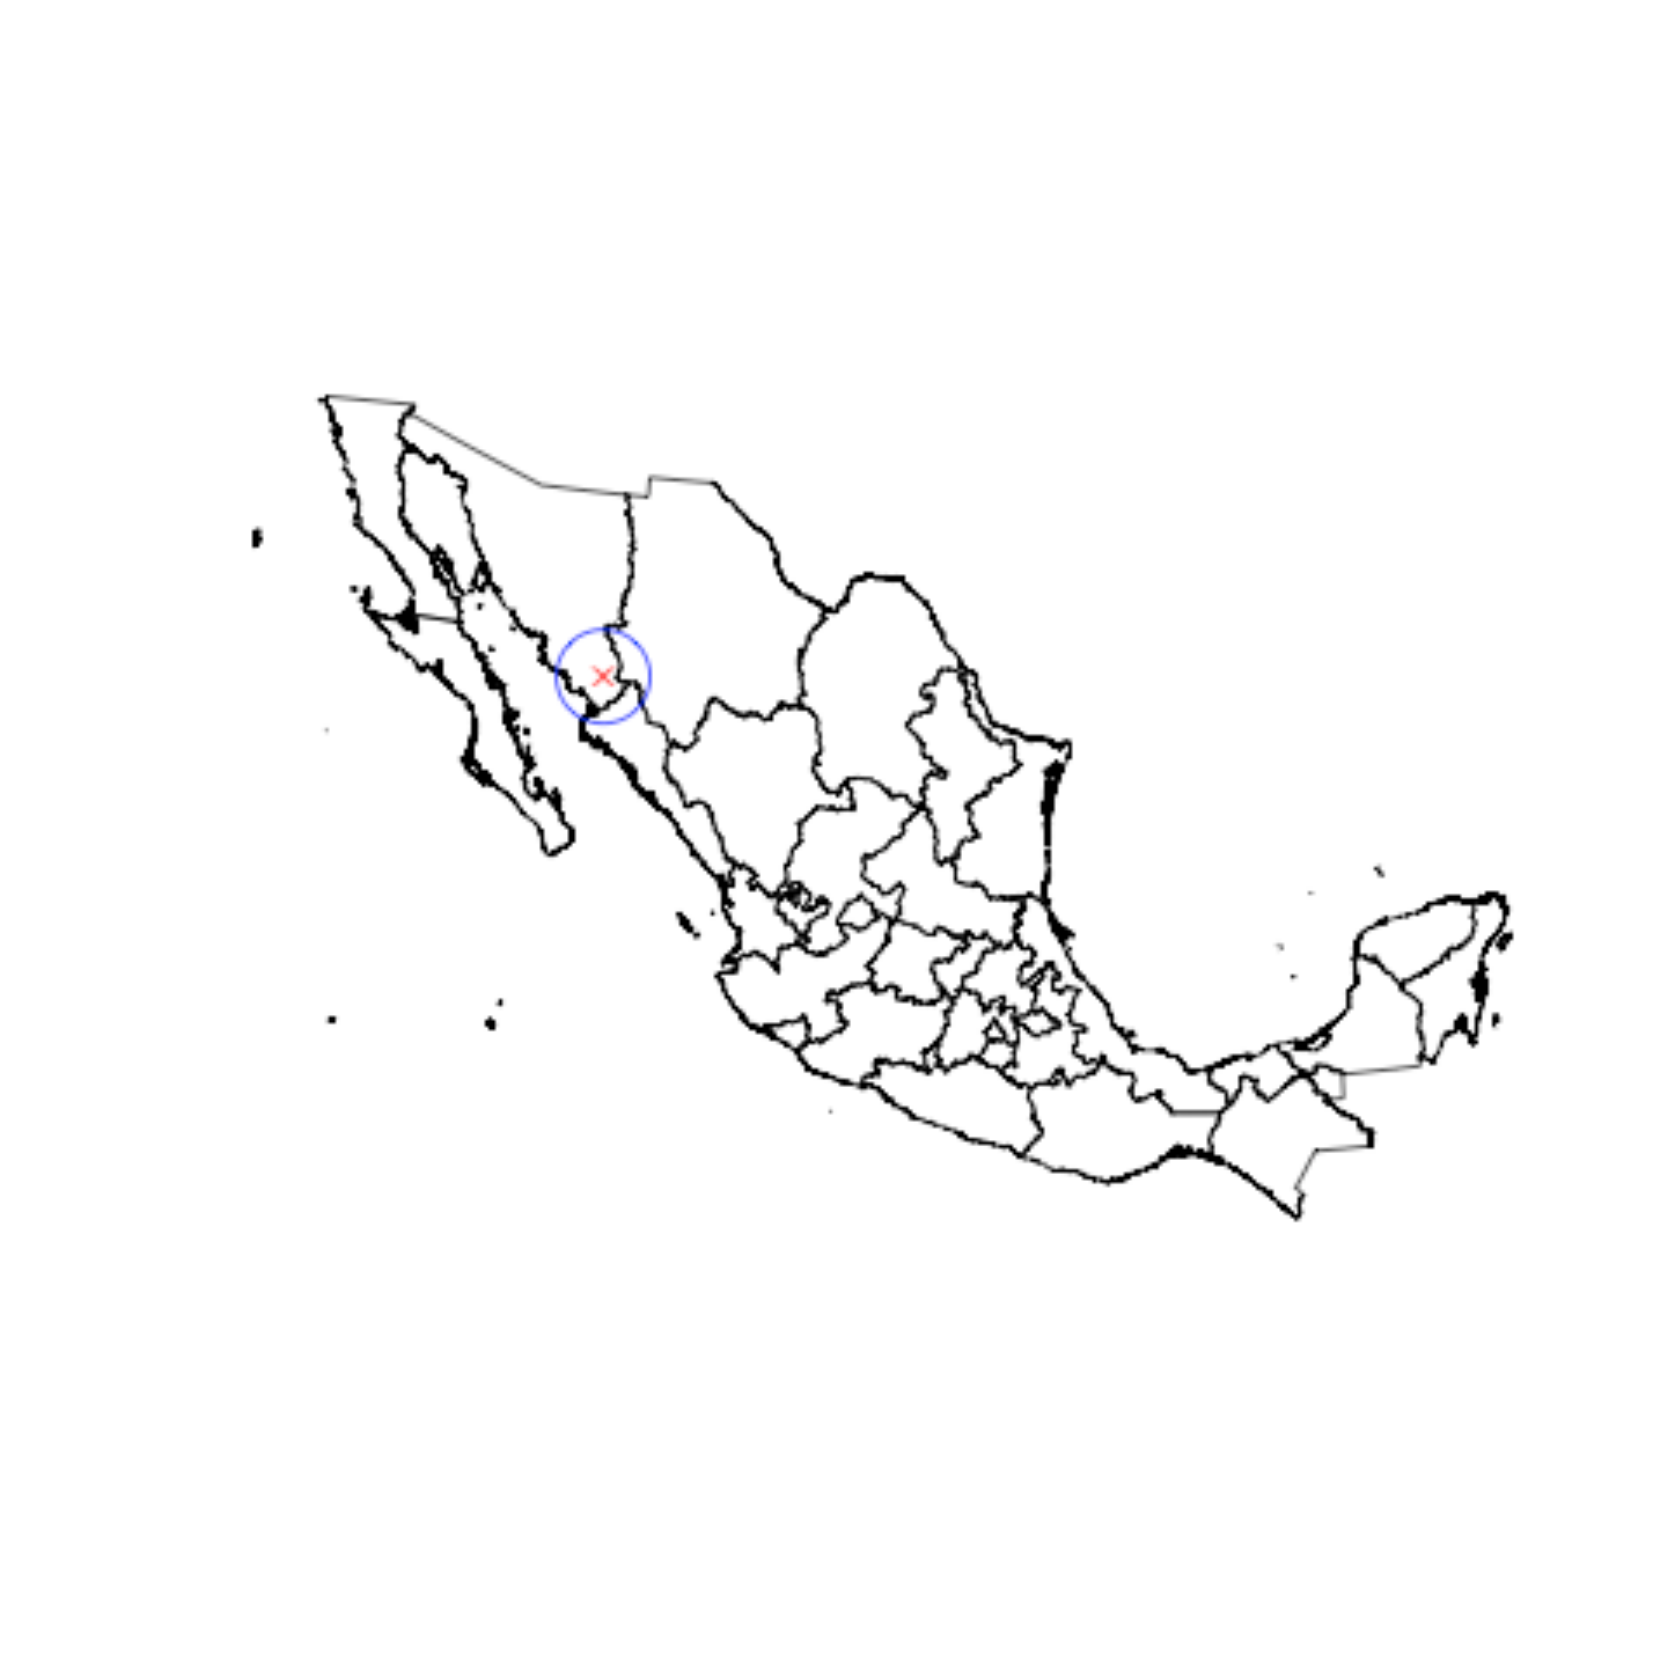}
      	     \caption{Location}
      	     \label{fig:sfig1d}
      	   \end{subfigure}   
         \begin{subfigure}{.5\textwidth}
           \centering
           \includegraphics[width=1\textwidth]{./2_Data/legend_landUse}
           \caption{Land use legend}
           \label{fig:legend}
         \end{subfigure}
      	   %%         --- .5\textwidth stands for 50% of text width
      	   \caption[NALCMS land-use classification of Sonora74 site, 2005 and 2010 at 250m resolution.]%<<-- Legend for the list of figures at the beginning of you thesis
      	   {NALCMS land-use classification of Sonora74 site, 2005 and 2010 at 250m resolution.}% legend displayed below the graph.
      	   \label{fig:landUseSonora74}
      	 \end{figure}
		
   		\begin{center}
   			\footnotesize\addtolength{\tabcolsep}{-2pt}
   			% latex table generated in R 3.3.1 by xtable 1.8-2 package
% Sun Mar  5 16:03:51 2017
\begin{table}[ht]
\centering
\begingroup\tiny
\begin{tabular}{rrrrrrrrrrrrrrrrrrrrr}
  & \begin{sideways} Temperate or sub-polar needleleaf forest \end{sideways} & \begin{sideways} Sub-polar taiga needleleaf forest \end{sideways} & \begin{sideways} Tropical or sub-tropical broadleaf evergreen forest \end{sideways} & \begin{sideways} Tropical or sub-tropical broadleaf deciduous forest \end{sideways} & \begin{sideways} Temperate or sub-polar broadleaf deciduous forest \end{sideways} & \begin{sideways} Mixed Forest \end{sideways} & \begin{sideways} Tropical or sub-tropical shrubland \end{sideways} & \begin{sideways} Temperate or sub-polar shrubland \end{sideways} & \begin{sideways} Tropical or sub-tropical grassland \end{sideways} & \begin{sideways} Temperate or sub-polar grassland \end{sideways} & \begin{sideways} Sub-polar or polar shrubland-lichen-moss \end{sideways} & \begin{sideways} Sub-polar or polar grassland-lichen-moss \end{sideways} & \begin{sideways} Sub-polar or polar barren-lichen-moss \end{sideways} & \begin{sideways} Wetland \end{sideways} & \begin{sideways} Cropland \end{sideways} & \begin{sideways} Barren Lands \end{sideways} & \begin{sideways} Urban and Built-up \end{sideways} & \begin{sideways} Water \end{sideways} & \begin{sideways} Snow and Ice \end{sideways} & \begin{sideways} Total \end{sideways} \\ 
  \hline
Temperate or sub-polar needleleaf forest &    0 &    0 &    0 &    0 &    0 &    0 &    0 &    0 &    0 &    0 &    0 &    0 &    0 &    0 &    0 &    0 &    0 &    0 &    0 &    0 \\ 
  Sub-polar taiga needleleaf forest &    0 &    0 &    0 &    0 &    0 &    0 &    0 &    0 &    0 &    0 &    0 &    0 &    0 &    0 &    0 &    0 &    0 &    0 &    0 &    0 \\ 
  Tropical or sub-tropical broadleaf evergreen forest &    0 &    0 &    0 &    0 &    0 &    0 &    0 &    0 &    0 &    0 &    0 &    0 &    0 &    0 &    0 &    0 &    0 &    0 &    0 &    0 \\ 
  Tropical or sub-tropical broadleaf deciduous forest &    0 &    0 &    0 & 8788 &    0 &    0 &   16 &    0 &    0 &    0 &    0 &    0 &    0 &    0 &    0 &   57 &    0 &    1 &    0 & 8862 \\ 
  Temperate or sub-polar broadleaf deciduous forest &    0 &    0 &    0 &    0 &   16 &    0 &    0 &    0 &    0 &    0 &    0 &    0 &    0 &    0 &    0 &    0 &    0 &    0 &    0 &   16 \\ 
  Mixed Forest &    0 &    0 &    0 &    0 &    0 &    0 &    0 &    0 &    0 &    0 &    0 &    0 &    0 &    0 &    0 &    0 &    0 &    0 &    0 &    0 \\ 
   \hline
Tropical or sub-tropical shrubland &    0 &    0 &    0 &    0 &    0 &    0 &   22 &    0 &    0 &    0 &    0 &    0 &    0 &    0 &    0 &    0 &    0 &    0 &    0 &   22 \\ 
  Temperate or sub-polar shrubland &    0 &    0 &    0 &    0 &    0 &    0 &    0 &    0 &    0 &    0 &    0 &    0 &    0 &    0 &    0 &    0 &    0 &    0 &    0 &    0 \\ 
  Tropical or sub-tropical grassland &    0 &    0 &    0 &    0 &    0 &    0 &    0 &    0 &    0 &    0 &    0 &    0 &    0 &    0 &    0 &    0 &    0 &    0 &    0 &    0 \\ 
  Temperate or sub-polar grassland &    0 &    0 &    0 &    0 &    0 &    0 &    0 &    0 &    0 &    0 &    0 &    0 &    0 &    0 &    0 &    0 &    0 &    0 &    0 &    0 \\ 
  Sub-polar or polar shrubland-lichen-moss &    0 &    0 &    0 &    0 &    0 &    0 &    0 &    0 &    0 &    0 &    0 &    0 &    0 &    0 &    0 &    0 &    0 &    0 &    0 &    0 \\ 
  Sub-polar or polar grassland-lichen-moss &    0 &    0 &    0 &    0 &    0 &    0 &    0 &    0 &    0 &    0 &    0 &    0 &    0 &    0 &    0 &    0 &    0 &    0 &    0 &    0 \\ 
  Sub-polar or polar barren-lichen-moss &    0 &    0 &    0 &    0 &    0 &    0 &    0 &    0 &    0 &    0 &    0 &    0 &    0 &    0 &    0 &    0 &    0 &    0 &    0 &    0 \\ 
  Wetland &    0 &    0 &    0 &    0 &    0 &    0 &    0 &    0 &    0 &    0 &    0 &    0 &    0 &    0 &    0 &    0 &    0 &    0 &    0 &    0 \\ 
  Cropland &    0 &    0 &    0 &    0 &    0 &    0 &    0 &    0 &    0 &    0 &    0 &    0 &    0 &    0 &  824 &    0 &    0 &    0 &    0 &  824 \\ 
  Barren Lands &    0 &    0 &    0 &    0 &    0 &    0 &    0 &    0 &    0 &    0 &    0 &    0 &    0 &    0 &    0 &    0 &    0 &    0 &    0 &    0 \\ 
  Urban and Built-up &    0 &    0 &    0 &    0 &    0 &    0 &    0 &    0 &    0 &    0 &    0 &    0 &    0 &    0 &    0 &    0 &    5 &    0 &    0 &    5 \\ 
  Water &    0 &    0 &    0 &    0 &    0 &    0 &    0 &    0 &    0 &    0 &    0 &    0 &    0 &    0 &    0 &    0 &    0 &  271 &    0 &  271 \\ 
  Snow and Ice &    0 &    0 &    0 &    0 &    0 &    0 &    0 &    0 &    0 &    0 &    0 &    0 &    0 &    0 &    0 &    0 &    0 &    0 &    0 &    0 \\ 
   \hline
Total &    0 &    0 &    0 & 8788 &   16 &    0 &   38 &    0 &    0 &    0 &    0 &    0 &    0 &    0 &  824 &   57 &    5 &  272 &    0 & 10000 \\ 
   \hline
\end{tabular}
\endgroup
\caption[NALCMS land-use distribution for site Sonora74, 2005 and 2010.]{NALCMS land-use distribution for site Sonora74, 2005 and 2010.} 
\end{table}

   			\label{tab:landUseSonora}
   		\end{center}
		
   		\begin{figure}[H]%--- Picture 'H'ere, 'B'ottom or 'T'op; '!' Try to
   		                    %impose your will to LaTeX
   		  \centering
   		  \includegraphics[width=.5\textwidth]{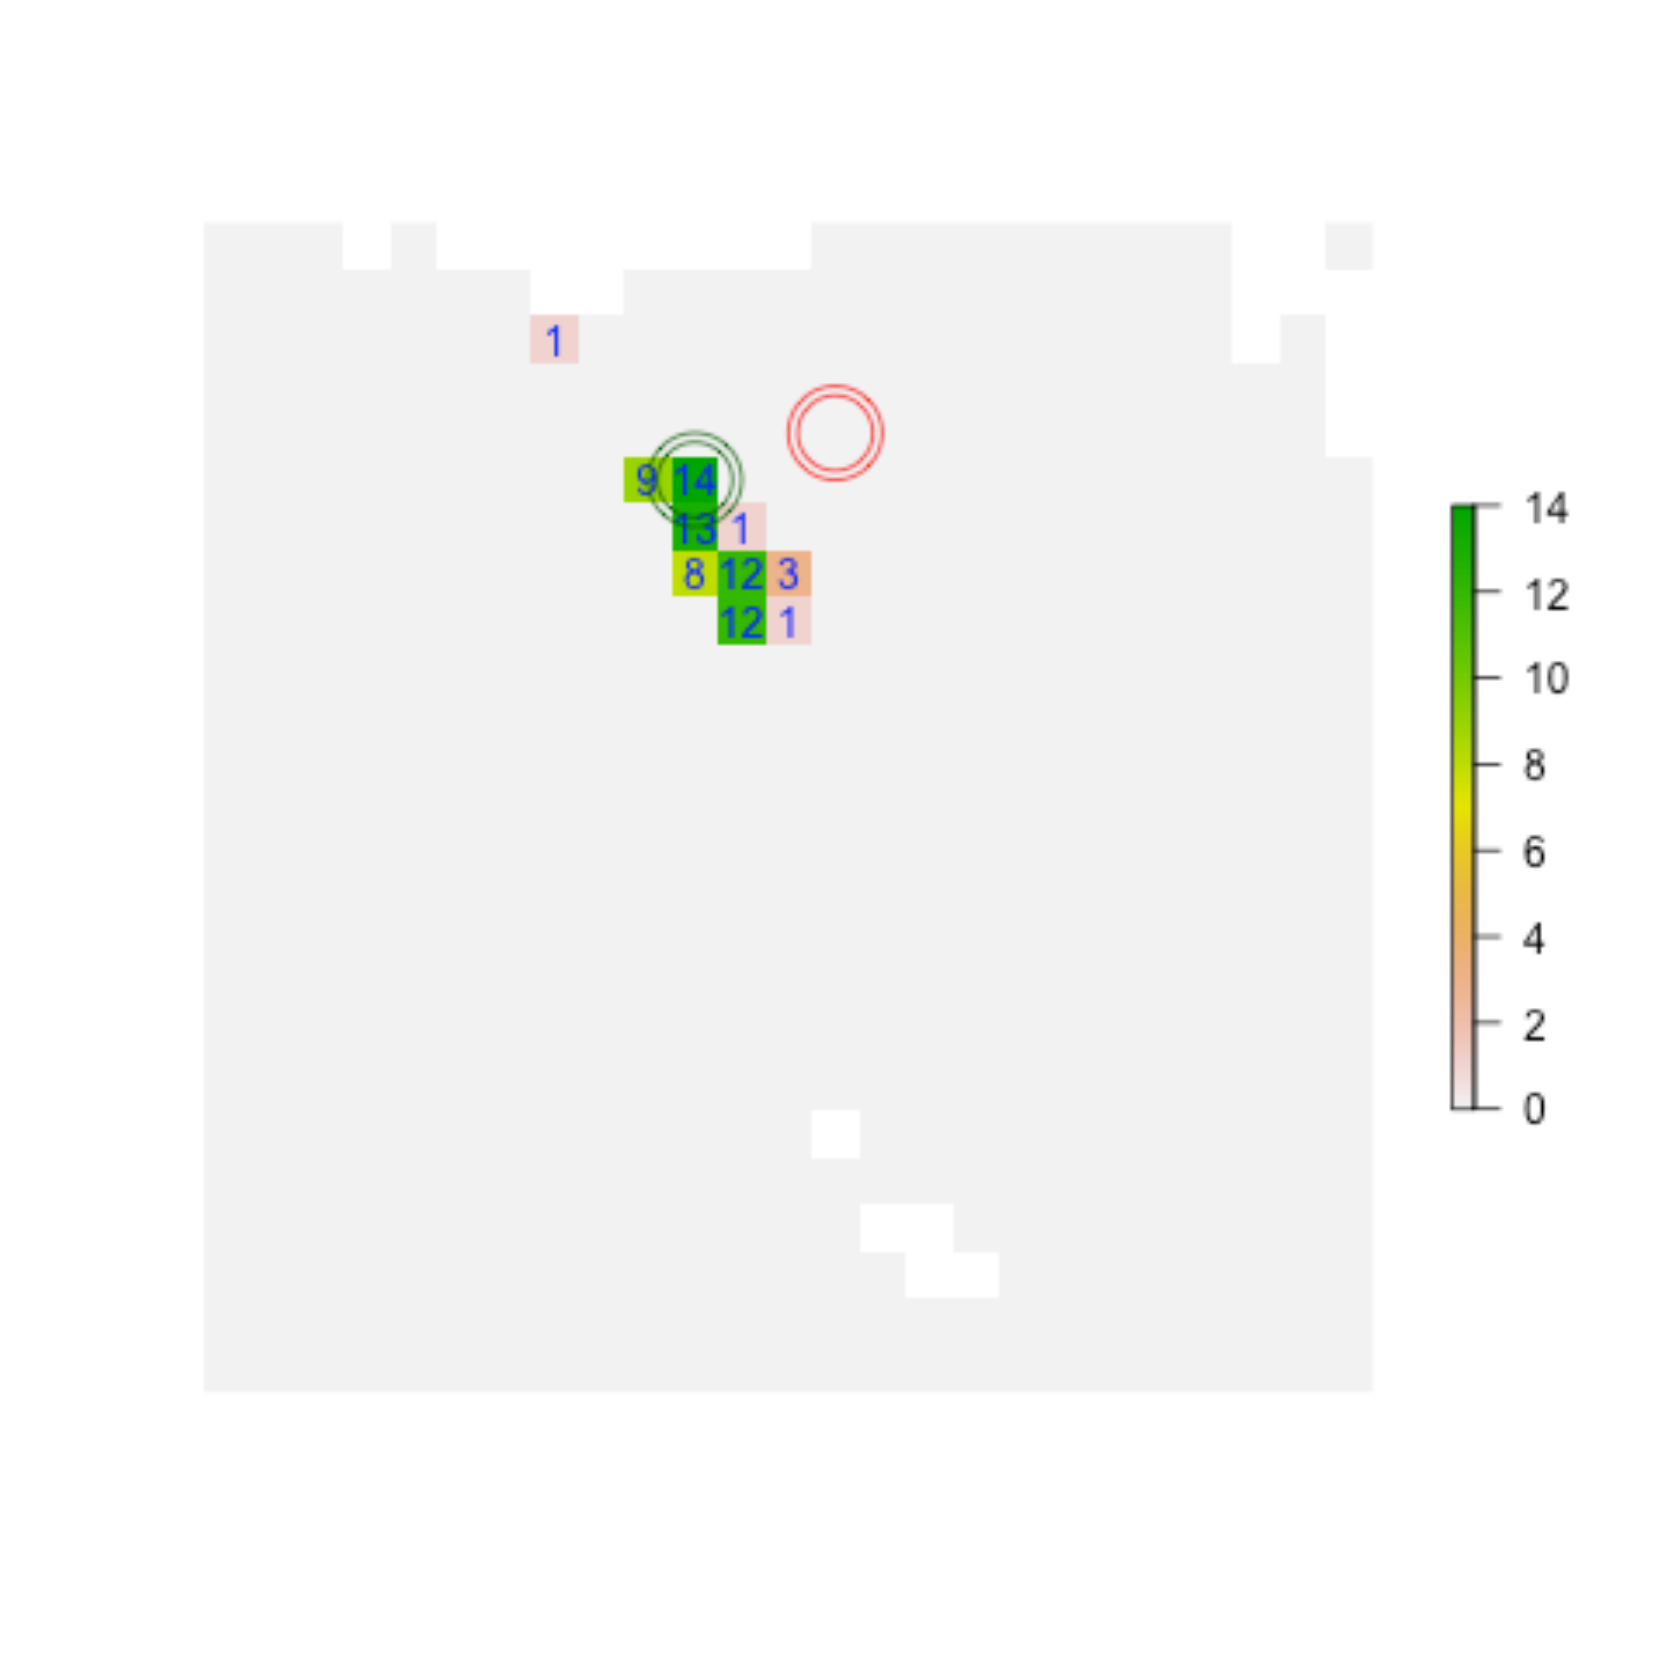} %<< no file extension
   		  %%         --- .5\textwidth stands for 50% of text width
   		  \caption[Deforestation in Sonora74 site at 1km resolution]%<<-- Legend for the list of figures at the beginning of you thesis
   		  {Deforestation in Sonora74 site at 1km resolution: number of 250m pixels deforested out of 16}% legend displayed below the graph.
   		  \label{fig:defoSonora74}
   		\end{figure}
		
   		 \begin{figure}[H]
   	      \begin{subfigure}{.5\textwidth}
   	        \centering
   	    	\includegraphics[width=1\textwidth]{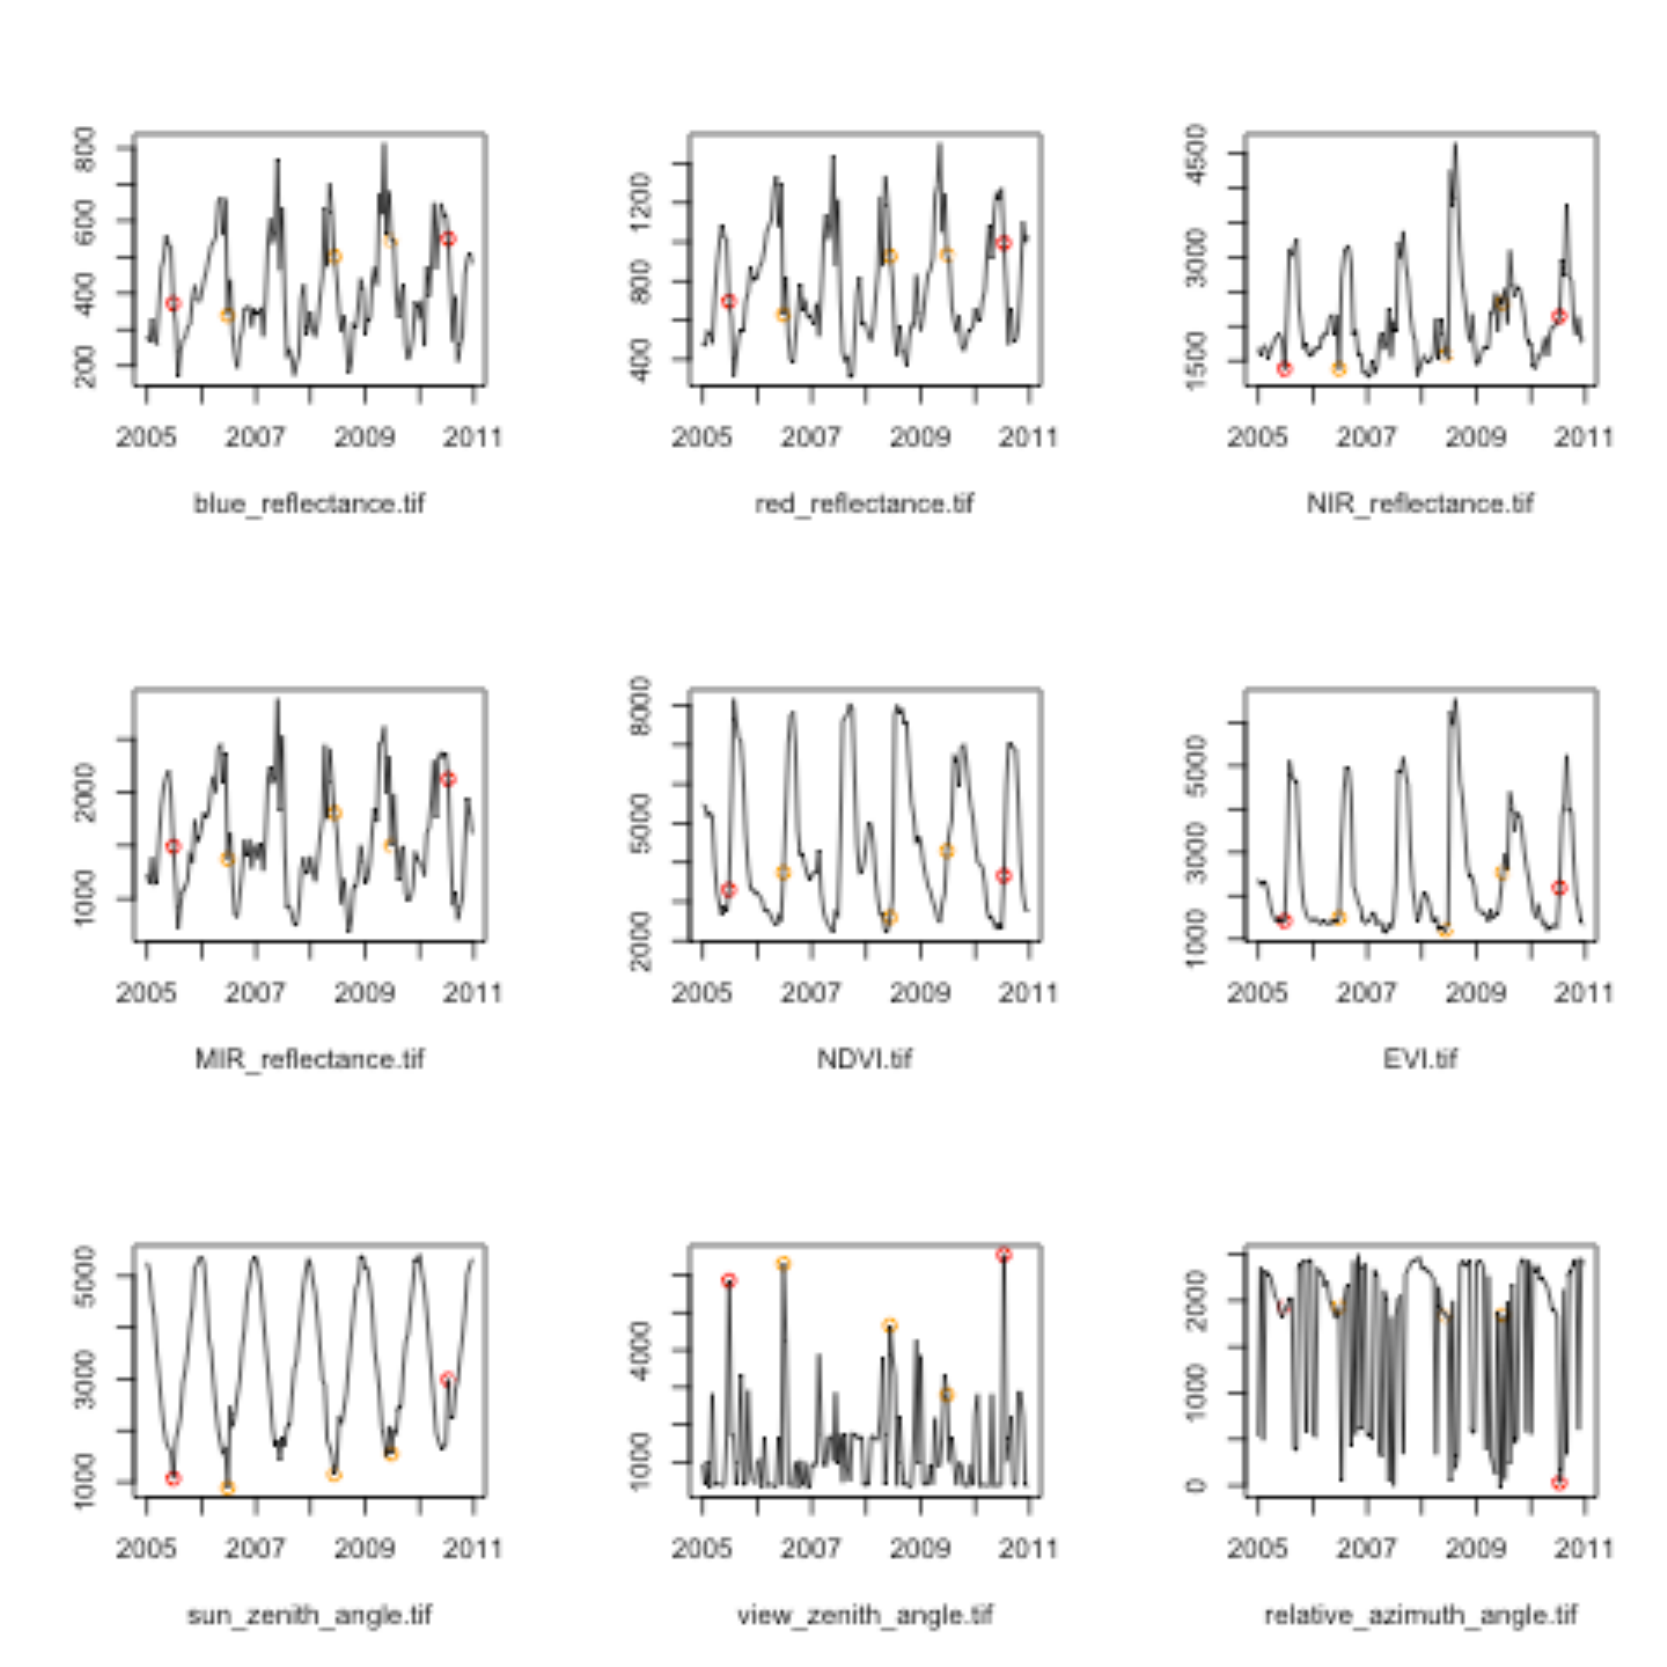} 
   	        \caption{deforested pixel}
   	        \label{fig:defo_pix}
   	      \end{subfigure}%
   	      \begin{subfigure}{.5\textwidth}
   	        \centering
   	        \includegraphics[width=1\textwidth]{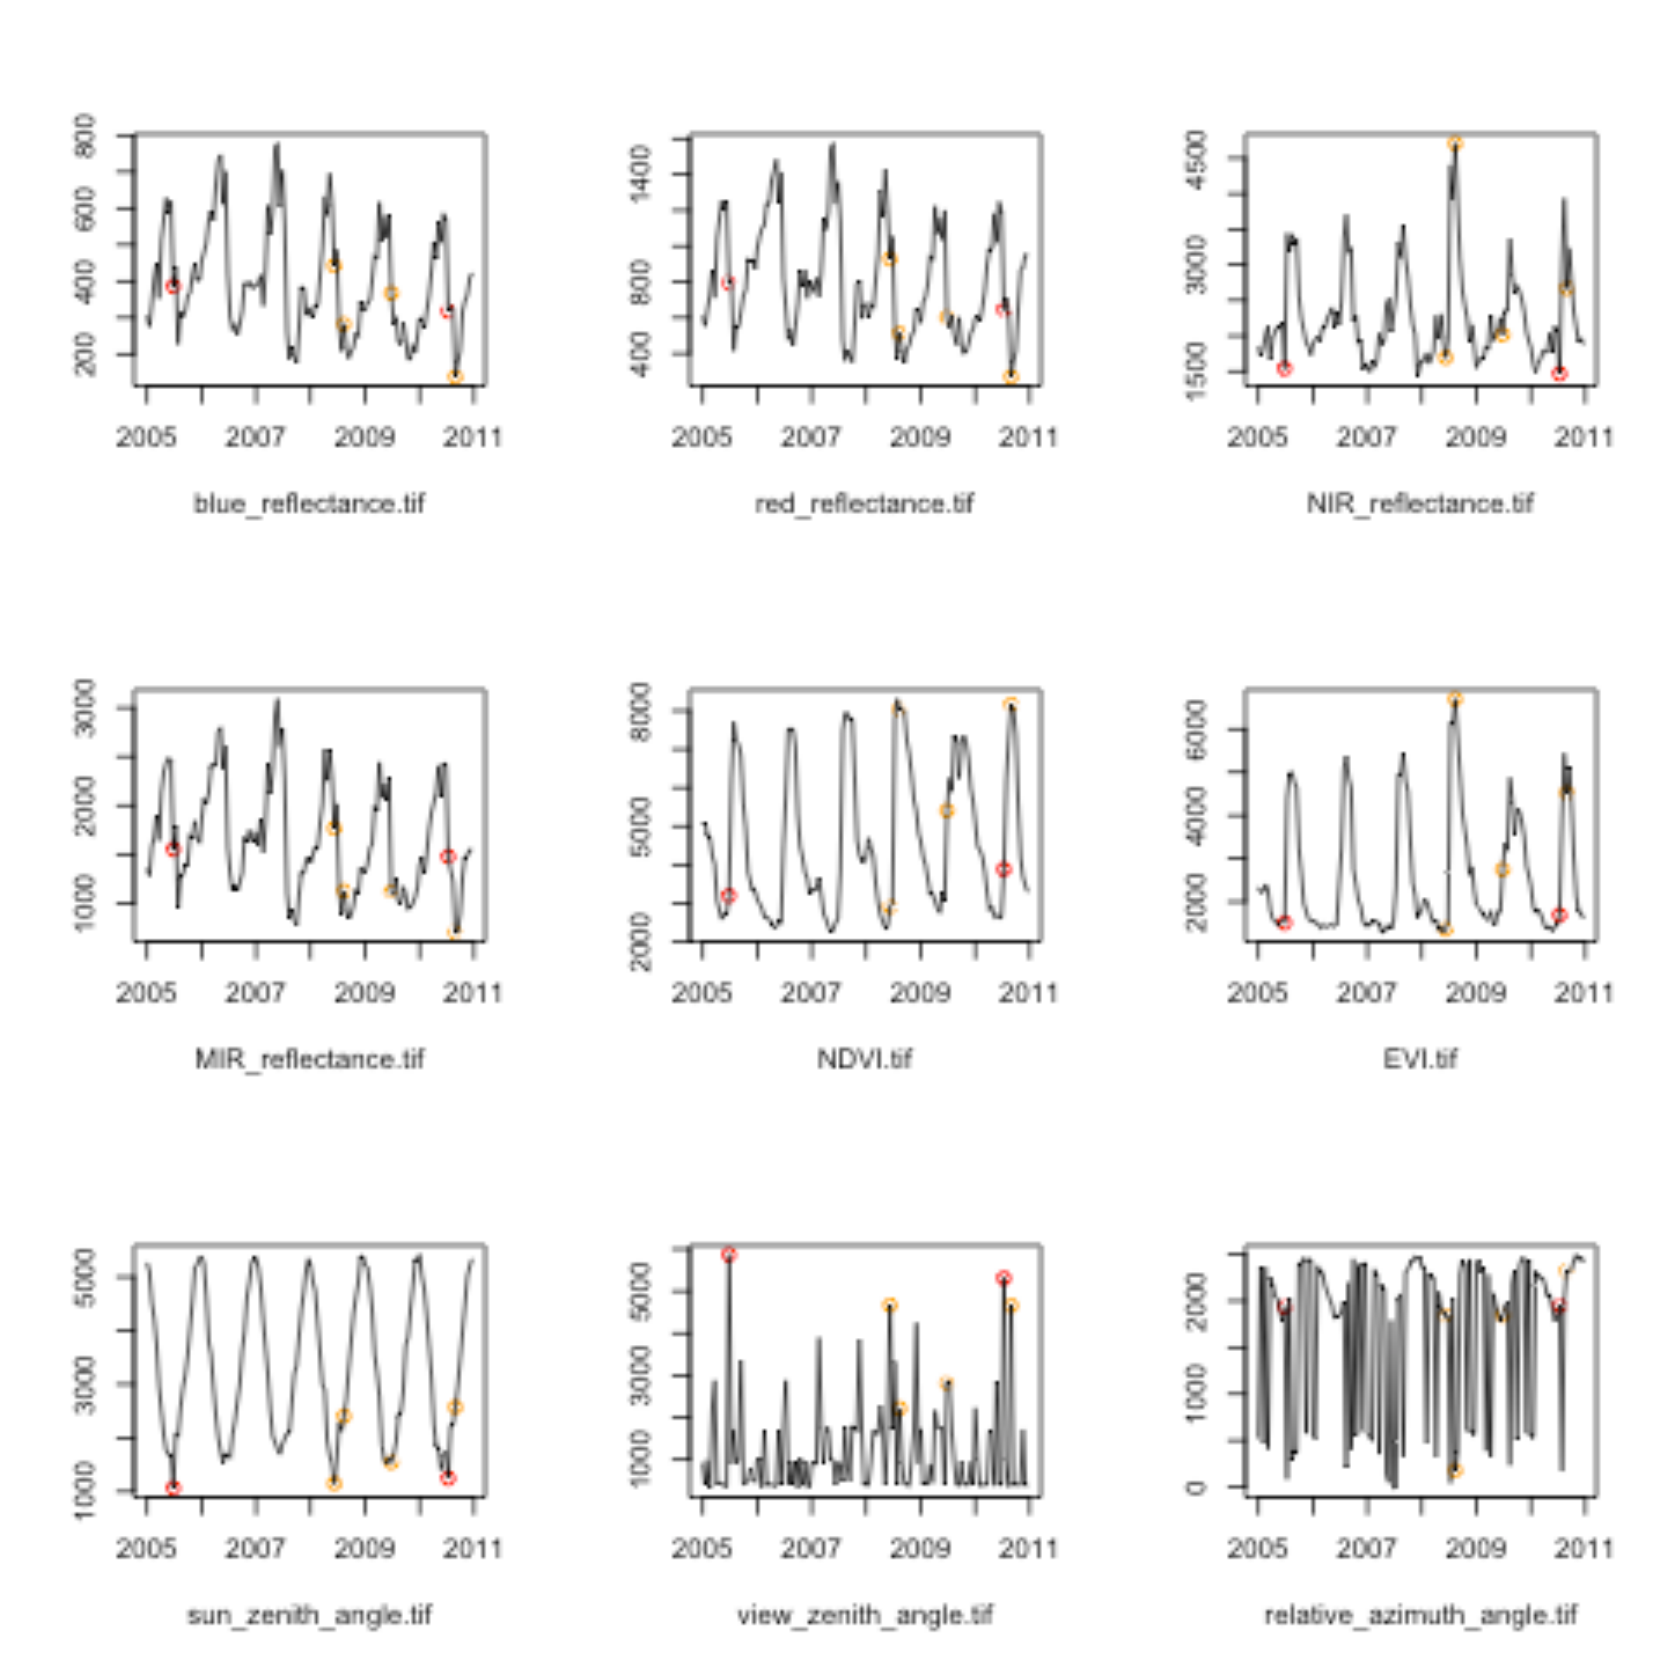}
   	        \caption{non-deforested pixel}
   	        \label{fig:non_defo_pix}
   	      \end{subfigure}
   	      %%         --- .5\textwidth stands for 50% of text width
   	      \caption[Reflectance, vegetation indices and sun-sensor geometry time series for deforested and non-deforested pixel in Yucatan 180 site.]%<<-- Legend for the list of figures at the beginning of you thesis
   	      {Reflectance, vegetation indices and sun-sensor geometry time series for deforested and non-deforested pixel in Sonora74 site, identified in figure \ref{fig:defoSonora74} with green and red circles respectively. Orange marked points are \emph{marginal data} and red marked points are \emph{cloudy} or \emph{not processed}}% legend displayed below the graph.
   	      \label{fig:timeSeries}
   	    \end{figure}
