# Supplementary material for: Online deforestation detection
Source: arXiv:1704.00829 source file (2017-04-03)
Supplement: Supplementary file 2 [file 7B_AppendixGridSearch.tex]

\chapter{Grid search} \label{app:gridSearch}

We include the figures for the remaining 7 sites not included in section \ref{s:gridSearch}.  

\subsection{Forest to water sites}

		\subsubsection{Jalisco164}
		
		\begin{figure}[H]%--- Picture 'H'ere, 'B'ottom or 'T'op; '!' Try to
		                    %impose your will to LaTeX
		  \centering
		  \includegraphics[width=.5\textwidth]{./graphs/graphs_batch1_allPix_FINAL/_--_NIR_reflectance_train_Jalisco164} %<< no file extension
		  %%         --- .5\textwidth stands for 50% of text width
		  \caption[Grid search for optimal NIR reflectance threshold for Jalisco164 site (training $1-tss$).]%<<-- Legend for the list of figures at the beginning of you thesis
		  {Grid search for optimal NIR reflectance threshold for Jalisco164 site (training $1-tss$).}% legend displayed below the graph.
		  \label{fig:grdSrch_Jalisco164}
		\end{figure}
		
		 \begin{figure}[H]
	      \begin{subfigure}{.5\textwidth}
	        \centering
	    	\includegraphics[width=1\textwidth]{./graphs/graphs_batch1_allPix_FINAL/_--_NIR_reflectance_tss_CV_Jalisco164} 
	        \caption{$1-tss$}
	        \label{fig:defo_pix}
	      \end{subfigure}%
	      \begin{subfigure}{.5\textwidth}
	        \centering
	        \includegraphics[width=1\textwidth]{./graphs/graphs_batch1_allPix_FINAL/_--_NIR_reflectance_acc_CV_Jalisco164}
	        \caption{$a_p$ and $a_u$}
	        \label{fig:non_defo_pix}
	      \end{subfigure}
	      %%         --- .5\textwidth stands for 50% of text width
	      \caption[Grid search for optimal NIR reflectance threshold for Jalisco164 site (cross-validated $1-tss$, $a_p$ and $a_u$).]%<<-- Legend for the list of figures at the beginning of you thesis
	      {Grid search for optimal NIR reflectance threshold for Jalisco164 site (cross-validated $1-tss$, $a_p$ and $a_u$).}% legend displayed below the graph.
	      \label{fig:grid_srch_cv_Jalisco164}
	    \end{figure}
		
		\begin{figure}[H]%--- Picture 'H'ere, 'B'ottom or 'T'op; '!' Try to
		                    %impose your will to LaTeX
		  \centering
		  \includegraphics[width=.5\textwidth]{./graphs/graphs_batch1_allPix_FINAL/_--_NIR_reflectance_train_consec3_raster_Jalisco164} %<< no file extension
		  %%         --- .5\textwidth stands for 50% of text width
		  \caption[Spatial results for Jalisco164 site of applying optimal threshold using 3 consecutive violation rule.]%<<-- Legend for the list of figures at the beginning of you thesis
		  {Spatial results for Jalisco164 site of applying optimal threshold using 3 consecutive violation rule.}% legend displayed below the graph.
		  \label{fig:grdSrch_spatial_Jalisco164}
		\end{figure}
		
		\subsubsection{Nayarit151}
		
		\begin{figure}[H]%--- Picture 'H'ere, 'B'ottom or 'T'op; '!' Try to
		                    %impose your will to LaTeX
		  \centering
		  \includegraphics[width=.5\textwidth]{./graphs/graphs_batch1_allPix_FINAL/_--_NIR_reflectance_train_Nayarit151} %<< no file extension
		  %%         --- .5\textwidth stands for 50% of text width
		  \caption[Grid search for optimal NIR reflectance threshold for Nayarit151 site (training $1-tss$).]%<<-- Legend for the list of figures at the beginning of you thesis
		  {Grid search for optimal NIR reflectance threshold for Nayarit151 site (training $1-tss$).}% legend displayed below the graph.
		  \label{fig:grdSrch_Nayarit151}
		\end{figure}
		
		 \begin{figure}[H]
	      \begin{subfigure}{.5\textwidth}
	        \centering
	    	\includegraphics[width=1\textwidth]{./graphs/graphs_batch1_allPix_FINAL/_--_NIR_reflectance_tss_CV_Nayarit151} 
	        \caption{$1-tss$}
	        \label{fig:defo_pix}
	      \end{subfigure}%
	      \begin{subfigure}{.5\textwidth}
	        \centering
	        \includegraphics[width=1\textwidth]{./graphs/graphs_batch1_allPix_FINAL/_--_NIR_reflectance_acc_CV_Nayarit151}
	        \caption{$a_p$ and $a_u$}
	        \label{fig:non_defo_pix}
	      \end{subfigure}
	      %%         --- .5\textwidth stands for 50% of text width
	      \caption[Grid search for optimal NIR reflectance threshold for Nayarit151 site (cross-validated $1-tss$, $a_p$ and $a_u$).]%<<-- Legend for the list of figures at the beginning of you thesis
	      {Grid search for optimal NIR reflectance threshold for Nayarit151 site (cross-validated $1-tss$, $a_p$ and $a_u$).}% legend displayed below the graph.
	      \label{fig:grid_srch_cv_Nayarit151}
	    \end{figure}
		
		\begin{figure}[H]%--- Picture 'H'ere, 'B'ottom or 'T'op; '!' Try to
		                    %impose your will to LaTeX
		  \centering
		  \includegraphics[width=.5\textwidth]{./graphs/graphs_batch1_allPix_FINAL/_--_NIR_reflectance_train_consec3_raster_Nayarit151} %<< no file extension
		  %%         --- .5\textwidth stands for 50% of text width
		  \caption[Spatial results for Nayarit151 site of applying optimal threshold using 3 consecutive violation rule.]%<<-- Legend for the list of figures at the beginning of you thesis
		  {Spatial results for Nayarit151 site of applying optimal threshold using 3 consecutive violation rule.}% legend displayed below the graph.
		  \label{fig:grdSrch_spatial_Nayarit151}
		\end{figure}
		
		\subsubsection{Nayarit109}
		
		\begin{figure}[H]%--- Picture 'H'ere, 'B'ottom or 'T'op; '!' Try to
		                    %impose your will to LaTeX
		  \centering
		  \includegraphics[width=.5\textwidth]{./graphs/graphs_batch1_allPix_FINAL/_--_NIR_reflectance_train_Nayarit109} %<< no file extension
		  %%         --- .5\textwidth stands for 50% of text width
		  \caption[Grid search for optimal NIR reflectance threshold for Nayarit109 site (training $1-tss$).]%<<-- Legend for the list of figures at the beginning of you thesis
		  {Grid search for optimal NIR reflectance threshold for Nayarit109 site (training $1-tss$).}% legend displayed below the graph.
		  \label{fig:grdSrch_Nayarit109}
		\end{figure}
		
		 \begin{figure}[H]
	      \begin{subfigure}{.5\textwidth}
	        \centering
	    	\includegraphics[width=1\textwidth]{./graphs/graphs_batch1_allPix_FINAL/_--_NIR_reflectance_tss_CV_Nayarit109} 
	        \caption{$1-tss$}
	        \label{fig:defo_pix}
	      \end{subfigure}%
	      \begin{subfigure}{.5\textwidth}
	        \centering
	        \includegraphics[width=1\textwidth]{./graphs/graphs_batch1_allPix_FINAL/_--_NIR_reflectance_acc_CV_Nayarit109}
	        \caption{$a_p$ and $a_u$}
	        \label{fig:non_defo_pix}
	      \end{subfigure}
	      %%         --- .5\textwidth stands for 50% of text width
	      \caption[Grid search for optimal NIR reflectance threshold for Nayarit109 site (cross-validated $1-tss$, $a_p$ and $a_u$).]%<<-- Legend for the list of figures at the beginning of you thesis
	      {Grid search for optimal NIR reflectance threshold for Nayarit109 site (cross-validated $1-tss$, $a_p$ and $a_u$).}% legend displayed below the graph.
	      \label{fig:grid_srch_cv_Nayarit109}
	    \end{figure}
		
		\begin{figure}[H]%--- Picture 'H'ere, 'B'ottom or 'T'op; '!' Try to
		                    %impose your will to LaTeX
		  \centering
		  \includegraphics[width=.5\textwidth]{./graphs/graphs_batch1_allPix_FINAL/_--_NIR_reflectance_train_consec3_raster_Nayarit109} %<< no file extension
		  %%         --- .5\textwidth stands for 50% of text width
		  \caption[Spatial results for Nayarit109 site of applying optimal threshold using 3 consecutive violation rule.]%<<-- Legend for the list of figures at the beginning of you thesis
		  {Spatial results for Nayarit109 site of applying optimal threshold using 3 consecutive violation rule.}% legend displayed below the graph.
		  \label{fig:grdSrch_spatial_Nayarit109}
		\end{figure}

\subsection{Forest to urban or cropland sites}
		
		\subsubsection{QuintanaRoo100}
		
		\begin{figure}[H]%--- Picture 'H'ere, 'B'ottom or 'T'op; '!' Try to
		                    %impose your will to LaTeX
		  \centering
		  \includegraphics[width=.5\textwidth]{./graphs/graphs_batch1_allPix_FINAL/_--_NDVI_train_QuintanaRoo100} %<< no file extension
		  %%         --- .5\textwidth stands for 50% of text width
		  \caption[Grid search for optimal NDVI threshold for QuintanaRoo100 site (training $1-tss$).]%<<-- Legend for the list of figures at the beginning of you thesis
		  {Grid search for optimal NDVI threshold for QuintanaRoo100 site (training $1-tss$).}% legend displayed below the graph.
		  \label{fig:grdSrch_QuintanaRoo100}
		\end{figure}
		
		 \begin{figure}[H]
	      \begin{subfigure}{.5\textwidth}
	        \centering
	    	\includegraphics[width=1\textwidth]{./graphs/graphs_batch1_allPix_FINAL/_--_NDVI_tss_CV_QuintanaRoo100} 
	        \caption{$1-tss$}
	        \label{fig:defo_pix}
	      \end{subfigure}%
	      \begin{subfigure}{.5\textwidth}
	        \centering
	        \includegraphics[width=1\textwidth]{./graphs/graphs_batch1_allPix_FINAL/_--_NDVI_acc_CV_QuintanaRoo100}
	        \caption{$a_p$ and $a_u$}
	        \label{fig:non_defo_pix}
	      \end{subfigure}
	      %%         --- .5\textwidth stands for 50% of text width
	      \caption[Grid search for optimal NDVI threshold for QuintanaRoo100 site (cross-validated $1-tss$, $a_p$ and $a_u$).]%<<-- Legend for the list of figures at the beginning of you thesis
	      {Grid search for optimal NDVI threshold for QuintanaRoo100 site (cross-validated $1-tss$, $a_p$ and $a_u$).}% legend displayed below the graph.
	      \label{fig:grid_srch_cv_QuintanaRoo100}
	    \end{figure}
		
		\begin{figure}[H]%--- Picture 'H'ere, 'B'ottom or 'T'op; '!' Try to
		                    %impose your will to LaTeX
		  \centering
		  \includegraphics[width=.5\textwidth]{./graphs/graphs_batch1_allPix_FINAL/_--_NDVI_train_consec3_raster_QuintanaRoo100} %<< no file extension
		  %%         --- .5\textwidth stands for 50% of text width
		  \caption[Spatial results for QuintanaRoo100 site of applying optimal threshold using 3 consecutive violation rule.]%<<-- Legend for the list of figures at the beginning of you thesis
		  {Spatial results for QuintanaRoo100 site of applying optimal threshold using 3 consecutive violation rule.}% legend displayed below the graph.
		  \label{fig:grdSrch_spatial_QuintanaRoo100}
		\end{figure}

		\subsubsection{Michoacan98}
		
		\begin{figure}[H]%--- Picture 'H'ere, 'B'ottom or 'T'op; '!' Try to
		                    %impose your will to LaTeX
		  \centering
		  \includegraphics[width=.5\textwidth]{./graphs/graphs_batch1_allPix_FINAL/_--_NDVI_train_Michoacan98} %<< no file extension
		  %%         --- .5\textwidth stands for 50% of text width
		  \caption[Grid search for optimal NDVI threshold for Michoacan98 site (training $1-tss$).]%<<-- Legend for the list of figures at the beginning of you thesis
		  {Grid search for optimal NDVI threshold for Michoacan98 site (training $1-tss$).}% legend displayed below the graph.
		  \label{fig:grdSrch_Michoacan98}
		\end{figure}
		
		 \begin{figure}[H]
	      \begin{subfigure}{.5\textwidth}
	        \centering
	    	\includegraphics[width=1\textwidth]{./graphs/graphs_batch1_allPix_FINAL/_--_NDVI_tss_CV_Michoacan98} 
	        \caption{$1-tss$}
	        \label{fig:defo_pix}
	      \end{subfigure}%
	      \begin{subfigure}{.5\textwidth}
	        \centering
	        \includegraphics[width=1\textwidth]{./graphs/graphs_batch1_allPix_FINAL/_--_NDVI_acc_CV_Michoacan98}
	        \caption{$a_p$ and $a_u$}
	        \label{fig:non_defo_pix}
	      \end{subfigure}
	      %%         --- .5\textwidth stands for 50% of text width
	      \caption[Grid search for optimal NDVI threshold for Michoacan98 site (cross-validated $1-tss$, $a_p$ and $a_u$).]%<<-- Legend for the list of figures at the beginning of you thesis
	      {Grid search for optimal NDVI threshold for Michoacan98 site (cross-validated $1-tss$, $a_p$ and $a_u$).}% legend displayed below the graph.
	      \label{fig:grid_srch_cv_Michoacan98}
	    \end{figure}
		
		\begin{figure}[H]%--- Picture 'H'ere, 'B'ottom or 'T'op; '!' Try to
		                    %impose your will to LaTeX
		  \centering
		  \includegraphics[width=.5\textwidth]{./graphs/graphs_batch1_allPix_FINAL/_--_NDVI_train_consec3_raster_Michoacan98} %<< no file extension
		  %%         --- .5\textwidth stands for 50% of text width
		  \caption[Spatial results for Michoacan98 site of applying optimal threshold using 3 consecutive violation rule.]%<<-- Legend for the list of figures at the beginning of you thesis
		  {Spatial results for Michoacan98 site of applying optimal threshold using 3 consecutive violation rule.}% legend displayed below the graph.
		  \label{fig:grdSrch_spatial_Michoacan98}
		\end{figure}

		\subsubsection{QuintanaRoo77}
			
		\begin{figure}[H]%--- Picture 'H'ere, 'B'ottom or 'T'op; '!' Try to
		                    %impose your will to LaTeX
		  \centering
		  \includegraphics[width=.5\textwidth]{./graphs/graphs_batch1_allPix_FINAL/_--_NDVI_train_QuintanaRoo77} %<< no file extension
		  %%         --- .5\textwidth stands for 50% of text width
		  \caption[Grid search for optimal NDVI threshold for QuintanaRoo77 site (training $1-tss$).]%<<-- Legend for the list of figures at the beginning of you thesis
		  {Grid search for optimal NDVI threshold for QuintanaRoo77 site (training $1-tss$).}% legend displayed below the graph.
		  \label{fig:grdSrch_QuintanaRoo77}
		\end{figure}
		
		 \begin{figure}[H]
	      \begin{subfigure}{.5\textwidth}
	        \centering
	    	\includegraphics[width=1\textwidth]{./graphs/graphs_batch1_allPix_FINAL/_--_NDVI_tss_CV_QuintanaRoo77} 
	        \caption{$1-tss$}
	        \label{fig:defo_pix}
	      \end{subfigure}%
	      \begin{subfigure}{.5\textwidth}
	        \centering
	        \includegraphics[width=1\textwidth]{./graphs/graphs_batch1_allPix_FINAL/_--_NDVI_acc_CV_QuintanaRoo77}
	        \caption{$a_p$ and $a_u$}
	        \label{fig:non_defo_pix}
	      \end{subfigure}
	      %%         --- .5\textwidth stands for 50% of text width
	      \caption[Grid search for optimal NDVI threshold for QuintanaRoo77 site (cross-validated $1-tss$, $a_p$ and $a_u$).]%<<-- Legend for the list of figures at the beginning of you thesis
	      {Grid search for optimal NDVI threshold for QuintanaRoo77 site (cross-validated $1-tss$, $a_p$ and $a_u$).}% legend displayed below the graph.
	      \label{fig:grid_srch_cv_QuintanaRoo77}
	    \end{figure}
		
		\begin{figure}[H]%--- Picture 'H'ere, 'B'ottom or 'T'op; '!' Try to
		                    %impose your will to LaTeX
		  \centering
		  \includegraphics[width=.5\textwidth]{./graphs/graphs_batch1_allPix_FINAL/_--_NDVI_train_consec3_raster_QuintanaRoo77} %<< no file extension
		  %%         --- .5\textwidth stands for 50% of text width
		  \caption[Spatial results for QuintanaRoo77 site of applying optimal threshold using 3 consecutive violation rule.]%<<-- Legend for the list of figures at the beginning of you thesis
		  {Spatial results for QuintanaRoo77 site of applying optimal threshold using 3 consecutive violation rule.}% legend displayed below the graph.
		  \label{fig:grdSrch_spatial_QuintanaRoo77}
		\end{figure}

		\subsubsection{Sonora74}
		
		\begin{figure}[H]%--- Picture 'H'ere, 'B'ottom or 'T'op; '!' Try to
		                    %impose your will to LaTeX
		  \centering
		  \includegraphics[width=.5\textwidth]{./graphs/graphs_batch1_allPix_FINAL/_--_NDVI_train_Sonora74} %<< no file extension
		  %%         --- .5\textwidth stands for 50% of text width
		  \caption[Grid search for optimal NDVI threshold for Sonora74 site (training $1-tss$).]%<<-- Legend for the list of figures at the beginning of you thesis
		  {Grid search for optimal NDVI threshold for Sonora74 site (training $1-tss$).}% legend displayed below the graph.
		  \label{fig:grdSrch_Sonora74}
		\end{figure}
		
		 \begin{figure}[H]
	      \begin{subfigure}{.5\textwidth}
	        \centering
	    	\includegraphics[width=1\textwidth]{./graphs/graphs_batch1_allPix_FINAL/_--_NDVI_tss_CV_Sonora74} 
	        \caption{$1-tss$}
	        \label{fig:defo_pix}
	      \end{subfigure}%
	      \begin{subfigure}{.5\textwidth}
	        \centering
	        \includegraphics[width=1\textwidth]{./graphs/graphs_batch1_allPix_FINAL/_--_NDVI_acc_CV_Sonora74}
	        \caption{$a_p$ and $a_u$}
	        \label{fig:non_defo_pix}
	      \end{subfigure}
	      %%         --- .5\textwidth stands for 50% of text width
	      \caption[Grid search for optimal NDVI threshold for Sonora74 site (cross-validated $1-tss$, $a_p$ and $a_u$).]%<<-- Legend for the list of figures at the beginning of you thesis
	      {Grid search for optimal NDVI threshold for Sonora74 site (cross-validated $1-tss$, $a_p$ and $a_u$).}% legend displayed below the graph.
	      \label{fig:grid_srch_cv_Sonora74}
	    \end{figure}
		
		\begin{figure}[H]%--- Picture 'H'ere, 'B'ottom or 'T'op; '!' Try to
		                    %impose your will to LaTeX
		  \centering
		  \includegraphics[width=.5\textwidth]{./graphs/graphs_batch1_allPix_FINAL/_--_NDVI_train_consec3_raster_Sonora74} %<< no file extension
		  %%         --- .5\textwidth stands for 50% of text width
		  \caption[Spatial results for Sonora74 site of applying optimal threshold using 3 consecutive violation rule.]%<<-- Legend for the list of figures at the beginning of you thesis
		  {Spatial results for Sonora74 site of applying optimal threshold using 3 consecutive violation rule.}% legend displayed below the graph.
		  \label{fig:grdSrch_spatial_Sonora74}
		\end{figure}
