# Supplementary material for: Online deforestation detection
Source: arXiv:1704.00829 source file (2017-04-03)
Supplement: Supplementary file 3 [file 7C_AppendixGridSearchMahalanobis.tex]

\chapter{Mahalanobis distance extended results} \label{app:gridSearchMahl}

\section{Overall grid search}

			\begin{figure}[H]%--- Picture 'H'ere, 'B'ottom or 'T'op; '!' Try to
			                    %impose your will to LaTeX
			  \centering
			  \includegraphics[width=.5\textwidth]{./graphs/graphs_batch1_allPix_FINAL/_--_Mahl_dist_train_all} %<< no file extension
			  %%         --- .5\textwidth stands for 50% of text width
			  \caption[Grid search for optimal Mahalanobis distance threshold for all 9 sites (training $1-tss$).]%<<-- Legend for the list of figures at the beginning of you thesis
			  {Grid search for optimal Mahalanobis distance threshold for all 9 sites (training $1-tss$).}% legend displayed below the graph.
			  \label{fig:grdSrch_all_mahl}
			\end{figure}
		
			 \begin{figure}[H]
		      \begin{subfigure}{.5\textwidth}
		        \centering
		    	\includegraphics[width=1\textwidth]{./graphs/graphs_batch1_allPix_FINAL/_--_Mahl_dist_tss_CV_all} 
		        \caption{$1-tss$}
		        \label{fig:defo_pix}
		      \end{subfigure}%
		      \begin{subfigure}{.5\textwidth}
		        \centering
		        \includegraphics[width=1\textwidth]{./graphs/graphs_batch1_allPix_FINAL/_--_Mahl_dist_acc_CV_all}
		        \caption{$a_p$ and $a_u$}
		        \label{fig:non_defo_pix}
		      \end{subfigure}
		      %%         --- .5\textwidth stands for 50% of text width
		      \caption[Grid search for optimal Mahalanobis distance threshold for all 9 sites (cross-validated $1-tss$, $a_p$ and $a_u$).]%<<-- Legend for the list of figures at the beginning of you thesis
		      {Grid search for optimal Mahalanobis distance threshold for all 9 sites (cross-validated $1-tss$, $a_p$ and $a_u$).}% legend displayed below the graph.
			      \label{fig:grid_srch_cv_all_mahl}
		    \end{figure}
			
			\begin{center}
				\footnotesize\addtolength{\tabcolsep}{-2pt}
				% latex table generated in R 3.3.2 by xtable 1.8-2 package
% Thu Mar  9 23:29:51 2017
\begin{table}[ht]
\centering
\begingroup\tiny
\begin{tabular}{lll|ccccc|ccccc|ccccc}
 data & site & variable & 2 & 3 & 4 & 5 & 6 & 2 & 3 & 4 & 5 & 6 & 2 & 3 & 4 & 5 & 6 \\ 
  \hline
train & all & Mahl. dist. & 15.17 & 17.24 & 11.72 & 8.28 & 5.52 & 72.00 & 68.98 & 68.84 & 69.88 & 70.03 & 29.41 & 31.38 & 28.53 & 31.37 & 30.33 \\ 
  cv & all & Mahl. dist. & 15.17 & 17.24 & 11.72 & 8.28 & 5.52 & 74.94 & 70.17 & 68.96 & 72.90 & 72.16 & 29.42 & 31.34 & 29.91 & 30.34 & 30.27 \\ 
   \hline
\end{tabular}
\endgroup
\caption[optimal threshold, 1-tss and user/producer accuracy for all sites, Mahalanobis distance]{optimal threshold, 1-tss and user/producer accuracy for all sites, Mahalanobis distance} 
\end{table}

				\label{tab:grdSrch_consecVaries_all_mahl}
			\end{center}

			\begin{center}
				\footnotesize\addtolength{\tabcolsep}{-2pt}
				% latex table generated in R 3.3.2 by xtable 1.8-2 package
% Thu Mar  9 23:13:26 2017
\begin{table}[ht]
\centering
\begingroup\tiny
\begin{tabular}{lcl|ccccc}
 site & threshold & variable & 2 & 3 & 4 & 5 & 6 \\ 
  \hline
all & 17.24 & Mahl. dist. & 72.58 & 68.98 & 76.93 & 80.99 & 84.37 \\ 
  \end{tabular}
\endgroup
\caption[1-tss  all sites, Mahalanobis distance]{1-tss  all sites, Mahalanobis distance} 
\end{table}

				\label{tab:grdSrch_consecFix_all_mahl}
			\end{center}

\section{Site by site grid search}

			\begin{center}
				\footnotesize\addtolength{\tabcolsep}{-2pt}
				% latex table generated in R 3.3.2 by xtable 1.8-2 package
% Thu Mar  9 20:16:17 2017
\begin{table}[ht]
\centering
\begingroup\tiny
\begin{tabular}{ll|ccccc|ccccc|ccccc}
 site & variable & 2 & 3 & 4 & 5 & 6 & 2 & 3 & 4 & 5 & 6 & 2 & 3 & 4 & 5 & 6 \\ 
  \hline
Sonora232 & Mahl. dist. & 9.66 & 17.24 & 5.52 & 13.10 & 5.52 & 93.13 & 86.19 & 89.64 & 92.99 & 91.10 & 17.85 & 20.65 & 18.69 & 14.88 & 15.39 \\ 
  Jalisco164 & Mahl. dist. & 16.55 & 13.10 & 12.41 & 8.28 & 5.52 & 36.56 & 37.44 & 37.66 & 32.99 & 33.23 & 64.38 & 66.04 & 66.67 & 68.78 & 68.83 \\ 
  Nayarit151 & Mahl. dist. & 13.79 & 11.72 & 11.72 & 10.34 & 8.28 & 34.42 & 38.42 & 40.94 & 40.18 & 35.80 & 52.57 & 58.54 & 55.84 & 58.04 & 67.06 \\ 
  Nayarit109 & Mahl. dist. & 9.66 & 8.28 & 8.97 & 8.97 & 3.45 & 33.73 & 34.52 & 37.30 & 40.87 & 36.31 & 59.03 & 54.09 & 51.47 & 53.12 & 54.09 \\ 
   \hline
Yucatan180 & Mahl. dist. & 20.00 & 18.62 & 12.41 & 13.10 & 8.28 & 91.56 & 62.32 & 68.86 & 69.70 & 68.06 & 43.53 & 40.30 & 32.39 & 24.94 & 22.29 \\ 
  QuintanaRoo100 & Mahl. dist. & 15.17 & 9.66 & 9.66 & 4.14 & 3.45 & 82.02 & 92.79 & 80.73 & 78.57 & 85.92 & 13.17 & 5.72 & 24.44 & 19.05 & 10.32 \\ 
  Michoacan98 & Mahl. dist. & 9.66 & 7.59 & 5.52 & 4.14 & 3.45 & 81.07 & 76.47 & 74.37 & 71.65 & 64.71 & 9.02 & 6.48 & 13.15 & 13.15 & 17.88 \\ 
  QuintanaRoo77 & Mahl. dist. & 19.31 & 13.10 & 9.66 & 5.52 & 5.52 & 71.72 & 68.57 & 59.88 & 54.69 & 64.69 & 27.88 & 30.79 & 20.53 & 21.64 & 15.39 \\ 
  Sonora74 & Mahl. dist. & 17.93 & 15.17 & 12.41 & 11.72 & 9.66 & 69.15 & 65.93 & 66.78 & 75.59 & 74.75 & 20.00 & 23.82 & 19.09 & 10.56 & 21.11 \\ 
   \hline
\end{tabular}
\endgroup
\caption{optimal threshold, 1-tss and user/producer accuracy for each site (training data), Mahalanobis distance} 
\end{table}

				\label{tab:grdSrch_consecVaries_mahl}
			\end{center}
		
			\begin{center}
				\footnotesize\addtolength{\tabcolsep}{-2pt}
				% latex table generated in R 3.3.2 by xtable 1.8-2 package
% Thu Mar  9 20:16:25 2017
\begin{table}[ht]
\centering
\begingroup\tiny
\begin{tabular}{ll|ccccc|ccccc|ccccc}
 site & variable & 2 & 3 & 4 & 5 & 6 & 2 & 3 & 4 & 5 & 6 & 2 & 3 & 4 & 5 & 6 \\ 
  \hline
Sonora232 & Mahl. dist. & 9.66 & 17.24 & 5.52 & 13.10 & 5.52 & 98.87 & 86.21 & 96.03 & 96.84 & 97.36 & 19.13 & 20.06 & 18.85 & 15.99 & 15.50 \\ 
  Jalisco164 & Mahl. dist. & 16.55 & 13.10 & 12.41 & 8.28 & 5.52 & 37.92 & 39.18 & 38.68 & 31.93 & 36.80 & 67.07 & 67.93 & 64.02 & 68.67 & 69.69 \\ 
  Nayarit151 & Mahl. dist. & 13.79 & 11.72 & 11.72 & 10.34 & 8.28 & 45.93 & 44.39 & 45.25 & 41.76 & 38.74 & 53.67 & 59.26 & 58.80 & 57.87 & 65.00 \\ 
  Nayarit109 & Mahl. dist. & 9.66 & 8.28 & 8.97 & 8.97 & 3.45 & 48.91 & 42.11 & 58.91 & 51.50 & 43.51 & 50.19 & 43.73 & 41.16 & 51.94 & 49.07 \\ 
   \hline
Yucatan180 & Mahl. dist. & 20.00 & 18.62 & 12.41 & 13.10 & 8.28 & 97.13 & 69.91 & 76.99 & 77.37 & 73.98 & 43.23 & 40.17 & 32.60 & 24.97 & 22.24 \\ 
  QuintanaRoo100 & Mahl. dist. & 15.17 & 9.66 & 9.66 & 4.14 & 3.45 & 85.35 & 102.77 & 89.01 & 77.30 & 80.71 & 17.66 & 12.56 & 21.80 & 19.62 & 17.96 \\ 
  Michoacan98 & Mahl. dist. & 9.66 & 7.59 & 5.52 & 4.14 & 3.45 & 99.52 & 81.72 & 87.21 & 79.93 & 78.98 & 8.77 & 6.33 & 13.84 & 13.76 & 17.35 \\ 
  QuintanaRoo77 & Mahl. dist. & 19.31 & 13.10 & 9.66 & 5.52 & 5.52 & 81.54 & 87.53 & 67.82 & 68.62 & 79.32 & 26.69 & 22.38 & 15.00 & 21.46 & 14.09 \\ 
  Sonora74 & Mahl. dist. & 17.93 & 15.17 & 12.41 & 11.72 & 9.66 & 77.80 & 74.41 & 81.92 & 82.95 & 86.88 & 21.02 & 24.44 &  &  &  \\ 
   \hline
\end{tabular}
\endgroup
\caption[optimal threshold, 1-tss and user/producer accuracy for each site (cross validation), Mahalanobis distance]{optimal threshold, 1-tss and user/producer accuracy for each site (cross validation), Mahalanobis distance} 
\end{table}

				\label{tab:grdSrch_consecVaries_mahl}
			\end{center}

			 \begin{figure}[H]
		      \begin{subfigure}{.5\textwidth}
		        \centering
		    	\includegraphics[width=1\textwidth]{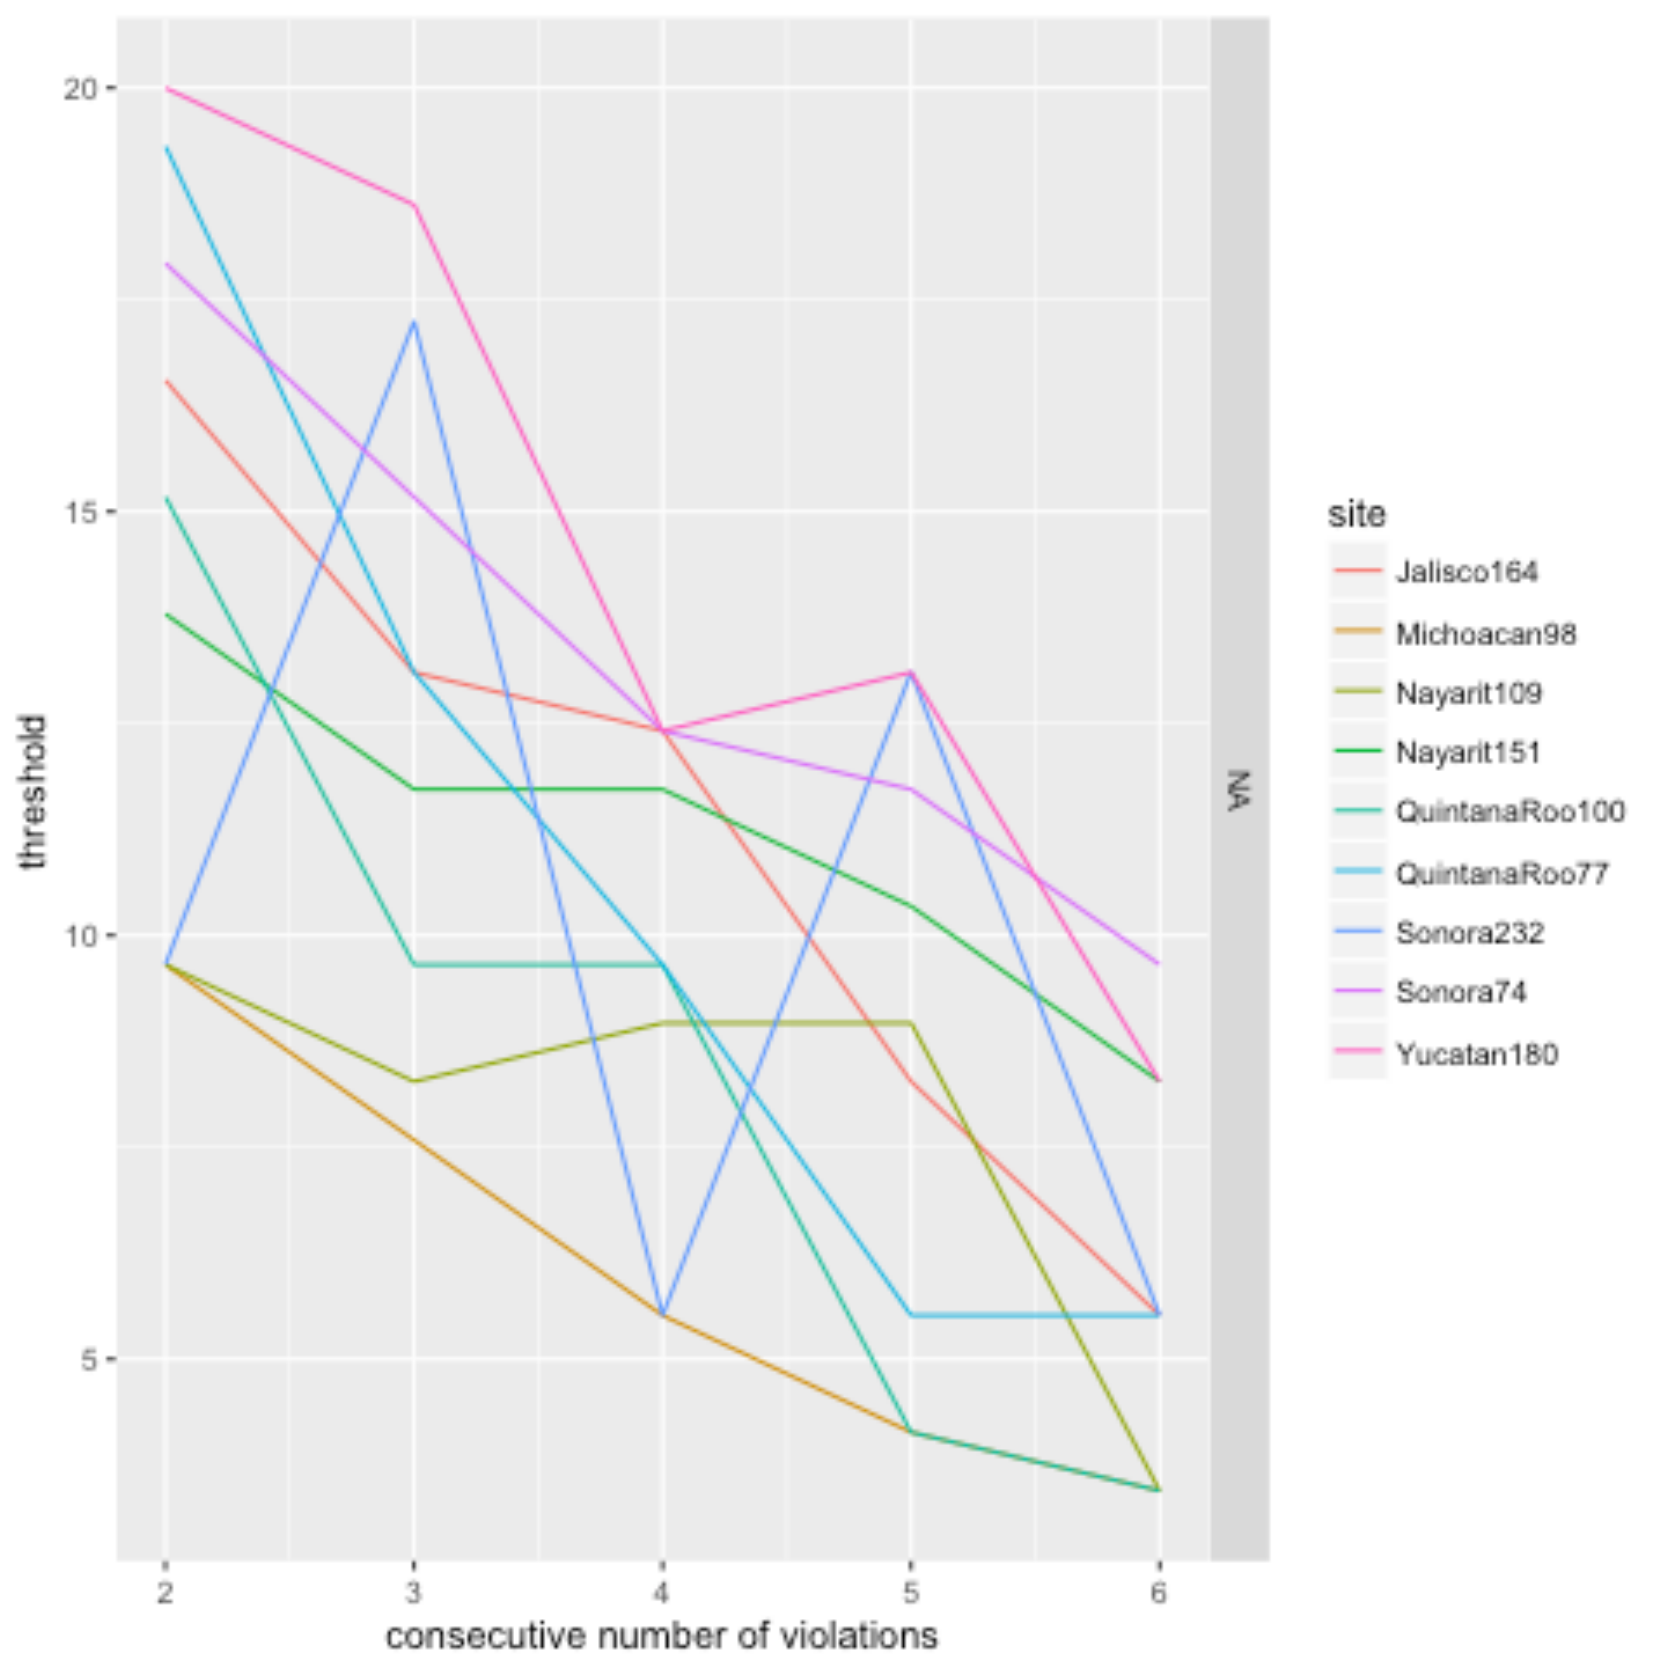} 
		        \caption{Optimal thresholds by site and consecutive number of violations}
		        \label{fig:defo_pix}
		      \end{subfigure}%
		      \begin{subfigure}{.5\textwidth}
		        \centering
		        \includegraphics[width=1\textwidth]{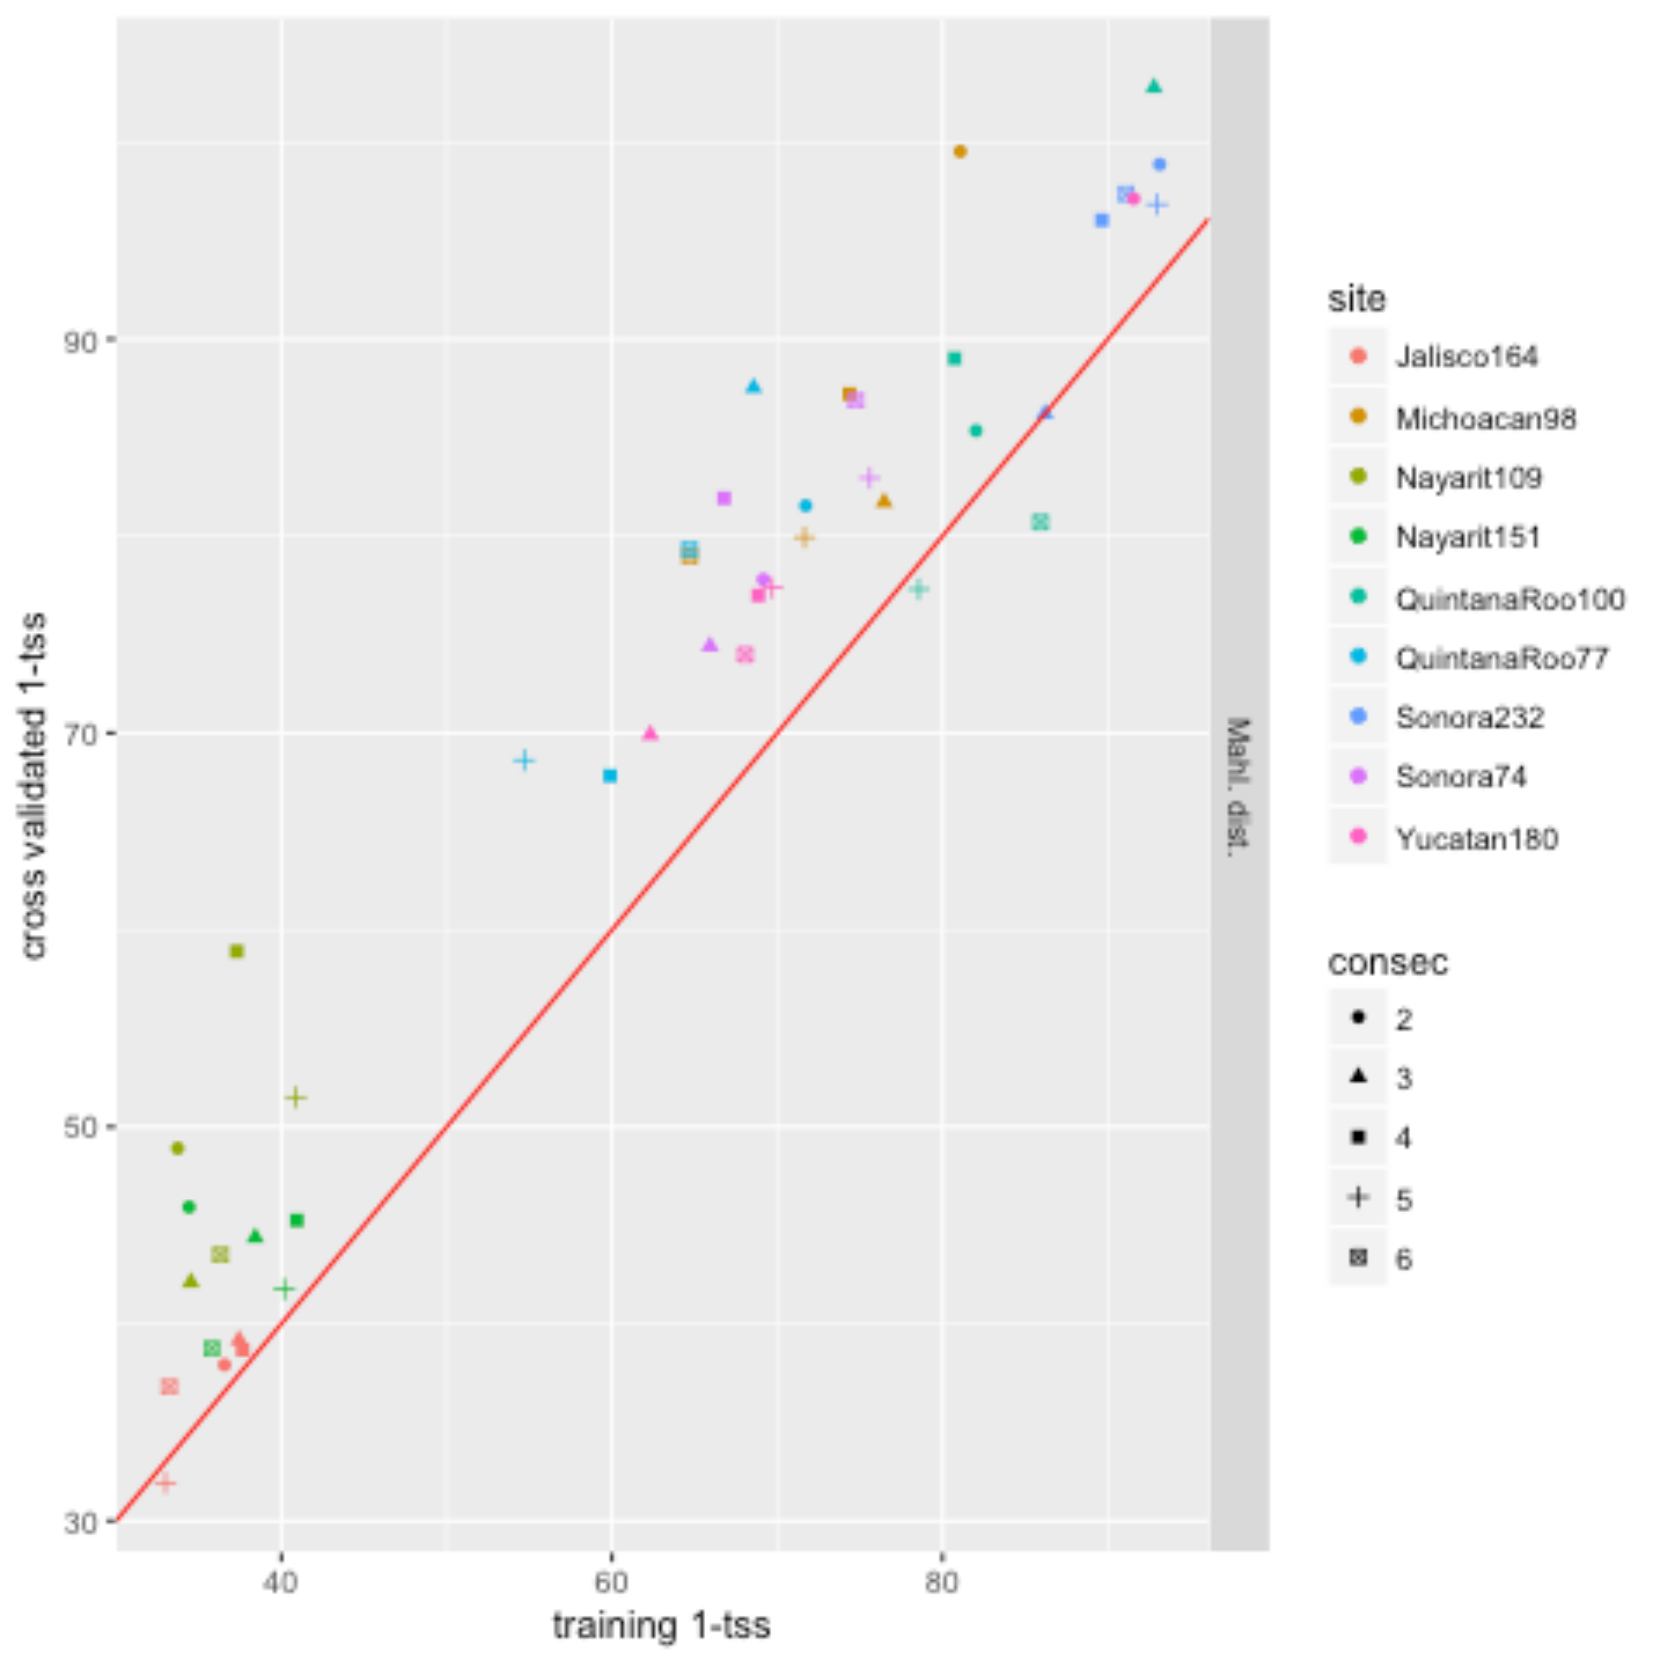}
		        \caption{Training vs. cross-validated $1-tss$}
		        \label{fig:non_defo_pix}
		      \end{subfigure}
		      %%         --- .5\textwidth stands for 50% of text width
		      \caption[Comparison of optimal thresholds by site and comparison between training and cross validated results for grid-search]%<<-- Legend for the list of figures at the beginning of you thesis
		      {Comparison of optimal thresholds by site and comparison between training and cross validated results for grid-search}% legend displayed below the graph.
		      \label{fig:grid_srch_train_cv_mahl}
		    \end{figure}

			\begin{center}
				\footnotesize\addtolength{\tabcolsep}{-2pt}
				% latex table generated in R 3.3.2 by xtable 1.8-2 package
% Thu Mar  9 20:15:35 2017
\begin{table}[ht]
\centering
\begingroup\tiny
\begin{tabular}{lcl|ccccc}
 site & threshold & variable & 2 & 3 & 4 & 5 & 6 \\ 
  \hline
Sonora232 & 17.241 & Mahl. dist. & 99.610 & 86.194 & 92.108 & 96.932 & 99.124 \\ 
  Jalisco164 & 13.103 & Mahl. dist. & 52.349 & 37.438 & 38.954 & 39.920 & 45.470 \\ 
  Nayarit151 & 11.724 & Mahl. dist. & 48.810 & 38.420 & 40.936 & 48.945 & 53.139 \\ 
  Nayarit109 & 8.276 & Mahl. dist. & 40.873 & 34.524 & 39.881 & 42.063 & 45.040 \\ 
   \hline
Yucatan180 & 18.621 & Mahl. dist. & 92.720 & 62.321 & 77.728 & 82.165 & 83.878 \\ 
  QuintanaRoo100 & 9.655 & Mahl. dist. & 91.317 & 92.791 & 80.727 & 84.942 & 94.981 \\ 
  Michoacan98 & 7.586 & Mahl. dist. & 92.306 & 76.467 & 77.503 & 89.888 & 92.353 \\ 
  QuintanaRoo77 & 13.103 & Mahl. dist. & 95.367 & 68.567 & 81.518 & 85.399 & 89.280 \\ 
  Sonora74 & 15.172 & Mahl. dist. & 79.661 & 65.932 & 82.034 & 91.356 & 91.017 \\ 
   \hline
\end{tabular}
\endgroup
\caption[1-tss for each site trained separately with Mahalanobis distance time series]{1-tss for each site trained separately with Mahalanobis distance time series} 
\end{table}

				\label{tab:grdSrch_consecFix_mahl}
			\end{center}
	
			\begin{figure}[H]%--- Picture 'H'ere, 'B'ottom or 'T'op; '!' Try to
			                    %impose your will to LaTeX
			  \centering
			  \includegraphics[width=.5\textwidth]{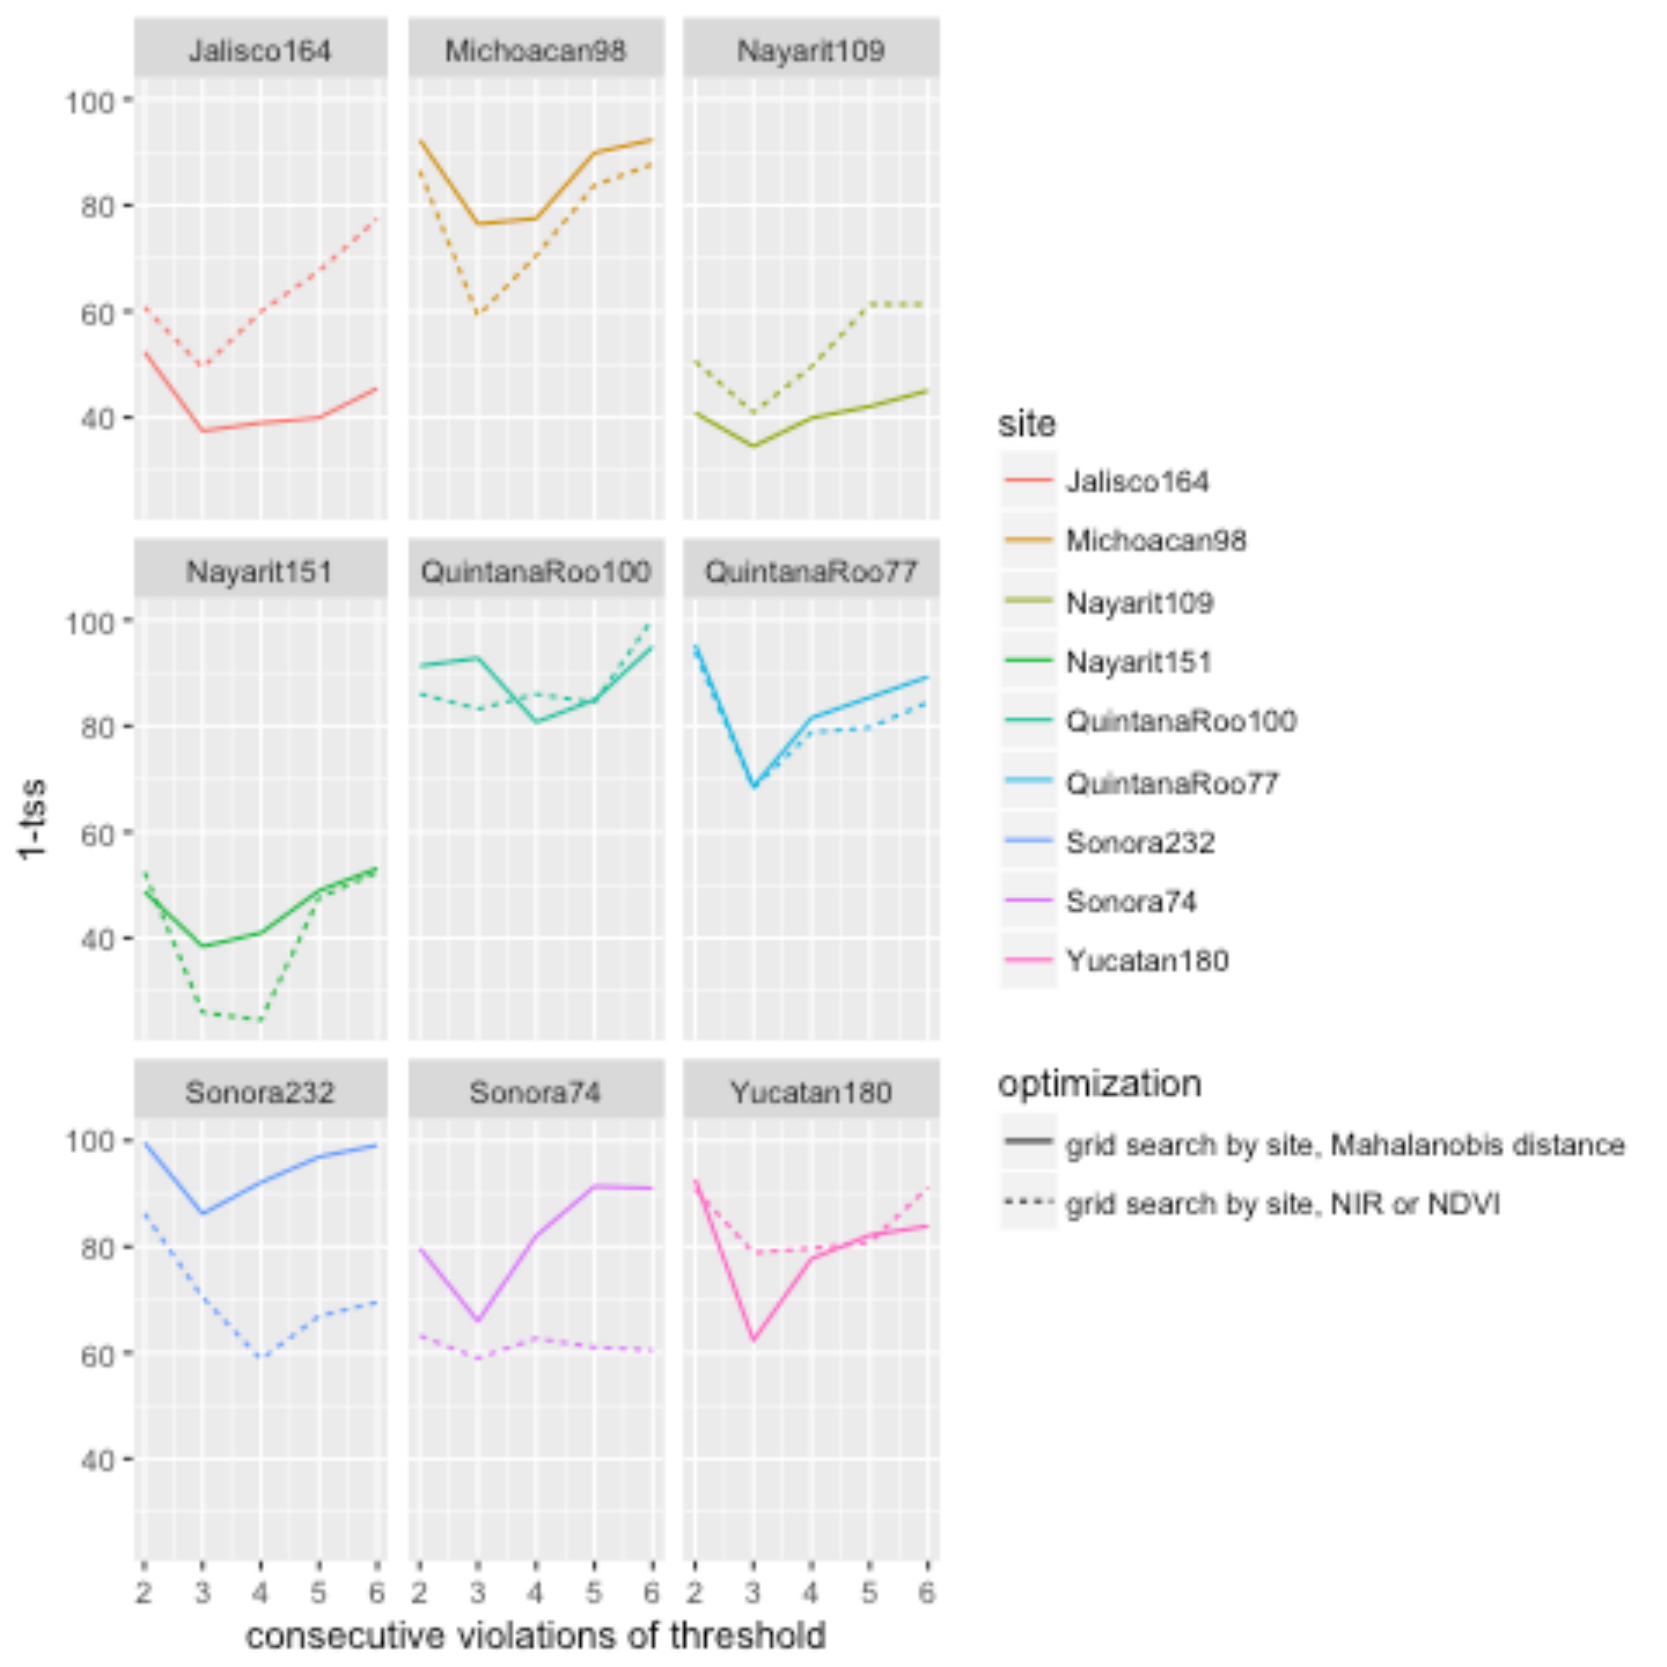} %<< no file extension
			  %%         --- .5\textwidth stands for 50% of text width
			  \caption[$1-tss$ results for each site trained separately. Results for optimal threshold for 3 consecutive violations.]%<<-- Legend for the list of figures at the beginning of you thesis
			  {$1-tss$ results for each site trained separately. Results for optimal threshold for 3 consecutive violations.}% legend displayed below the graph.
			  \label{fig:grdSrch_consecFix_mahl}
			\end{figure}

We include the figures showing site by site training of thresholds with Mahalanobis distance for all 9 sites .  

\subsection{Forest to water sites}

		\subsubsection{Sonora232}
		
		\begin{figure}[H]%--- Picture 'H'ere, 'B'ottom or 'T'op; '!' Try to
		                    %impose your will to LaTeX
		  \centering
		  \includegraphics[width=.5\textwidth]{./graphs/graphs_batch1_allPix_FINAL/_--_Mahl_dist_train_Sonora232} %<< no file extension
		  %%         --- .5\textwidth stands for 50% of text width
		  \caption[Grid search for optimal Mahalanobis distance threshold for Sonora232 site (training $1-tss$).]%<<-- Legend for the list of figures at the beginning of you thesis
		  {Grid search for optimal Mahalanobis distance threshold for Sonora232 site (training $1-tss$).}% legend displayed below the graph.
		  \label{fig:grdSrch_Sonora232_mahl}
		\end{figure}
		
		 \begin{figure}[H]
	      \begin{subfigure}{.5\textwidth}
	        \centering
	    	\includegraphics[width=1\textwidth]{./graphs/graphs_batch1_allPix_FINAL/_--_Mahl_dist_tss_CV_Sonora232} 
	        \caption{$1-tss$}
	        \label{fig:defo_pix}
	      \end{subfigure}%
	      \begin{subfigure}{.5\textwidth}
	        \centering
	        \includegraphics[width=1\textwidth]{./graphs/graphs_batch1_allPix_FINAL/_--_Mahl_dist_acc_CV_Sonora232}
	        \caption{$a_p$ and $a_u$}
	        \label{fig:non_defo_pix}
	      \end{subfigure}
	      %%         --- .5\textwidth stands for 50% of text width
	      \caption[Grid search for optimal Mahalanobis distance threshold for Sonora232 site (cross-validated $1-tss$, $a_p$ and $a_u$).]%<<-- Legend for the list of figures at the beginning of you thesis
	      {Grid search for optimal Mahalanobis distance threshold for Sonora232 site (cross-validated $1-tss$, $a_p$ and $a_u$).}% legend displayed below the graph.
	      \label{fig:grid_srch_cv_Sonora232_mahl}
	    \end{figure}
		
		\begin{figure}[H]%--- Picture 'H'ere, 'B'ottom or 'T'op; '!' Try to
		                    %impose your will to LaTeX
		  \centering
		  \includegraphics[width=.5\textwidth]{./graphs/graphs_batch1_allPix_FINAL/_--_Mahl_dist_train_consec3_raster_Sonora232} %<< no file extension
		  %%         --- .5\textwidth stands for 50% of text width
		  \caption[Spatial results for Sonora232 site of applying optimal threshold using 3 consecutive violation rule.]%<<-- Legend for the list of figures at the beginning of you thesis
		  {Spatial results for Sonora232 site of applying optimal threshold using 3 consecutive violation rule.}% legend displayed below the graph.
		  \label{fig:grdSrch_spatial_Sonora232_mahl}
		\end{figure}

		\subsubsection{Jalisco164}
		
		\begin{figure}[H]%--- Picture 'H'ere, 'B'ottom or 'T'op; '!' Try to
		                    %impose your will to LaTeX
		  \centering
		  \includegraphics[width=.5\textwidth]{./graphs/graphs_batch1_allPix_FINAL/_--_Mahl_dist_train_Jalisco164} %<< no file extension
		  %%         --- .5\textwidth stands for 50% of text width
		  \caption[Grid search for optimal Mahalanobis distance threshold for Jalisco164 site (training $1-tss$).]%<<-- Legend for the list of figures at the beginning of you thesis
		  {Grid search for optimal Mahalanobis distance threshold for Jalisco164 site (training $1-tss$).}% legend displayed below the graph.
		  \label{fig:grdSrch_Jalisco164_mahl}
		\end{figure}
		
		 \begin{figure}[H]
	      \begin{subfigure}{.5\textwidth}
	        \centering
	    	\includegraphics[width=1\textwidth]{./graphs/graphs_batch1_allPix_FINAL/_--_Mahl_dist_tss_CV_Jalisco164} 
	        \caption{$1-tss$}
	        \label{fig:defo_pix}
	      \end{subfigure}%
	      \begin{subfigure}{.5\textwidth}
	        \centering
	        \includegraphics[width=1\textwidth]{./graphs/graphs_batch1_allPix_FINAL/_--_Mahl_dist_acc_CV_Jalisco164}
	        \caption{$a_p$ and $a_u$}
	        \label{fig:non_defo_pix}
	      \end{subfigure}
	      %%         --- .5\textwidth stands for 50% of text width
	      \caption[Grid search for optimal Mahalanobis distance threshold for Jalisco164 site (cross-validated $1-tss$, $a_p$ and $a_u$).]%<<-- Legend for the list of figures at the beginning of you thesis
	      {Grid search for optimal Mahalanobis distance threshold for Jalisco164 site (cross-validated $1-tss$, $a_p$ and $a_u$).}% legend displayed below the graph.
	      \label{fig:grid_srch_cv_Jalisco164_mahl}
	    \end{figure}
		
		\begin{figure}[H]%--- Picture 'H'ere, 'B'ottom or 'T'op; '!' Try to
		                    %impose your will to LaTeX
		  \centering
		  \includegraphics[width=.5\textwidth]{./graphs/graphs_batch1_allPix_FINAL/_--_Mahl_dist_train_consec3_raster_Jalisco164} %<< no file extension
		  %%         --- .5\textwidth stands for 50% of text width
		  \caption[Spatial results for Jalisco164 site of applying optimal threshold using 3 consecutive violation rule.]%<<-- Legend for the list of figures at the beginning of you thesis
		  {Spatial results for Jalisco164 site of applying optimal threshold using 3 consecutive violation rule.}% legend displayed below the graph.
		  \label{fig:grdSrch_spatial_Jalisco164_mahl}
		\end{figure}
		
		\subsubsection{Nayarit151}
		
		\begin{figure}[H]%--- Picture 'H'ere, 'B'ottom or 'T'op; '!' Try to
		                    %impose your will to LaTeX
		  \centering
		  \includegraphics[width=.5\textwidth]{./graphs/graphs_batch1_allPix_FINAL/_--_Mahl_dist_train_Nayarit151} %<< no file extension
		  %%         --- .5\textwidth stands for 50% of text width
		  \caption[Grid search for optimal Mahalanobis distance threshold for Nayarit151 site (training $1-tss$).]%<<-- Legend for the list of figures at the beginning of you thesis
		  {Grid search for optimal Mahalanobis distance threshold for Nayarit151 site (training $1-tss$).}% legend displayed below the graph.
		  \label{fig:grdSrch_Nayarit151_mahl}
		\end{figure}
		
		 \begin{figure}[H]
	      \begin{subfigure}{.5\textwidth}
	        \centering
	    	\includegraphics[width=1\textwidth]{./graphs/graphs_batch1_allPix_FINAL/_--_Mahl_dist_tss_CV_Nayarit151} 
	        \caption{$1-tss$}
	        \label{fig:defo_pix}
	      \end{subfigure}%
	      \begin{subfigure}{.5\textwidth}
	        \centering
	        \includegraphics[width=1\textwidth]{./graphs/graphs_batch1_allPix_FINAL/_--_Mahl_dist_acc_CV_Nayarit151}
	        \caption{$a_p$ and $a_u$}
	        \label{fig:non_defo_pix}
	      \end{subfigure}
	      %%         --- .5\textwidth stands for 50% of text width
	      \caption[Grid search for optimal Mahalanobis distance threshold for Nayarit151 site (cross-validated $1-tss$, $a_p$ and $a_u$).]%<<-- Legend for the list of figures at the beginning of you thesis
	      {Grid search for optimal Mahalanobis distance threshold for Nayarit151 site (cross-validated $1-tss$, $a_p$ and $a_u$).}% legend displayed below the graph.
	      \label{fig:grid_srch_cv_Nayarit151_mahl}
	    \end{figure}
		
		\begin{figure}[H]%--- Picture 'H'ere, 'B'ottom or 'T'op; '!' Try to
		                    %impose your will to LaTeX
		  \centering
		  \includegraphics[width=.5\textwidth]{./graphs/graphs_batch1_allPix_FINAL/_--_Mahl_dist_train_consec3_raster_Nayarit151} %<< no file extension
		  %%         --- .5\textwidth stands for 50% of text width
		  \caption[Spatial results for Nayarit151 site of applying optimal threshold using 3 consecutive violation rule.]%<<-- Legend for the list of figures at the beginning of you thesis
		  {Spatial results for Nayarit151 site of applying optimal threshold using 3 consecutive violation rule.}% legend displayed below the graph.
		  \label{fig:grdSrch_spatial_Nayarit151_mahl}
		\end{figure}
		
		\subsubsection{Nayarit109}
		
		\begin{figure}[H]%--- Picture 'H'ere, 'B'ottom or 'T'op; '!' Try to
		                    %impose your will to LaTeX
		  \centering
		  \includegraphics[width=.5\textwidth]{./graphs/graphs_batch1_allPix_FINAL/_--_Mahl_dist_train_Nayarit109} %<< no file extension
		  %%         --- .5\textwidth stands for 50% of text width
		  \caption[Grid search for optimal Mahalanobis distance threshold for Nayarit109 site (training $1-tss$).]%<<-- Legend for the list of figures at the beginning of you thesis
		  {Grid search for optimal Mahalanobis distance threshold for Nayarit109 site (training $1-tss$).}% legend displayed below the graph.
		  \label{fig:grdSrch_Nayarit109_mahl}
		\end{figure}
		
		 \begin{figure}[H]
	      \begin{subfigure}{.5\textwidth}
	        \centering
	    	\includegraphics[width=1\textwidth]{./graphs/graphs_batch1_allPix_FINAL/_--_Mahl_dist_tss_CV_Nayarit109} 
	        \caption{$1-tss$}
	        \label{fig:defo_pix}
	      \end{subfigure}%
	      \begin{subfigure}{.5\textwidth}
	        \centering
	        \includegraphics[width=1\textwidth]{./graphs/graphs_batch1_allPix_FINAL/_--_Mahl_dist_acc_CV_Nayarit109}
	        \caption{$a_p$ and $a_u$}
	        \label{fig:non_defo_pix}
	      \end{subfigure}
	      %%         --- .5\textwidth stands for 50% of text width
	      \caption[Grid search for optimal Mahalanobis distance threshold for Nayarit109 site (cross-validated $1-tss$, $a_p$ and $a_u$).]%<<-- Legend for the list of figures at the beginning of you thesis
	      {Grid search for optimal Mahalanobis distance threshold for Nayarit109 site (cross-validated $1-tss$, $a_p$ and $a_u$).}% legend displayed below the graph.
	      \label{fig:grid_srch_cv_Nayarit109_mahl}
	    \end{figure}
		
		\begin{figure}[H]%--- Picture 'H'ere, 'B'ottom or 'T'op; '!' Try to
		                    %impose your will to LaTeX
		  \centering
		  \includegraphics[width=.5\textwidth]{./graphs/graphs_batch1_allPix_FINAL/_--_Mahl_dist_train_consec3_raster_Nayarit109} %<< no file extension
		  %%         --- .5\textwidth stands for 50% of text width
		  \caption[Spatial results for Nayarit109 site of applying optimal threshold using 3 consecutive violation rule.]%<<-- Legend for the list of figures at the beginning of you thesis
		  {Spatial results for Nayarit109 site of applying optimal threshold using 3 consecutive violation rule.}% legend displayed below the graph.
		  \label{fig:grdSrch_spatial_Nayarit109_mahl}
		\end{figure}

\subsection{Forest to urban or cropland sites}
		
		\subsubsection{Yucatan180}
		
		\begin{figure}[H]%--- Picture 'H'ere, 'B'ottom or 'T'op; '!' Try to
		                    %impose your will to LaTeX
		  \centering
		  \includegraphics[width=.5\textwidth]{./graphs/graphs_batch1_allPix_FINAL/_--_Mahl_dist_train_Yucatan180} %<< no file extension
		  %%         --- .5\textwidth stands for 50% of text width
		  \caption[Grid search for optimal Mahalanobis distance threshold for Yucatan180 site (training $1-tss$).]%<<-- Legend for the list of figures at the beginning of you thesis
		  {Grid search for optimal Mahalanobis distance threshold for Yucatan180 site (training $1-tss$).}% legend displayed below the graph.
		  \label{fig:grdSrch_Yucatan180_mahl}
		\end{figure}
		
		 \begin{figure}[H]
	      \begin{subfigure}{.5\textwidth}
	        \centering
	    	\includegraphics[width=1\textwidth]{./graphs/graphs_batch1_allPix_FINAL/_--_Mahl_dist_tss_CV_Yucatan180} 
	        \caption{$1-tss$}
	        \label{fig:defo_pix}
	      \end{subfigure}%
	      \begin{subfigure}{.5\textwidth}
	        \centering
	        \includegraphics[width=1\textwidth]{./graphs/graphs_batch1_allPix_FINAL/_--_Mahl_dist_acc_CV_Yucatan180}
	        \caption{$a_p$ and $a_u$}
	        \label{fig:non_defo_pix}
	      \end{subfigure}
	      %%         --- .5\textwidth stands for 50% of text width
	      \caption[Grid search for optimal Mahalanobis distance threshold for Yucatan180 site (cross-validated $1-tss$, $a_p$ and $a_u$).]%<<-- Legend for the list of figures at the beginning of you thesis
	      {Grid search for optimal Mahalanobis distance threshold for Yucatan180 site (cross-validated $1-tss$, $a_p$ and $a_u$).}% legend displayed below the graph.
	      \label{fig:grid_srch_cv_Yucatan180_mahl}
	    \end{figure}
		
		\begin{figure}[H]%--- Picture 'H'ere, 'B'ottom or 'T'op; '!' Try to
		                    %impose your will to LaTeX
		  \centering
		  \includegraphics[width=.5\textwidth]{./graphs/graphs_batch1_allPix_FINAL/_--_Mahl_dist_train_consec3_raster_Yucatan180} %<< no file extension
		  %%         --- .5\textwidth stands for 50% of text width
		  \caption[Spatial results for Yucatan180 site of applying optimal threshold using 3 consecutive violation rule.]%<<-- Legend for the list of figures at the beginning of you thesis
		  {Spatial results for Yucatan180 site of applying optimal threshold using 3 consecutive violation rule.}% legend displayed below the graph.
		  \label{fig:grdSrch_spatial_Yucatan180_mahl}
		\end{figure}

		\subsubsection{QuintanaRoo100}
		
		\begin{figure}[H]%--- Picture 'H'ere, 'B'ottom or 'T'op; '!' Try to
		                    %impose your will to LaTeX
		  \centering
		  \includegraphics[width=.5\textwidth]{./graphs/graphs_batch1_allPix_FINAL/_--_Mahl_dist_train_QuintanaRoo100} %<< no file extension
		  %%         --- .5\textwidth stands for 50% of text width
		  \caption[Grid search for optimal Mahalanobis distance threshold for QuintanaRoo100 site (training $1-tss$).]%<<-- Legend for the list of figures at the beginning of you thesis
		  {Grid search for optimal Mahalanobis distance threshold for QuintanaRoo100 site (training $1-tss$).}% legend displayed below the graph.
		  \label{fig:grdSrch_QuintanaRoo100_mahl}
		\end{figure}
		
		 \begin{figure}[H]
	      \begin{subfigure}{.5\textwidth}
	        \centering
	    	\includegraphics[width=1\textwidth]{./graphs/graphs_batch1_allPix_FINAL/_--_Mahl_dist_tss_CV_QuintanaRoo100} 
	        \caption{$1-tss$}
	        \label{fig:defo_pix}
	      \end{subfigure}%
	      \begin{subfigure}{.5\textwidth}
	        \centering
	        \includegraphics[width=1\textwidth]{./graphs/graphs_batch1_allPix_FINAL/_--_Mahl_dist_acc_CV_QuintanaRoo100}
	        \caption{$a_p$ and $a_u$}
	        \label{fig:non_defo_pix}
	      \end{subfigure}
	      %%         --- .5\textwidth stands for 50% of text width
	      \caption[Grid search for optimal Mahalanobis distance threshold for QuintanaRoo100 site (cross-validated $1-tss$, $a_p$ and $a_u$).]%<<-- Legend for the list of figures at the beginning of you thesis
	      {Grid search for optimal Mahalanobis distance threshold for QuintanaRoo100 site (cross-validated $1-tss$, $a_p$ and $a_u$).}% legend displayed below the graph.
	      \label{fig:grid_srch_cv_QuintanaRoo100_mahl}
	    \end{figure}
		
		\begin{figure}[H]%--- Picture 'H'ere, 'B'ottom or 'T'op; '!' Try to
		                    %impose your will to LaTeX
		  \centering
		  \includegraphics[width=.5\textwidth]{./graphs/graphs_batch1_allPix_FINAL/_--_Mahl_dist_train_consec3_raster_QuintanaRoo100} %<< no file extension
		  %%         --- .5\textwidth stands for 50% of text width
		  \caption[Spatial results for QuintanaRoo100 site of applying optimal threshold using 3 consecutive violation rule.]%<<-- Legend for the list of figures at the beginning of you thesis
		  {Spatial results for QuintanaRoo100 site of applying optimal threshold using 3 consecutive violation rule.}% legend displayed below the graph.
		  \label{fig:grdSrch_spatial_QuintanaRoo100_mahl}
		\end{figure}

		\subsubsection{Michoacan98}
		
		\begin{figure}[H]%--- Picture 'H'ere, 'B'ottom or 'T'op; '!' Try to
		                    %impose your will to LaTeX
		  \centering
		  \includegraphics[width=.5\textwidth]{./graphs/graphs_batch1_allPix_FINAL/_--_Mahl_dist_train_Michoacan98} %<< no file extension
		  %%         --- .5\textwidth stands for 50% of text width
		  \caption[Grid search for optimal Mahalanobis distance threshold for Michoacan98 site (training $1-tss$).]%<<-- Legend for the list of figures at the beginning of you thesis
		  {Grid search for optimal Mahalanobis distance threshold for Michoacan98 site (training $1-tss$).}% legend displayed below the graph.
		  \label{fig:grdSrch_Michoacan98_mahl}
		\end{figure}
		
		 \begin{figure}[H]
	      \begin{subfigure}{.5\textwidth}
	        \centering
	    	\includegraphics[width=1\textwidth]{./graphs/graphs_batch1_allPix_FINAL/_--_Mahl_dist_tss_CV_Michoacan98} 
	        \caption{$1-tss$}
	        \label{fig:defo_pix}
	      \end{subfigure}%
	      \begin{subfigure}{.5\textwidth}
	        \centering
	        \includegraphics[width=1\textwidth]{./graphs/graphs_batch1_allPix_FINAL/_--_Mahl_dist_acc_CV_Michoacan98}
	        \caption{$a_p$ and $a_u$}
	        \label{fig:non_defo_pix}
	      \end{subfigure}
	      %%         --- .5\textwidth stands for 50% of text width
	      \caption[Grid search for optimal Mahalanobis distance threshold for Michoacan98 site (cross-validated $1-tss$, $a_p$ and $a_u$).]%<<-- Legend for the list of figures at the beginning of you thesis
	      {Grid search for optimal Mahalanobis distance threshold for Michoacan98 site (cross-validated $1-tss$, $a_p$ and $a_u$).}% legend displayed below the graph.
	      \label{fig:grid_srch_cv_Michoacan98_mahl}
	    \end{figure}
		
		\begin{figure}[H]%--- Picture 'H'ere, 'B'ottom or 'T'op; '!' Try to
		                    %impose your will to LaTeX
		  \centering
		  \includegraphics[width=.5\textwidth]{./graphs/graphs_batch1_allPix_FINAL/_--_Mahl_dist_train_consec3_raster_Michoacan98} %<< no file extension
		  %%         --- .5\textwidth stands for 50% of text width
		  \caption[Spatial results for Michoacan98 site of applying optimal threshold using 3 consecutive violation rule.]%<<-- Legend for the list of figures at the beginning of you thesis
		  {Spatial results for Michoacan98 site of applying optimal threshold using 3 consecutive violation rule.}% legend displayed below the graph.
		  \label{fig:grdSrch_spatial_Michoacan98_mahl}
		\end{figure}

		\subsubsection{QuintanaRoo77}
			
		\begin{figure}[H]%--- Picture 'H'ere, 'B'ottom or 'T'op; '!' Try to
		                    %impose your will to LaTeX
		  \centering
		  \includegraphics[width=.5\textwidth]{./graphs/graphs_batch1_allPix_FINAL/_--_Mahl_dist_train_QuintanaRoo77} %<< no file extension
		  %%         --- .5\textwidth stands for 50% of text width
		  \caption[Grid search for optimal Mahalanobis distance threshold for QuintanaRoo77 site (training $1-tss$).]%<<-- Legend for the list of figures at the beginning of you thesis
		  {Grid search for optimal Mahalanobis distance threshold for QuintanaRoo77 site (training $1-tss$).}% legend displayed below the graph.
		  \label{fig:grdSrch_QuintanaRoo77_mahl}
		\end{figure}
		
		 \begin{figure}[H]
	      \begin{subfigure}{.5\textwidth}
	        \centering
	    	\includegraphics[width=1\textwidth]{./graphs/graphs_batch1_allPix_FINAL/_--_Mahl_dist_tss_CV_QuintanaRoo77} 
	        \caption{$1-tss$}
	        \label{fig:defo_pix}
	      \end{subfigure}%
	      \begin{subfigure}{.5\textwidth}
	        \centering
	        \includegraphics[width=1\textwidth]{./graphs/graphs_batch1_allPix_FINAL/_--_Mahl_dist_acc_CV_QuintanaRoo77}
	        \caption{$a_p$ and $a_u$}
	        \label{fig:non_defo_pix}
	      \end{subfigure}
	      %%         --- .5\textwidth stands for 50% of text width
	      \caption[Grid search for optimal Mahalanobis distance threshold for QuintanaRoo77 site (cross-validated $1-tss$, $a_p$ and $a_u$).]%<<-- Legend for the list of figures at the beginning of you thesis
	      {Grid search for optimal Mahalanobis distance threshold for QuintanaRoo77 site (cross-validated $1-tss$, $a_p$ and $a_u$).}% legend displayed below the graph.
	      \label{fig:grid_srch_cv_QuintanaRoo77_mahl}
	    \end{figure}
		
		\begin{figure}[H]%--- Picture 'H'ere, 'B'ottom or 'T'op; '!' Try to
		                    %impose your will to LaTeX
		  \centering
		  \includegraphics[width=.5\textwidth]{./graphs/graphs_batch1_allPix_FINAL/_--_Mahl_dist_train_consec3_raster_QuintanaRoo77} %<< no file extension
		  %%         --- .5\textwidth stands for 50% of text width
		  \caption[Spatial results for QuintanaRoo77 site of applying optimal threshold using 3 consecutive violation rule.]%<<-- Legend for the list of figures at the beginning of you thesis
		  {Spatial results for QuintanaRoo77 site of applying optimal threshold using 3 consecutive violation rule.}% legend displayed below the graph.
		  \label{fig:grdSrch_spatial_QuintanaRoo77_mahl}
		\end{figure}

		\subsubsection{Sonora74}
		
		\begin{figure}[H]%--- Picture 'H'ere, 'B'ottom or 'T'op; '!' Try to
		                    %impose your will to LaTeX
		  \centering
		  \includegraphics[width=.5\textwidth]{./graphs/graphs_batch1_allPix_FINAL/_--_Mahl_dist_train_Sonora74} %<< no file extension
		  %%         --- .5\textwidth stands for 50% of text width
		  \caption[Grid search for optimal Mahalanobis distance threshold for Sonora74 site (training $1-tss$).]%<<-- Legend for the list of figures at the beginning of you thesis
		  {Grid search for optimal Mahalanobis distance threshold for Sonora74 site (training $1-tss$).}% legend displayed below the graph.
		  \label{fig:grdSrch_Sonora74_mahl}
		\end{figure}
		
		 \begin{figure}[H]
	      \begin{subfigure}{.5\textwidth}
	        \centering
	    	\includegraphics[width=1\textwidth]{./graphs/graphs_batch1_allPix_FINAL/_--_Mahl_dist_tss_CV_Sonora74} 
	        \caption{$1-tss$}
	        \label{fig:defo_pix}
	      \end{subfigure}%
	      \begin{subfigure}{.5\textwidth}
	        \centering
	        \includegraphics[width=1\textwidth]{./graphs/graphs_batch1_allPix_FINAL/_--_Mahl_dist_acc_CV_Sonora74}
	        \caption{$a_p$ and $a_u$}
	        \label{fig:non_defo_pix}
	      \end{subfigure}
	      %%         --- .5\textwidth stands for 50% of text width
	      \caption[Grid search for optimal Mahalanobis distance threshold for Sonora74 site (cross-validated $1-tss$, $a_p$ and $a_u$).]%<<-- Legend for the list of figures at the beginning of you thesis
	      {Grid search for optimal Mahalanobis distance threshold for Sonora74 site (cross-validated $1-tss$, $a_p$ and $a_u$).}% legend displayed below the graph.
	      \label{fig:grid_srch_cv_Sonora74_mahl}
	    \end{figure}
		
		\begin{figure}[H]%--- Picture 'H'ere, 'B'ottom or 'T'op; '!' Try to
		                    %impose your will to LaTeX
		  \centering
		  \includegraphics[width=.5\textwidth]{./graphs/graphs_batch1_allPix_FINAL/_--_Mahl_dist_train_consec3_raster_Sonora74} %<< no file extension
		  %%         --- .5\textwidth stands for 50% of text width
		  \caption[Spatial results for Sonora74 site of applying optimal threshold using 3 consecutive violation rule.]%<<-- Legend for the list of figures at the beginning of you thesis
		  {Spatial results for Sonora74 site of applying optimal threshold using 3 consecutive violation rule.}% legend displayed below the graph.
		  \label{fig:grdSrch_spatial_Sonora74_mahl}
		\end{figure}
